# Supplementary material for: Lightweight Data Fusion with Conjugate Mappings
Source: arXiv:2011.10607 source file (2020-11-20)
Supplement: Supplementary file 1 [file appendix_homicide_distributions.tex]

\subsection*{Additional Results}

\subsubsection*{Latent Variable Posterior Distributions}

The latent variable posterior distributions $p(\theta_i \given x; \phi)$ are presented in Figures~\ref{fig-posteriors-homicide-largest} to \ref{fig-posteriors-homicide-smallest}. 
In each, the LDF posterior (red) and gamma-Poisson regression posterior (blue) are gamma-distributions; the posterior in Poisson regression (purple) is shown as a Dirac delta centered on the predicted mean. The LDF-MM posterior (gray) is a weighted sum of component gamma-distributions. The first figure represents counties with the largest population for their given state, the second are counties with median populations, and the third are counties with the lowest populations by state.

We observe that LDF often extracts more information from the auxiliary data than gamma-Poisson regression and Poisson regression and is thus able to obtain more confident posterior distributions when the distribution is skewed away from zero.

\subsubsection*{Posterior Predictive Distributions}

Here we provide the posterior predictive distributions for the primary data.  For each county, shown in the upper-right corner, the distributions are predicted by models that are \textit{not} trained on data from that county.

The posterior predictive distributions
\begin{align}
	p(y_i \given x; \phi) = \int p(y_i \given \theta_i) p(\theta_i \given x; \phi) \dif\theta_i
\end{align}
are presented Figures~\ref{fig-predictives-homicide-largest} to \ref{fig-predictives-homicide-smallest}. In each, the LDF predictive (red) and gamma-Poisson regression posterior predictive (blue) are gamma-Poisson distributions; the Poisson regression posterior predictive (purple) is Poisson-distributed. The LDF-MM posterior (gray) is a weighted sum of component gamma-Poisson-distributions. The observed data is shown by the black vertical line.

%%%%%%%%%%%%%%%%%%%%%%%%%%%%%%%%%%%%%%%%%%%%%%%%%%%%%%%%
%%%%%%%%%%%%%%%%%%%%%%%%%%%%%%%%%%%%%%%%%%%%%%%%%%%%%%%%
% Homicides
%%%%%%%%%%%%%%%%%%%%%%%%%%%%%%%%%%%%%%%%%%%%%%%%%%%%%%%%
%%%%%%%%%%%%%%%%%%%%%%%%%%%%%%%%%%%%%%%%%%%%%%%%%%%%%%%%
%largest posterior
\begin{figure}[t]
	\vskip 0.1in
	\begin{center}
		\begin{subfigure}[b]{\textwidth}
			\centering
			\includegraphics[width=\linewidth, trim={0cm 0cm 0cm 0cm},clip]{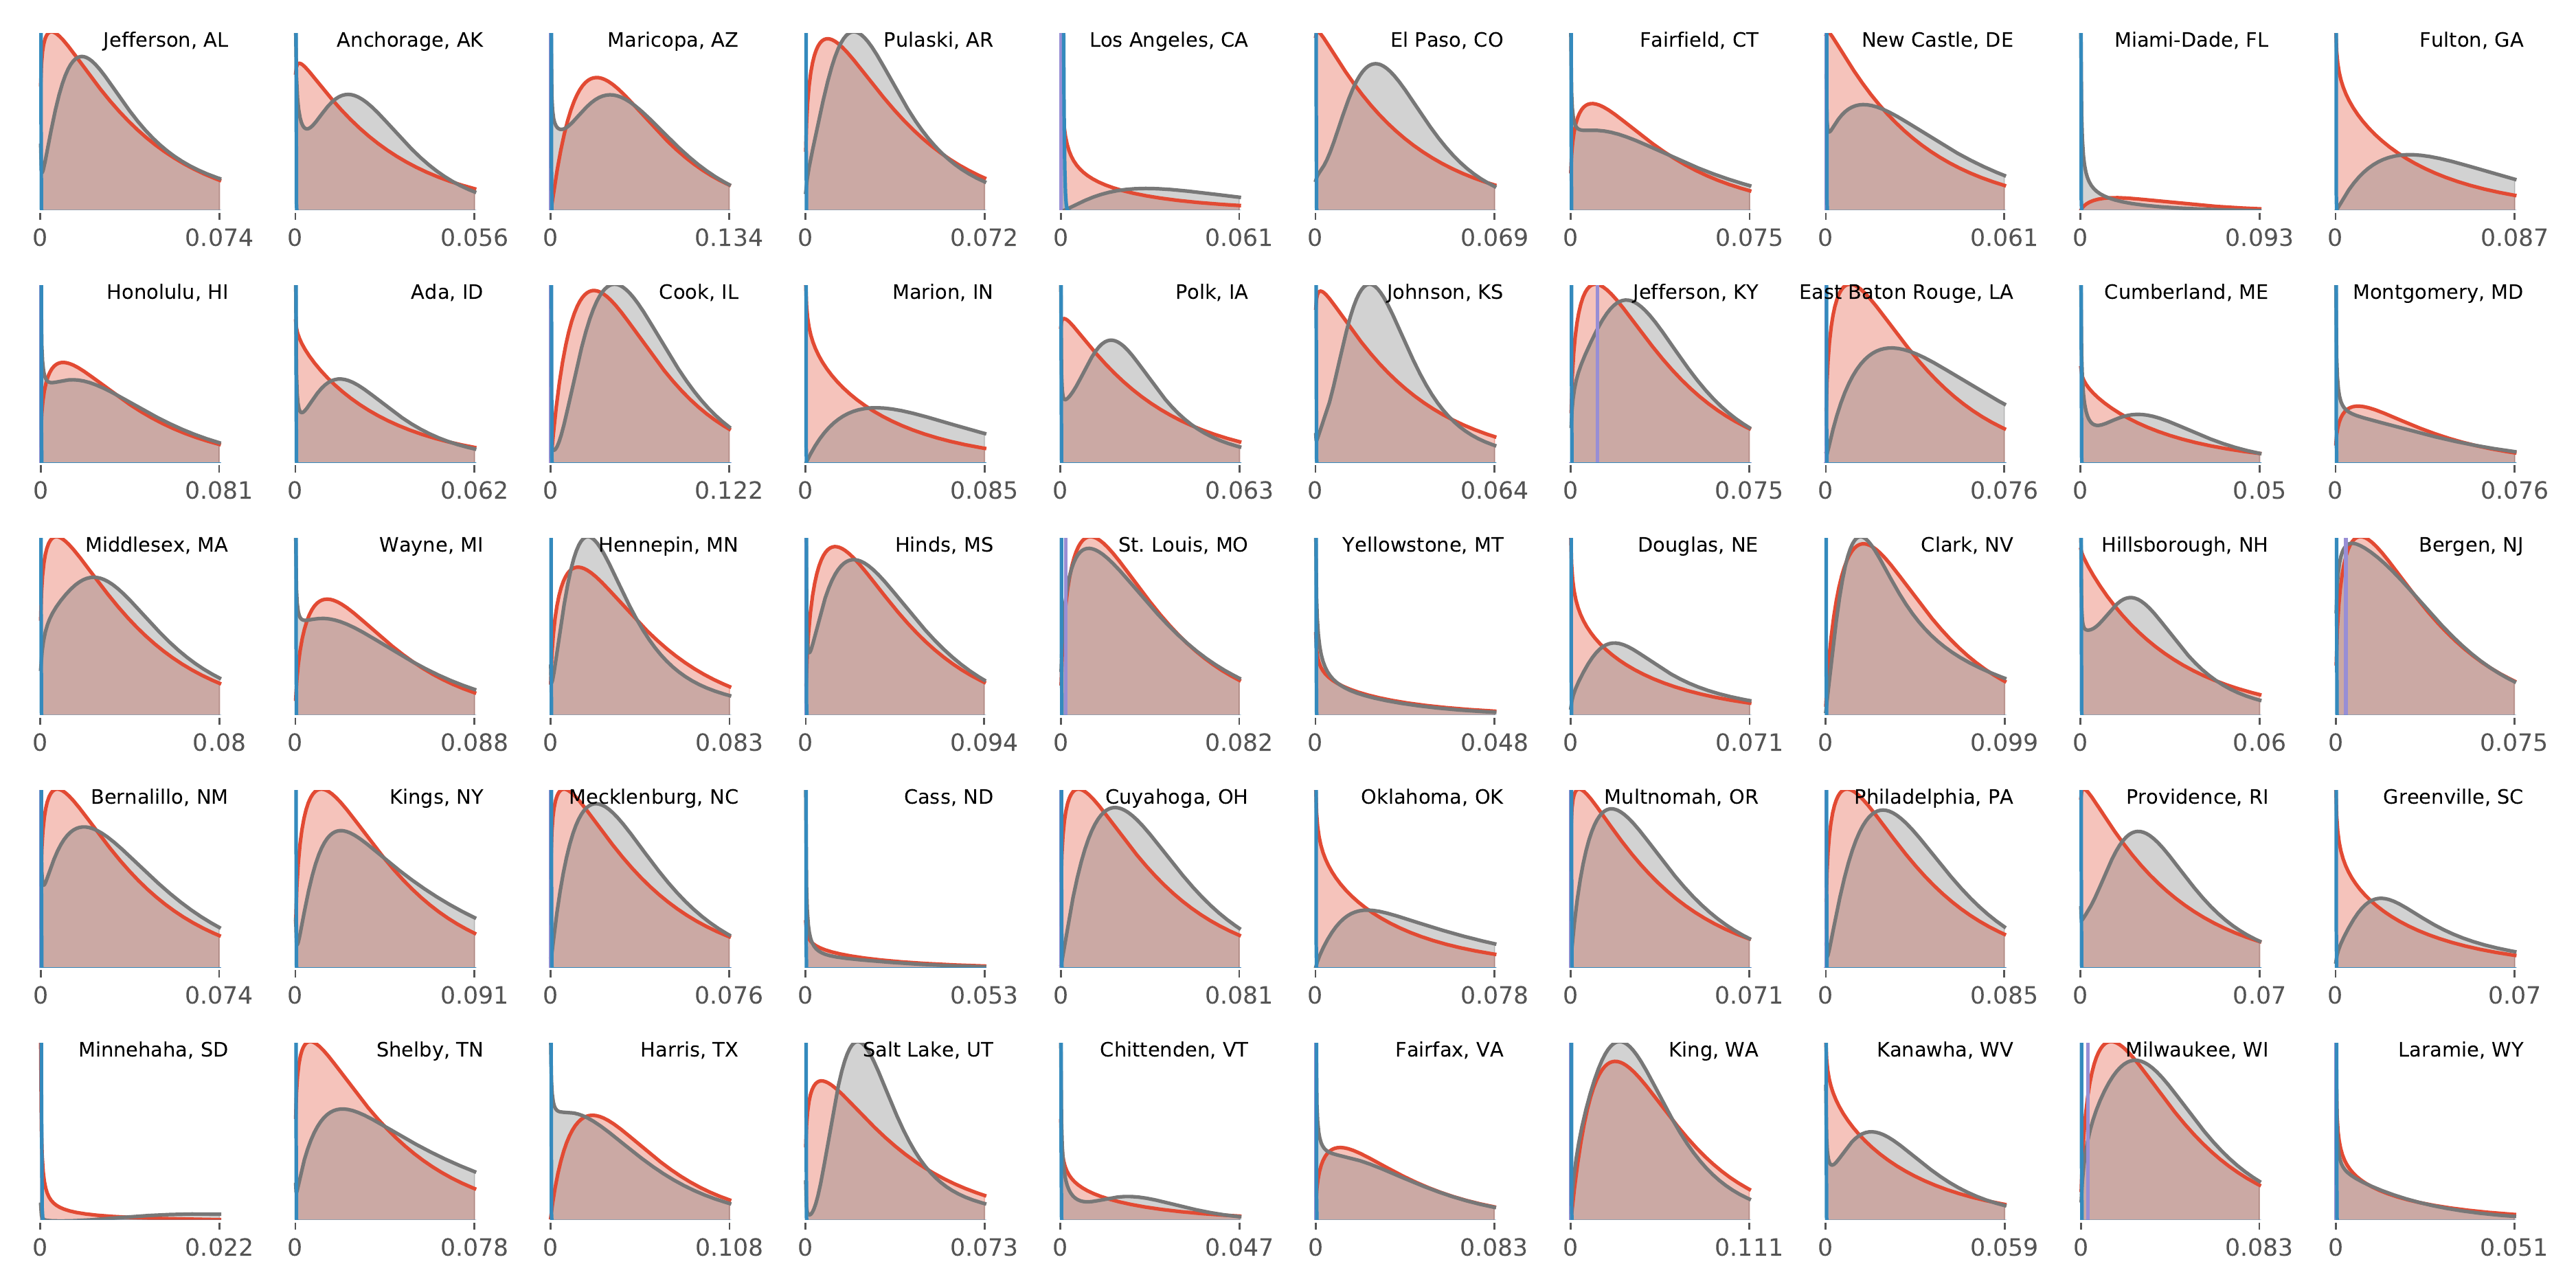}
		\end{subfigure}
		\caption{\small \textbf{Sample posterior distributions for homicide}. Posteriors $p(\theta_i|x_i;\phi)$ on homicide rates are shown for one county per state. 
			Distributions corresponding to LDF are in red, LDF-MM in gray, gamma-Poisson regression in blue, and Poisson regression in purple.
			The counties displayed are those with the largest population for their given state.} 
		\label{fig-posteriors-homicide-largest}
	\end{center}
	\vspace*{-5mm}
\end{figure}

%median posterior
\begin{figure}[t]
	\vskip 0.1in
	\begin{center}
		\begin{subfigure}[b]{\textwidth}
			\centering
			\includegraphics[width=\linewidth, trim={0cm 0cm 0cm 0cm},clip]{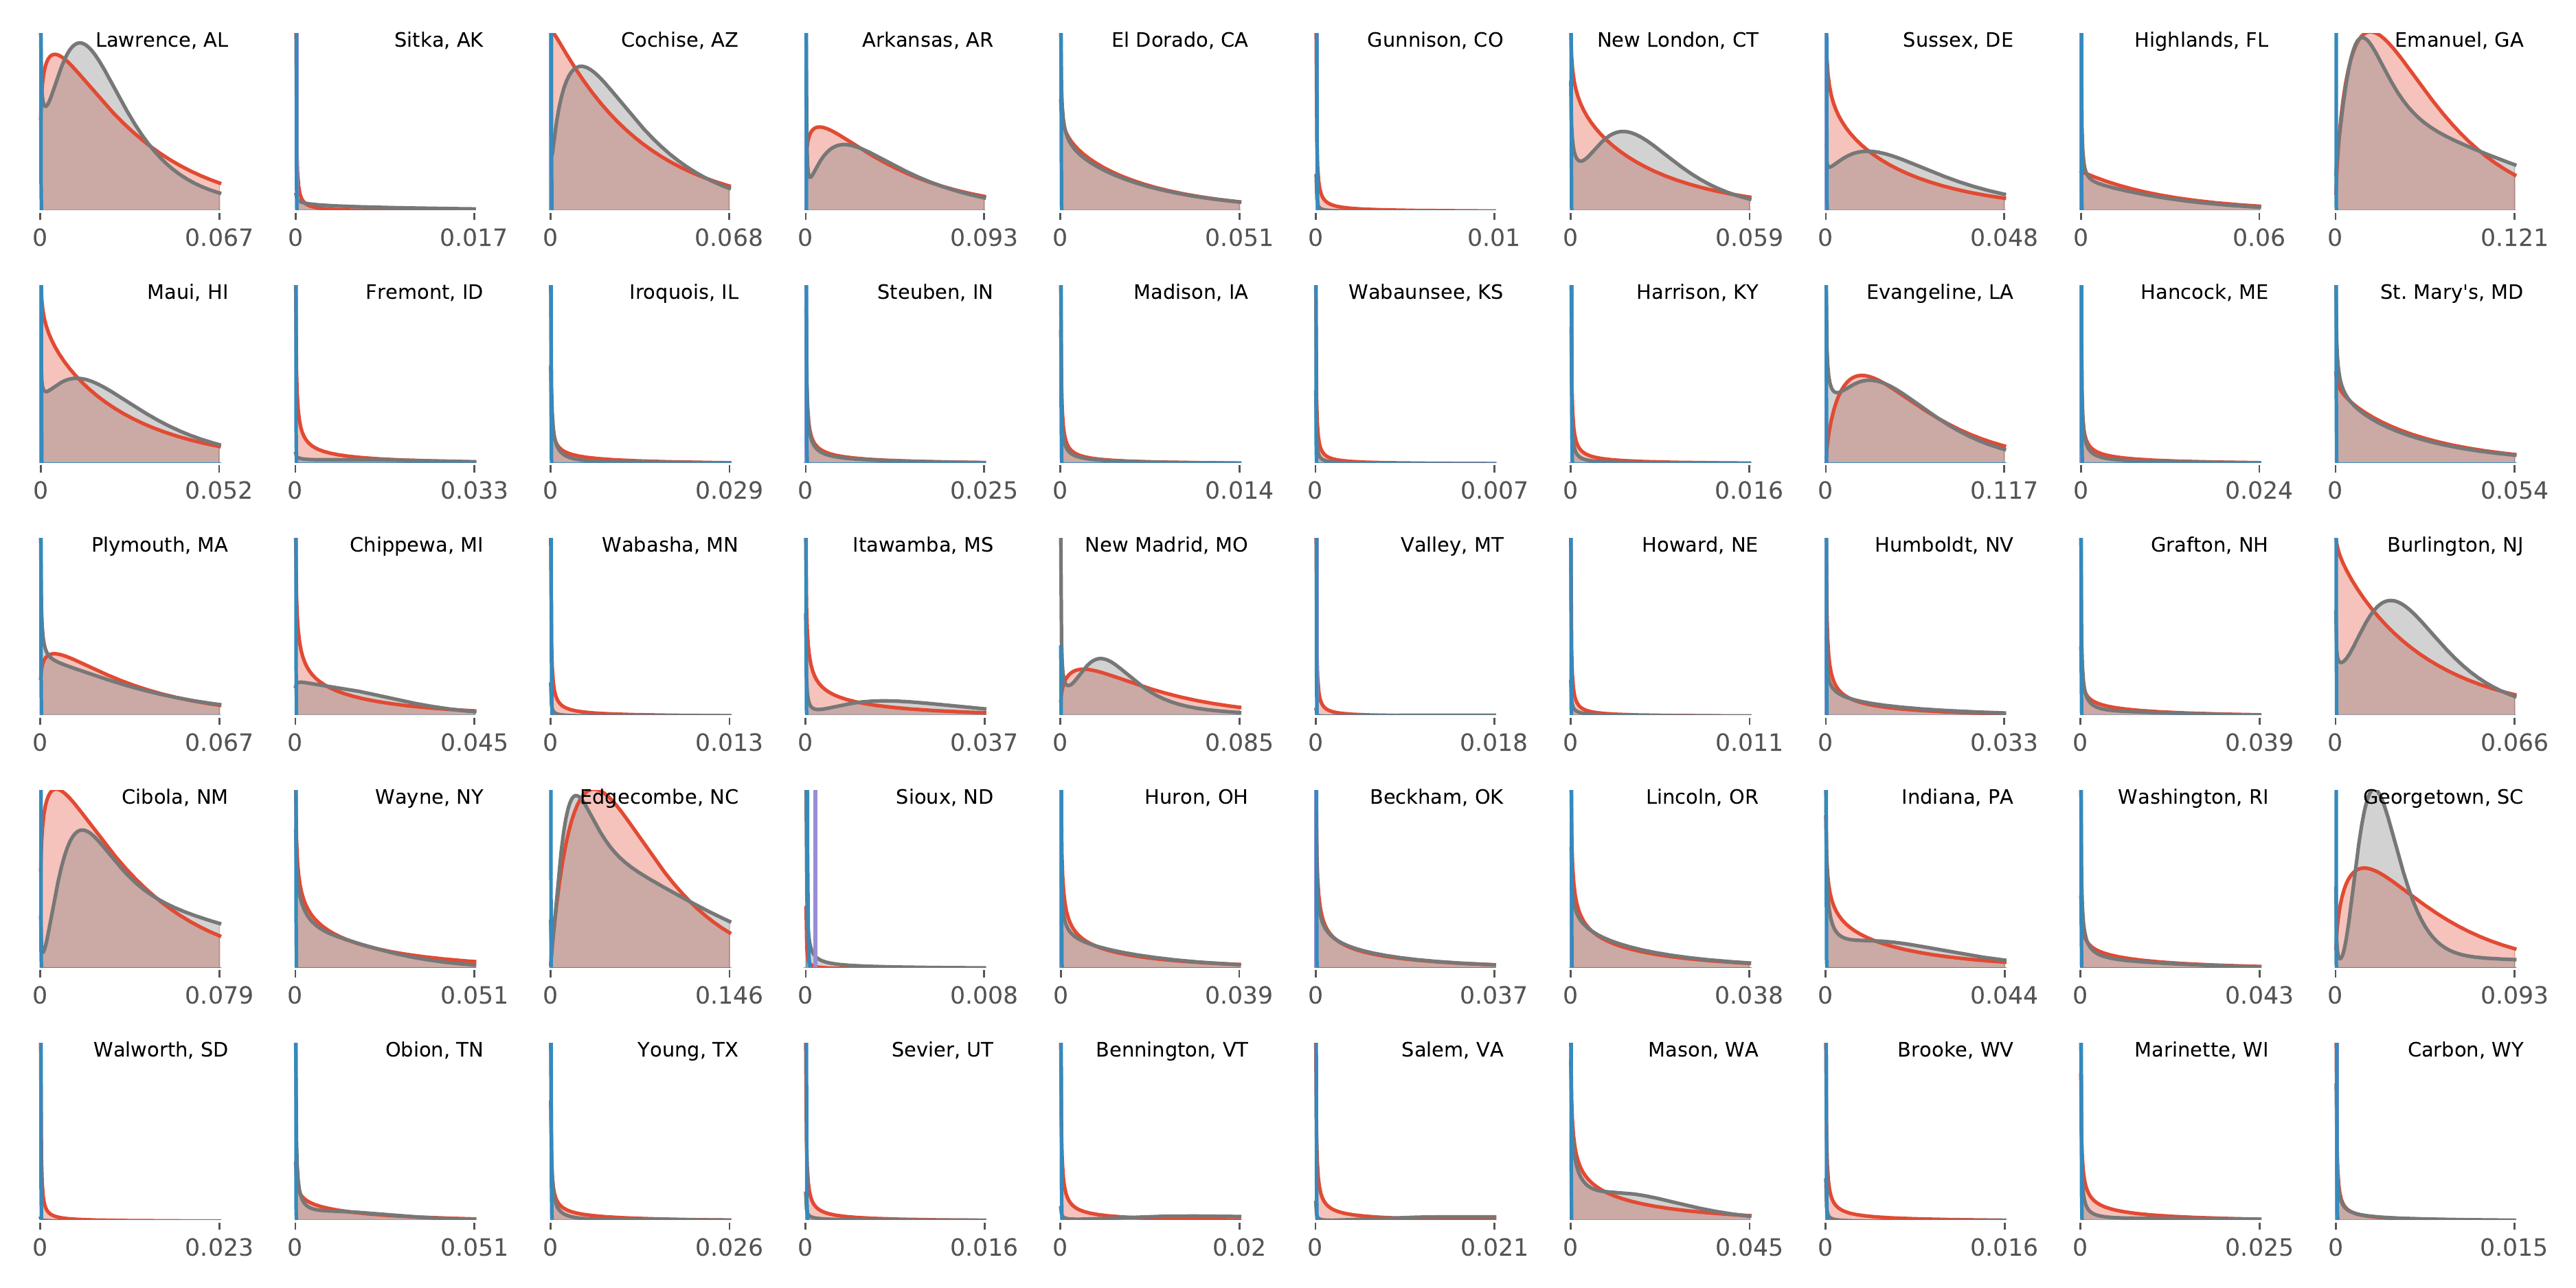}
		\end{subfigure}
		\caption{\small \textbf{Sample posterior distributions for homicide}. Posteriors $p(\theta_i|x_i;\phi)$ on homicide rates are shown for one county per state. 
			Distributions corresponding to LDF are in red, LDF-MM in gray, gamma-Poisson regression in blue, and Poisson regression in purple.
			The counties displayed are those with median populations for their given state.} 
		\label{fig-posteriors-homicide-median}
	\end{center}
	\vspace*{-5mm}
\end{figure}

%smallest posterior
\begin{figure}[t]
	\vskip 0.1in
	\begin{center}
		\begin{subfigure}[b]{\textwidth}
			\centering
			\includegraphics[width=\linewidth, trim={0cm 0cm 0cm 0cm},clip]{figures/crime_distributions/20200610_posteriors/posteriors_median_MURDER.pdf}
		\end{subfigure}
		\caption{\small \textbf{Sample posterior distributions for homicide}. Posteriors $p(\theta_i|x_i;\phi)$ on homicide rates are shown for one county per state. 
			Distributions corresponding to LDF are in red, LDF-MM in gray, gamma-Poisson regression in blue, and Poisson regression in purple.
			The counties displayed are those with the smallest population for their given state.} 
		\label{fig-posteriors-homicide-smallest}
	\end{center}
	\vspace*{-5mm}
\end{figure}

%largest predictive
\begin{figure}[t]
	\vskip 0.1in
	\begin{center}
		\begin{subfigure}[b]{\textwidth}
			\centering
			\includegraphics[width=\linewidth, trim={0cm 0cm 0cm 0cm},clip]{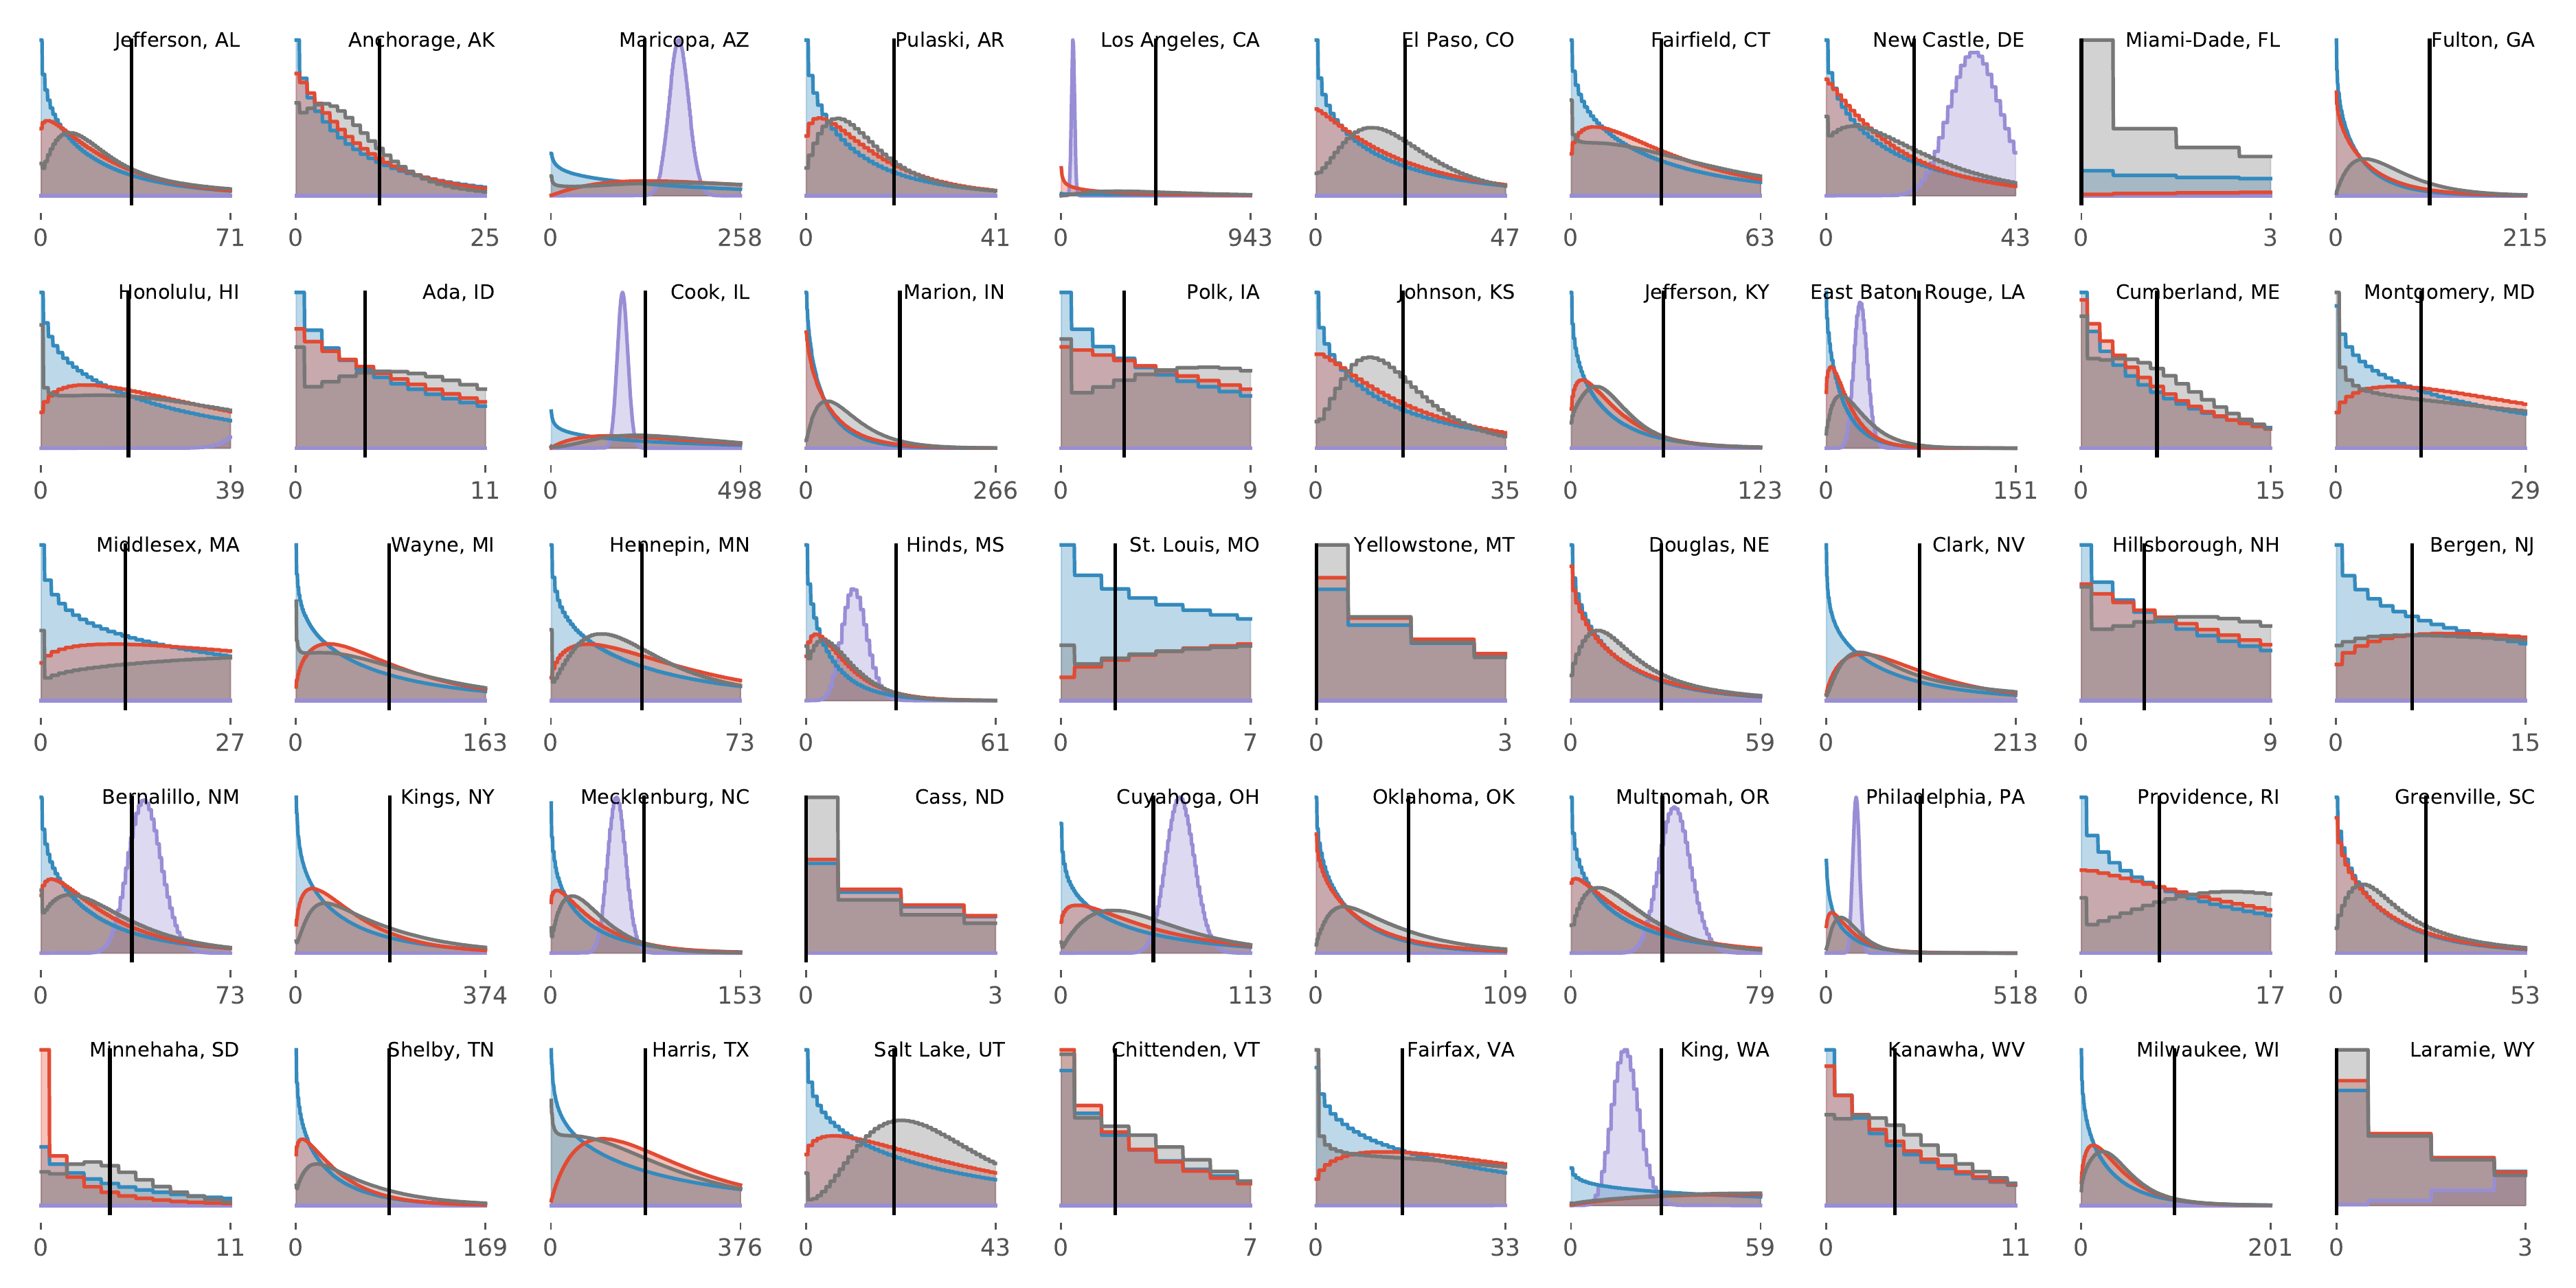}
		\end{subfigure}
		\caption{\small \textbf{Sample predictive distributions for homicide}. Predictive distributions $p(y_i|x_i;\phi)$ on homicide rates are shown for one county per state. 
			Distributions corresponding to LDF are in red, LDF-MM in gray, gamma-Poisson regression in blue, and Poisson regression in purple. The empirical rate is shown by the black line.
			The counties displayed are those with the largest population for their given state.} 
		\label{fig-predictives-homicide-largest}
	\end{center}
	\vspace*{-5mm}
\end{figure}

%median posterior
\begin{figure}[t]
	\vskip 0.1in
	\begin{center}
		\begin{subfigure}[b]{\textwidth}
			\centering
			\includegraphics[width=\linewidth, trim={0cm 0cm 0cm 0cm},clip]{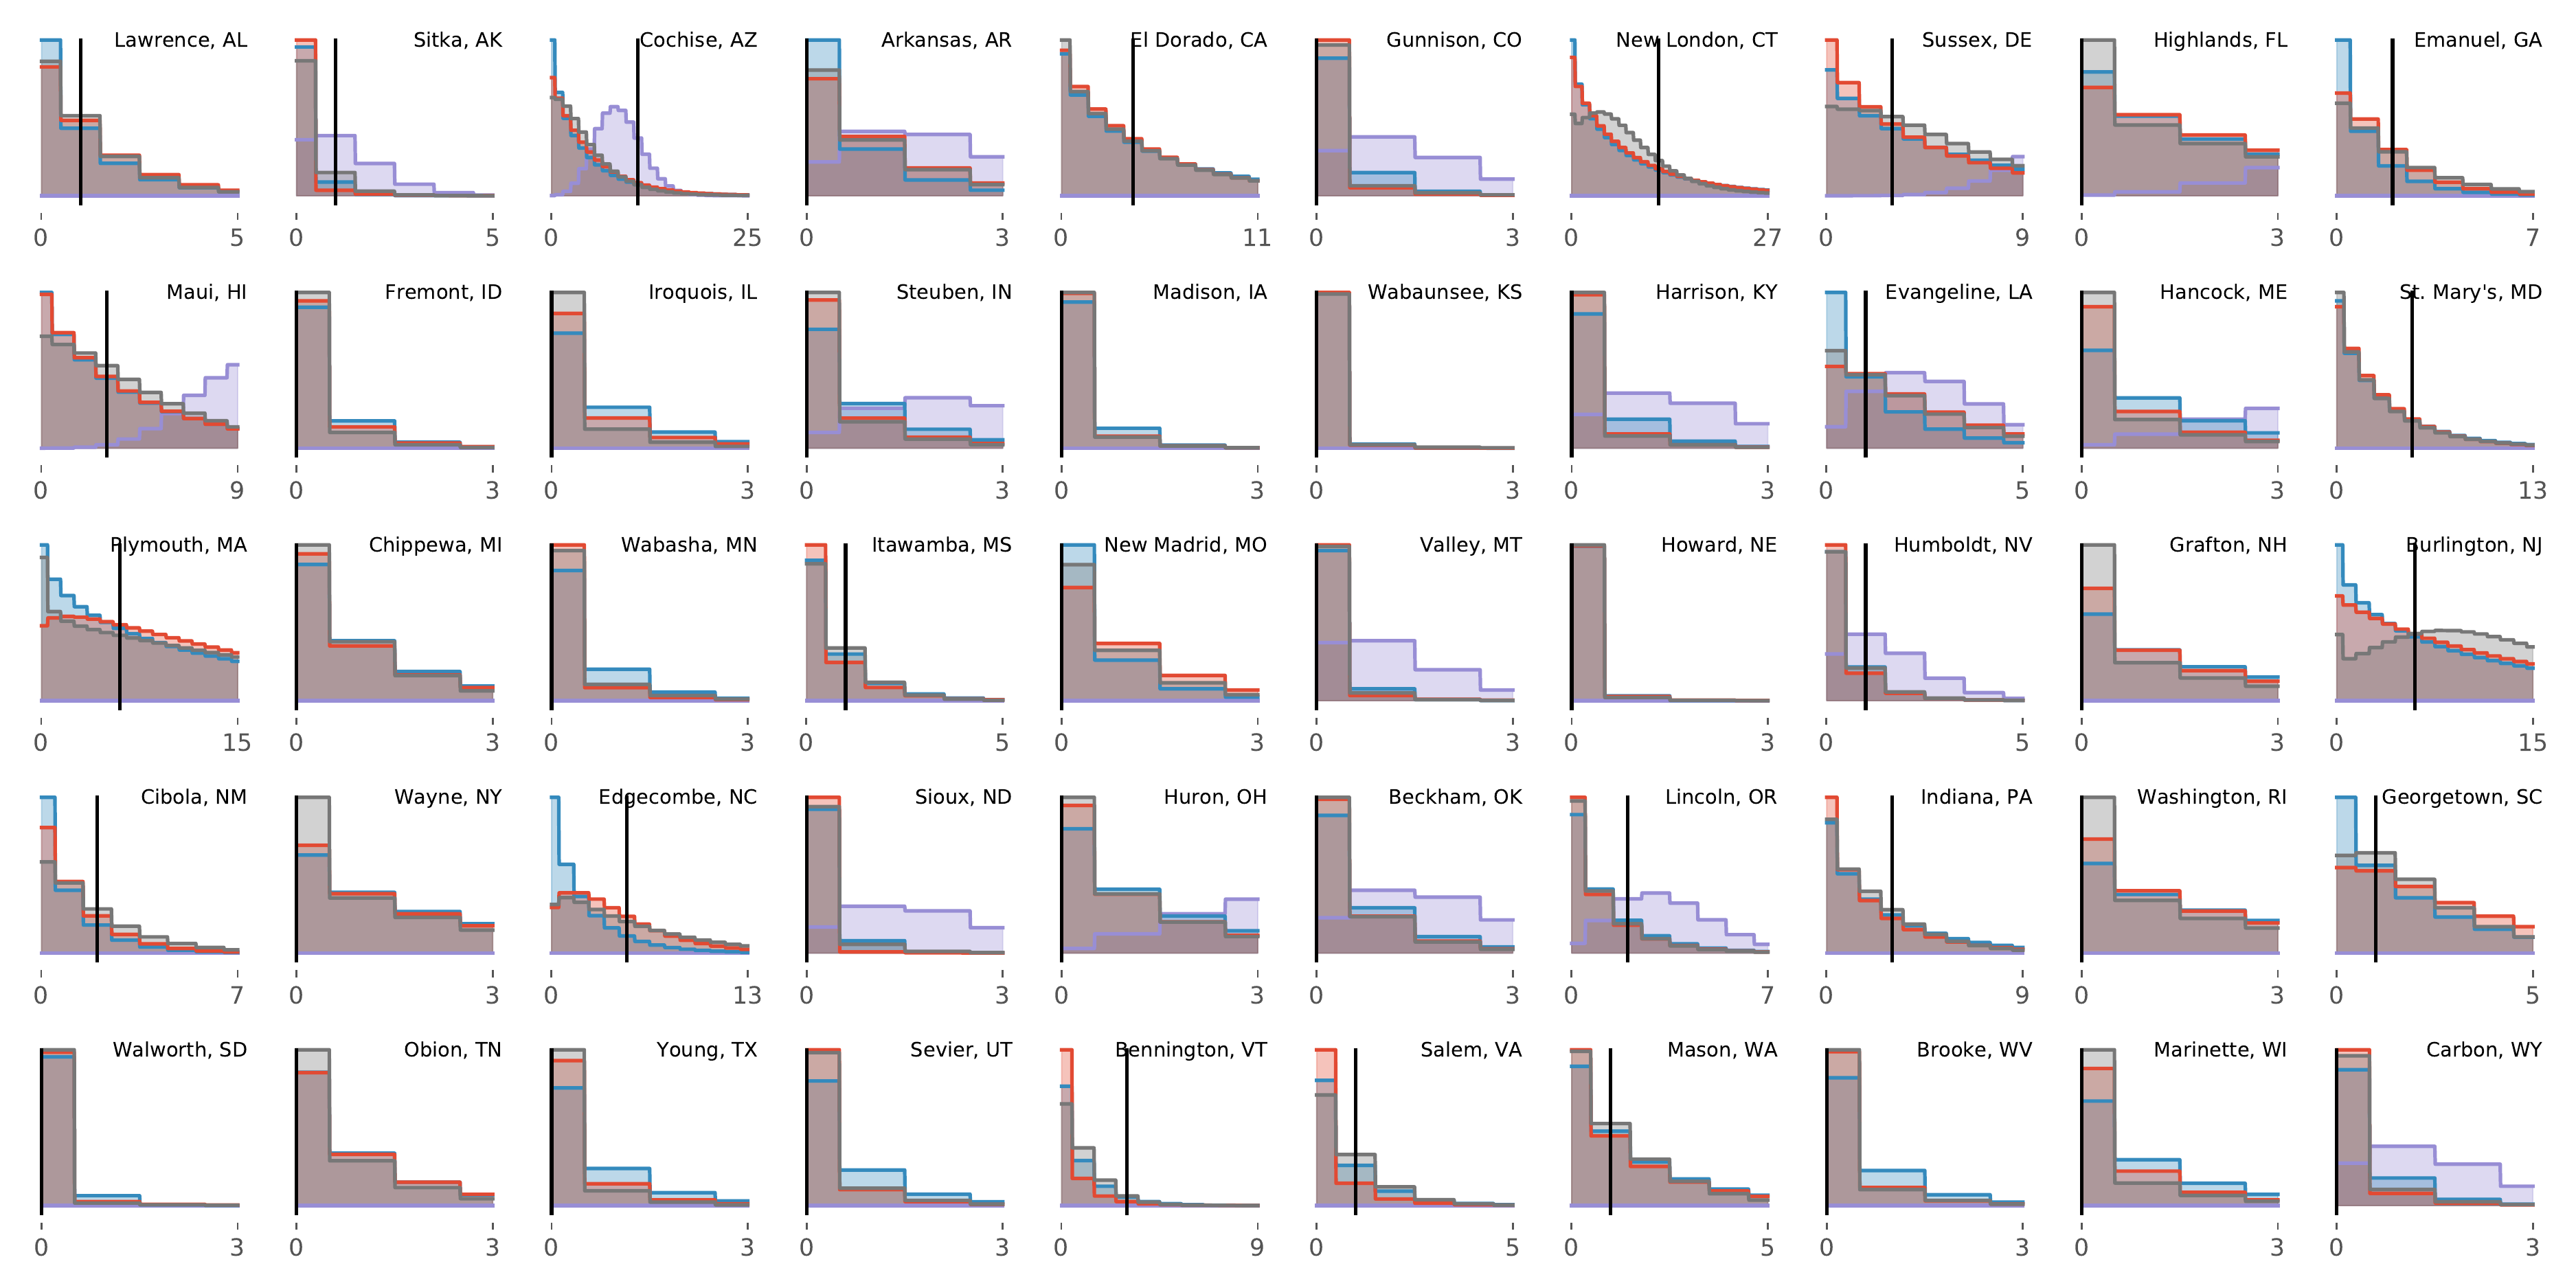}
		\end{subfigure}
		\caption{\small \textbf{Sample predictive distributions for homicide}. Predictive distributions $p(y_i|x_i;\phi)$ on homicide rates are shown for one county per state. 
			Distributions corresponding to LDF are in red, LDF-MM in gray, gamma-Poisson regression in blue, and Poisson regression in purple. The empirical rate is shown by the black line.
			The counties displayed are those with median populations for their given state.} 
		\label{fig-predictives-homicide-median}
	\end{center}
	\vspace*{-5mm}
\end{figure}

%smallest posterior
\begin{figure}[t]
	\vskip 0.1in
	\begin{center}
		\begin{subfigure}[b]{\textwidth}
			\centering
			\includegraphics[width=\linewidth, trim={0cm 0cm 0cm 0cm},clip]{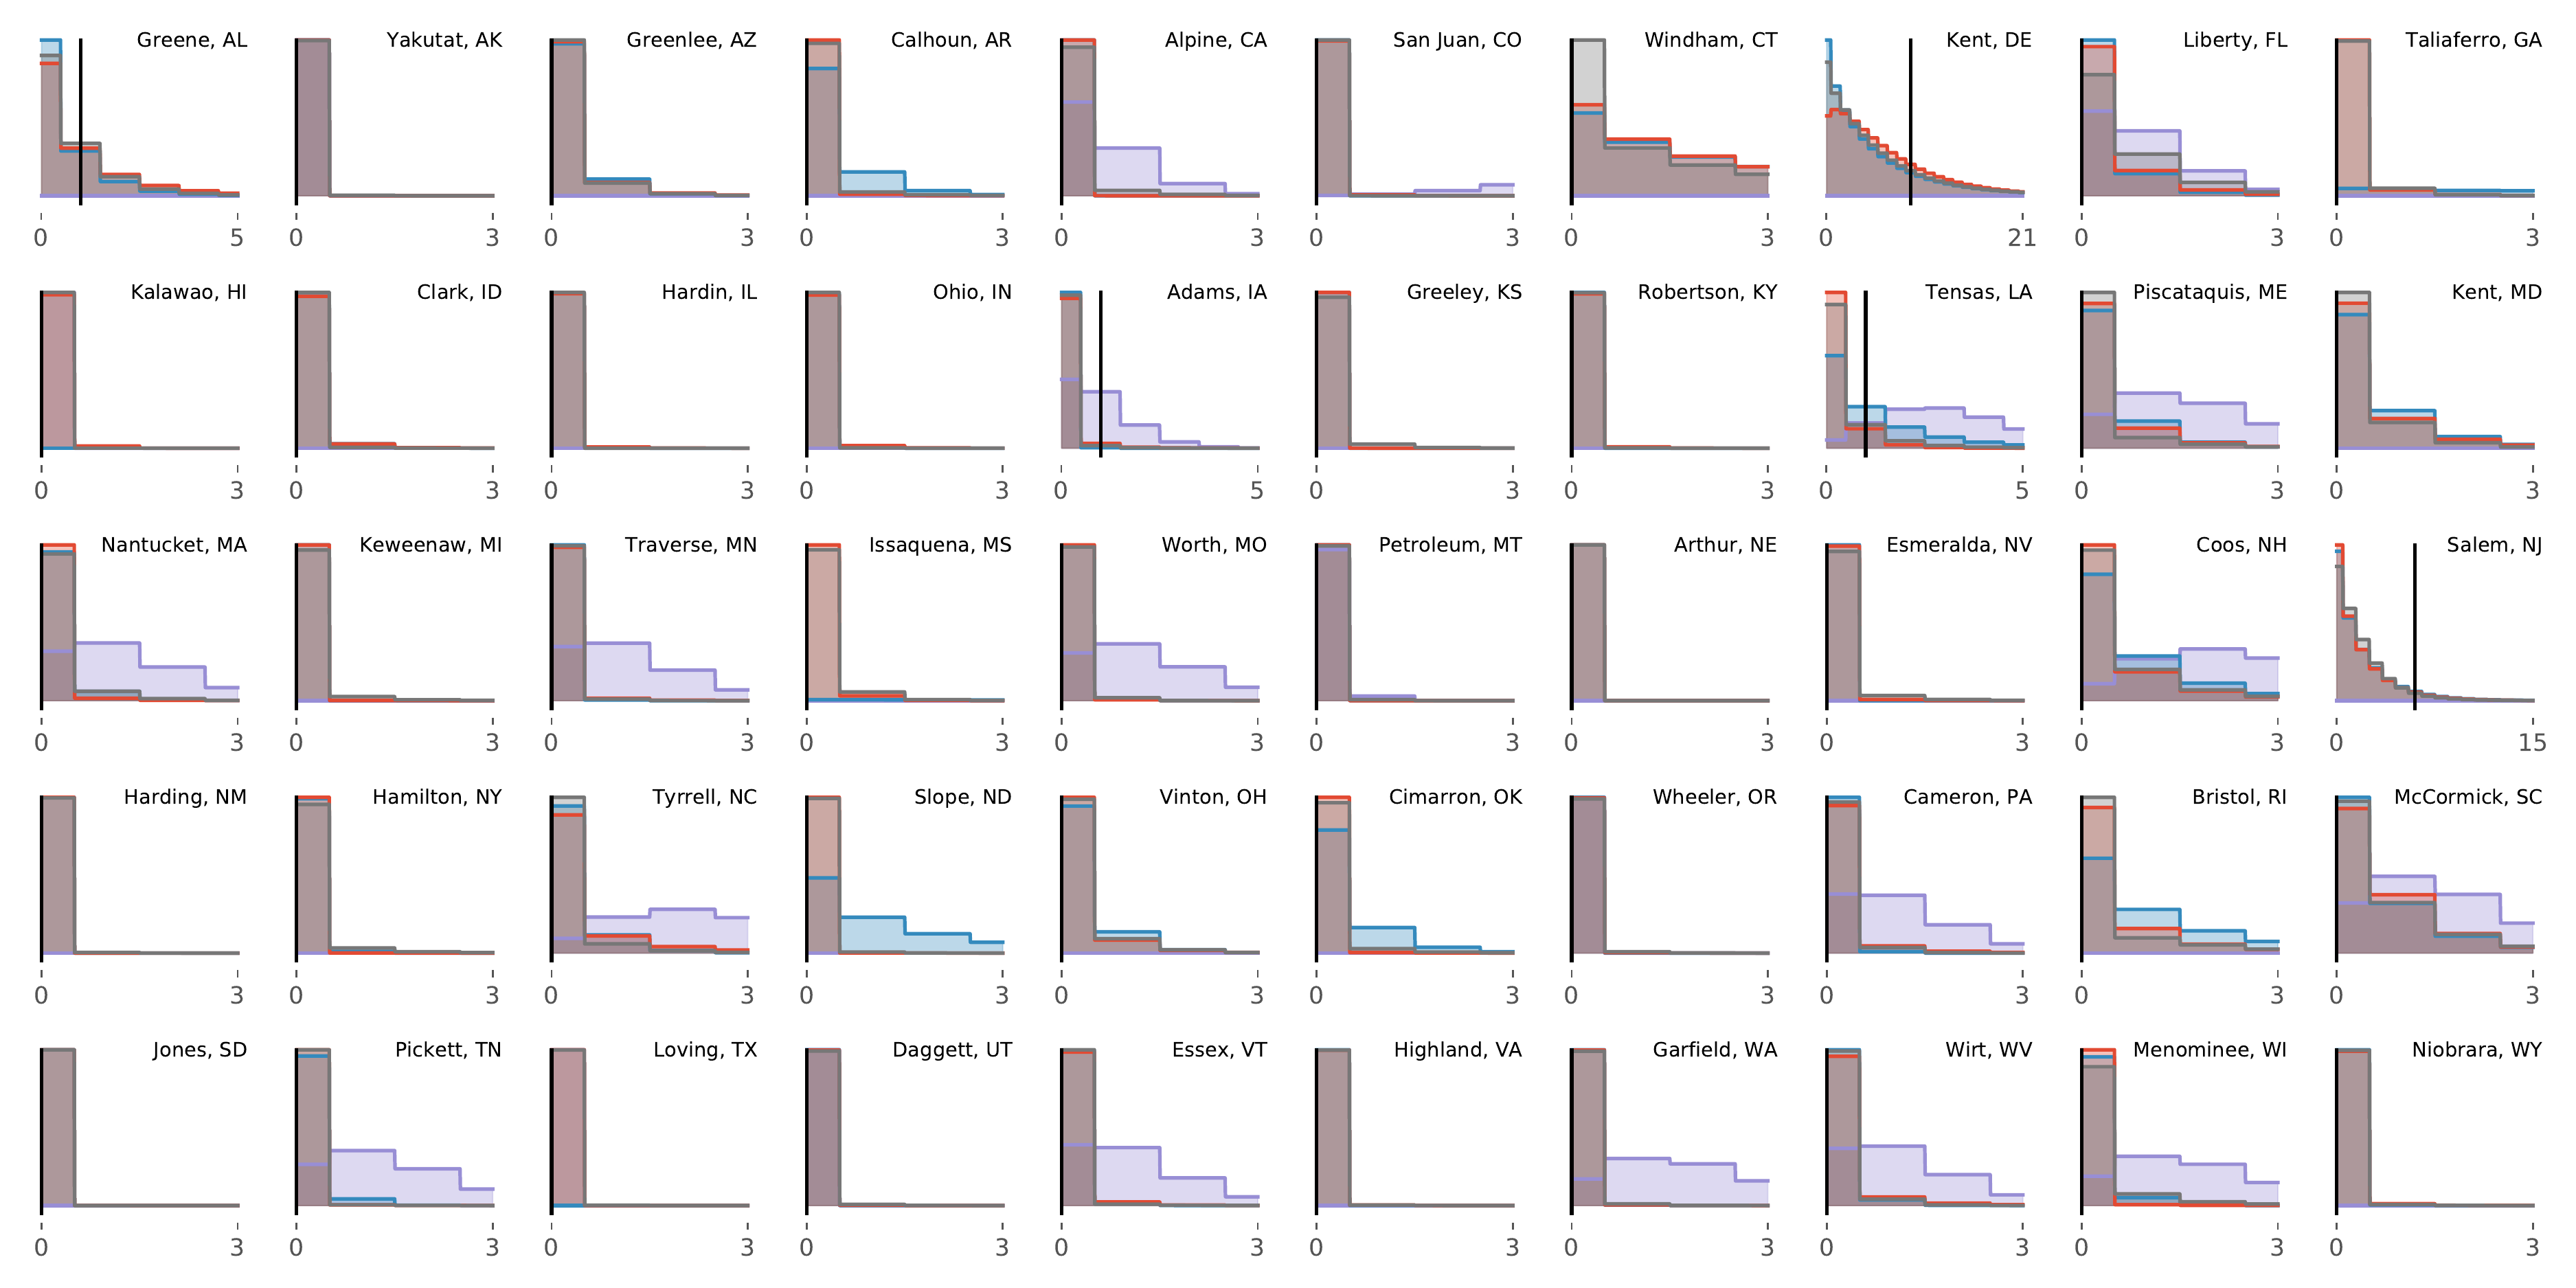}
		\end{subfigure}
		\caption{\small \textbf{Sample predictive distributions for homicide}. Predictive distributions $p(y_i|x_i;\phi)$ on homicide rates are shown for one county per state. 
			Distributions corresponding to LDF are in red, LDF-MM in gray, gamma-Poisson regression in blue, and Poisson regression in purple. The empirical rate is shown by the black line.
			The counties displayed are those with the smallest population for their given state.} 
		\label{fig-predictives-homicide-smallest}
	\end{center}
	\vspace*{-5mm}
\end{figure}
