# Supplementary material for: Lightweight Data Fusion with Conjugate Mappings
Source: arXiv:2011.10607 source file (2020-11-20)
Supplement: Supplementary file 2 [file appendix_electrification_distributions.tex]

\subsection*{Additional Results}

\subsubsection*{Latent Variable Posterior Distributions}

The latent variable posterior distributions $p(\theta_i \given x; \phi)$ are presented in Figs.~\ref{fig-supp-elec-aux-posterior-start} thru \ref{fig-supp-elec-aux-posterior-end}.  In each, the LDF posterior (red) and beta-binomial regression posterior (blue) are beta-distributions; the posterior in binomial regression is shown as a Dirac delta centered on the predicted mean.

We observe that LDF often extracts more information from the auxiliary data than beta-binomial regression, c.f. Figure 3 (right) in the main text, and is thus able to obtain a more confident posterior distributions when the distribution is skewed away from zero.

\begin{figure}[t]
  \vskip 0.1in
  \begin{center}
    \centerline{\includegraphics[width=0.75\linewidth, trim={0.375cm 1cm 0.375cm 1.5cm},clip]{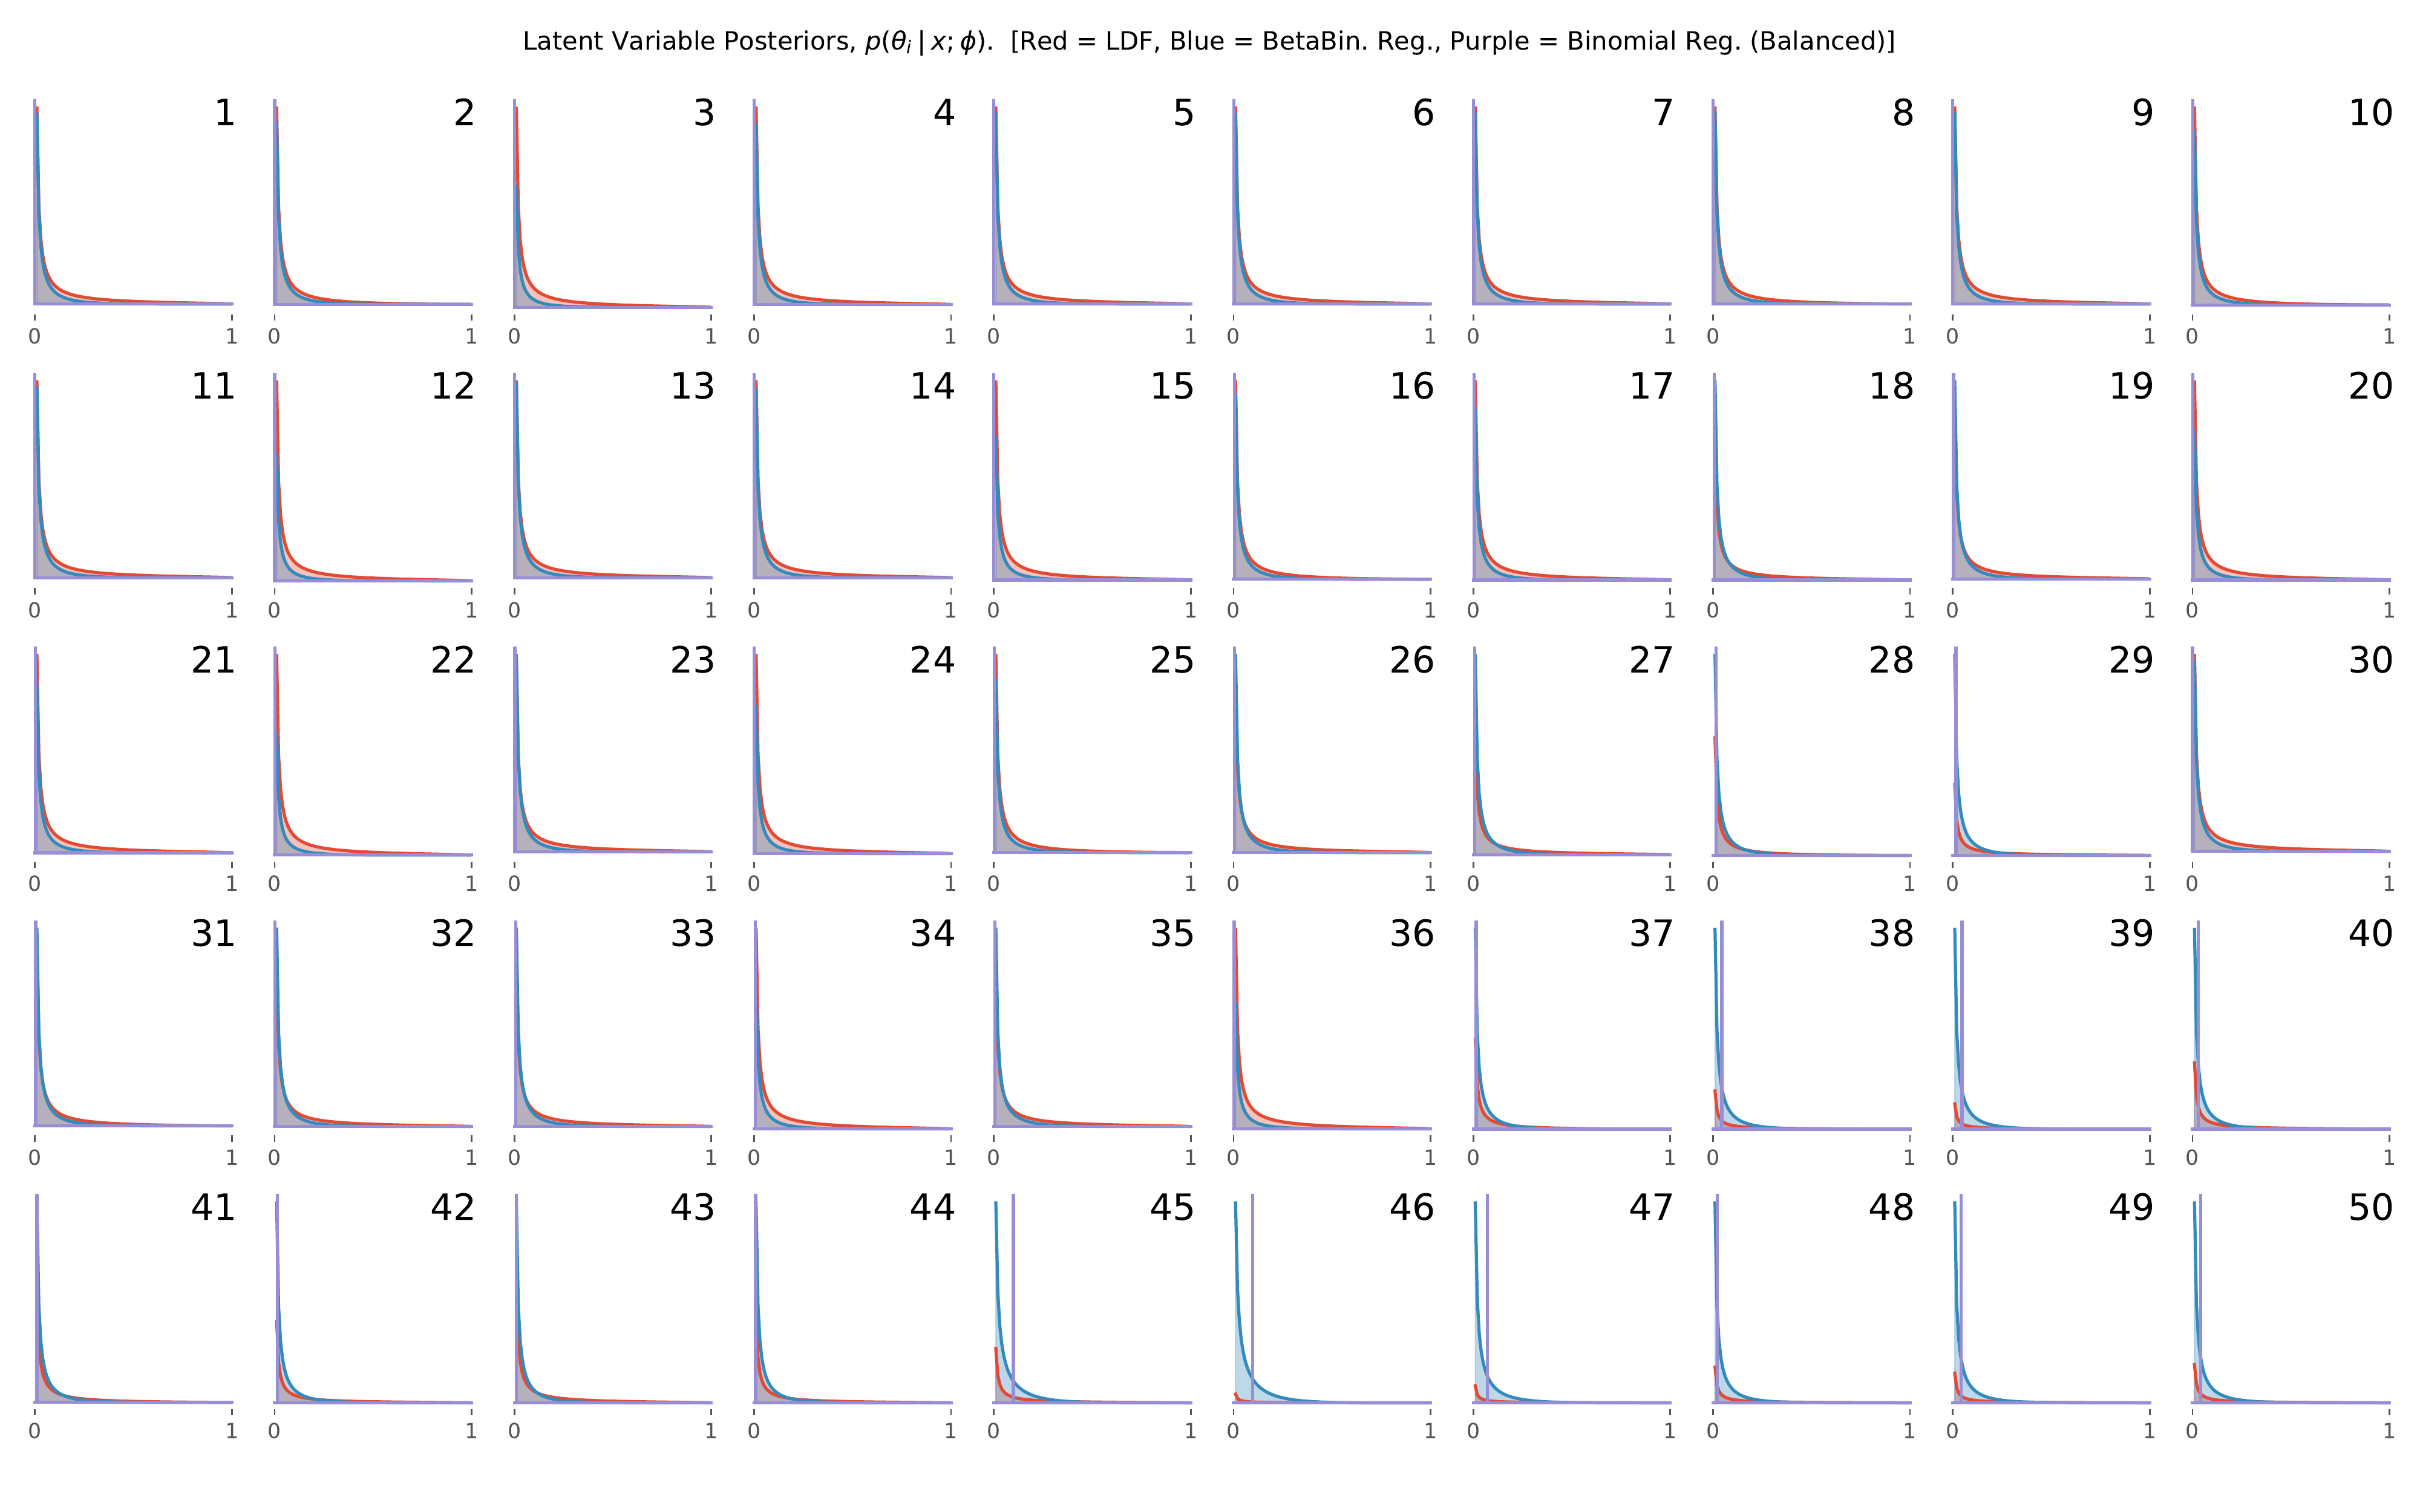}}
    \centerline{\includegraphics[width=0.75\linewidth, trim={0.375cm 1cm 0.375cm 1.5cm},clip]{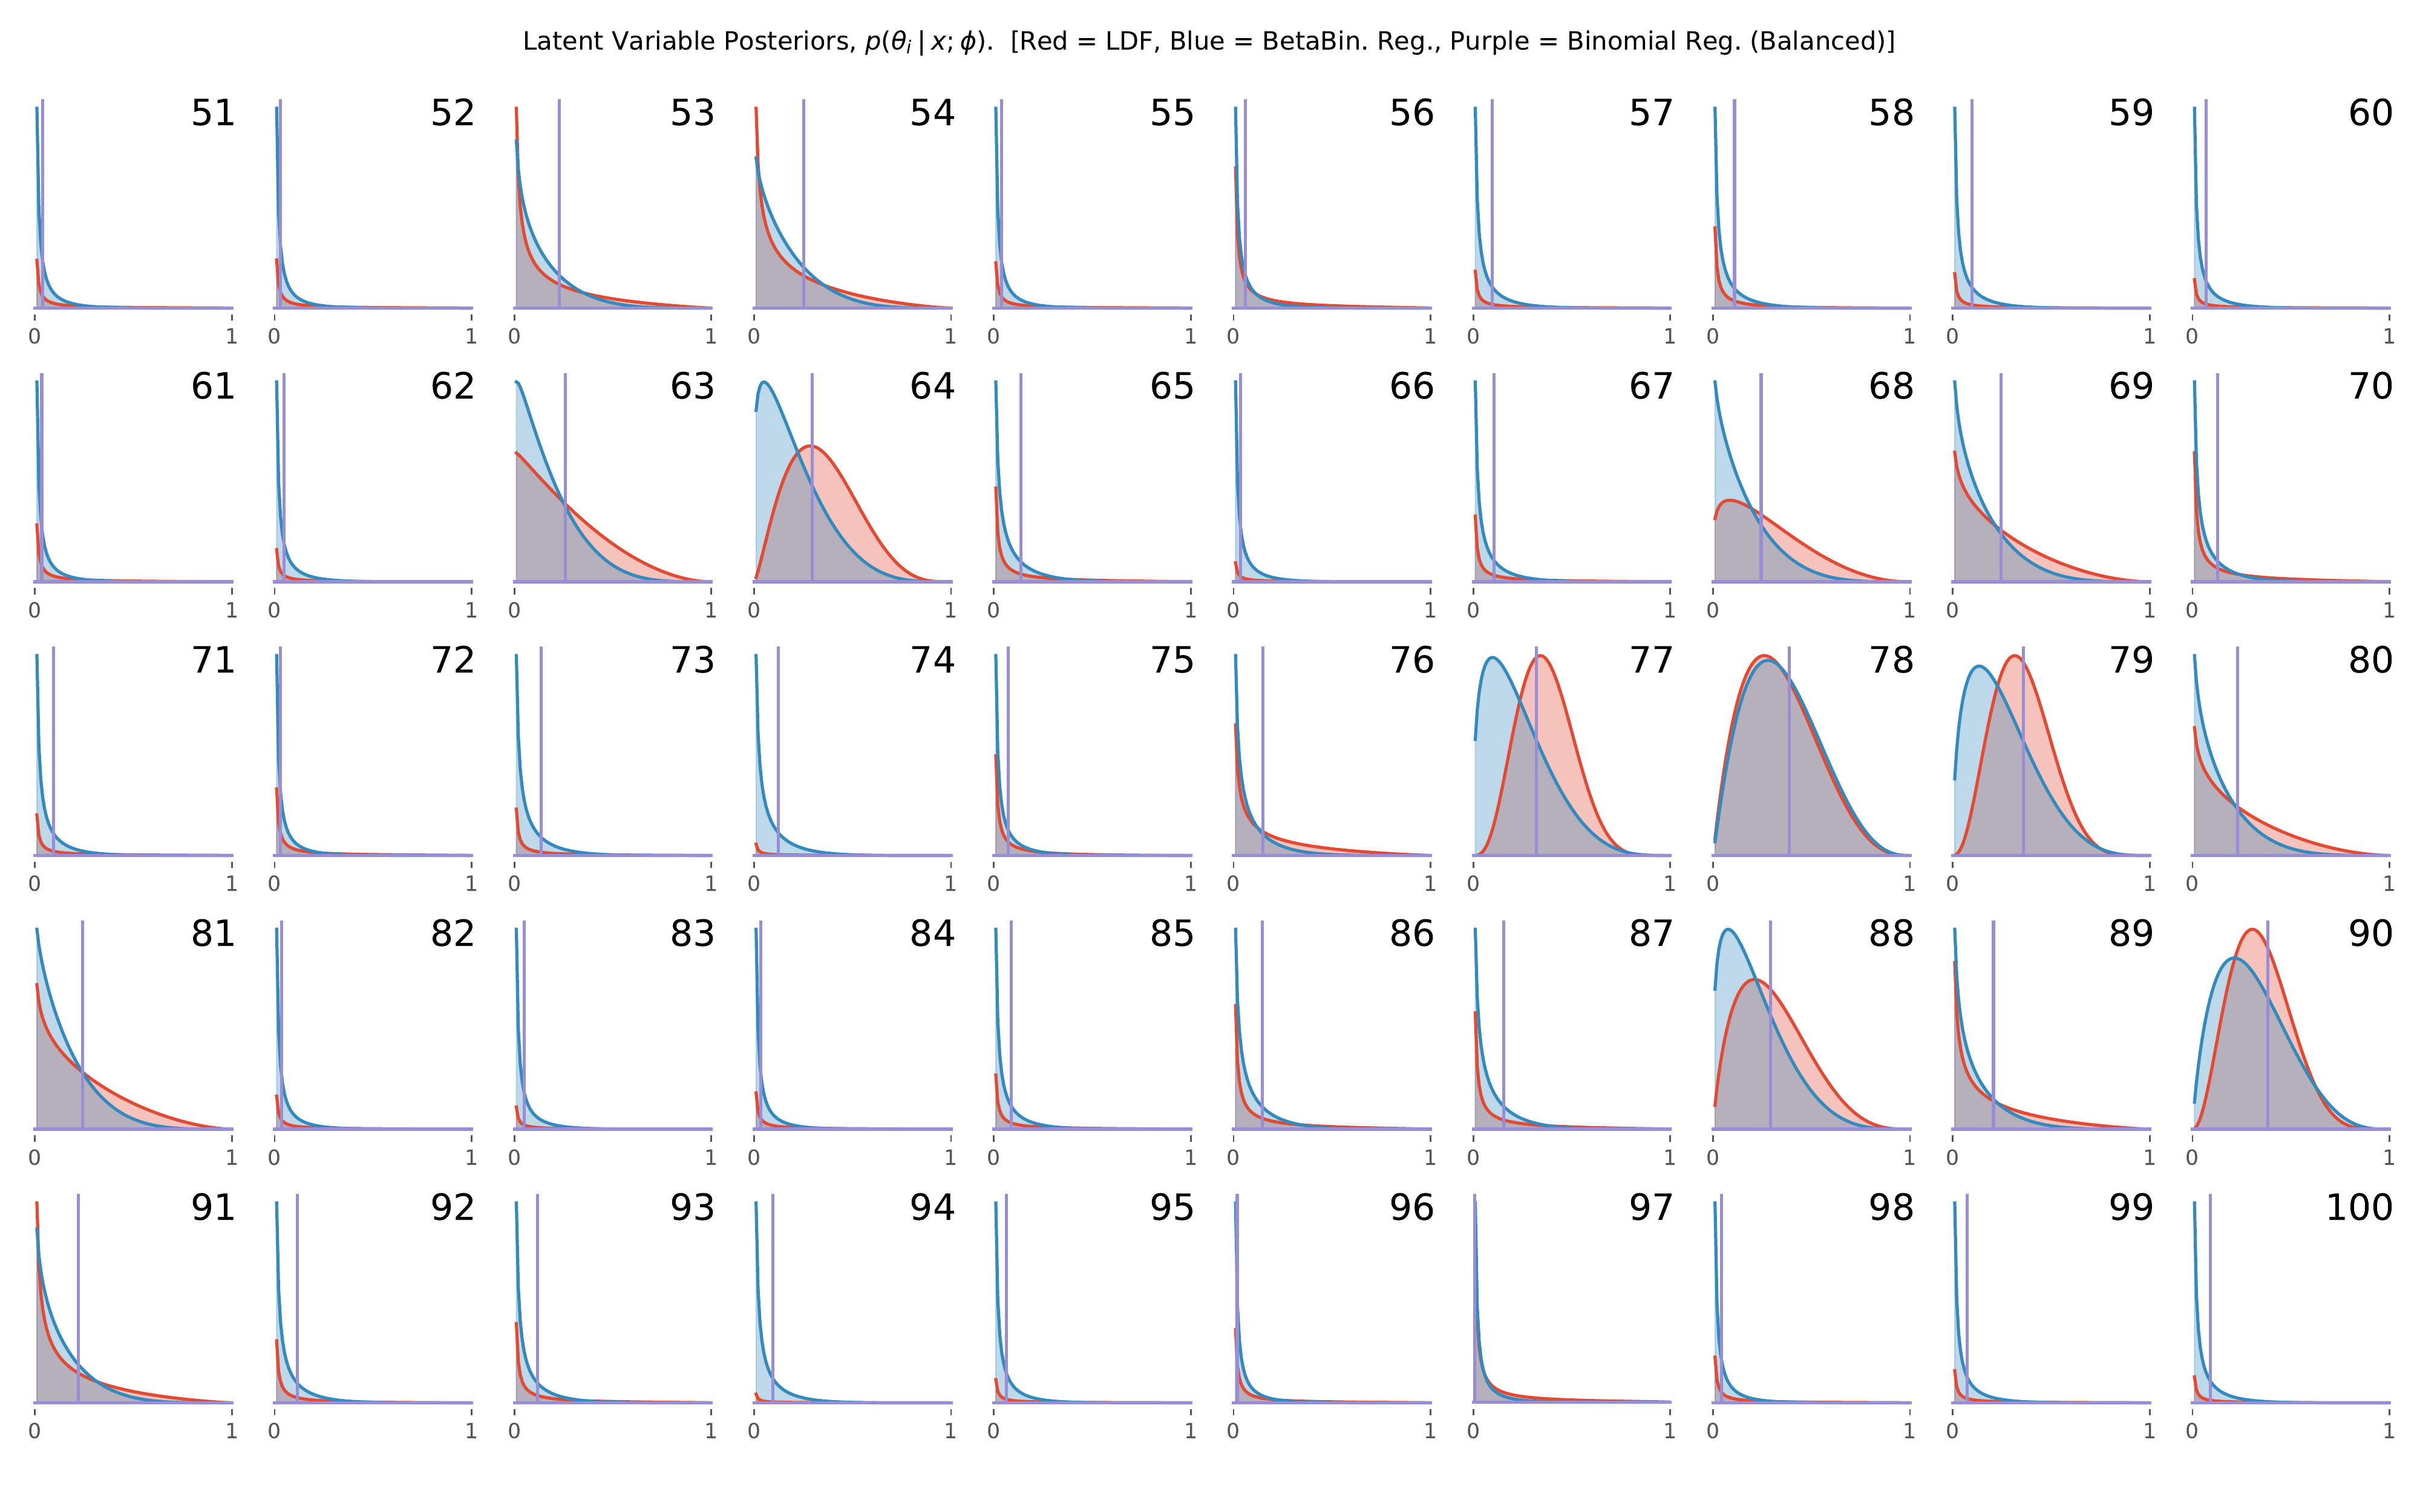}}
     \centerline{\includegraphics[width=0.75\linewidth, trim={0.375cm 1cm 0.375cm 1.5cm},clip]{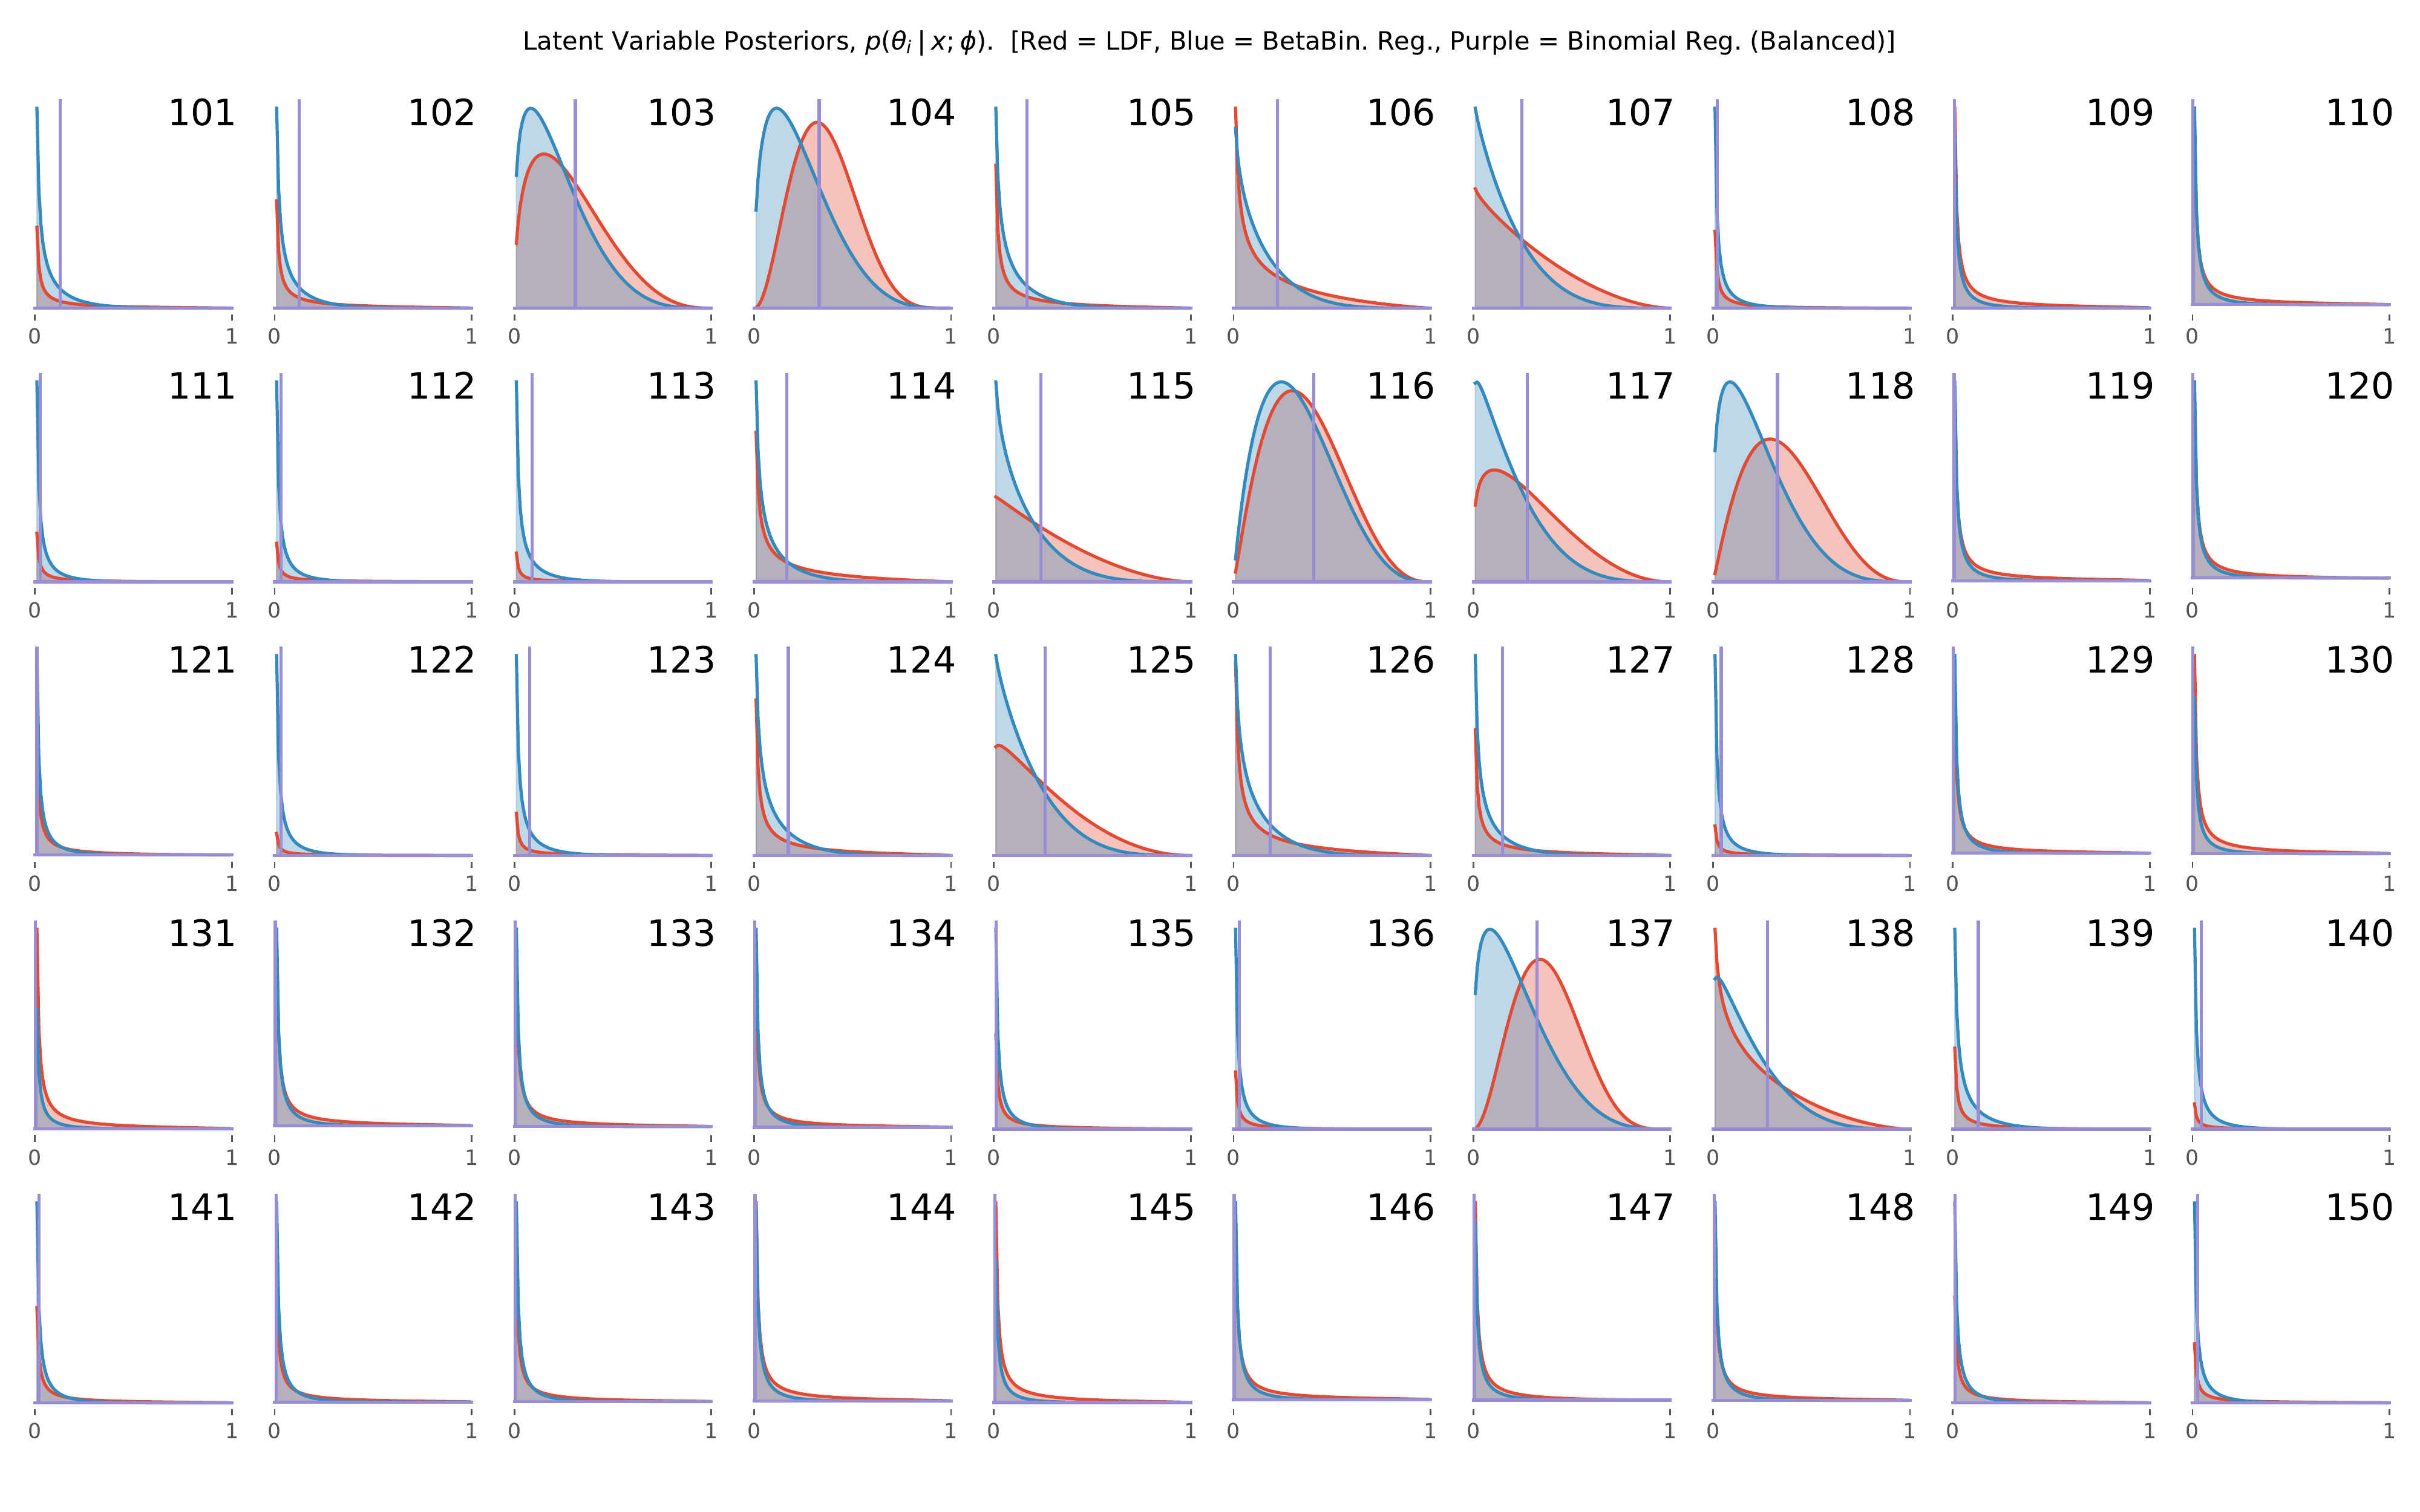}}
    \caption{\small \textbf{Latent variable posteriors.}  A sample of the posteriors $p(\theta_i \given x; \phi)$ for the electrification application.  LDF is red, beta-binomial regression is blue, and binomial regression is purple.}
    \label{fig-supp-elec-aux-posterior-start}
  \end{center}
  \vspace*{-5mm}
\end{figure}

\begin{figure}[t]
  \vskip 0.1in
  \begin{center}
    \centerline{\includegraphics[width=0.75\linewidth, trim={0.375cm 1cm 0.375cm 1.5cm},clip]{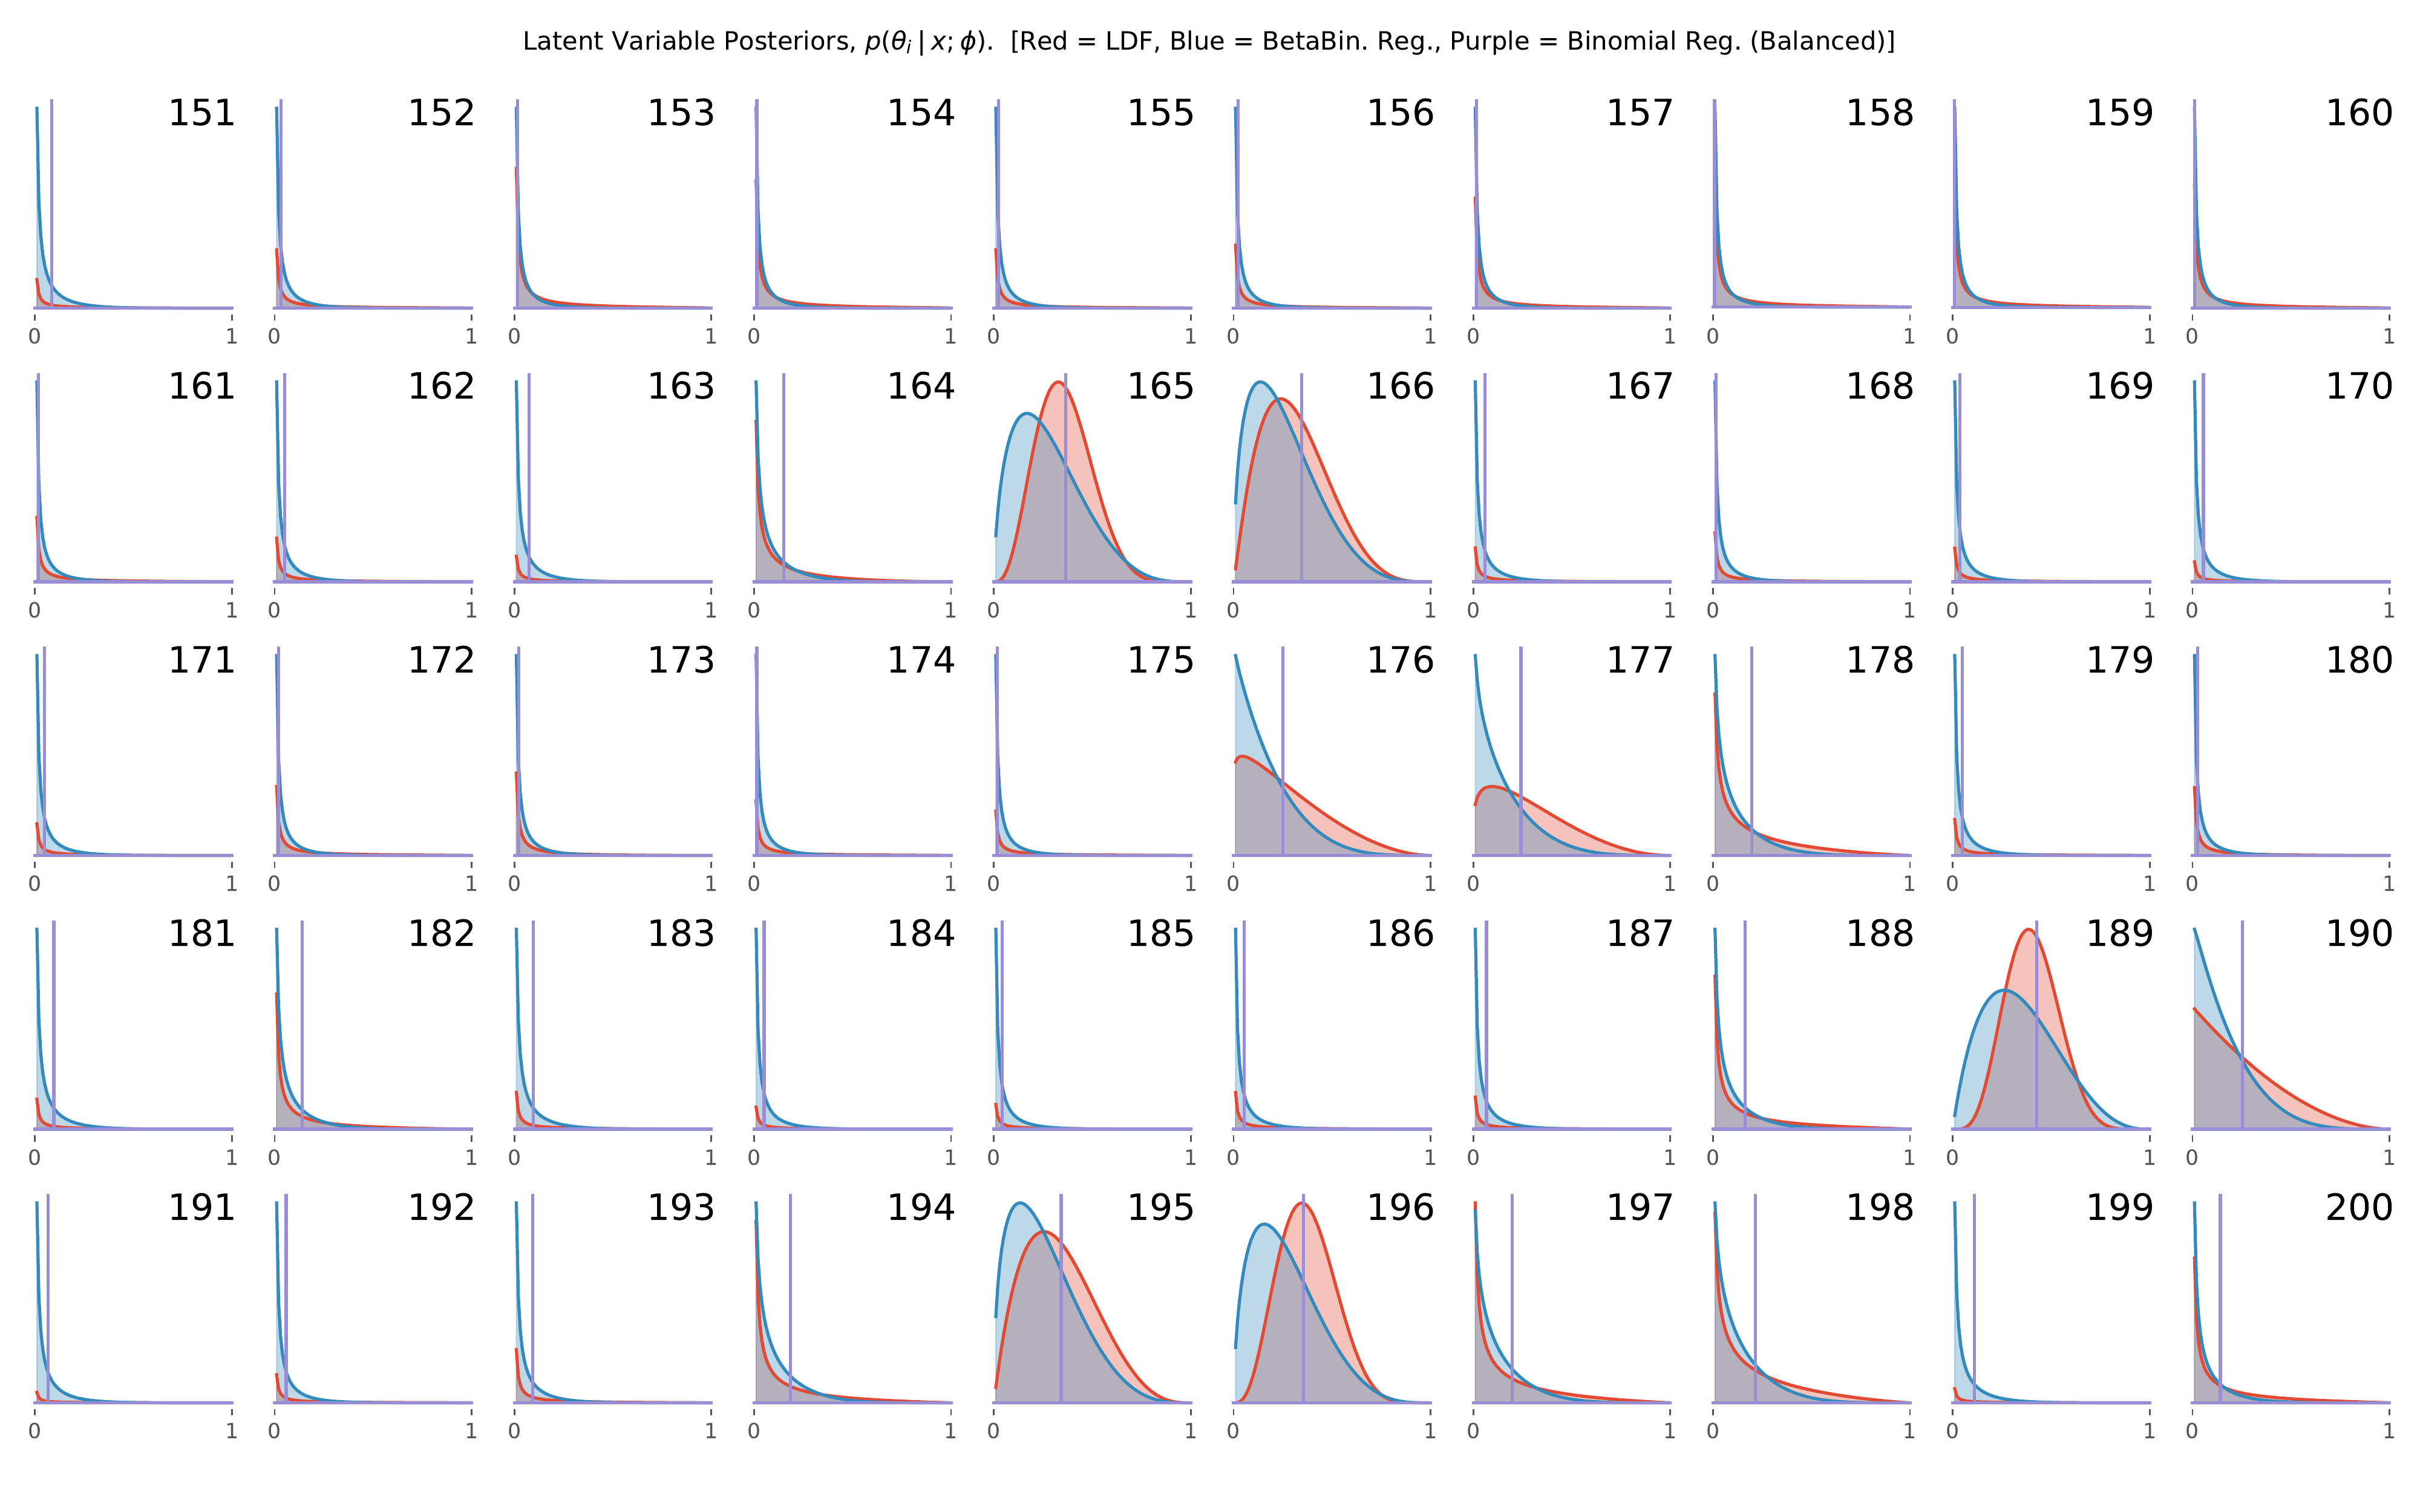}}
    \centerline{\includegraphics[width=0.75\linewidth, trim={0.375cm 1cm 0.375cm 1.5cm},clip]{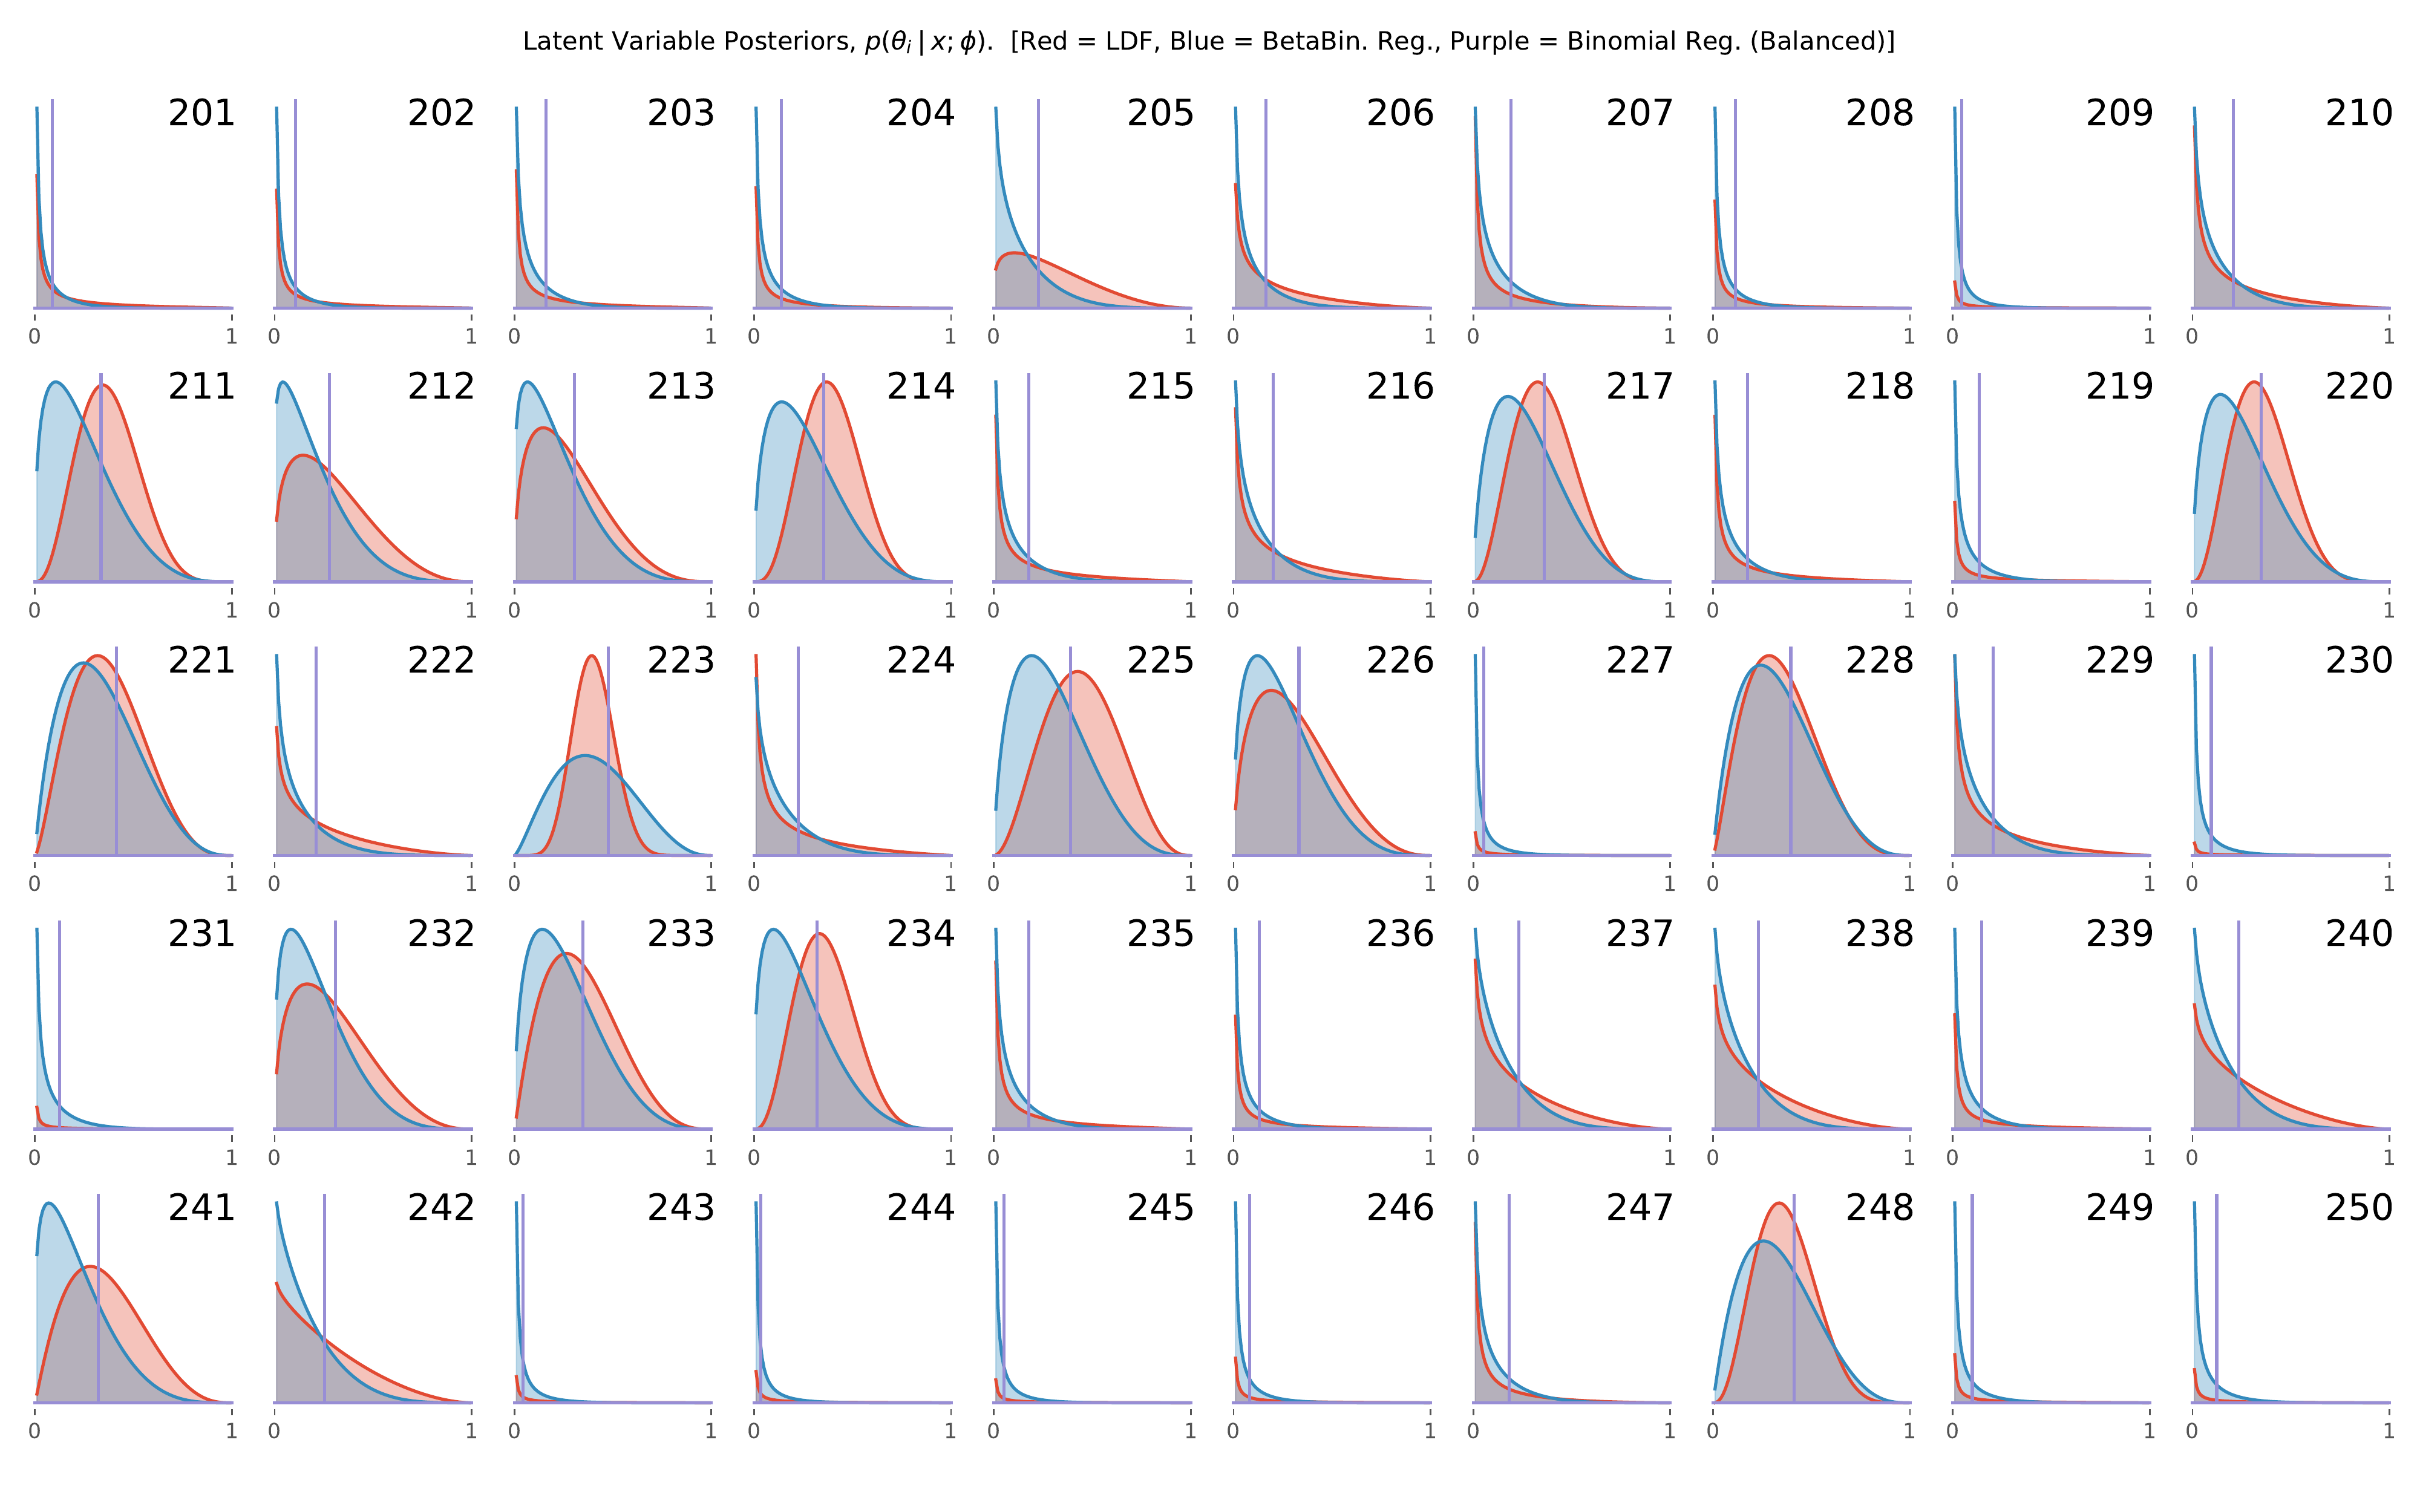}}
     \centerline{\includegraphics[width=0.75\linewidth, trim={0.375cm 1cm 0.375cm 1.5cm},clip]{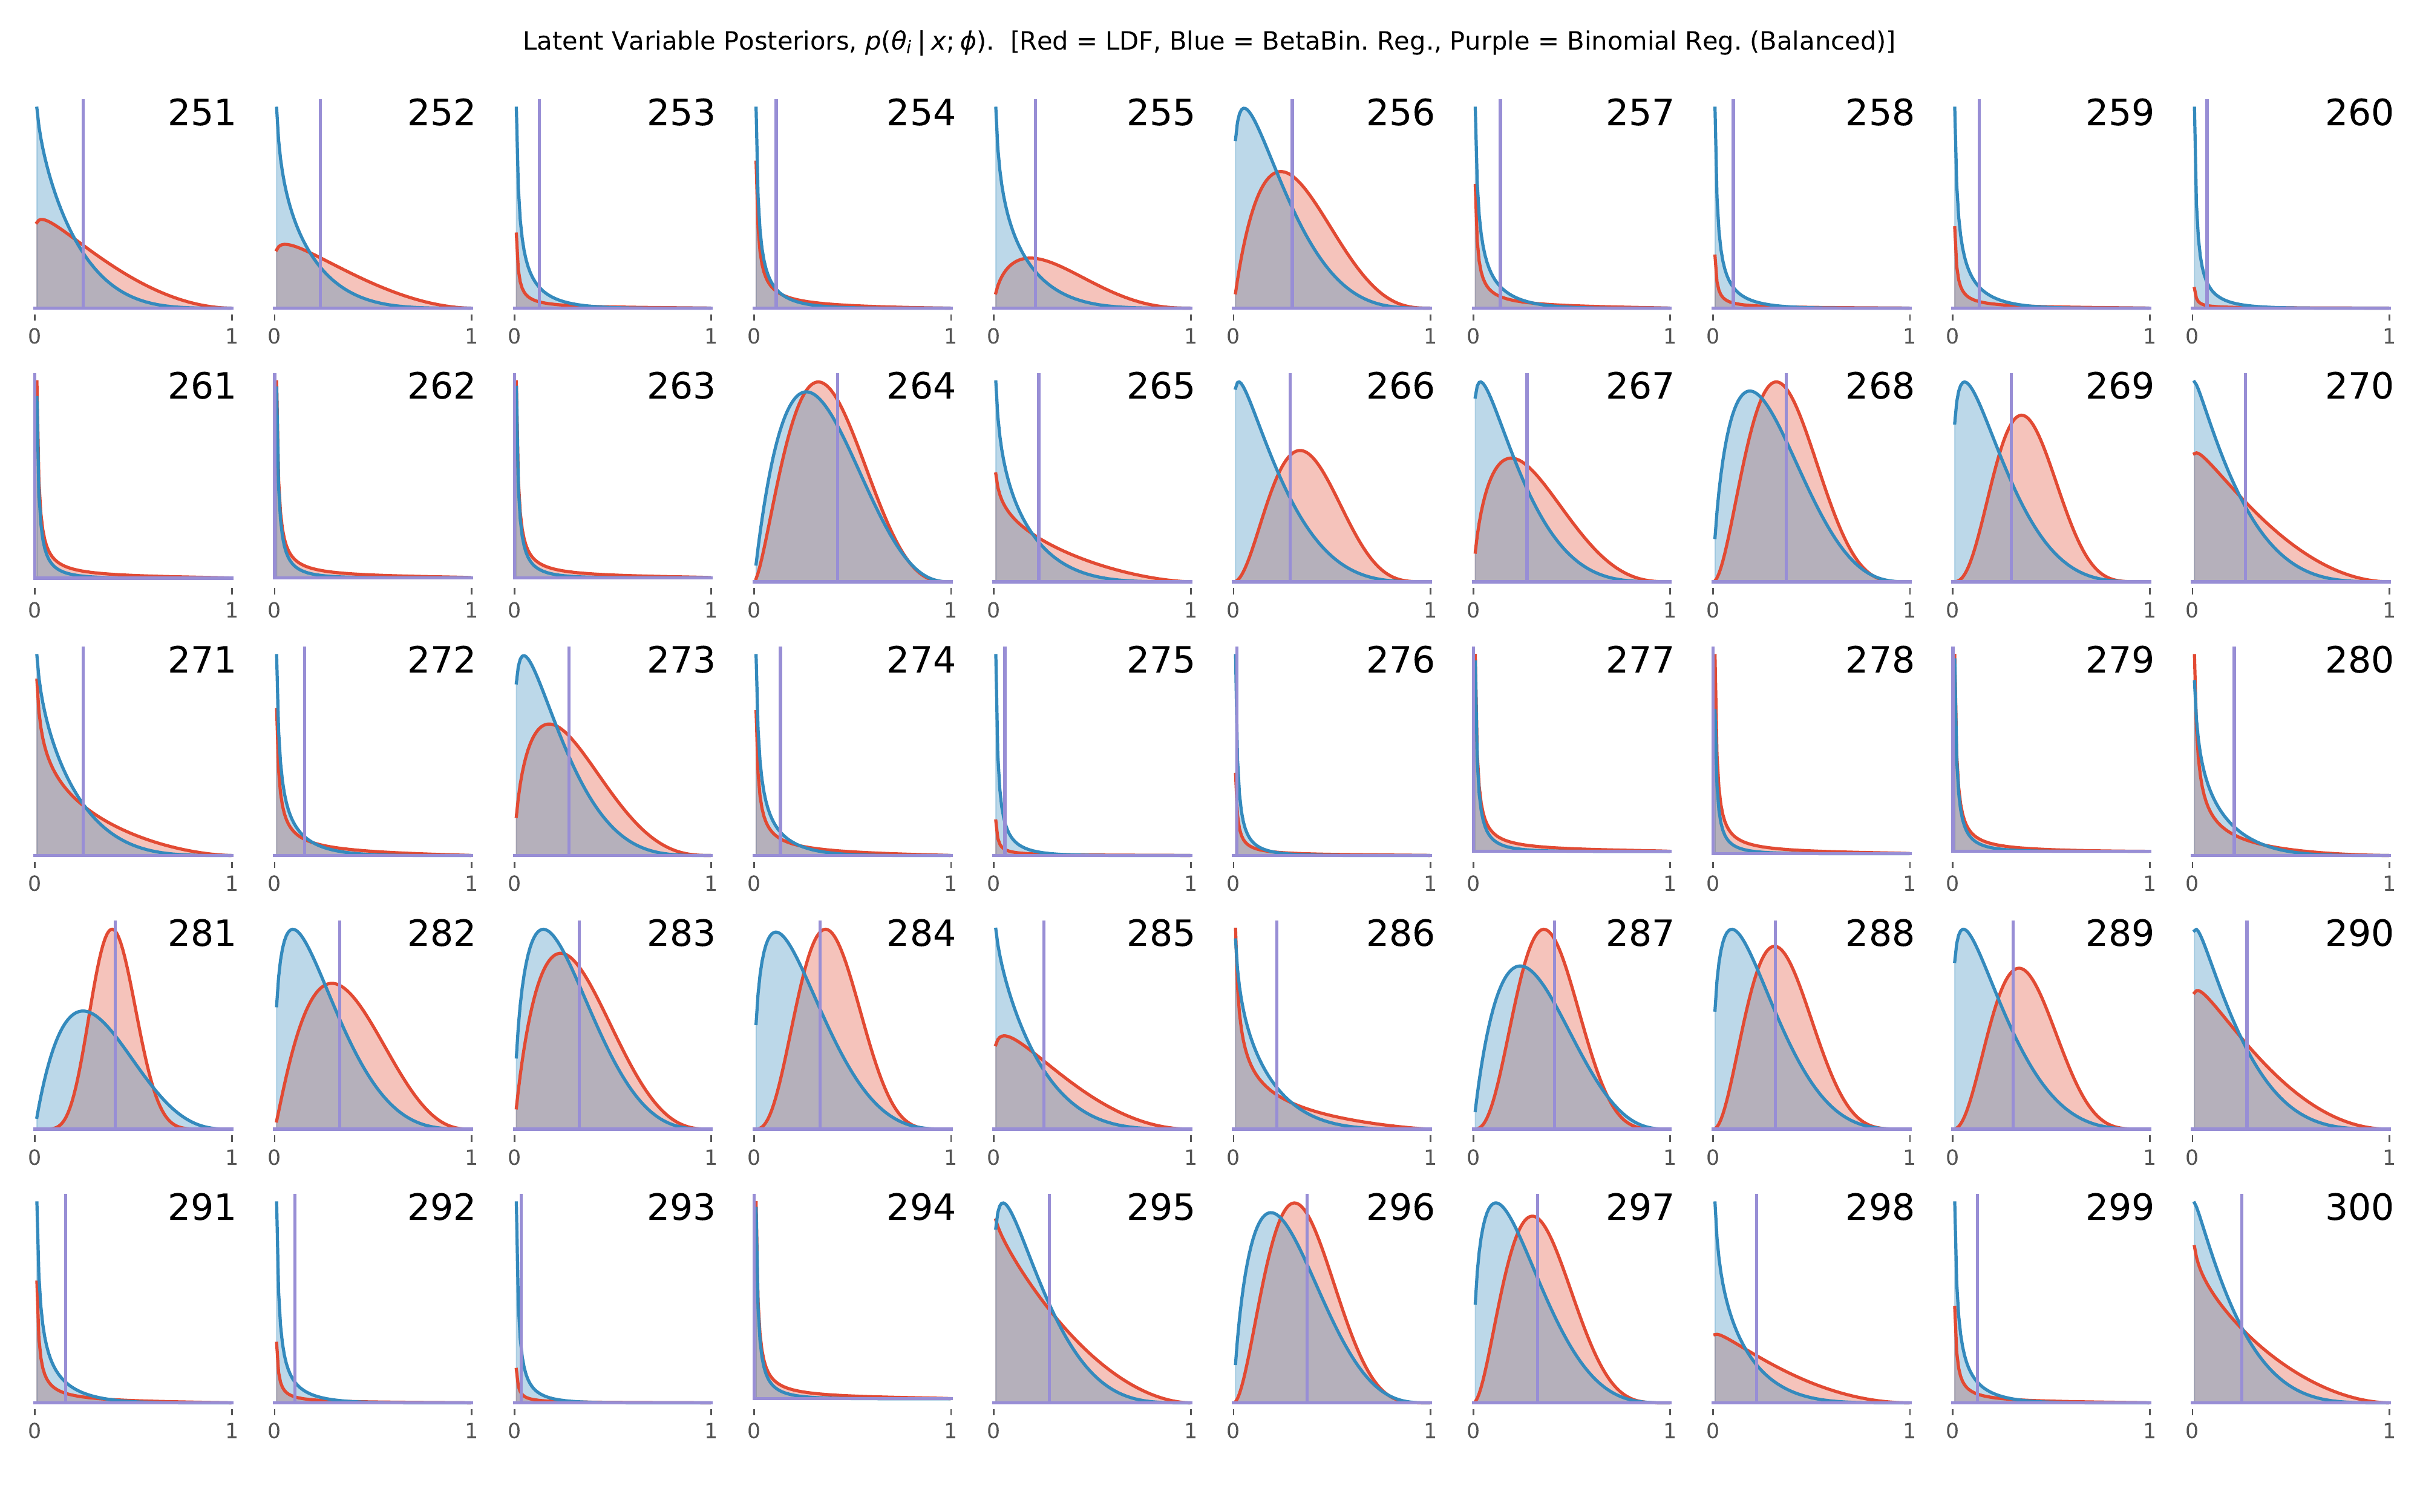}}
    \caption{\small \textbf{Latent variable posteriors (continued).}  A sample of the posteriors $p(\theta_i \given x; \phi)$ for the electrification application.  LDF is red, beta-binomial regression is blue, and binomial regression is purple.}
    
  \end{center}
  \vspace*{-5mm}
\end{figure}

\begin{figure}[t]
  \vskip 0.1in
  \begin{center}
    \centerline{\includegraphics[width=0.75\linewidth, trim={0.375cm 1cm 0.375cm 1.5cm},clip]{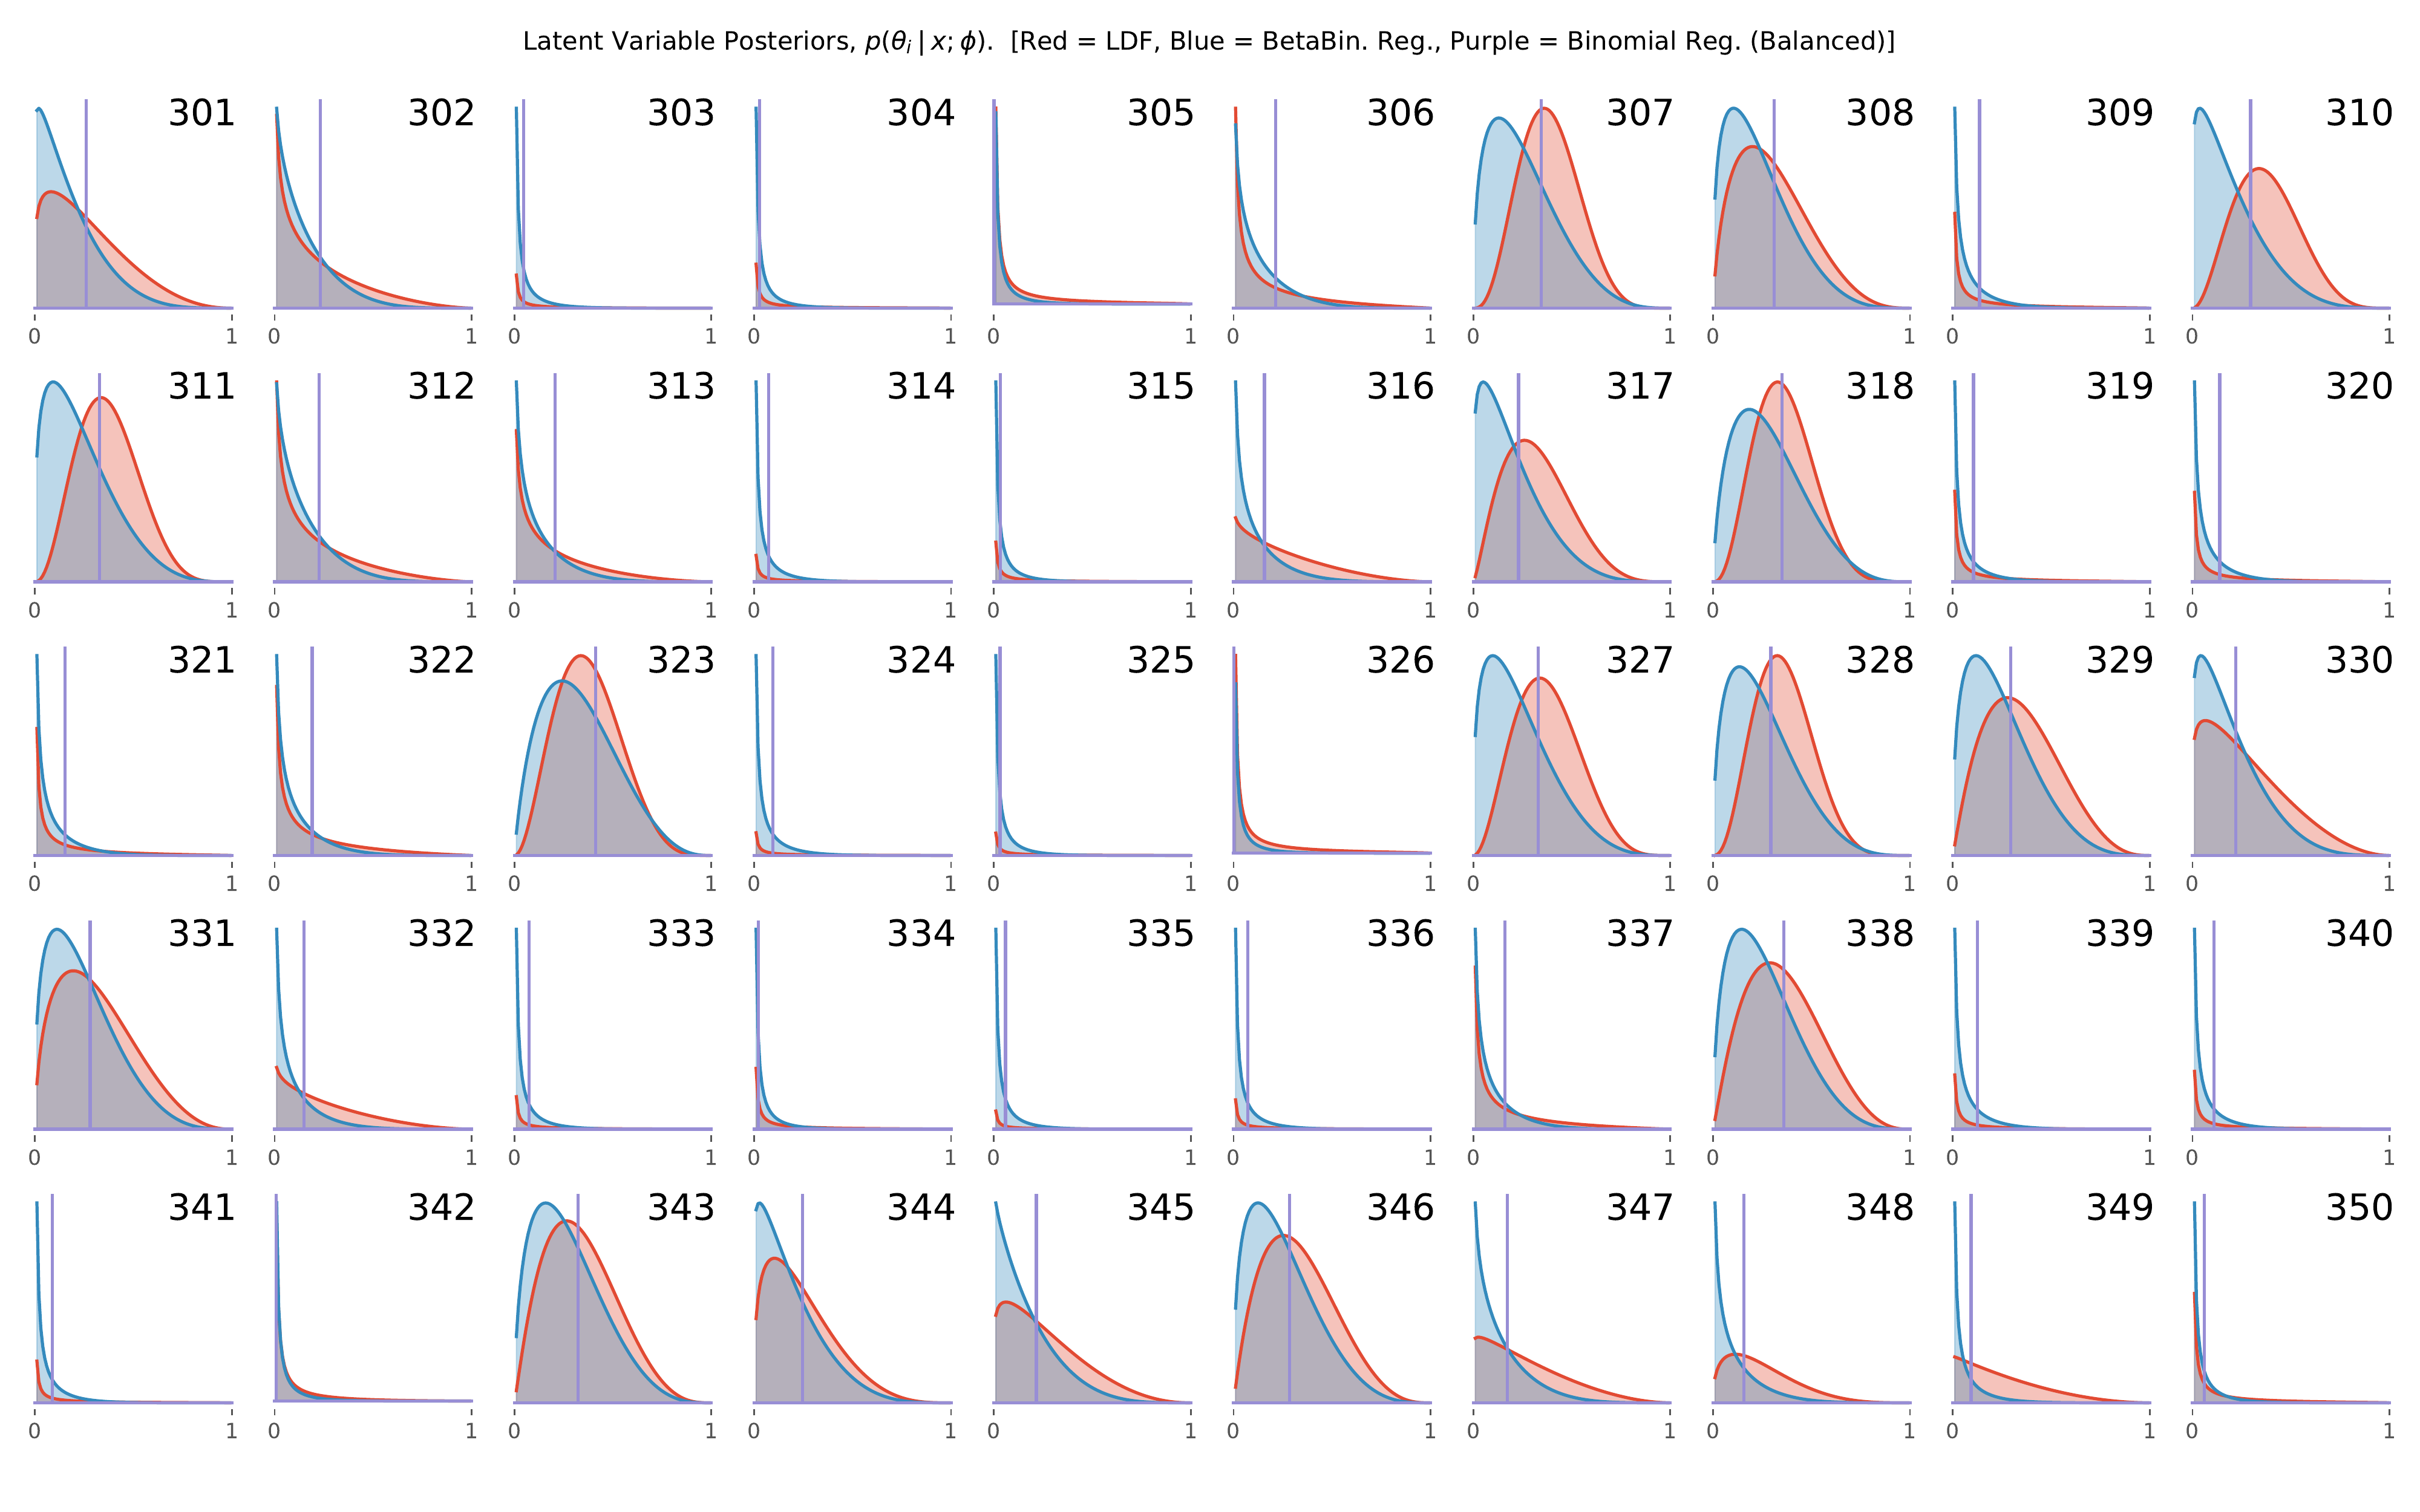}}
    \centerline{\includegraphics[width=0.75\linewidth, trim={0.375cm 1cm 0.375cm 1.5cm},clip]{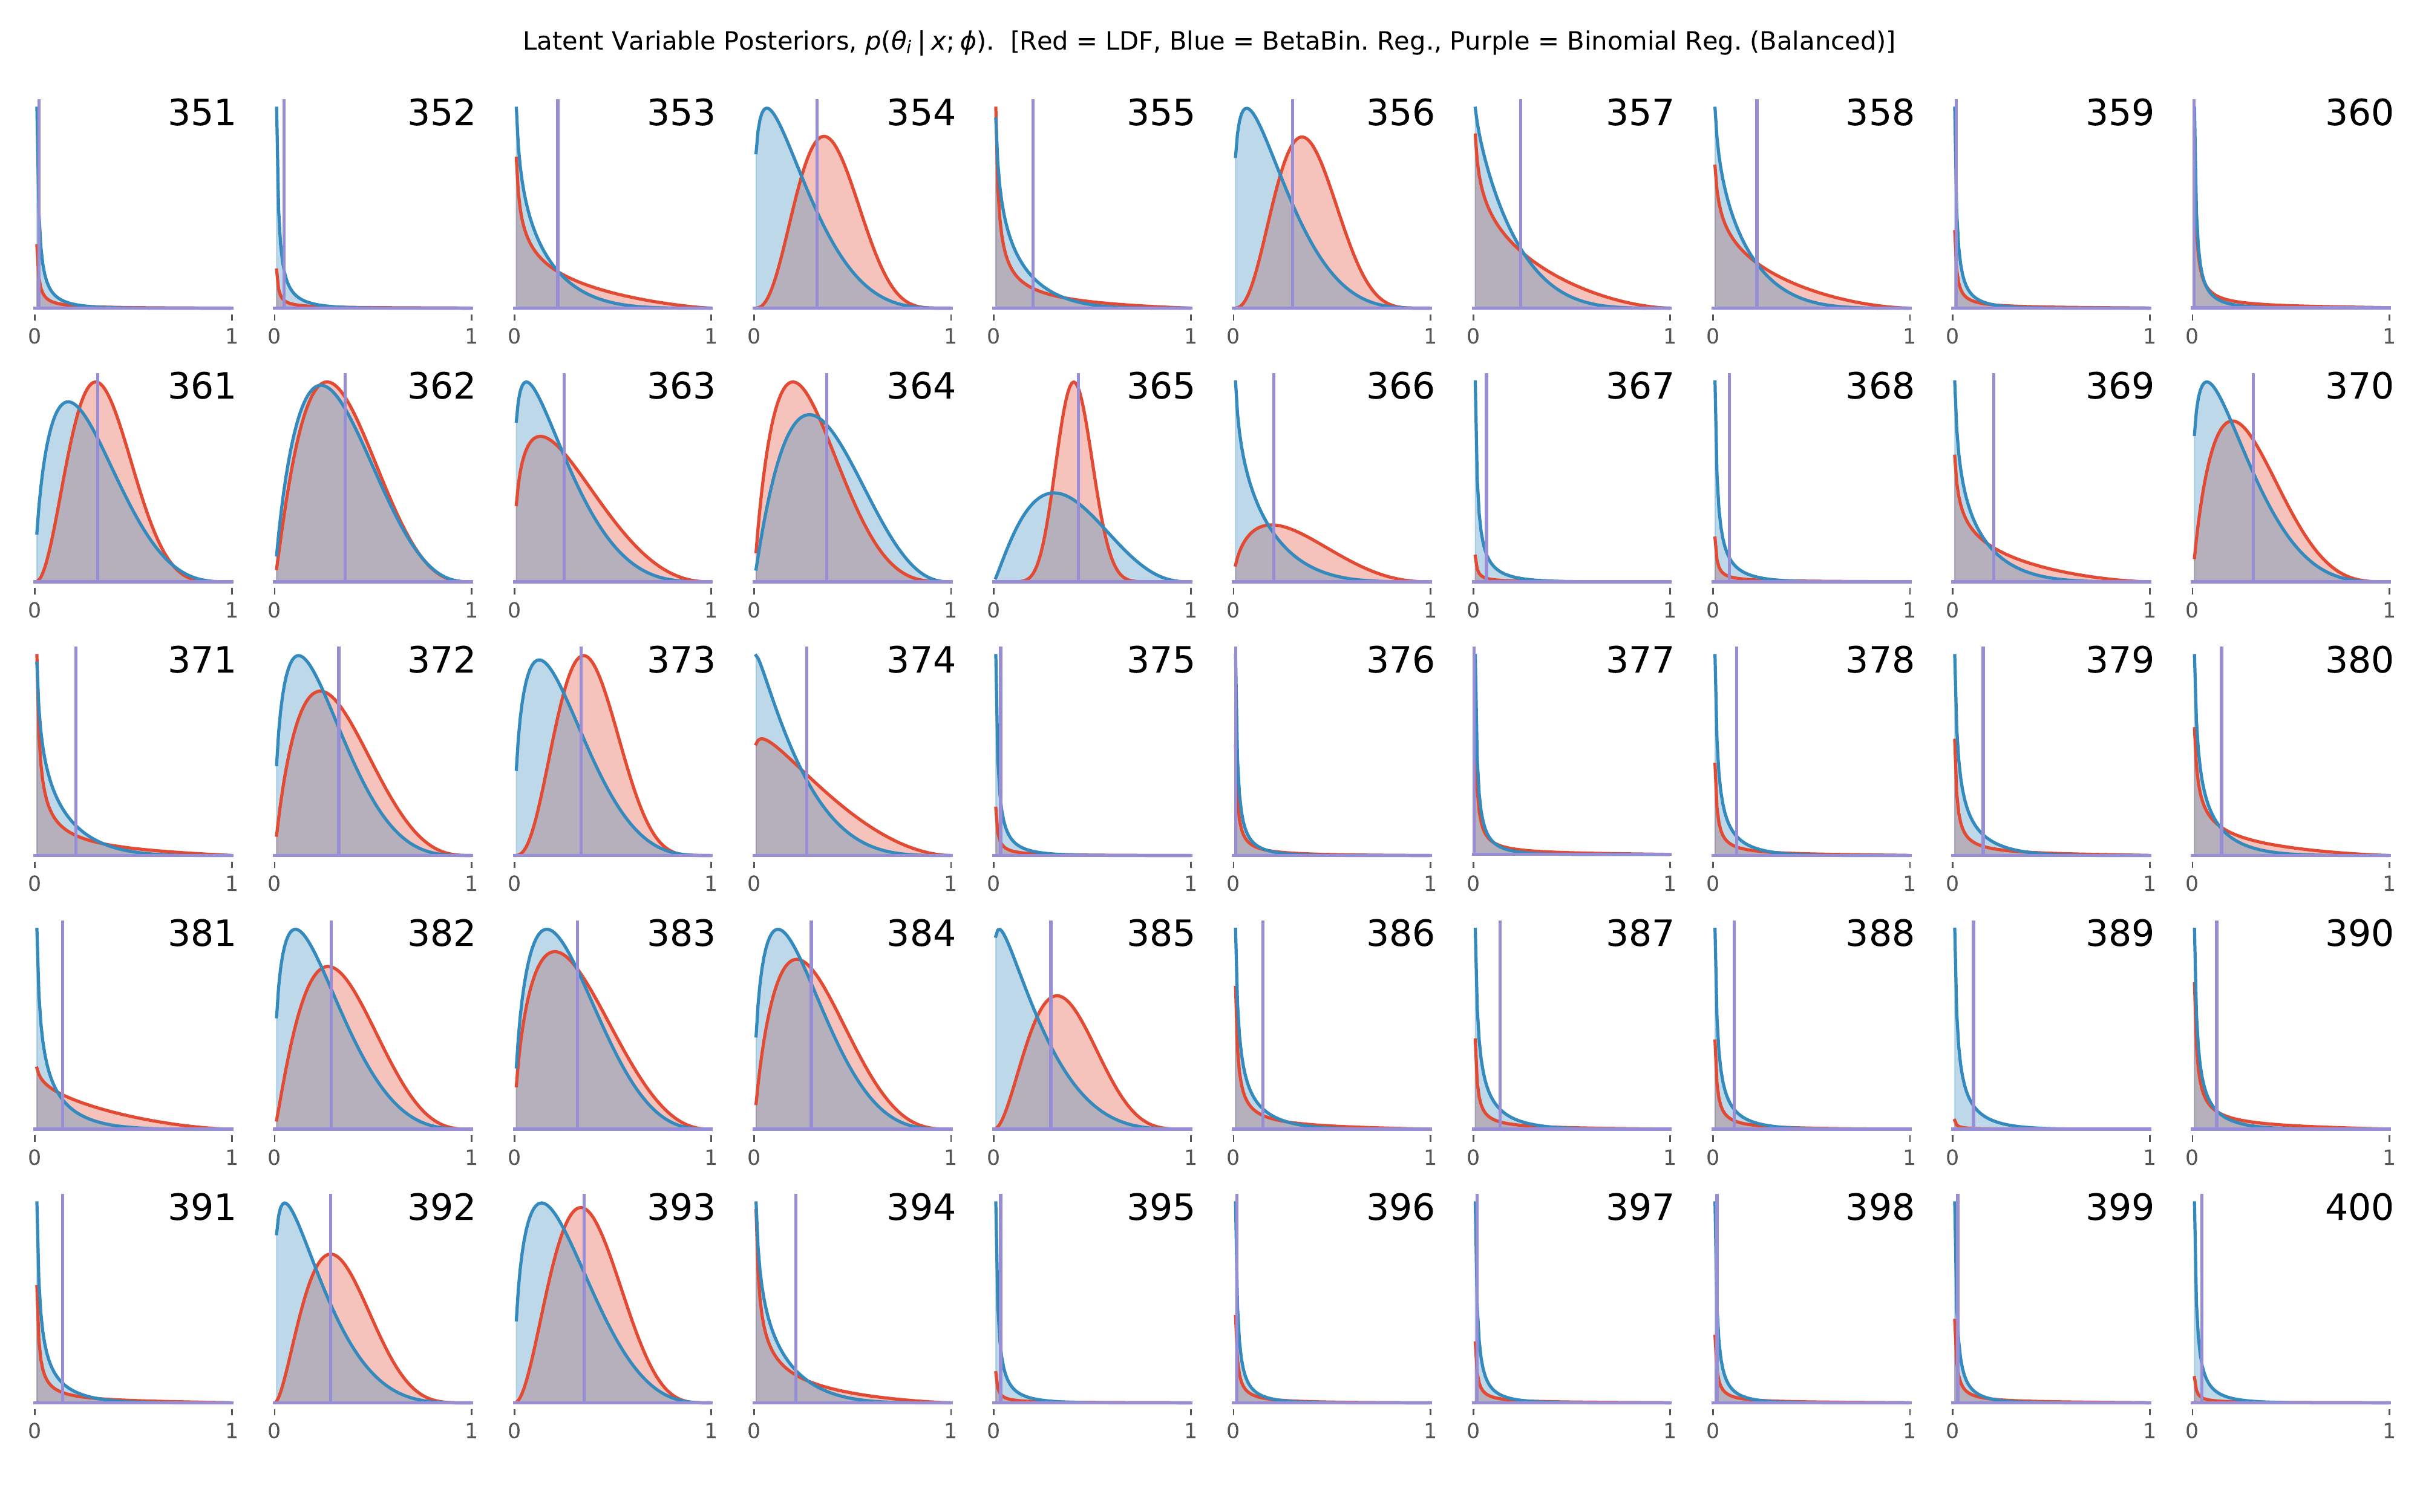}}
     \centerline{\includegraphics[width=0.75\linewidth, trim={0.375cm 1cm 0.375cm 1.5cm},clip]{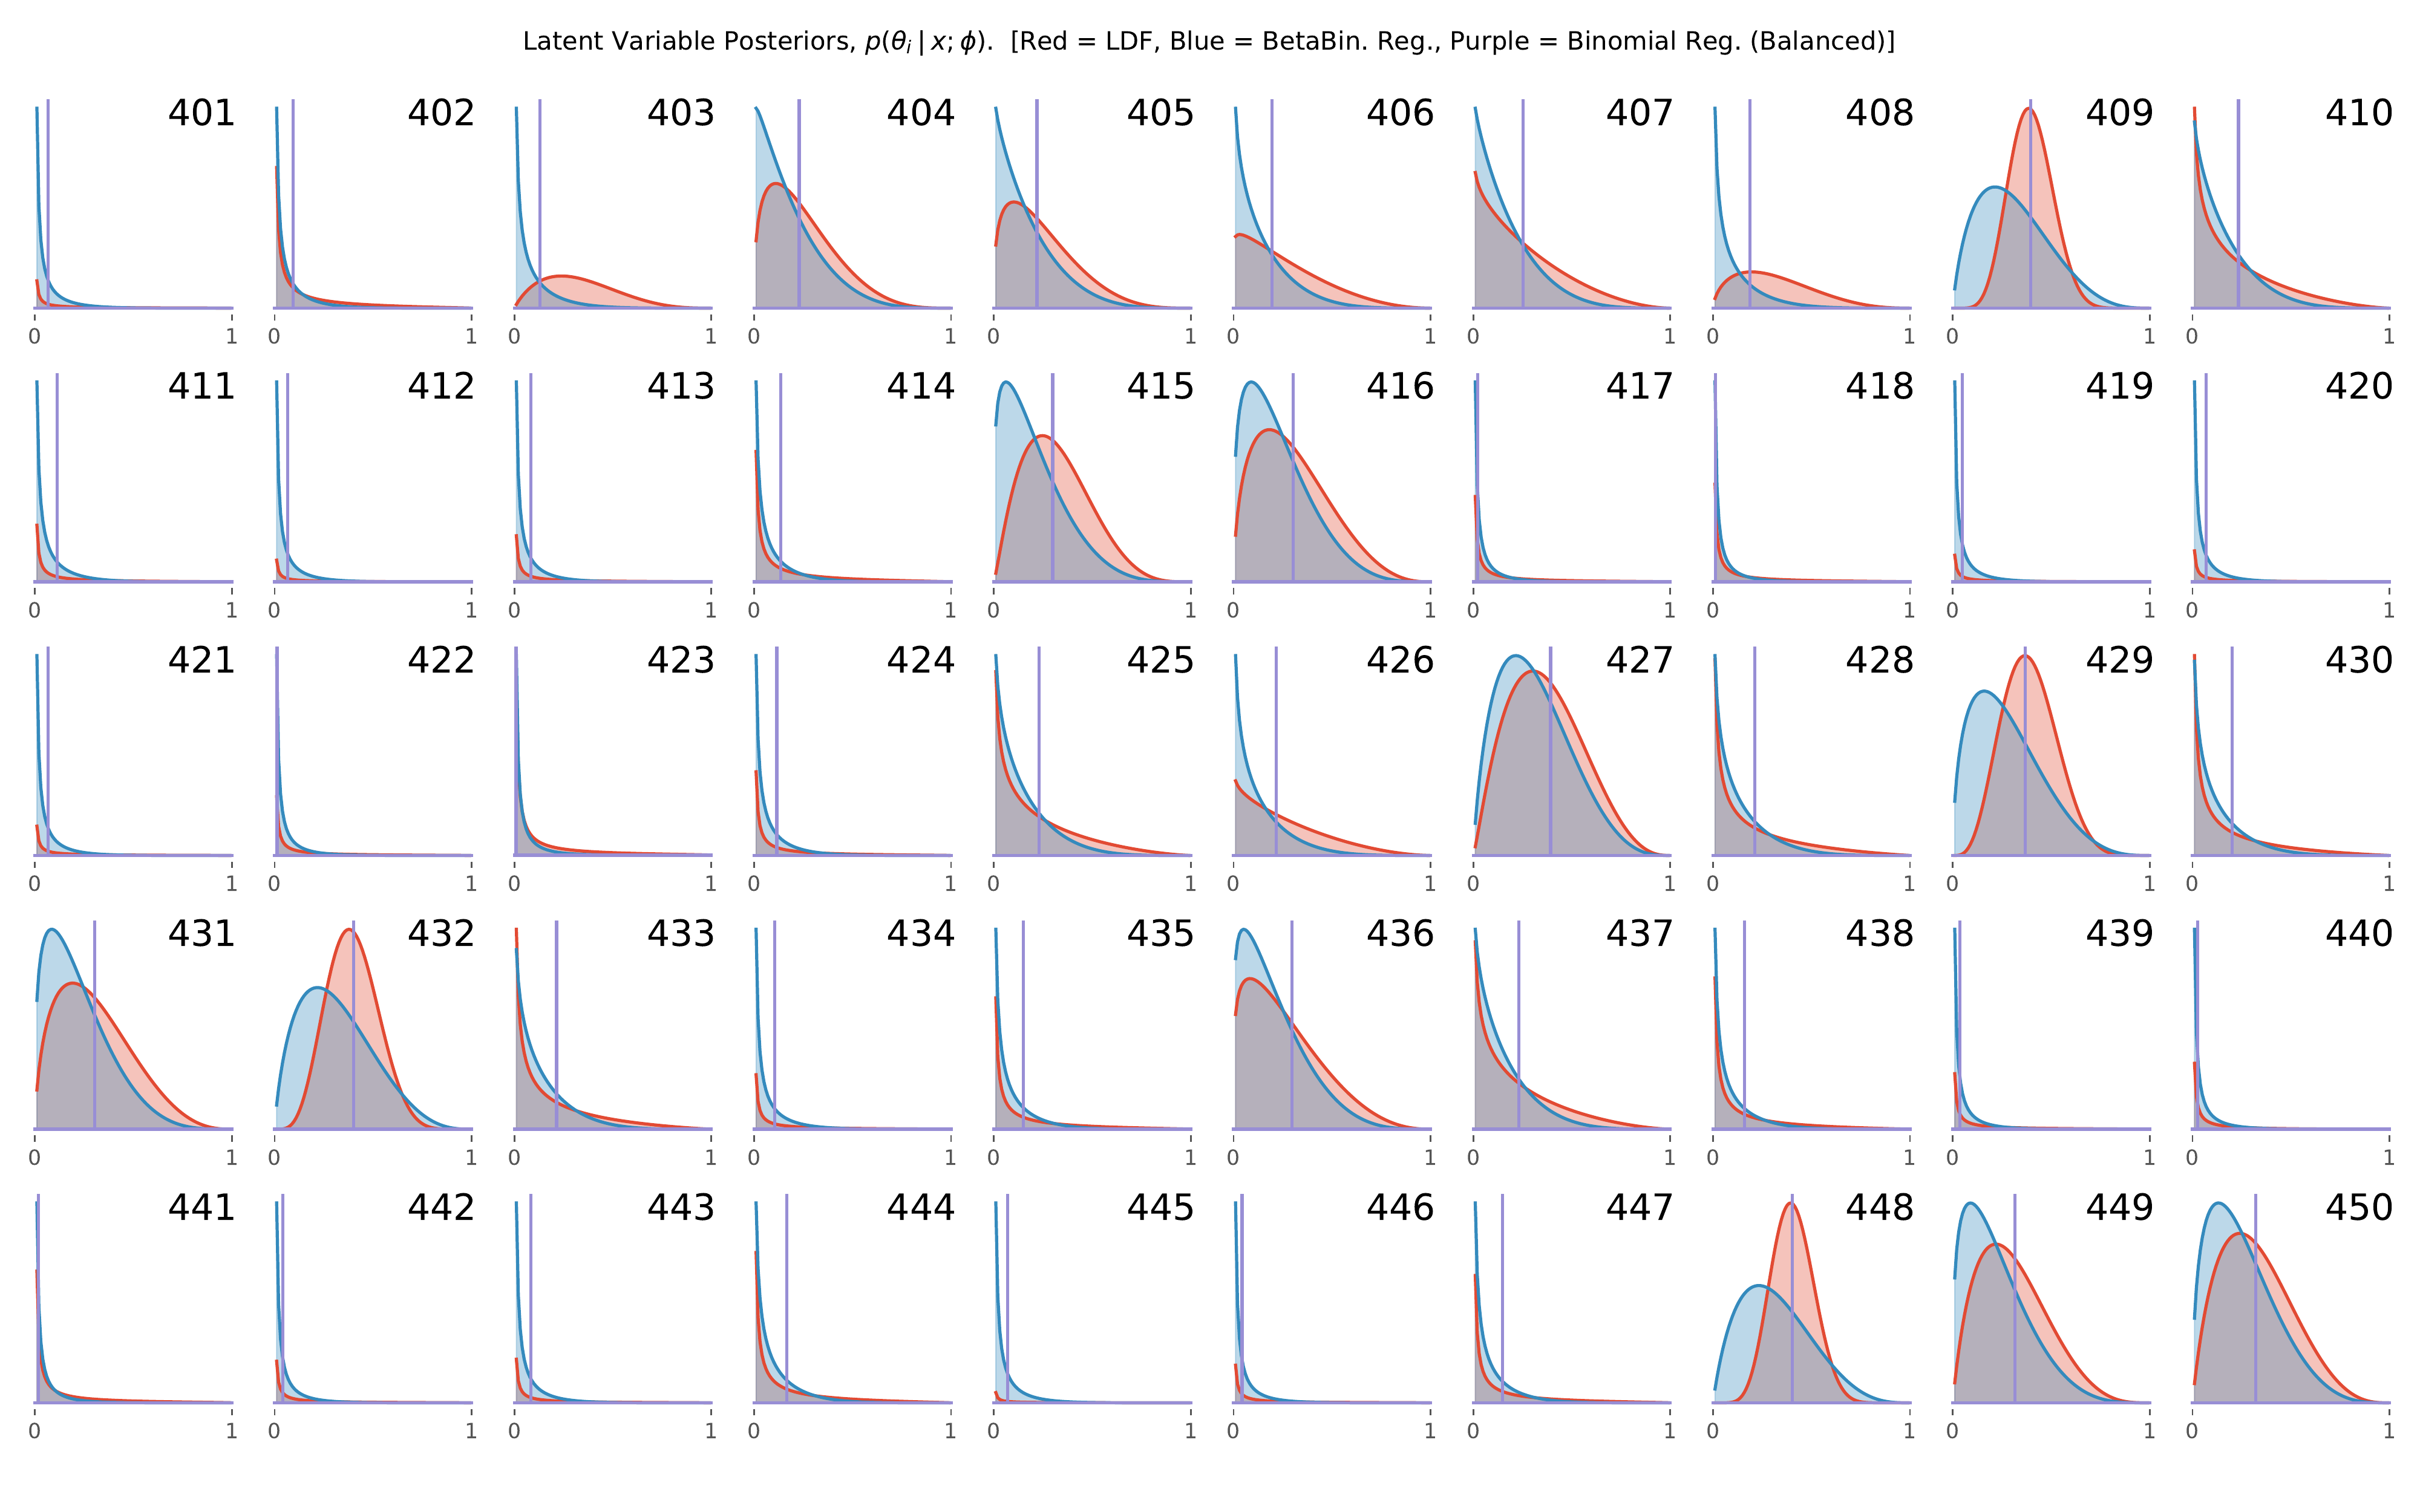}}
    \caption{\small \textbf{Latent variable posteriors (continued).}  A sample of the posteriors $p(\theta_i \given x; \phi)$ for the electrification application.  LDF is red, beta-binomial regression is blue, and binomial regression is purple.}
    
  \end{center}
  \vspace*{-5mm}
\end{figure}

\begin{figure}[t]
  \vskip 0.1in
  \begin{center}
    \centerline{\includegraphics[width=0.75\linewidth, trim={0.375cm 1cm 0.375cm 1.5cm},clip]{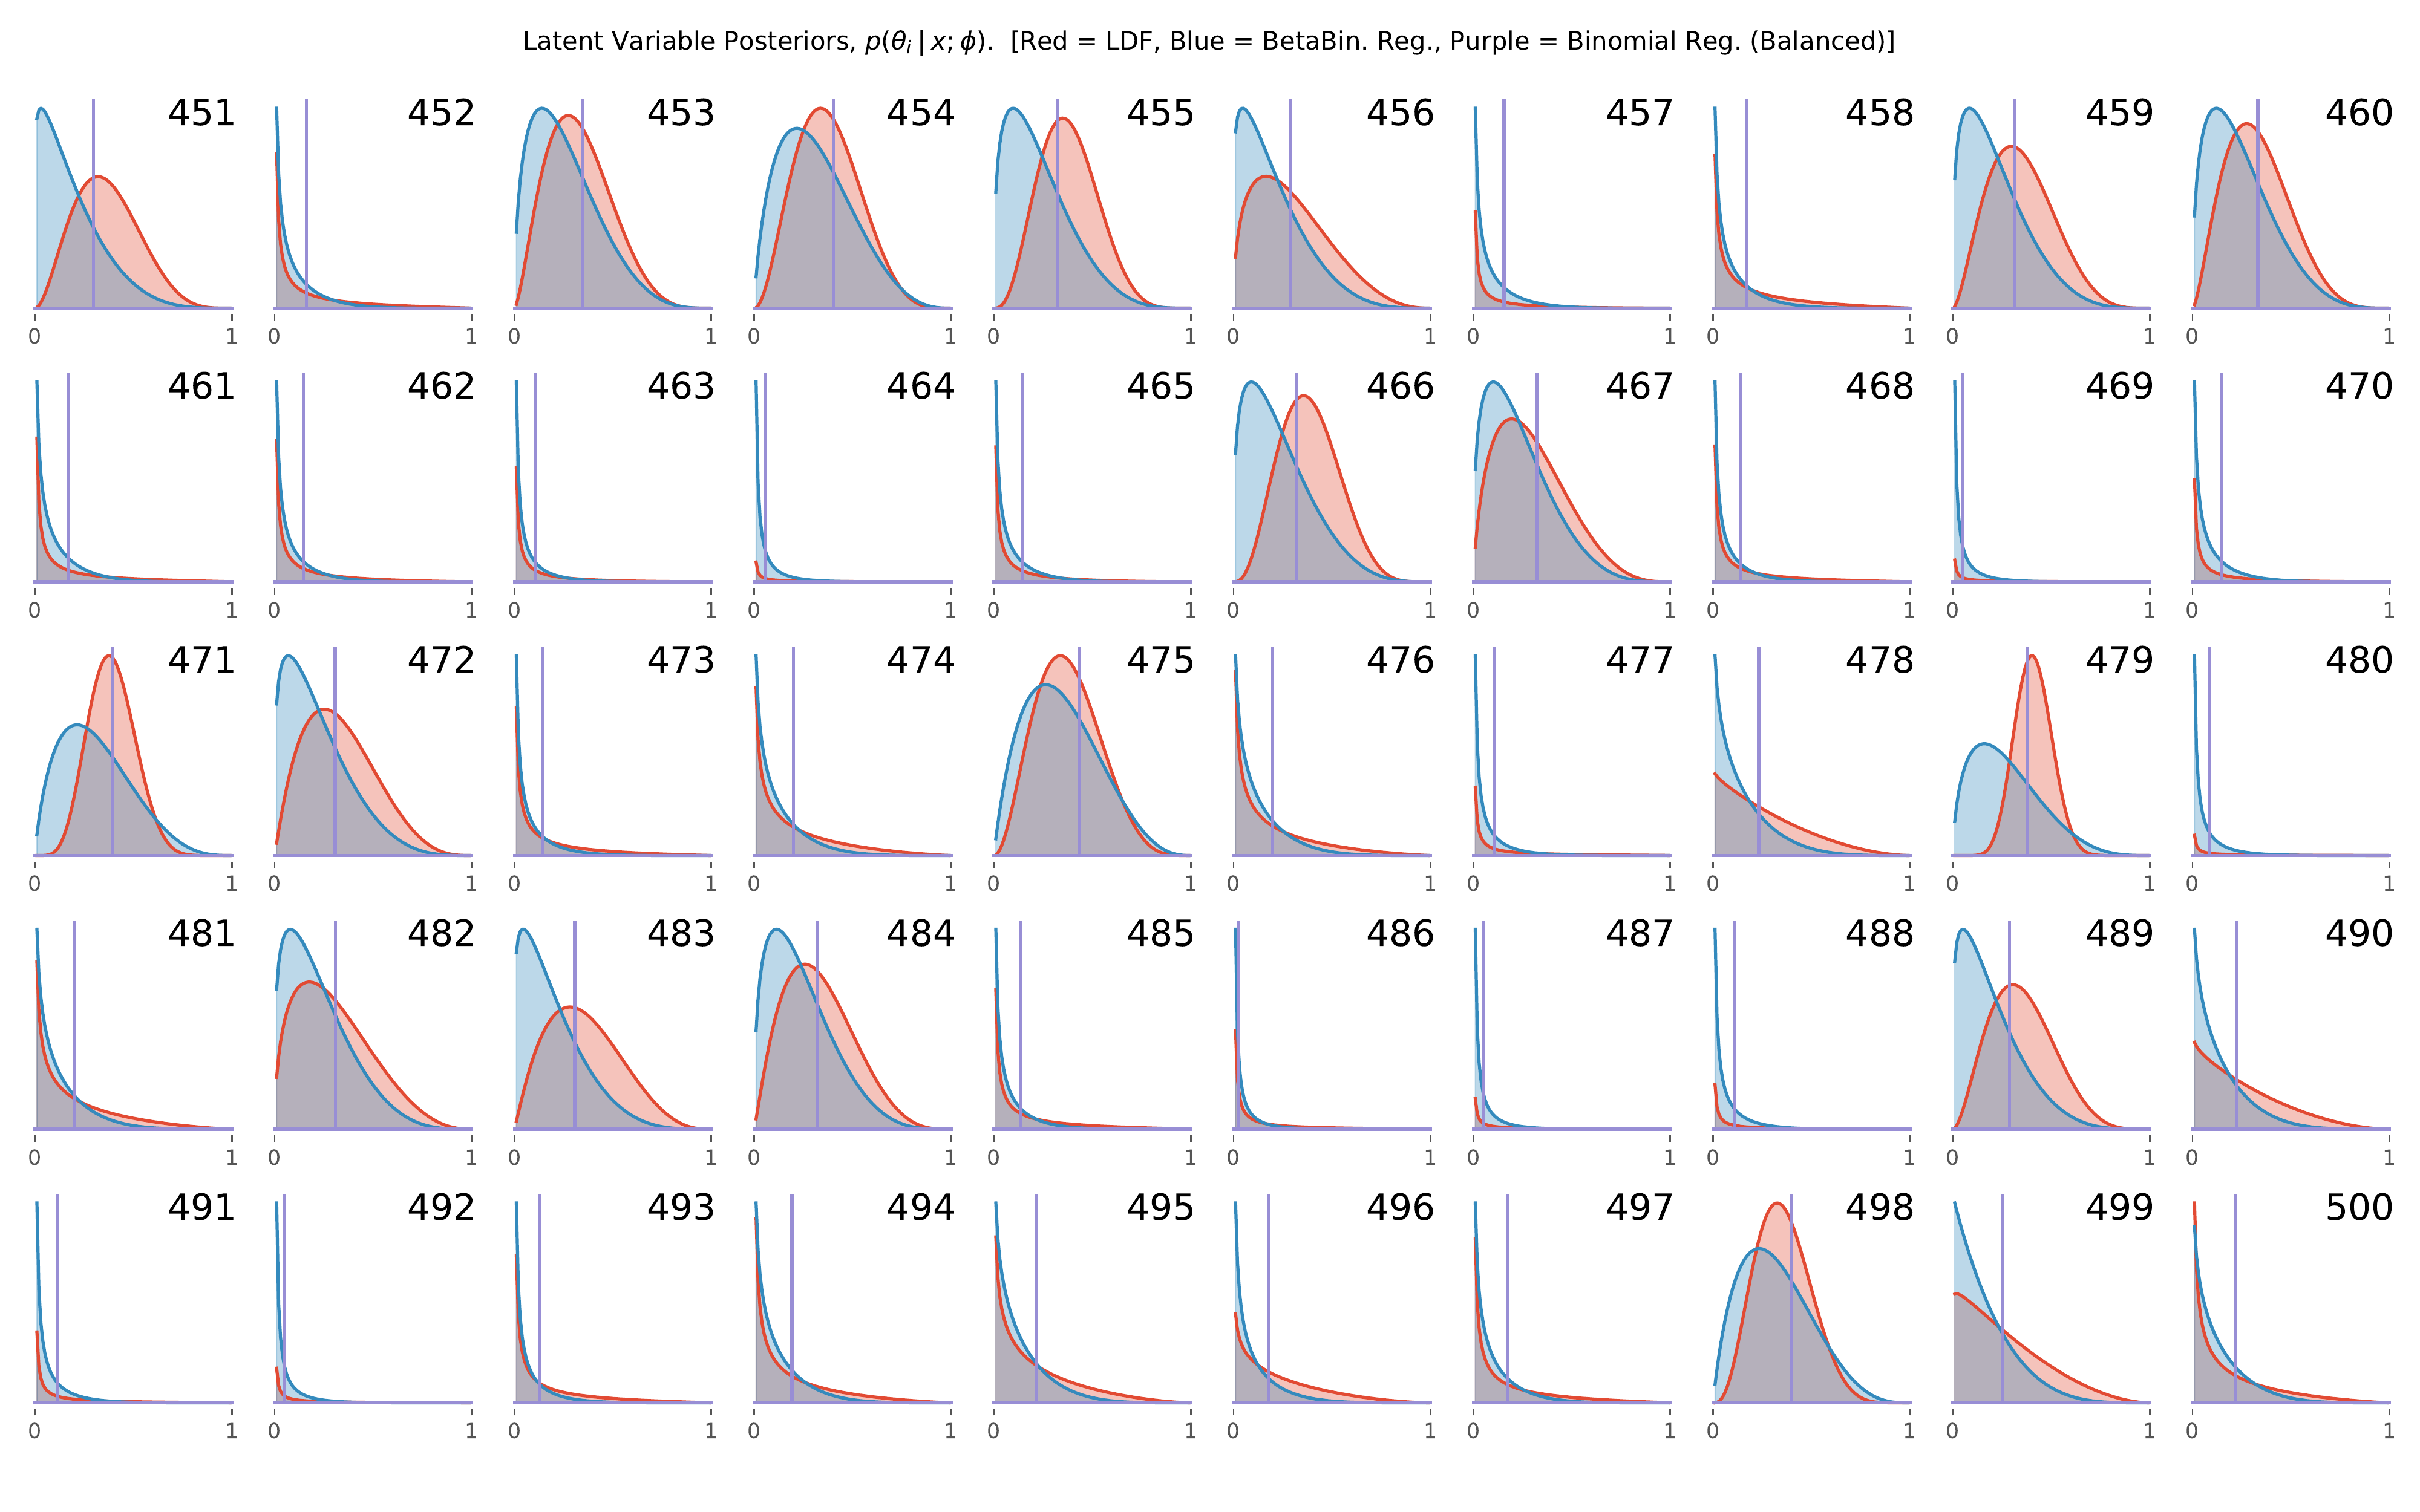}}
    \centerline{\includegraphics[width=0.75\linewidth, trim={0.375cm 1cm 0.375cm 1.5cm},clip]{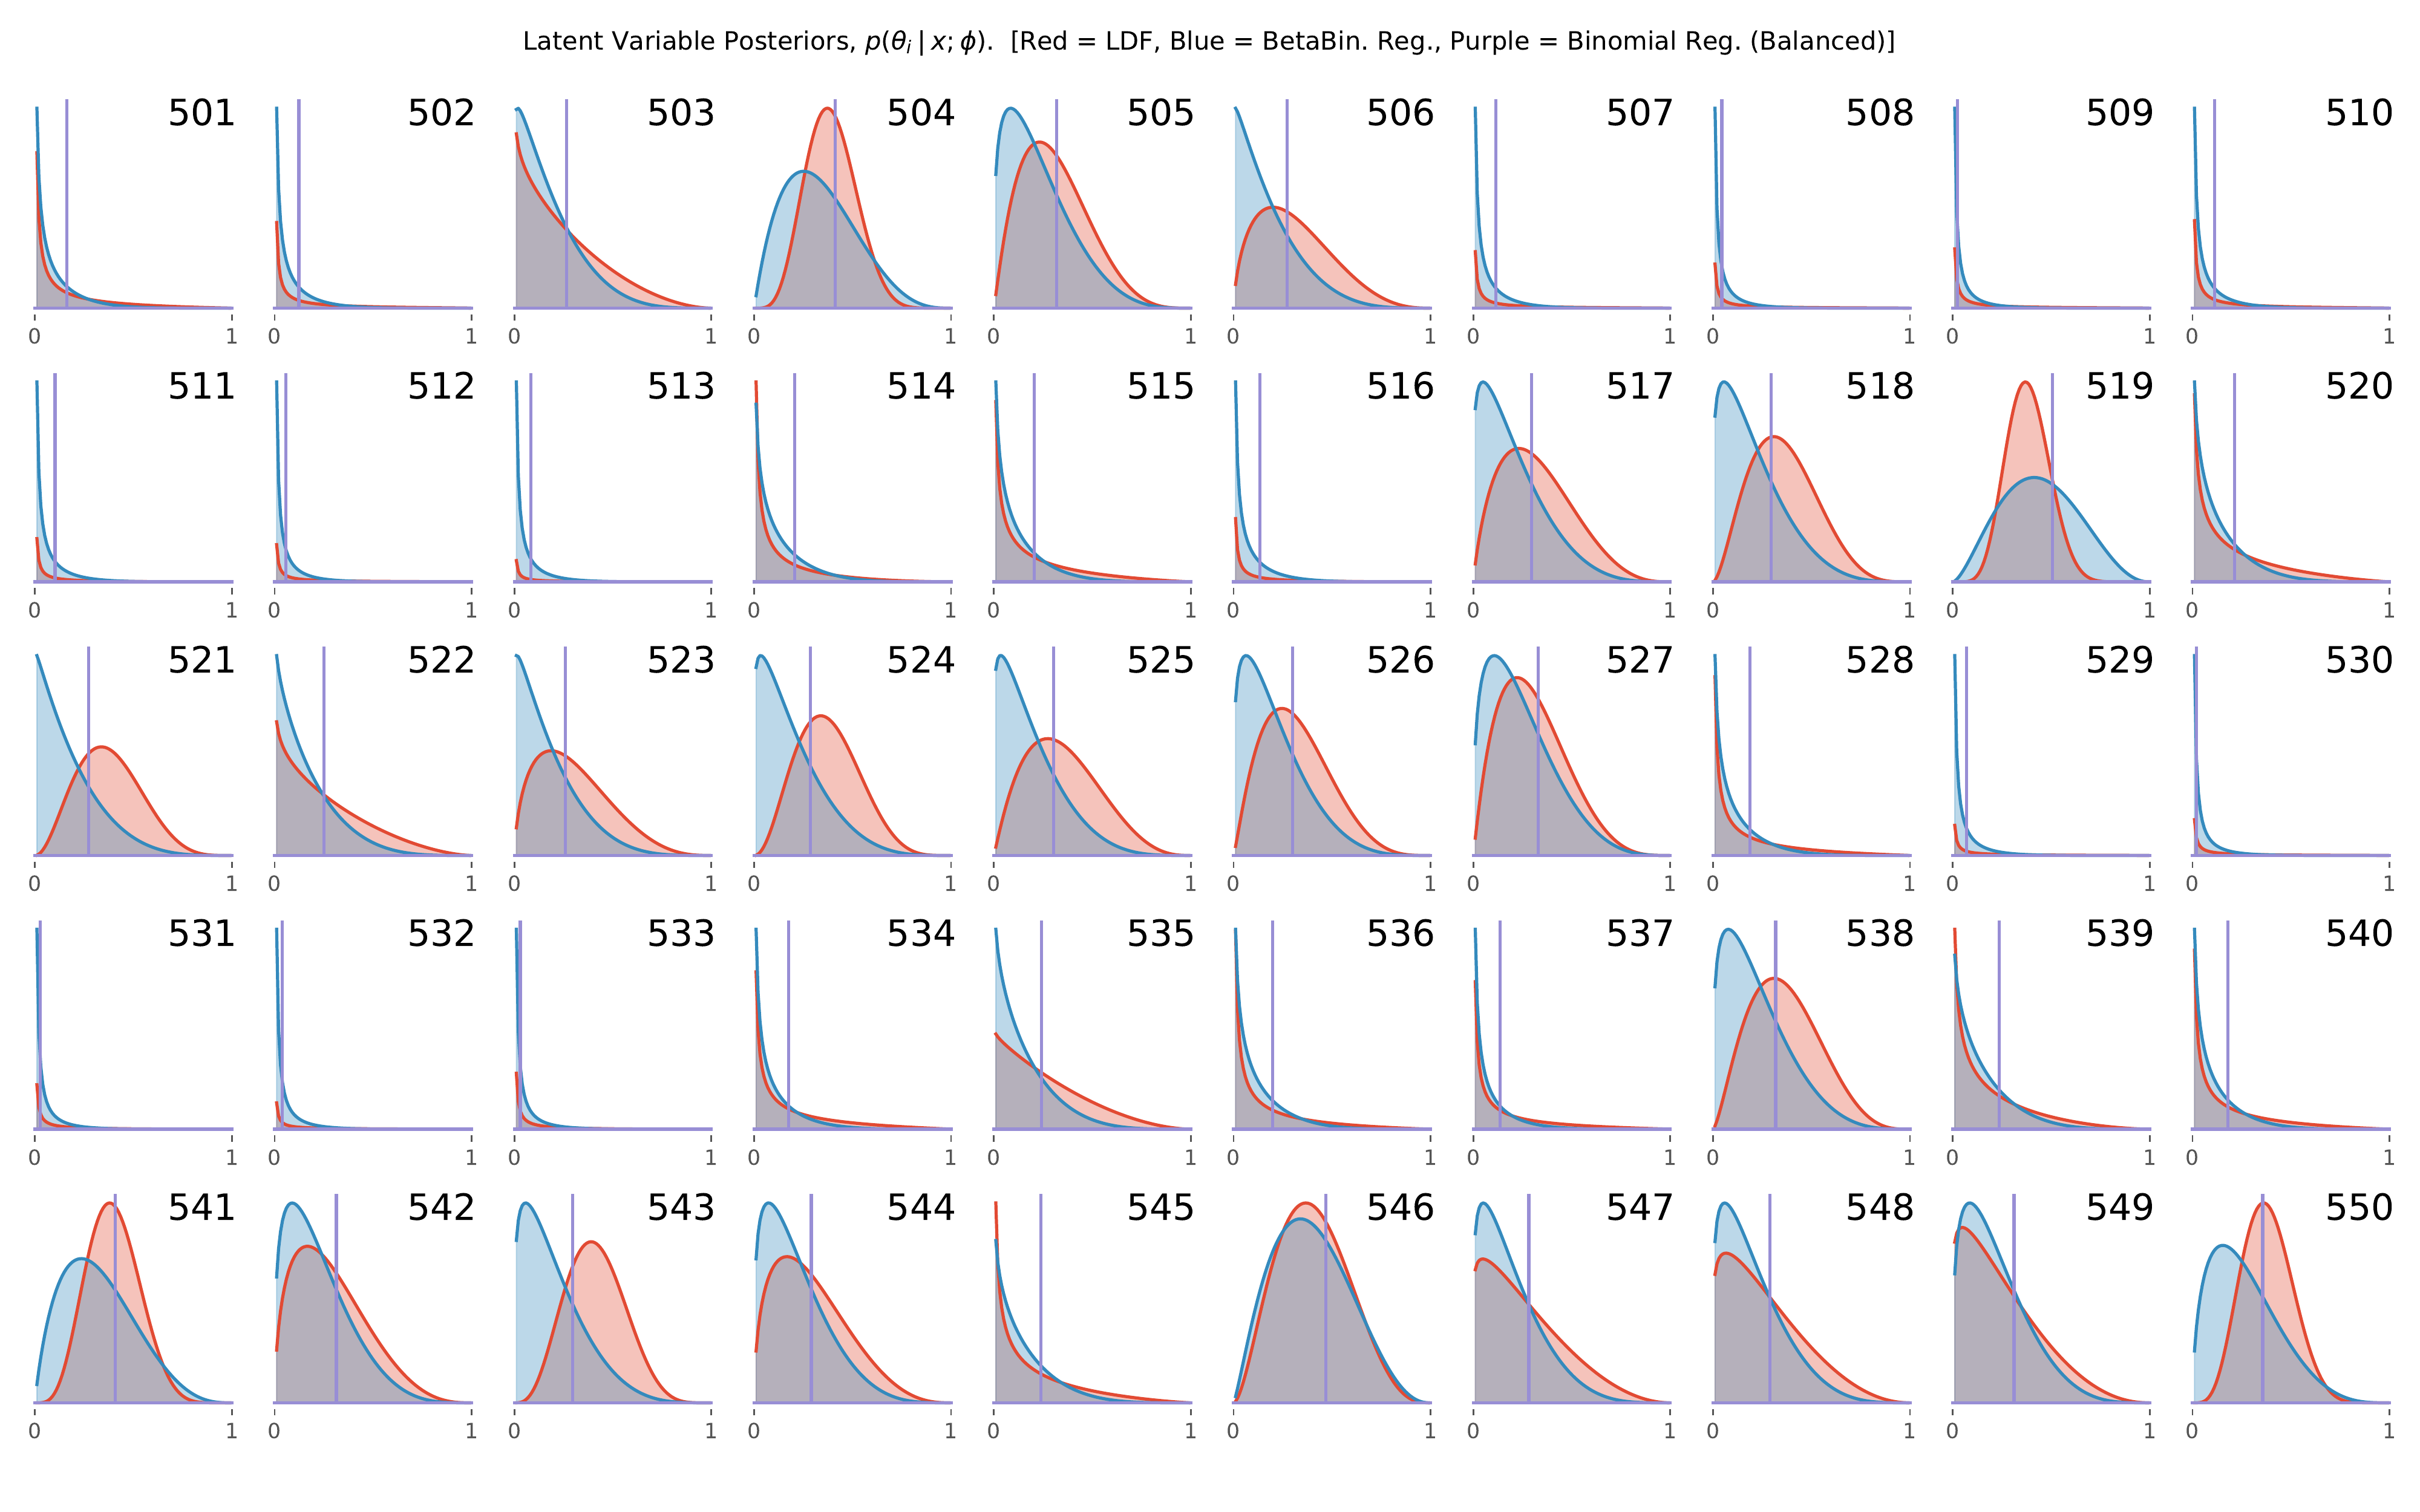}}
     \centerline{\includegraphics[width=0.75\linewidth, trim={0.375cm 1cm 0.375cm 1.5cm},clip]{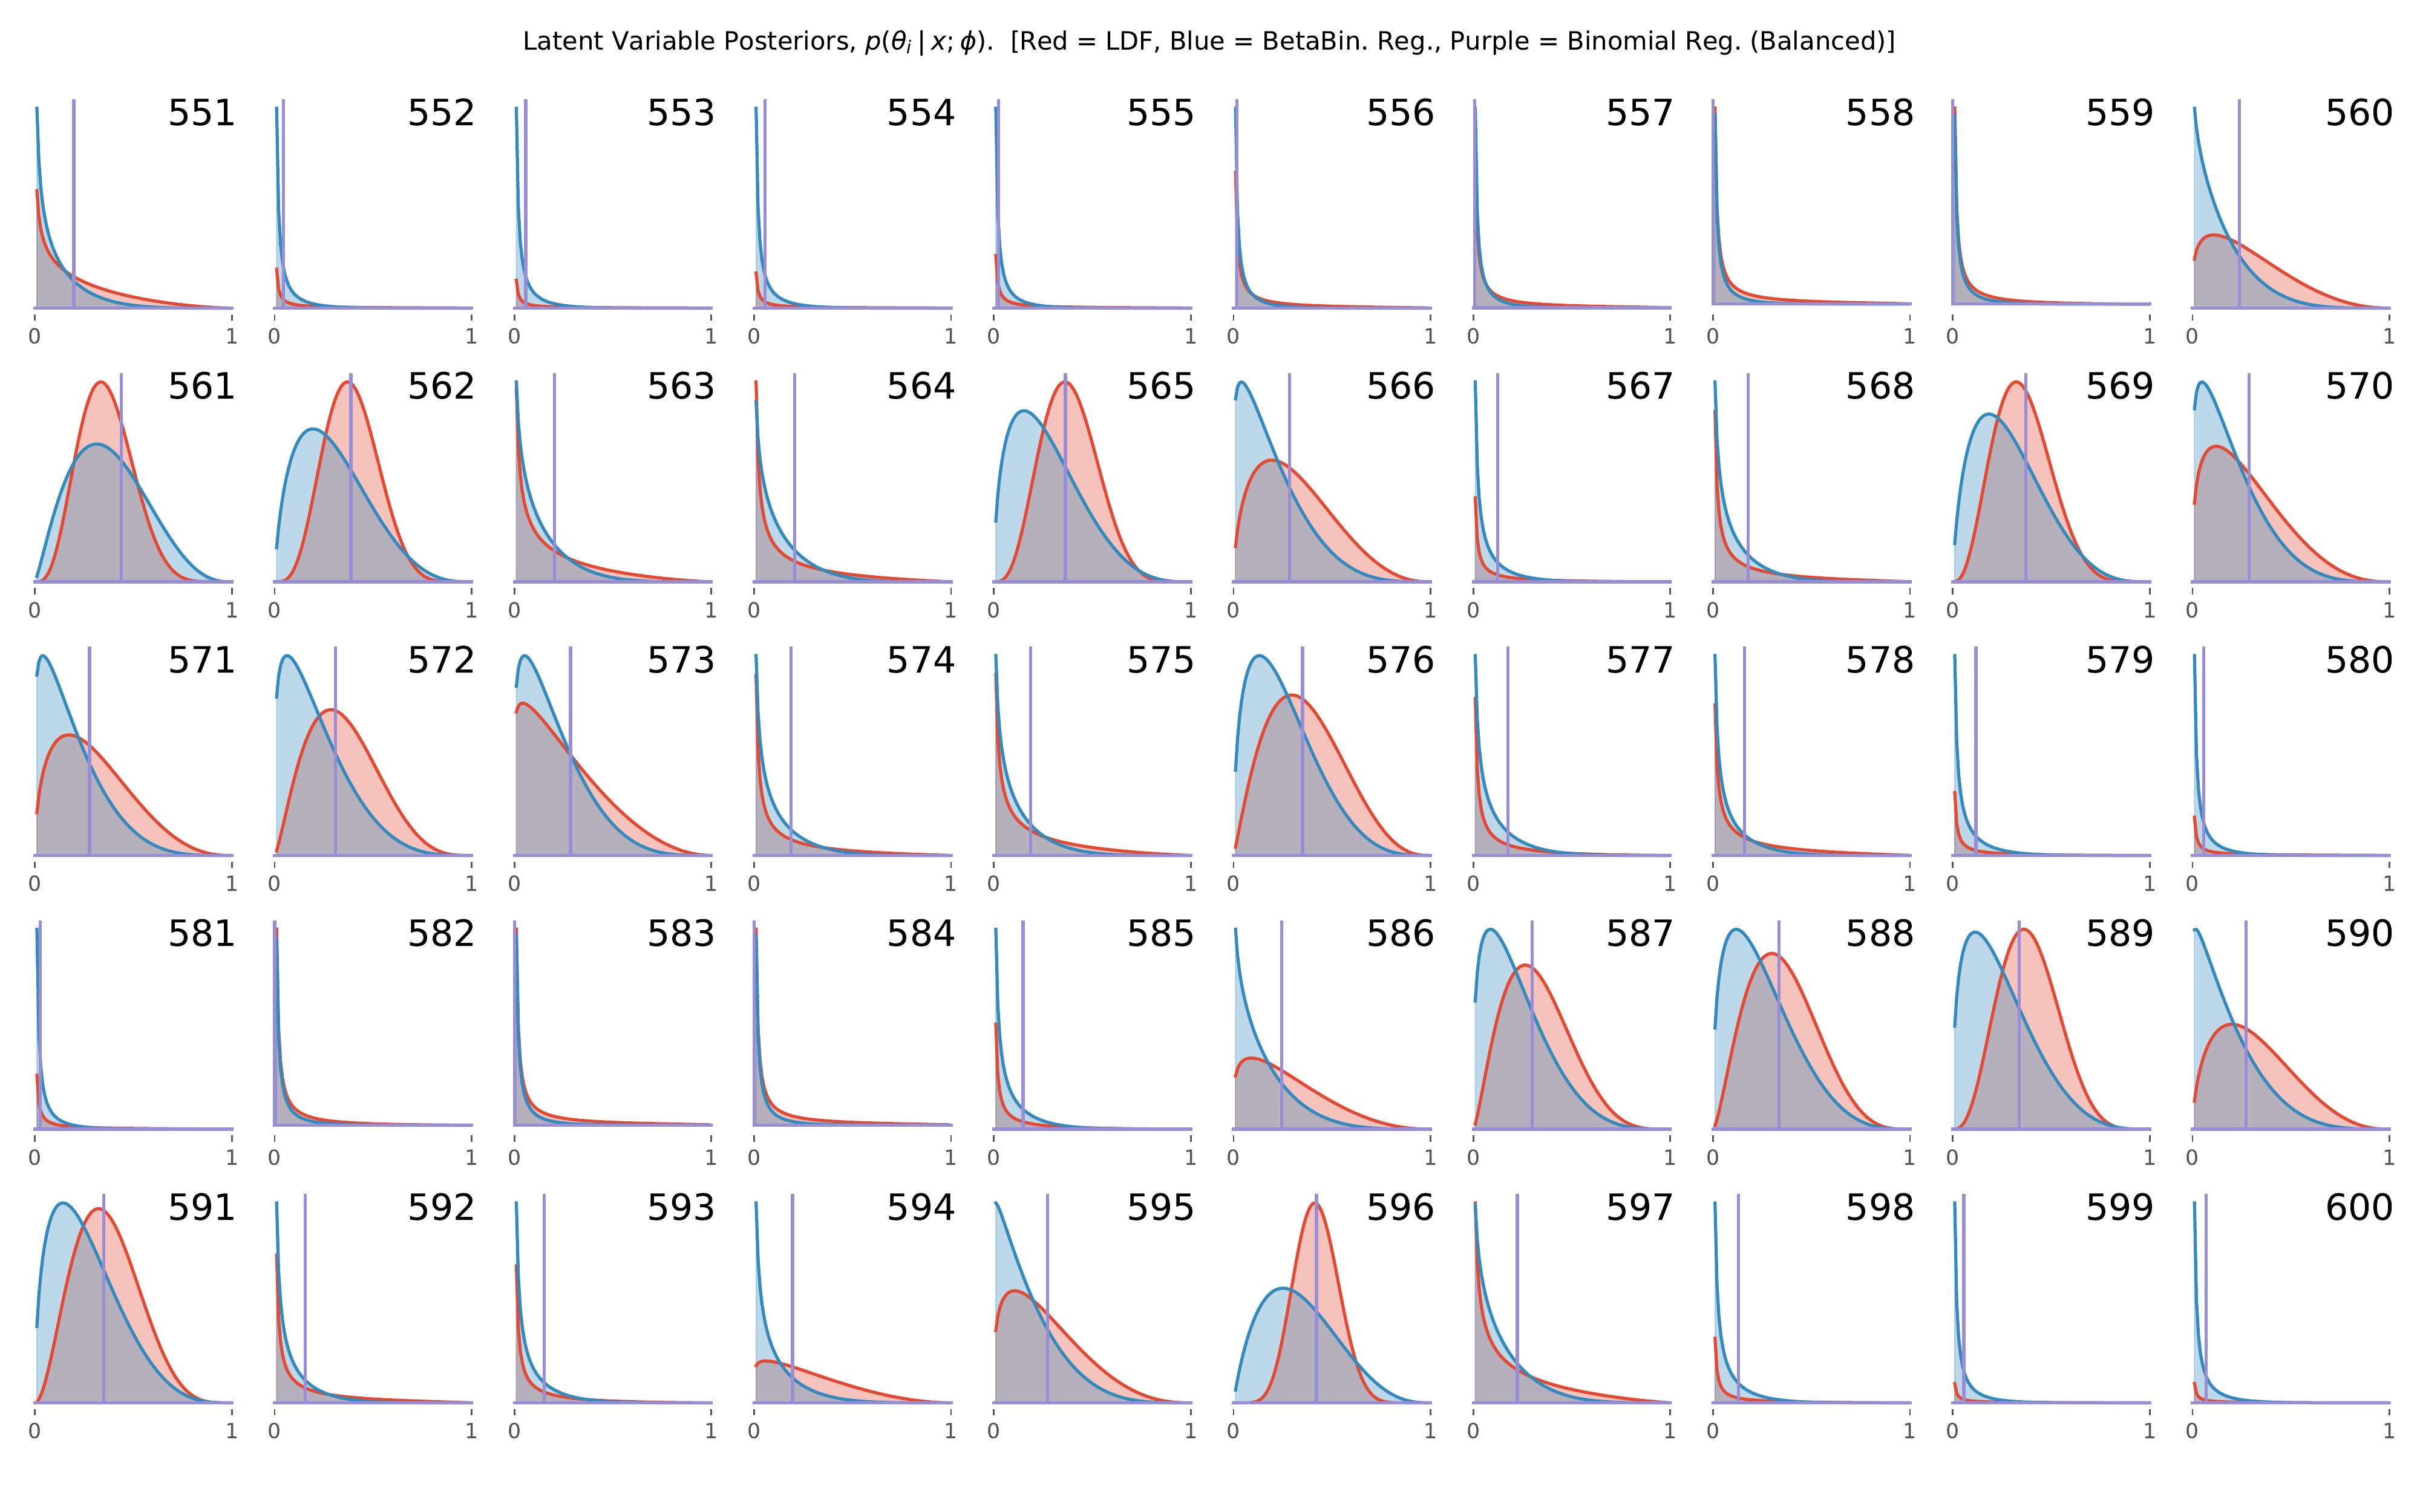}}
    \caption{\small \textbf{Latent variable posteriors (continued).}  A sample of the posteriors $p(\theta_i \given x; \phi)$ for the electrification application.  LDF is red, beta-binomial regression is blue, and binomial regression is purple.}
    
  \end{center}
  \vspace*{-5mm}
\end{figure}

\begin{figure}[t]
  \vskip 0.1in
  \begin{center}
    \centerline{\includegraphics[width=0.75\linewidth, trim={0.375cm 1cm 0.375cm 1.5cm},clip]{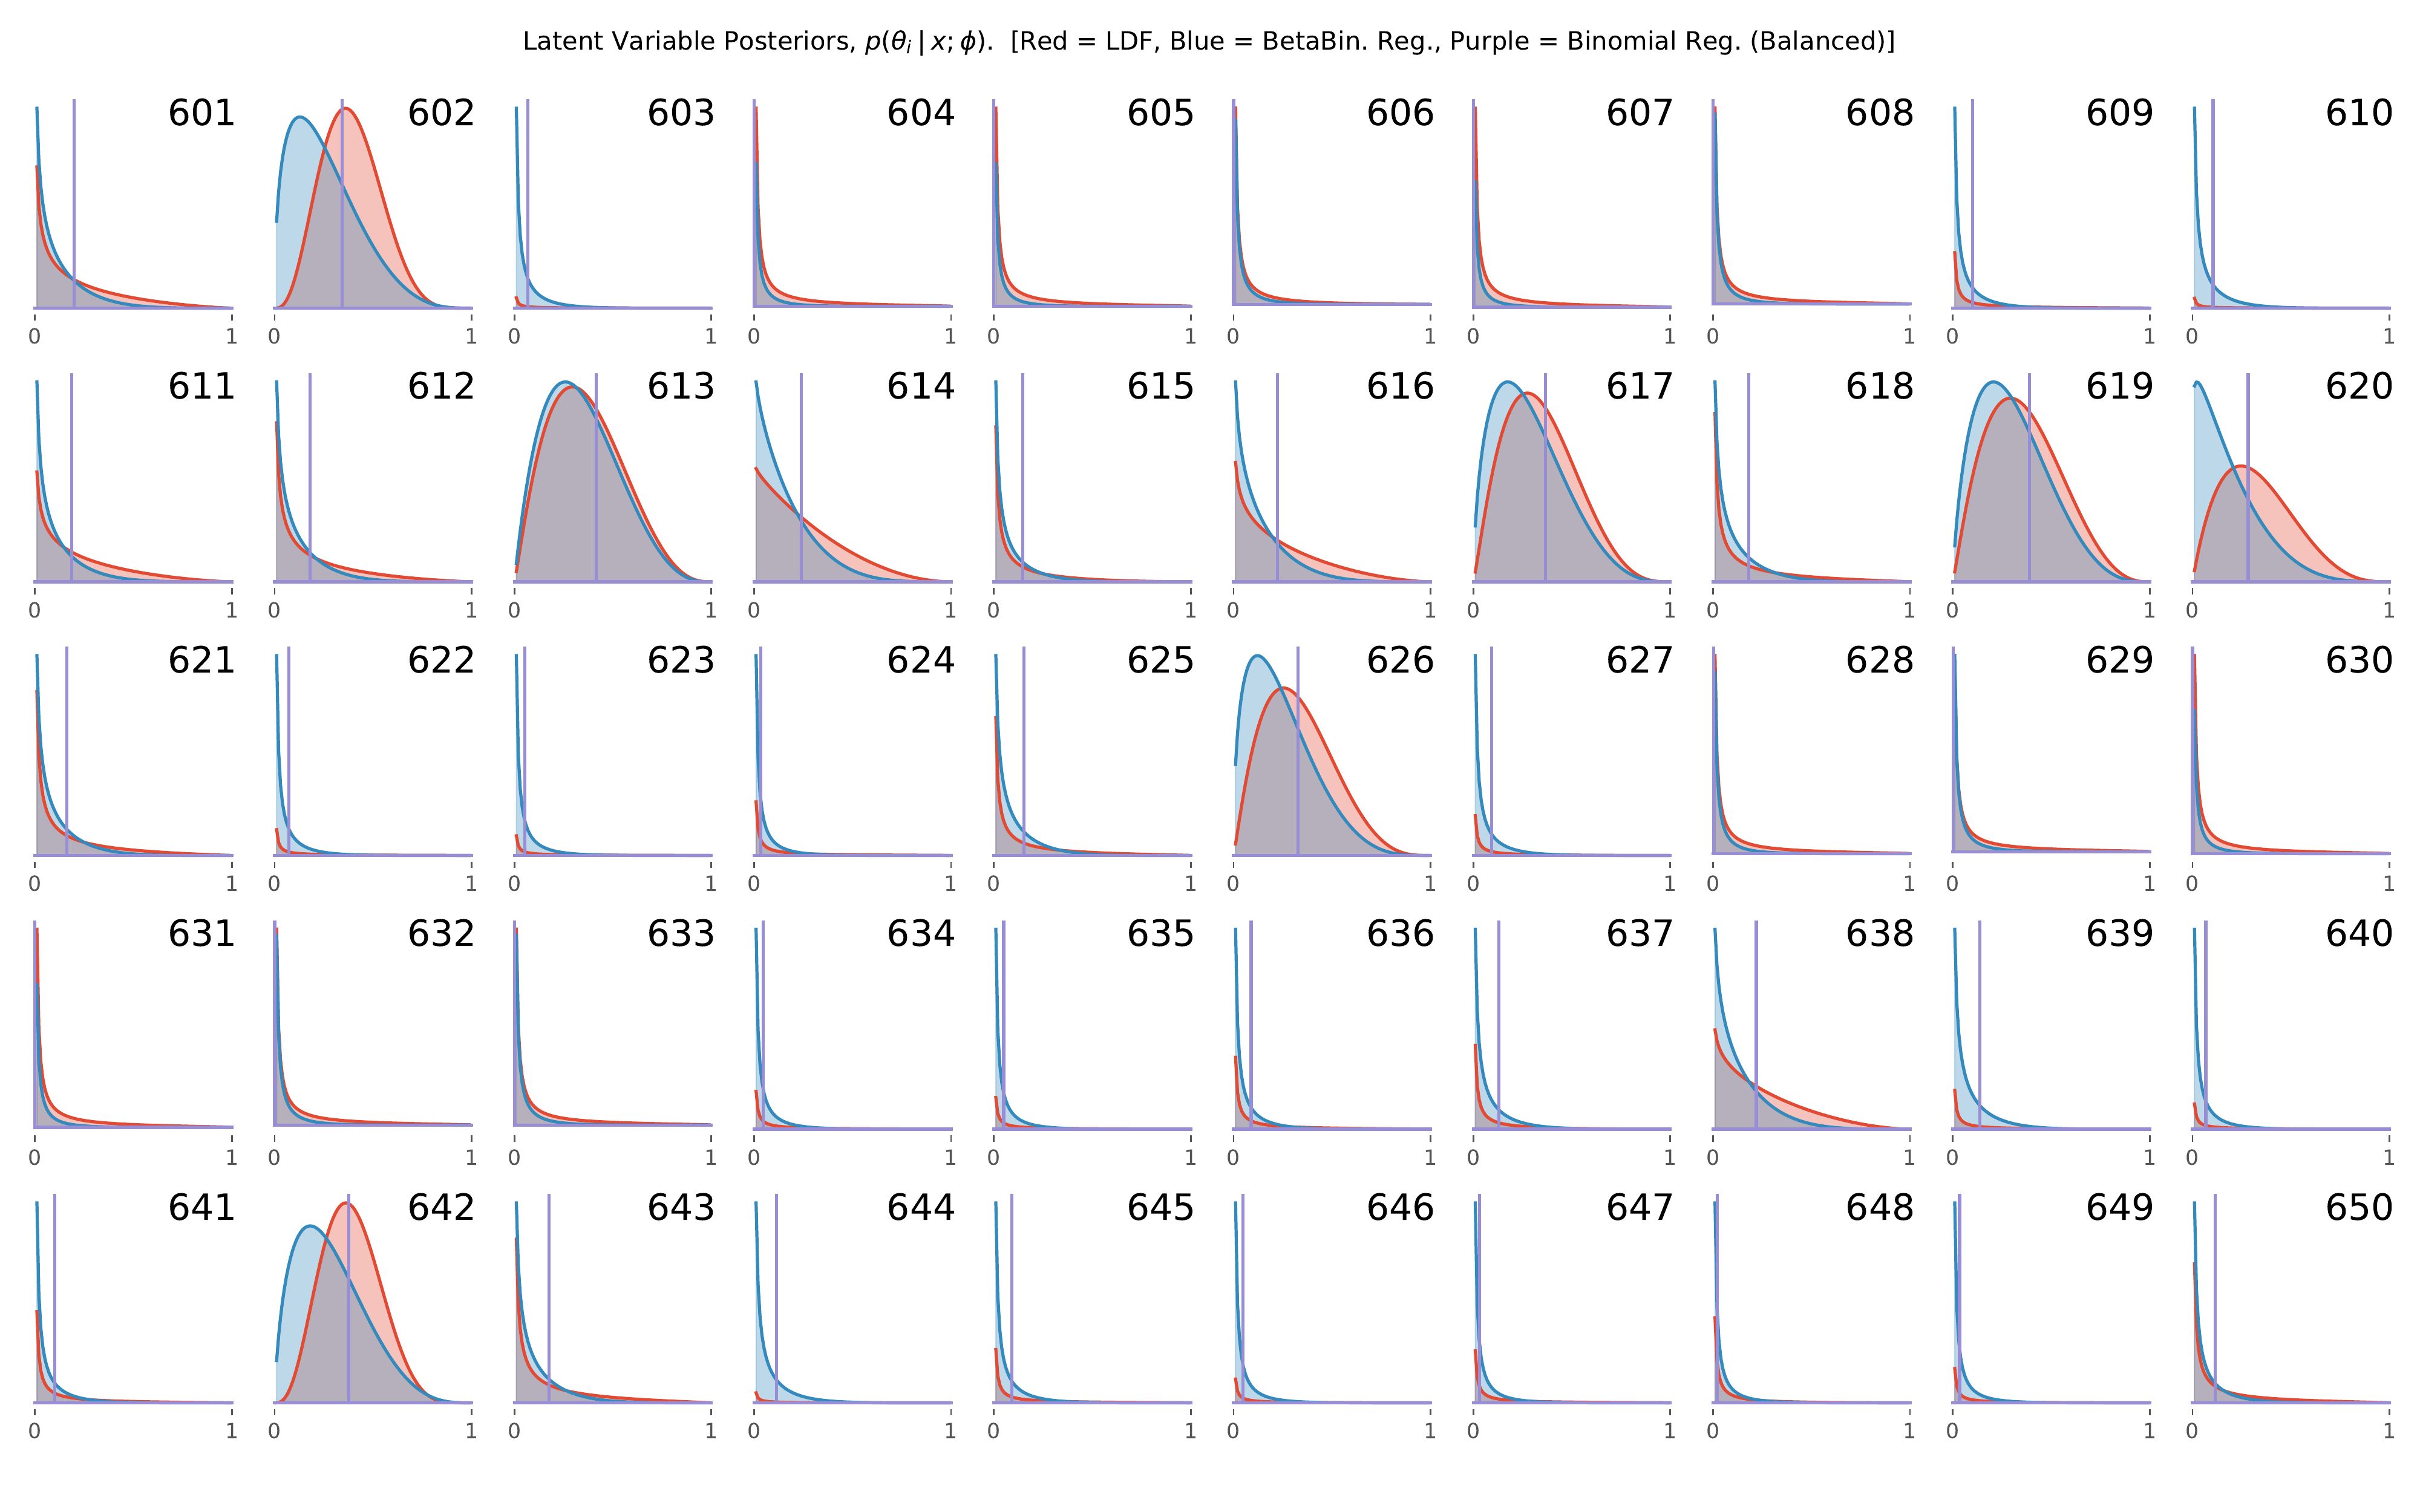}}
    \centerline{\includegraphics[width=0.75\linewidth, trim={0.375cm 1cm 0.375cm 1.5cm},clip]{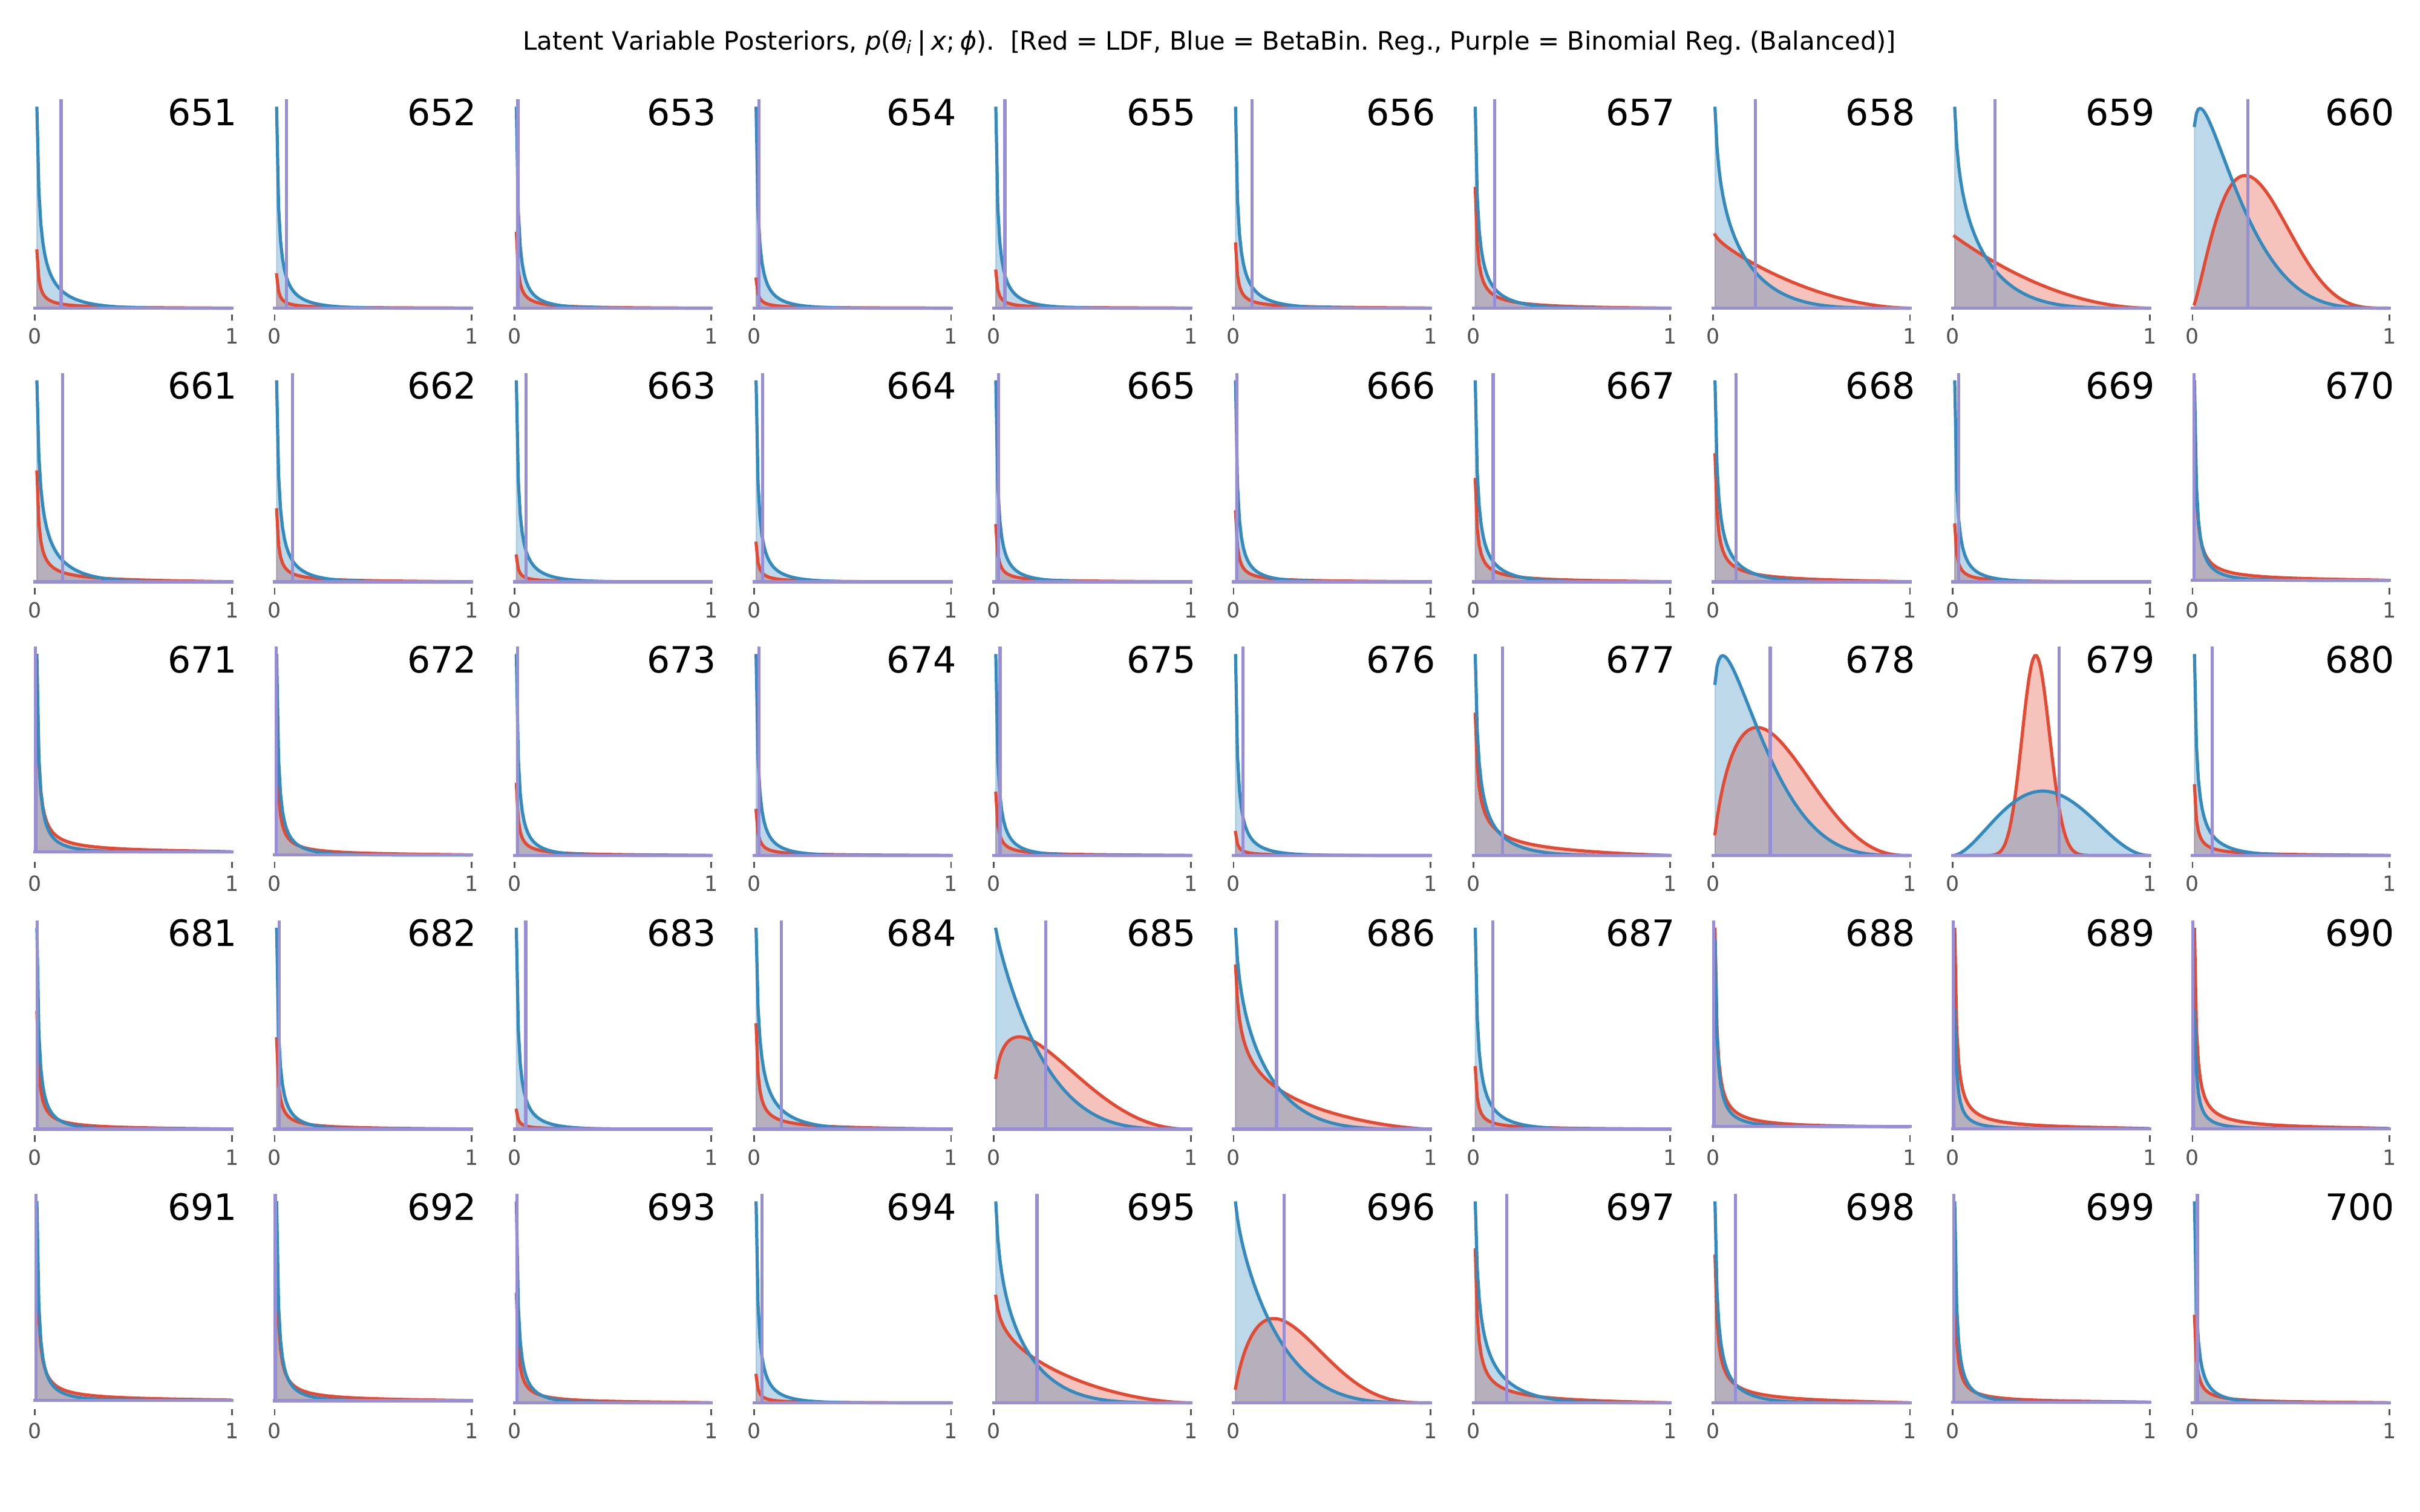}}
     \centerline{\includegraphics[width=0.75\linewidth, trim={0.375cm 1cm 0.375cm 1.5cm},clip]{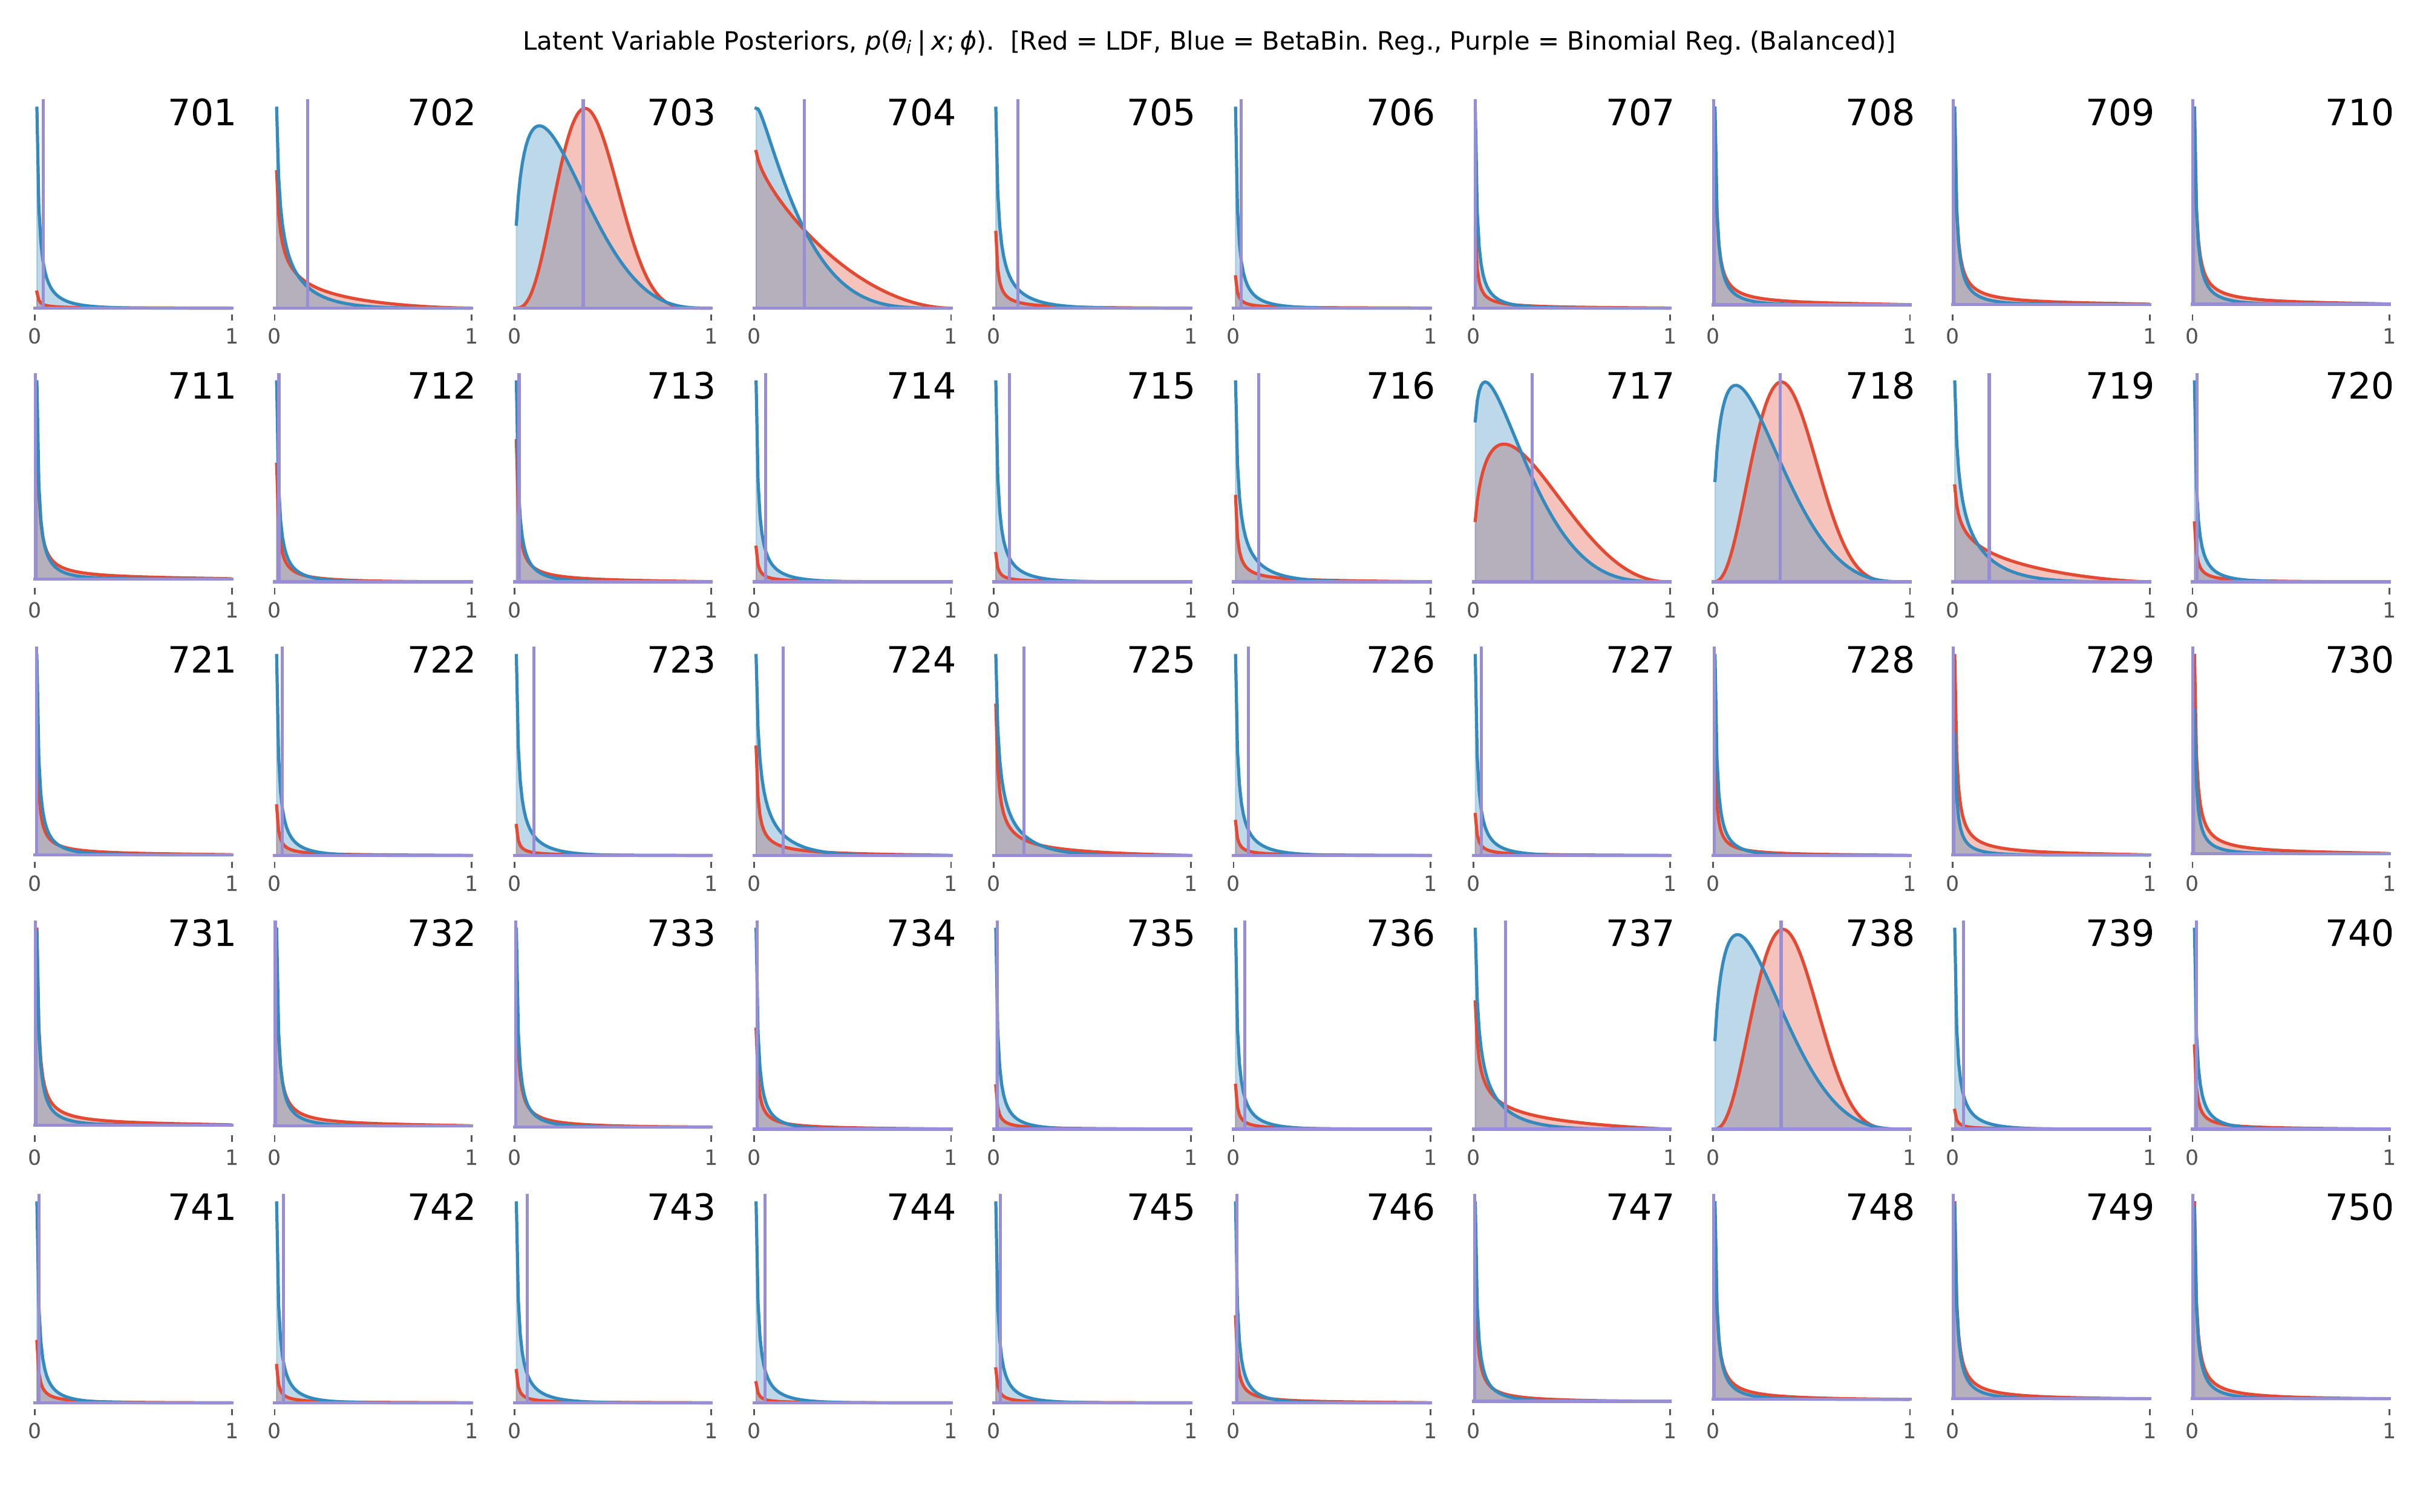}}
    \caption{\small \textbf{Latent variable posteriors (continued).}  A sample of the posteriors $p(\theta_i \given x; \phi)$ for the electrification application.  LDF is red, beta-binomial regression is blue, and binomial regression is purple.}
    
  \end{center}
  \vspace*{-5mm}
\end{figure}

\begin{figure}[t]
  \vskip 0.1in
  \begin{center}
    \centerline{\includegraphics[width=0.75\linewidth, trim={0.375cm 1cm 0.375cm 1.5cm},clip]{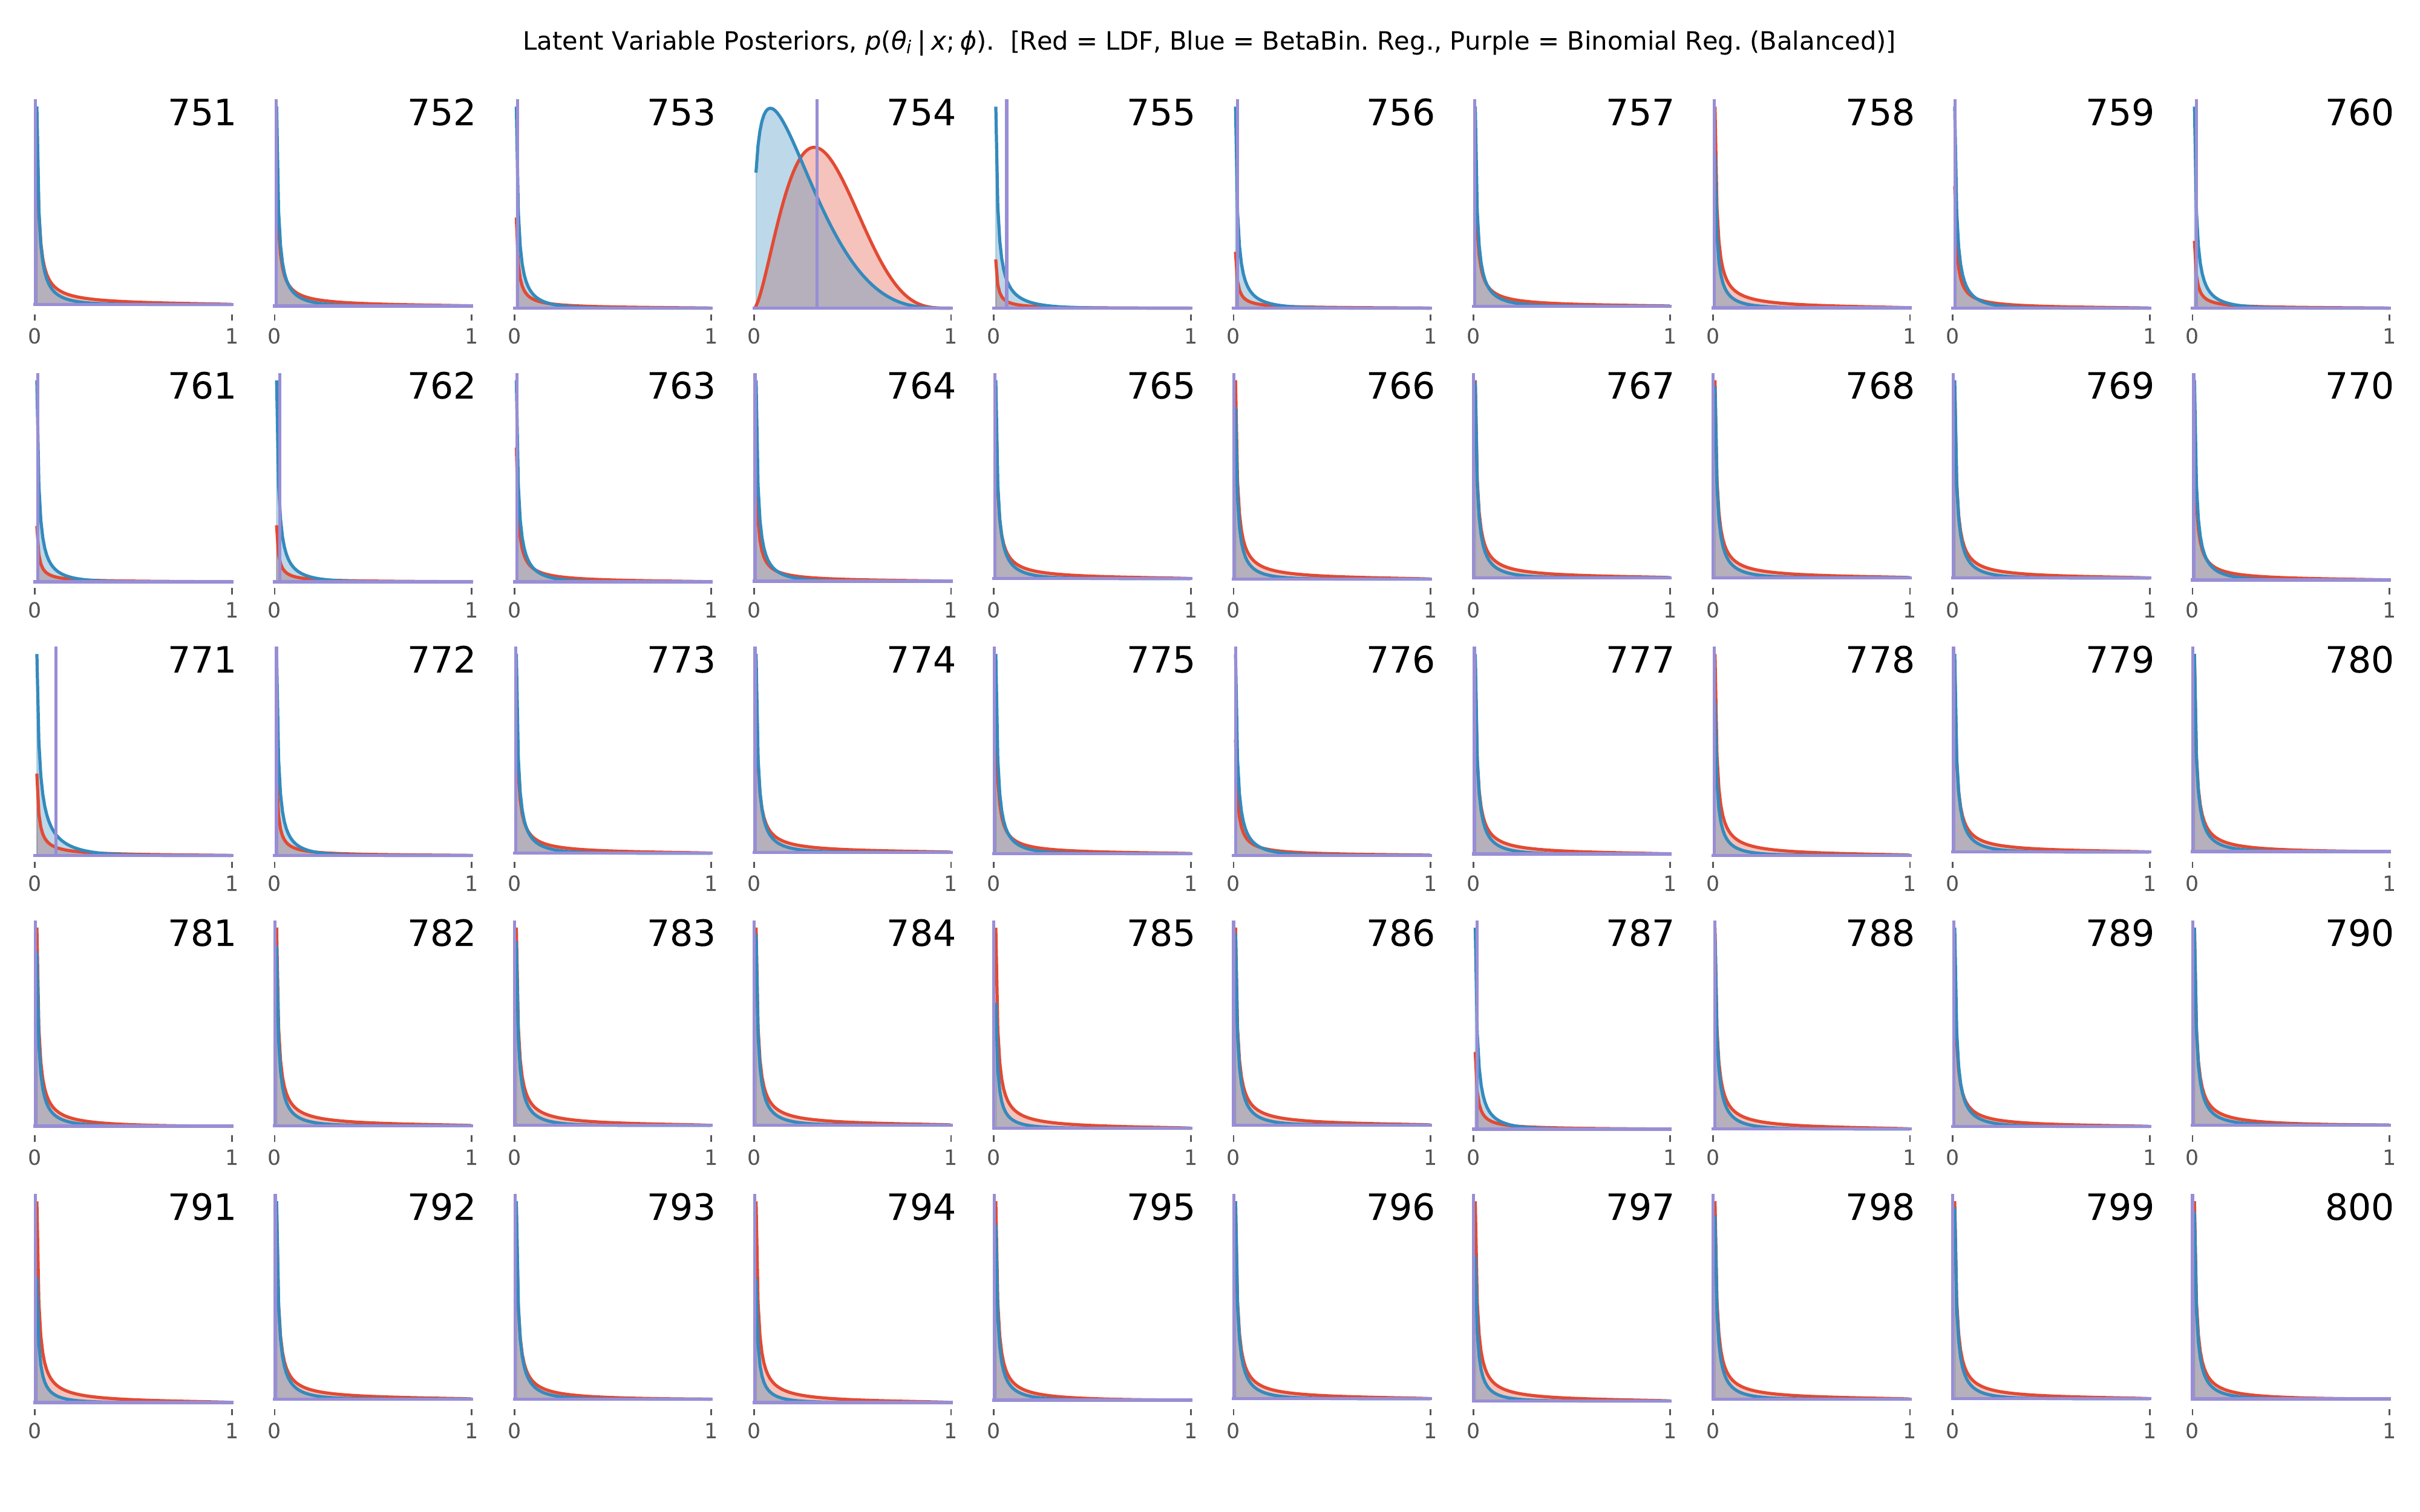}}
    \centerline{\includegraphics[width=0.75\linewidth, trim={0.375cm 1cm 0.375cm 1.5cm},clip]{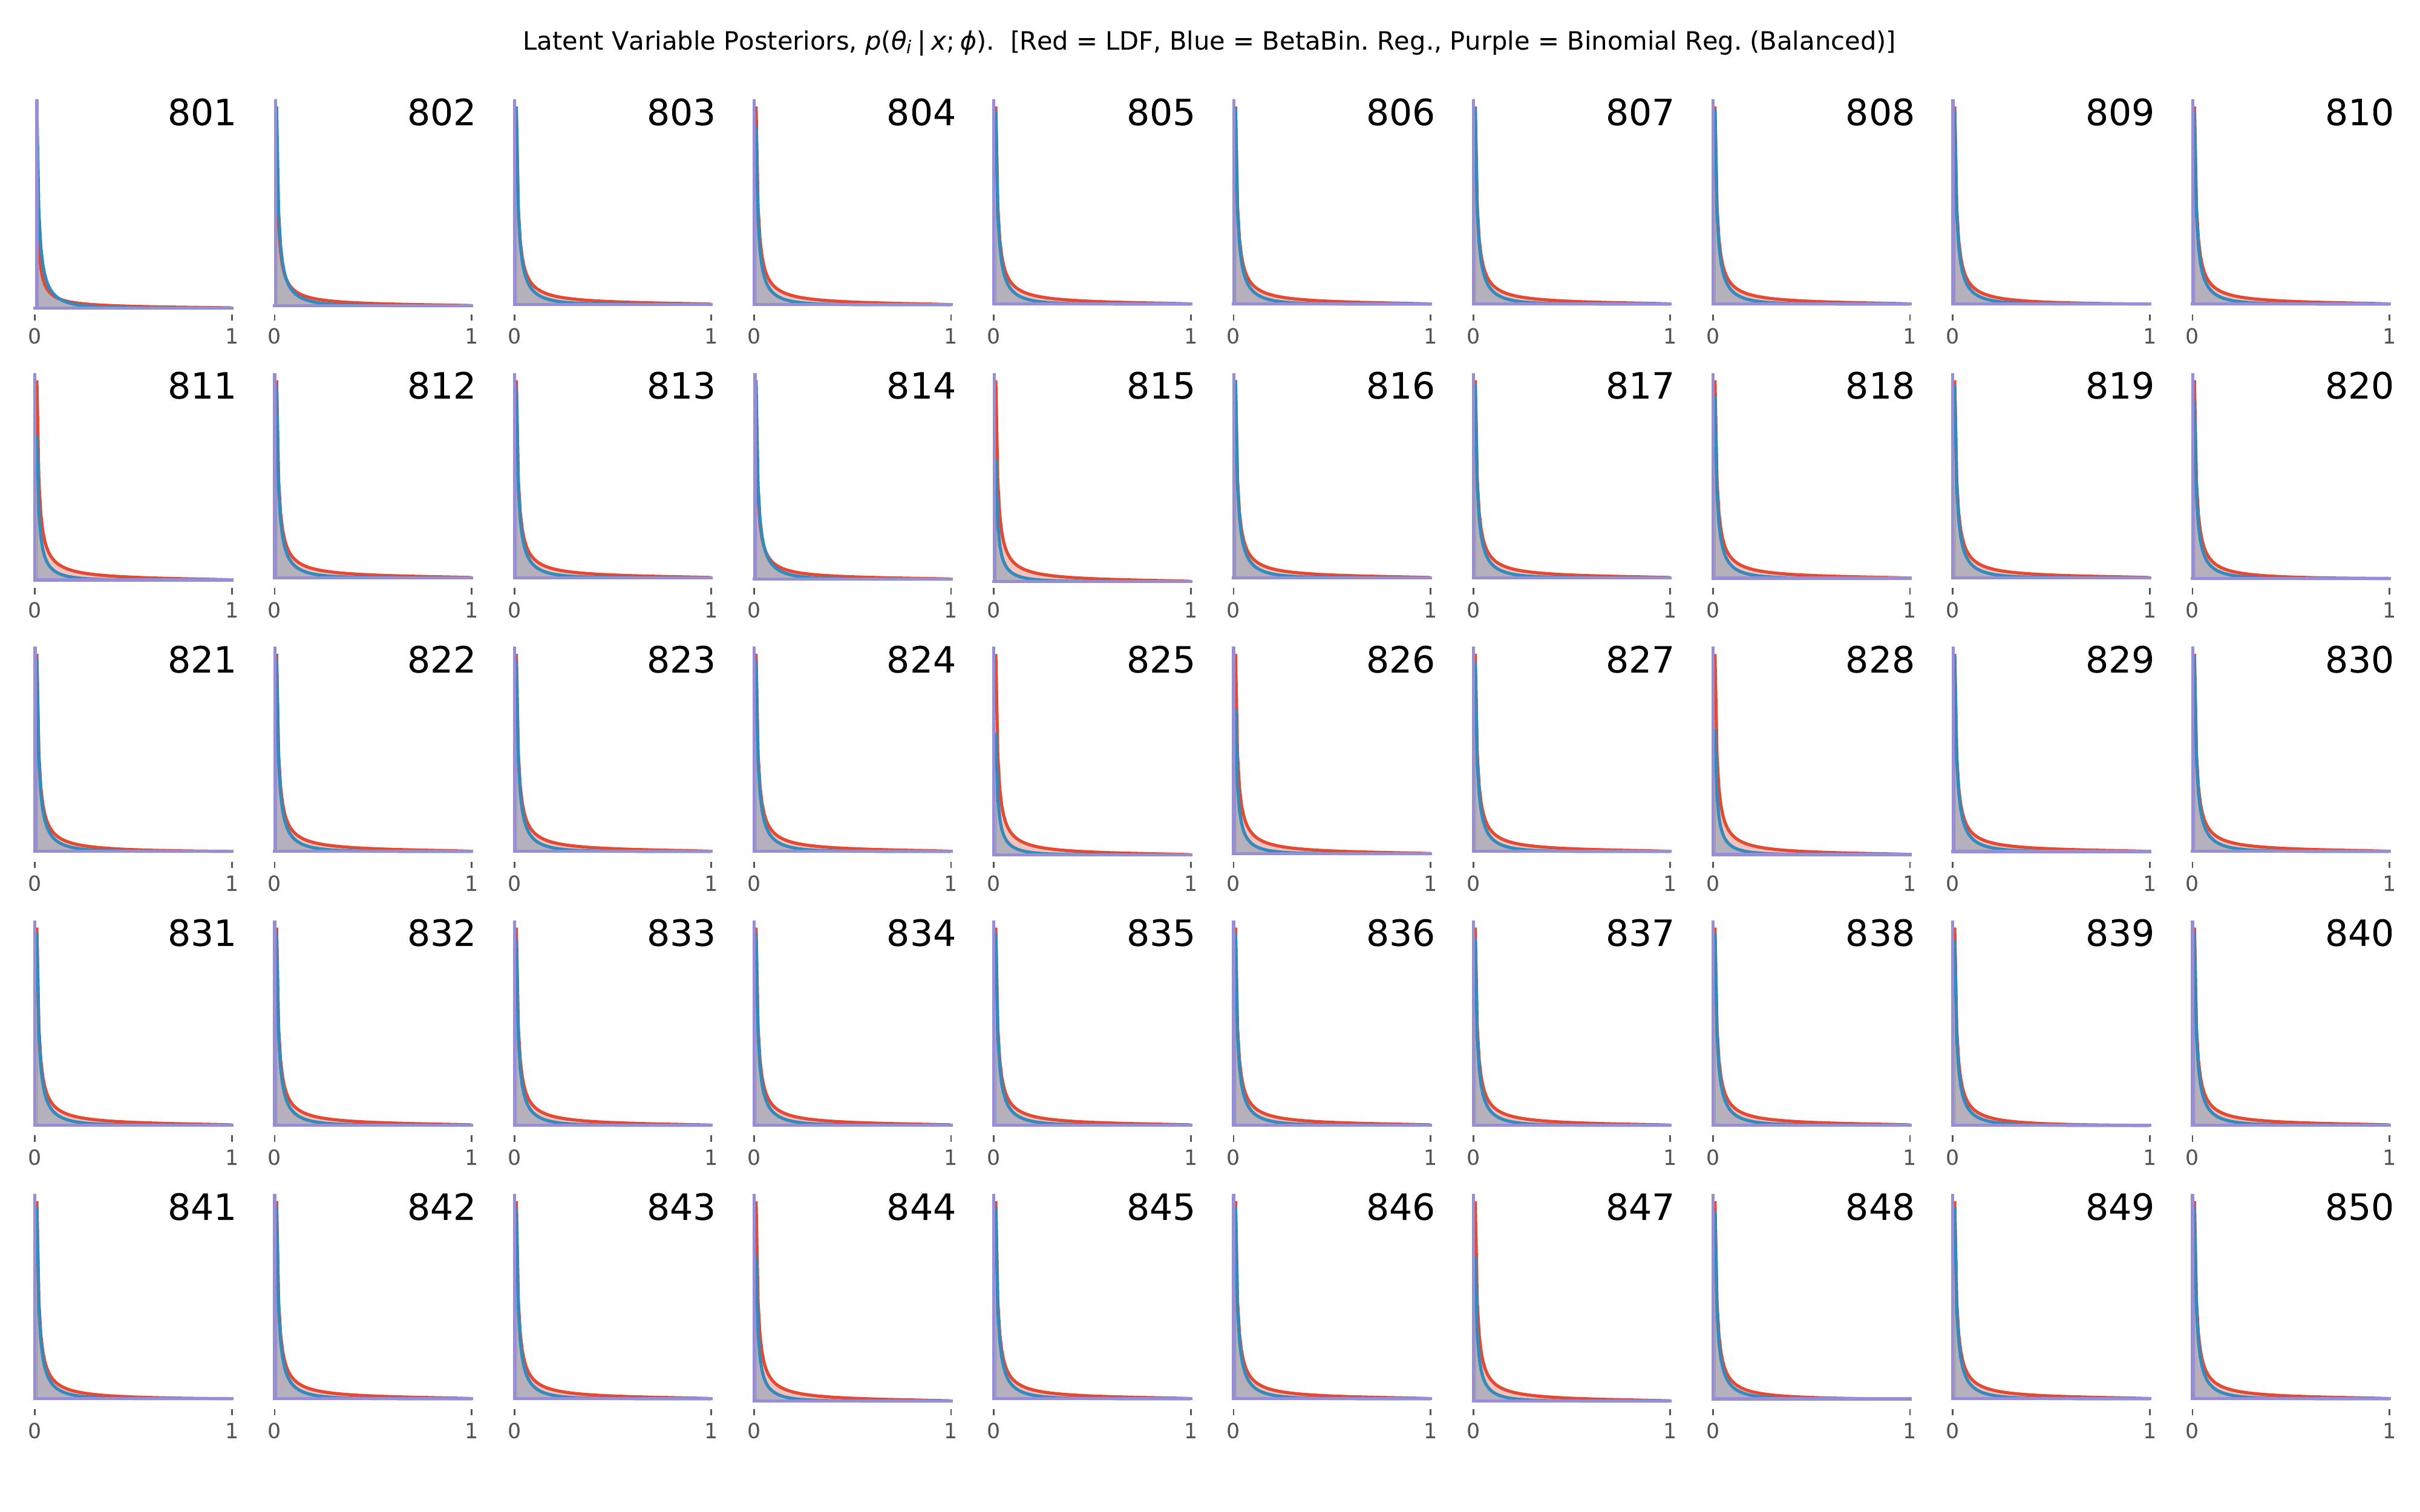}}
     \centerline{\includegraphics[width=0.75\linewidth, trim={0.375cm 19cm 0.375cm 1.5cm},clip]{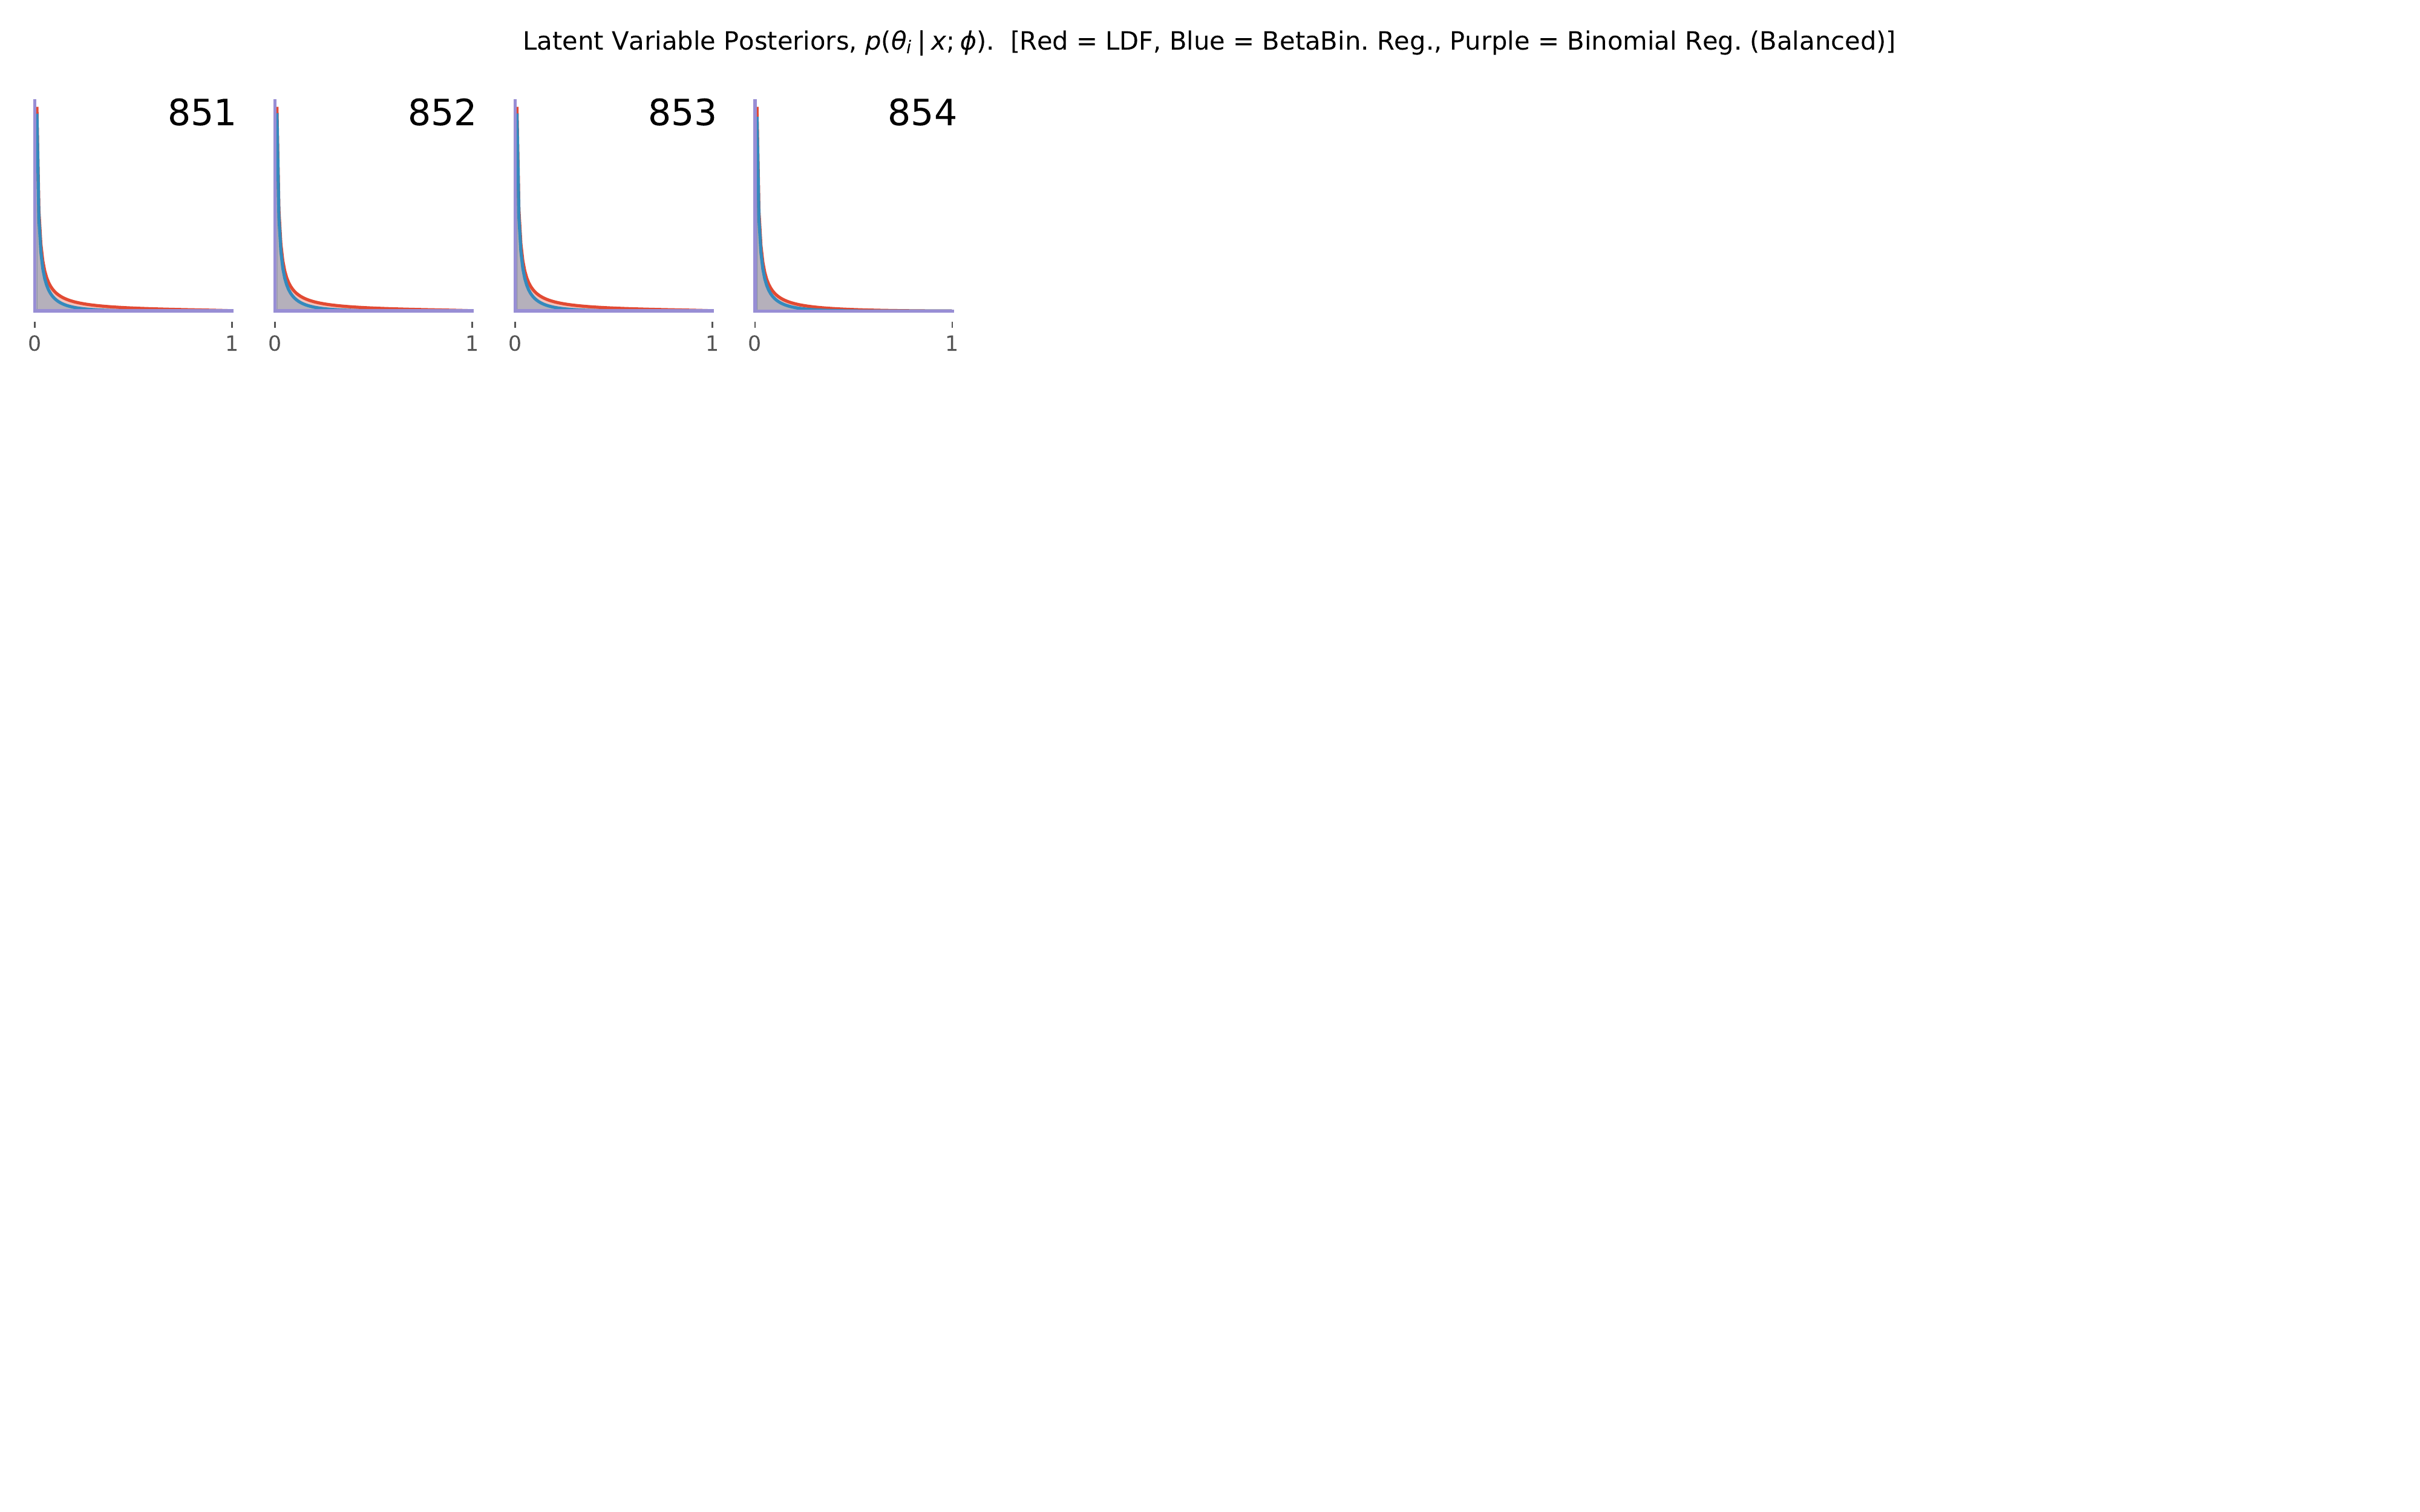}}
    \caption{\small \textbf{Latent variable posteriors (continued).}  A sample of the posteriors $p(\theta_i \given x; \phi)$ for the electrification application.  LDF is red, beta-binomial regression is blue, and binomial regression is purple.}
    \label{fig-supp-elec-aux-posterior-end}
  \end{center}
  \vspace*{-5mm}
\end{figure}

\subsubsection*{Posterior Predictive Distributions}

Here we provide the posterior predictive distributions for the primary data.  For each index, shown in the upper-right corner, the distributions are predicted by models that are \textit{not} trained on data from that index.
The posterior predictive distributions
\begin{align}
p(y_i \given x; \phi) = \int p(y_i \given \theta_i) p(\theta_i \given x; \phi) \dif\theta_i
\end{align}
are presented in Figs.~\ref{fig-supp-elec-predictive-start} thru \ref{fig-supp-elec-predictive-end}.  In each, the LDF predictive (red) and beta-binomial regression posterior predictive (blue) are beta-binomial distributions; the binomial regression posterior predictive is binomially-distributed.  The observed data is shown by the black vertical line.

\begin{figure}[t]
  \vskip 0.1in
  \begin{center}
    \centerline{\includegraphics[width=0.75\linewidth, trim={0.375cm 1cm 0.375cm 1.5cm},clip]{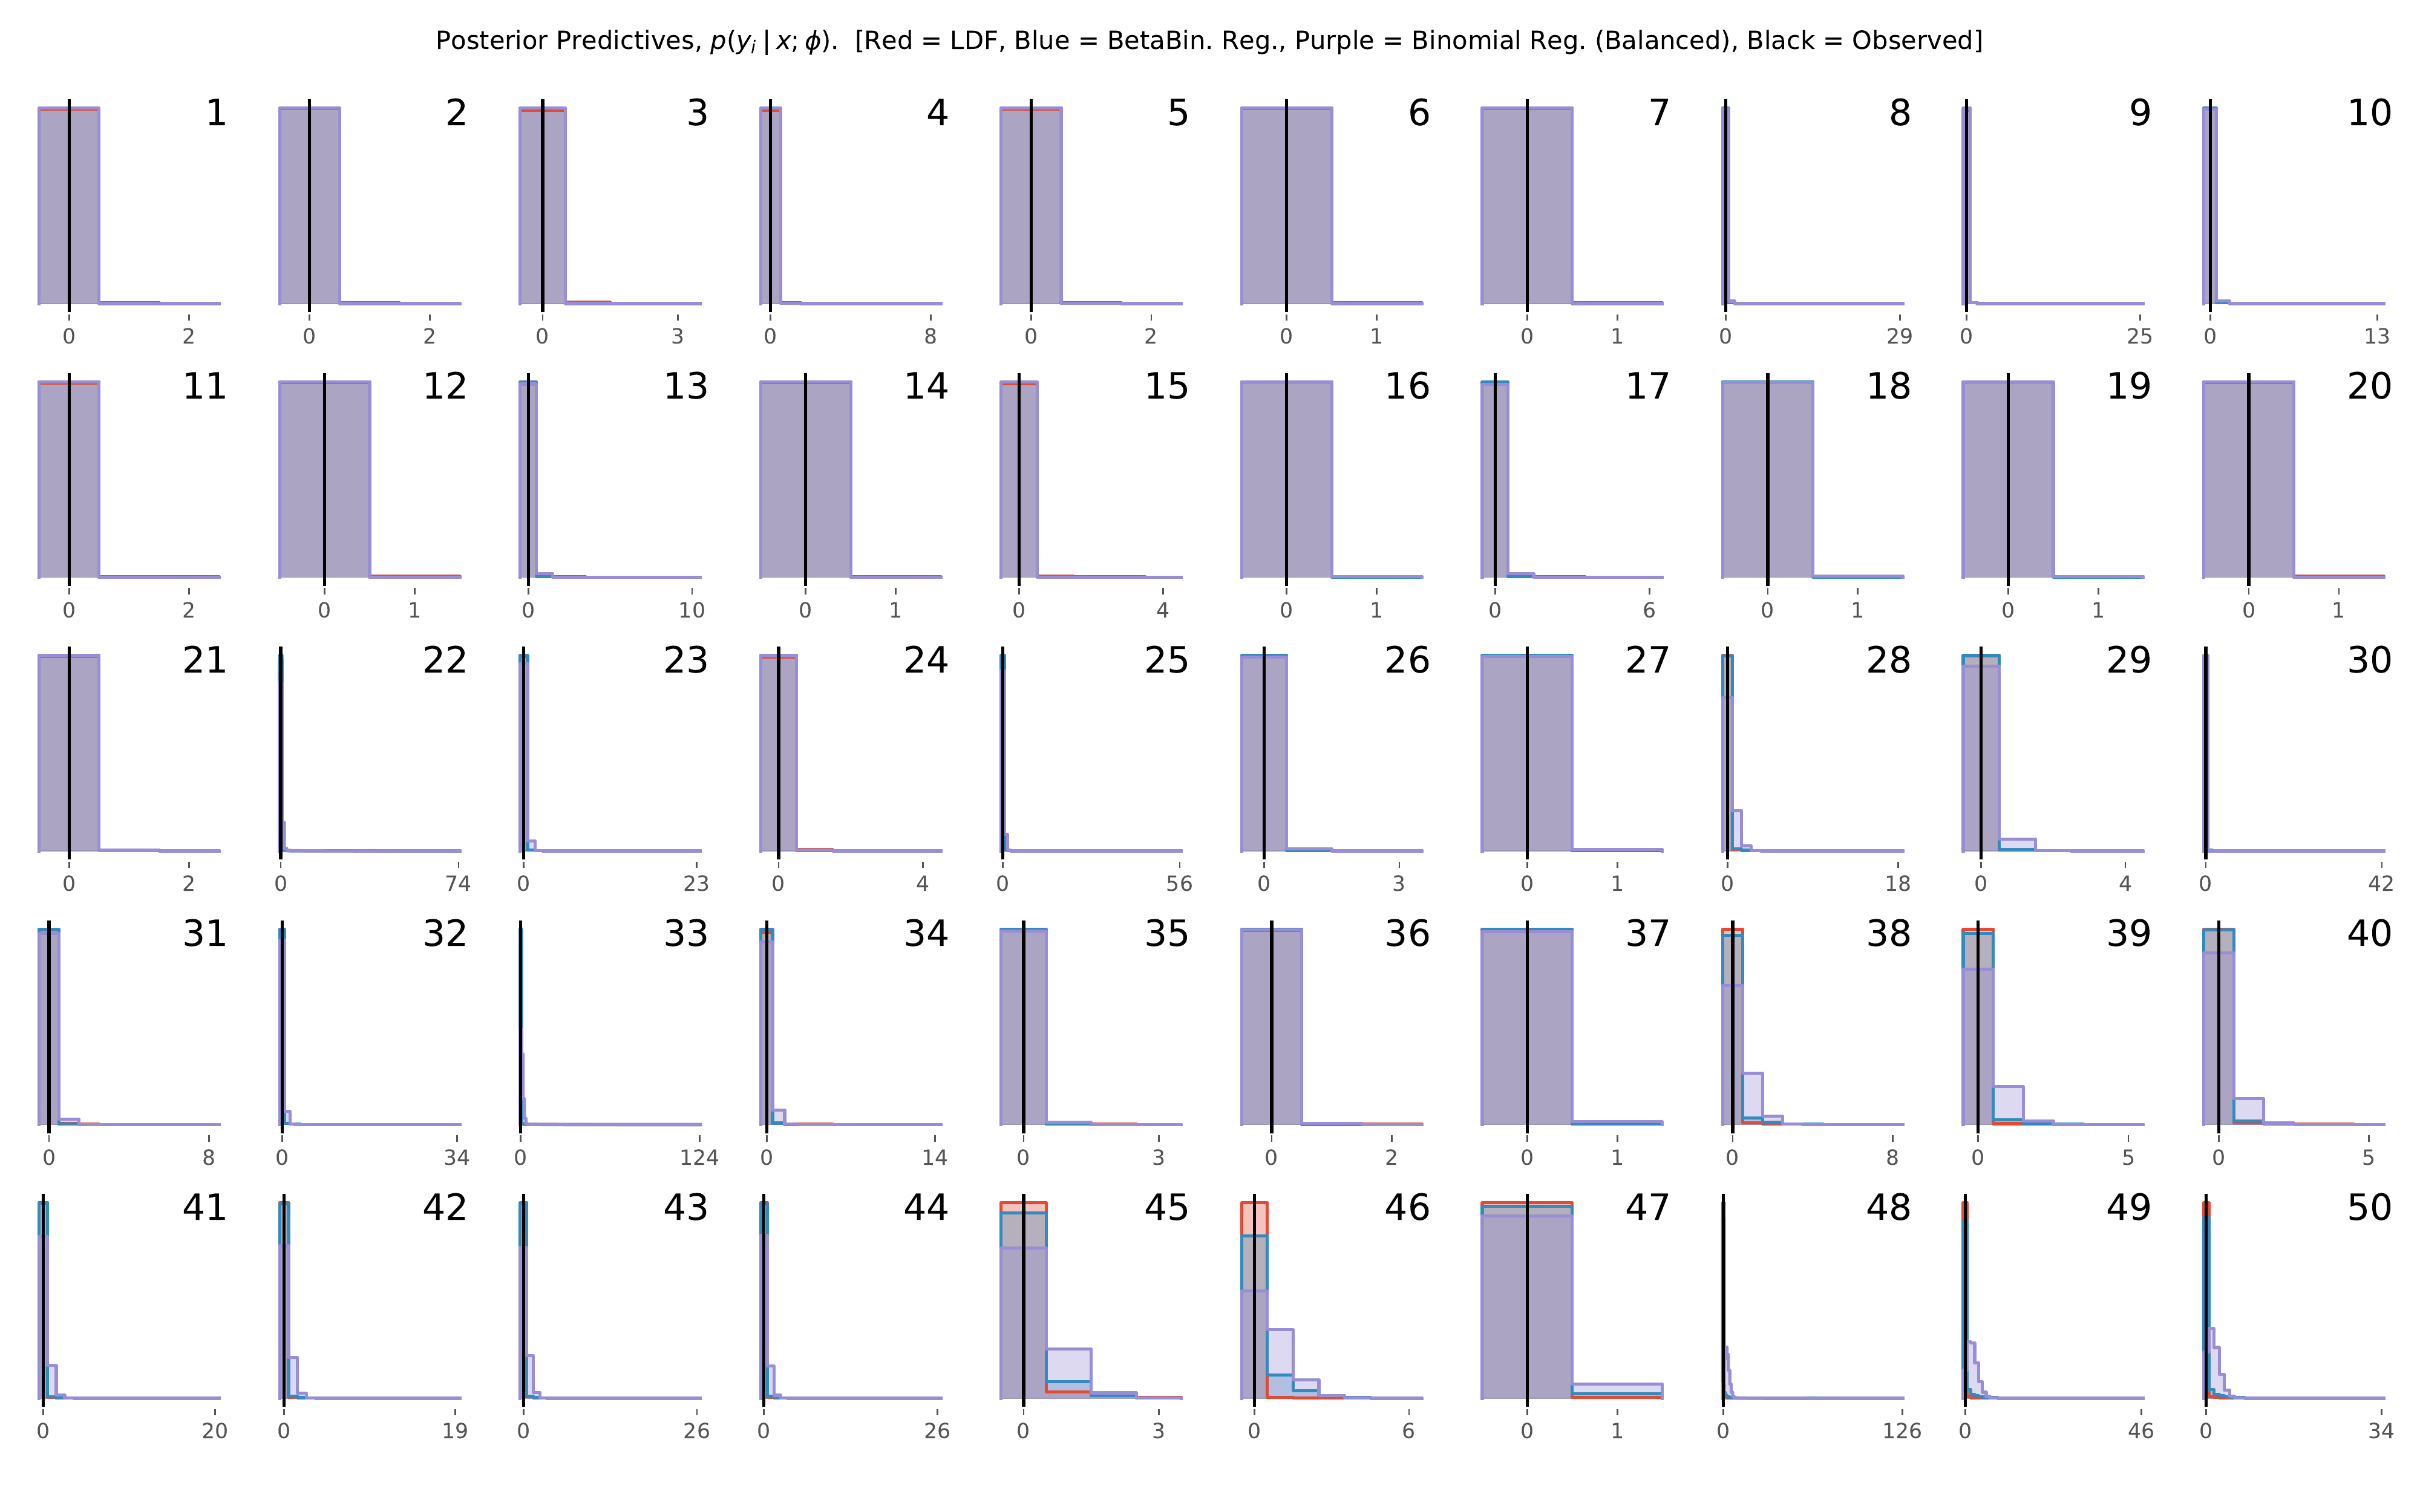}}
    \centerline{\includegraphics[width=0.75\linewidth, trim={0.375cm 1cm 0.375cm 1.5cm},clip]{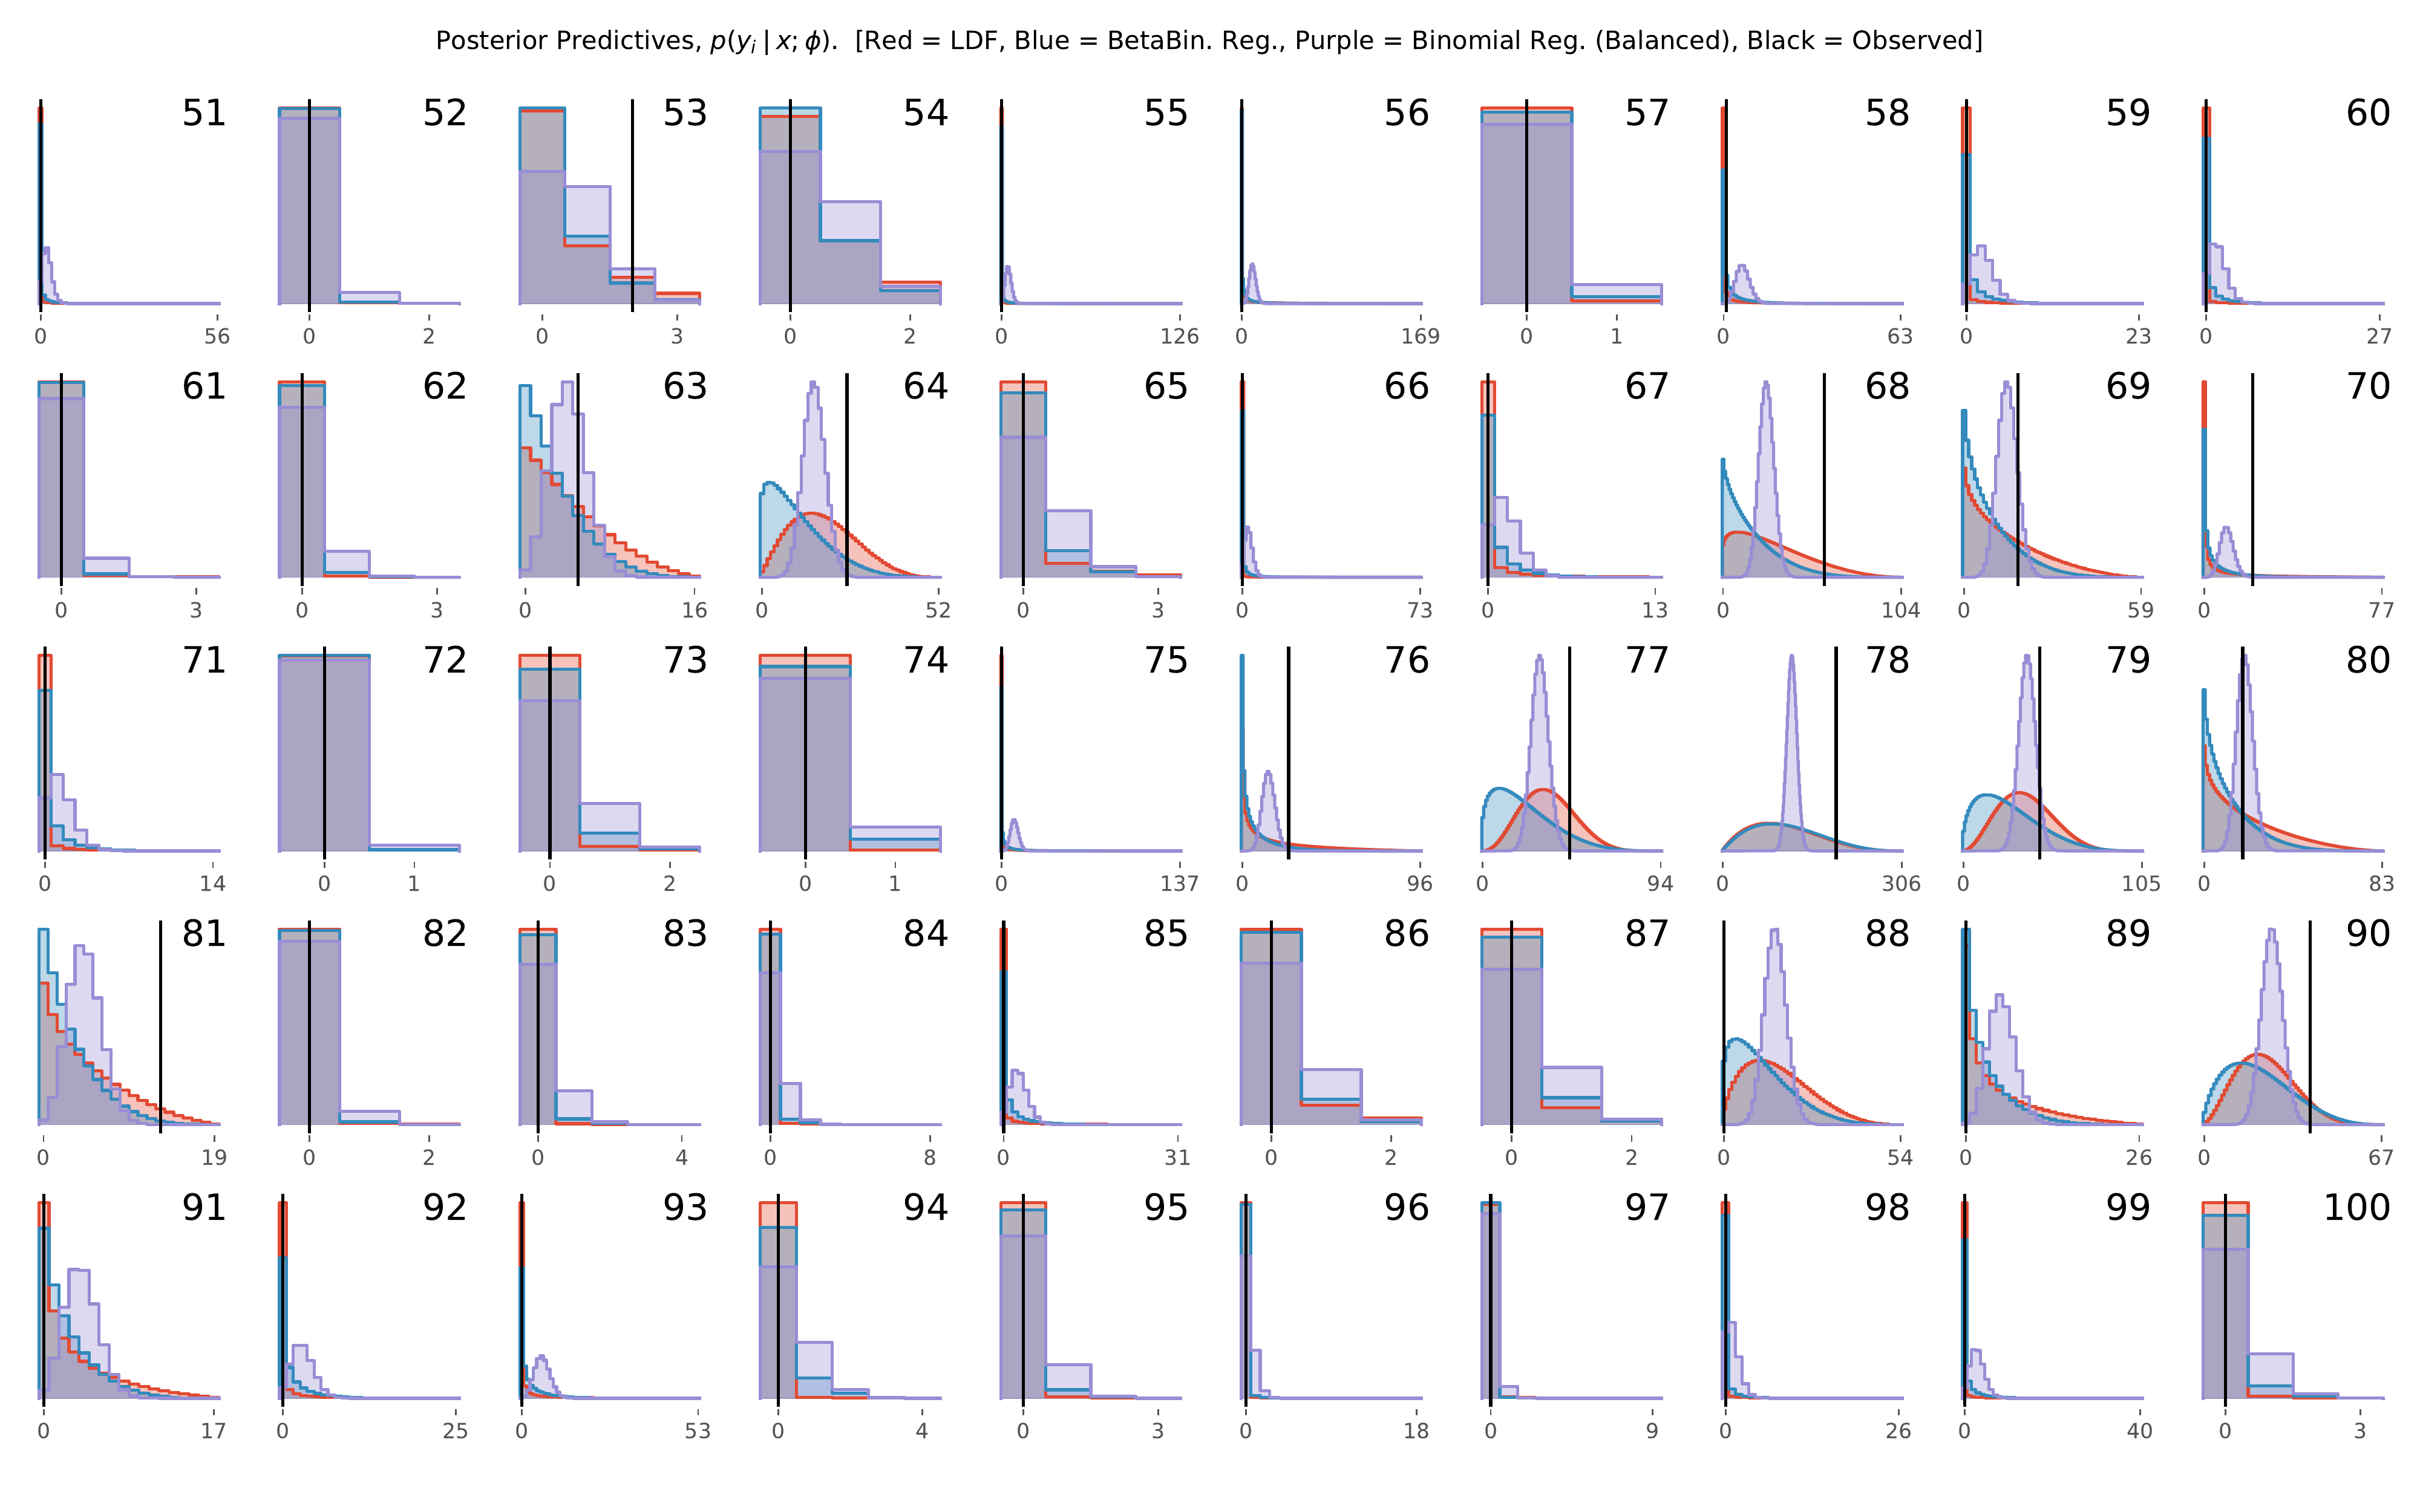}}
     \centerline{\includegraphics[width=0.75\linewidth, trim={0.375cm 1cm 0.375cm 1.5cm},clip]{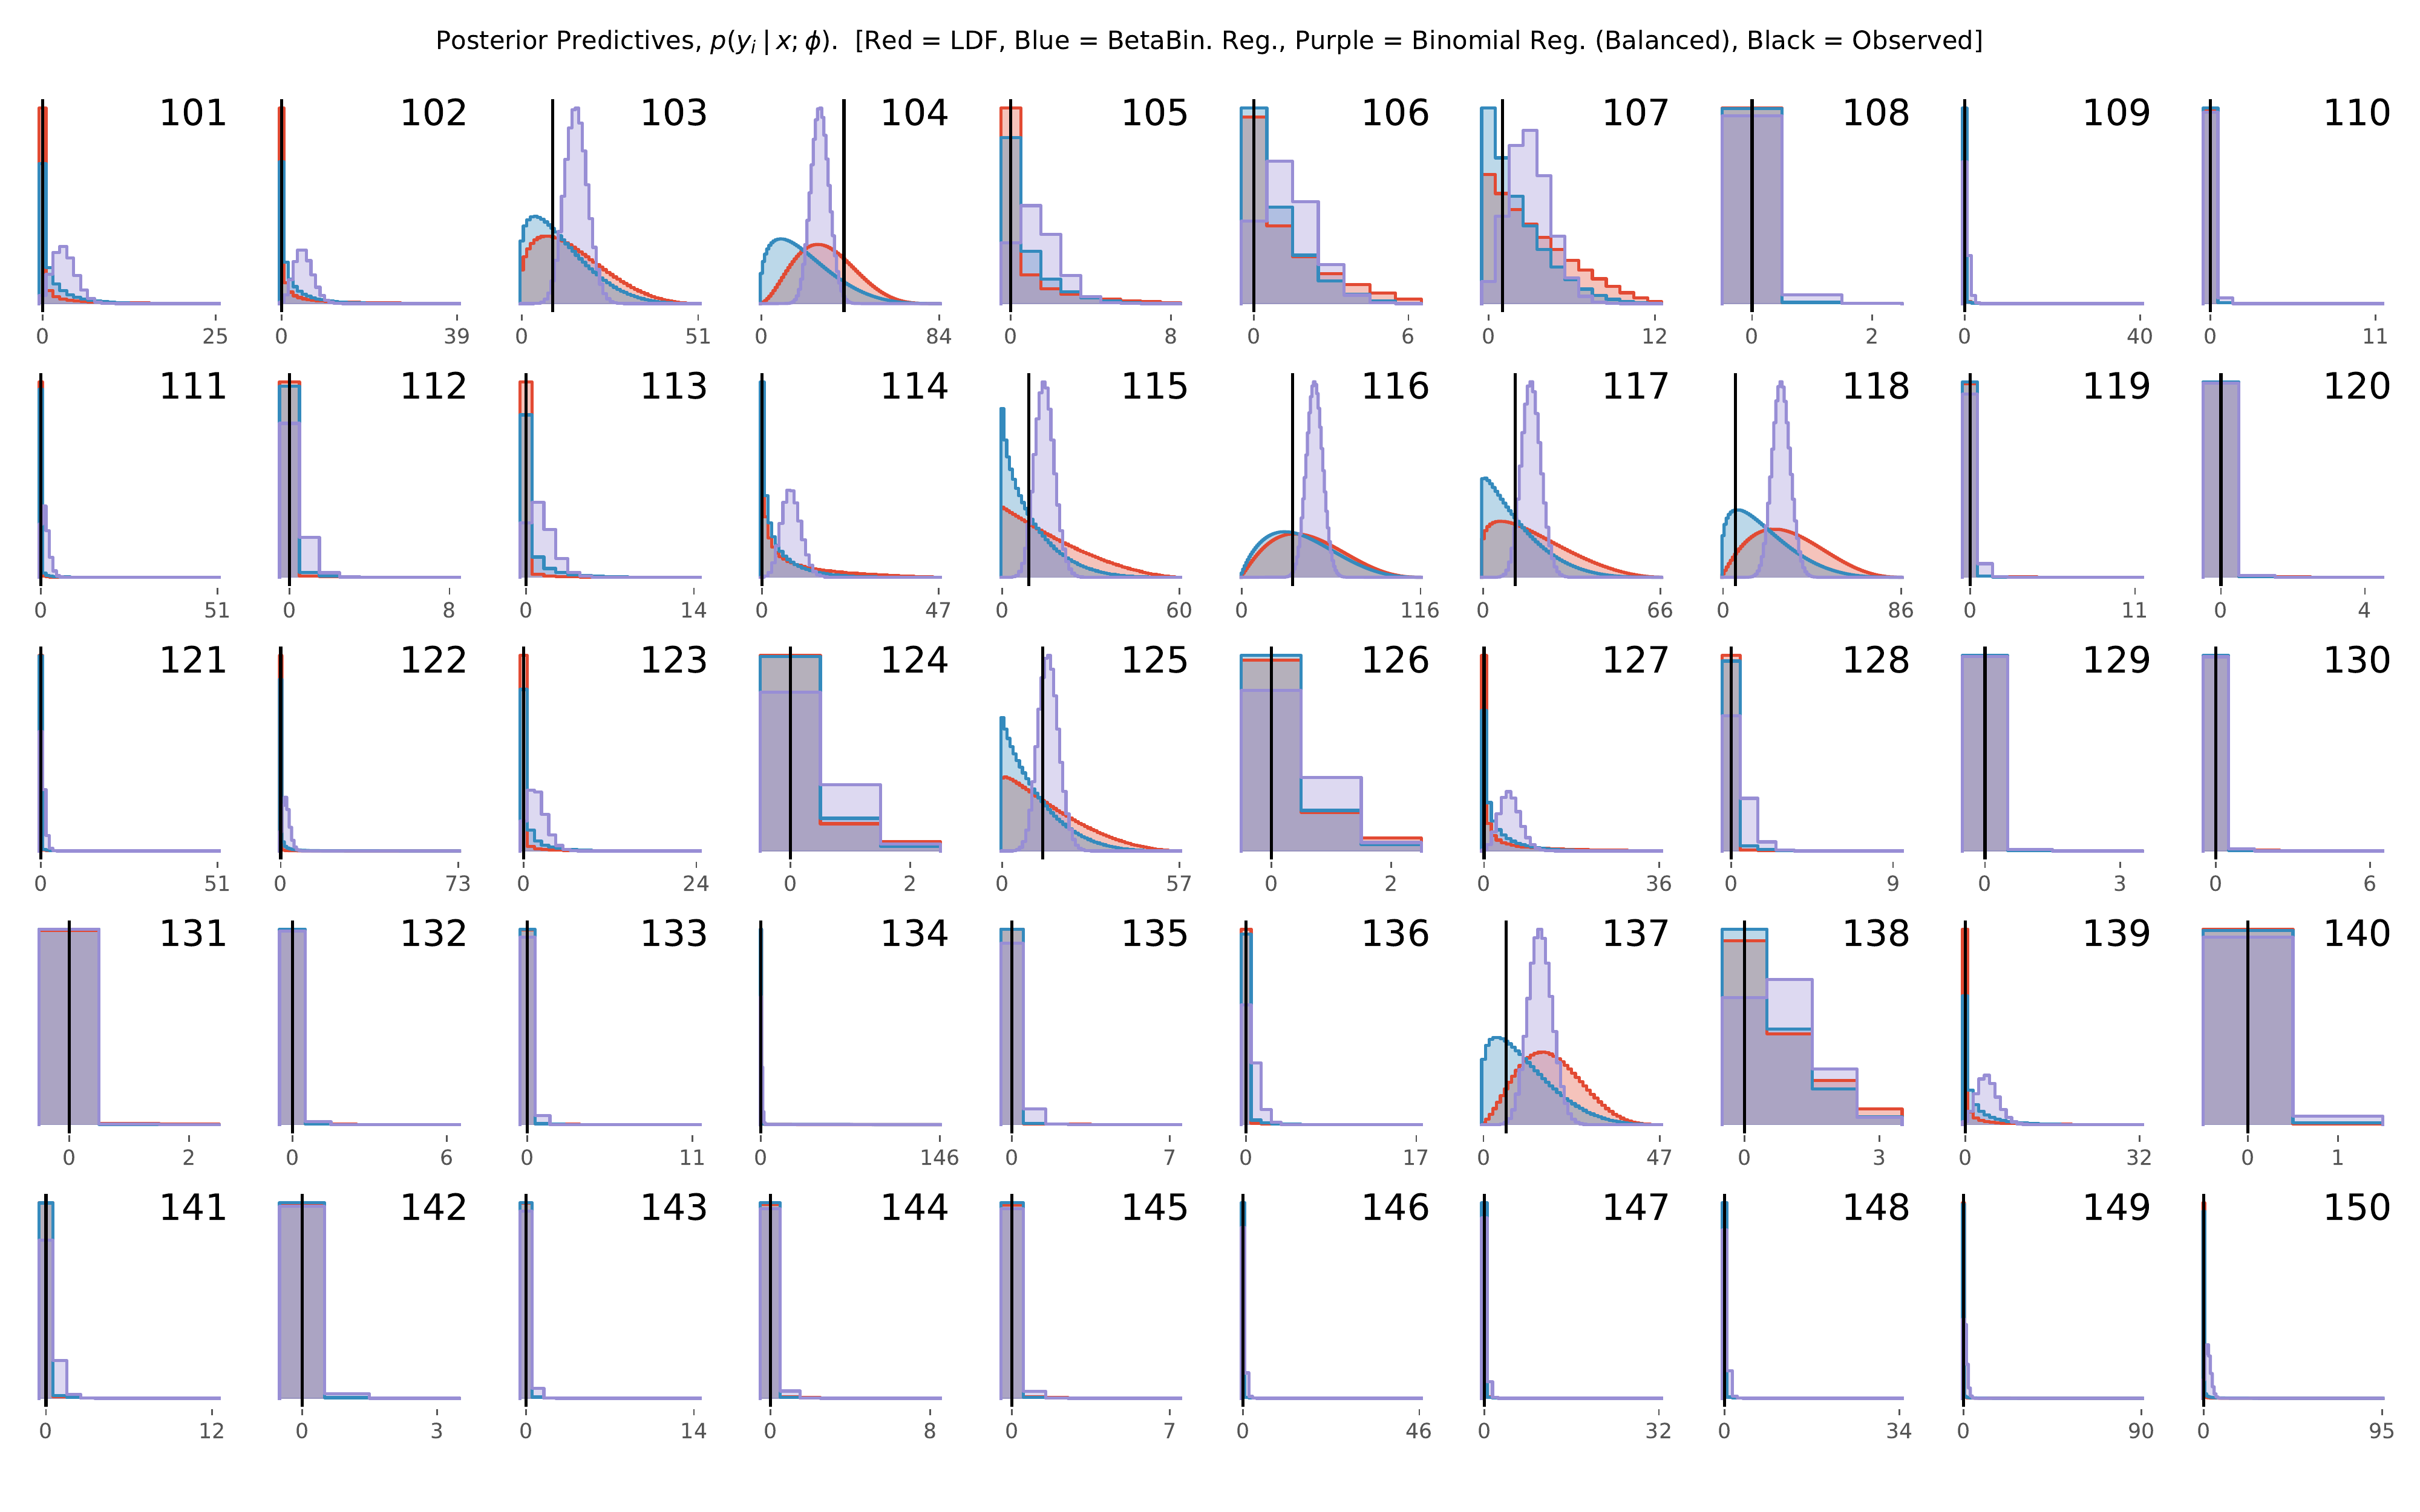}}
    \caption{\small \textbf{Primary data posterior predictives.}  A subset of the predictive likelihoods $p(y_i \given x; \phi)$ for the electrification application.  LDF is red, beta-binomial regression is blue, binomial regression is purple, and the observed value is black.}
    \label{fig-supp-elec-predictive-start}
  \end{center}
  \vspace*{-5mm}
\end{figure}

\begin{figure}[t]
  \vskip 0.1in
  \begin{center}
    \centerline{\includegraphics[width=0.75\linewidth, trim={0.375cm 1cm 0.375cm 1.5cm},clip]{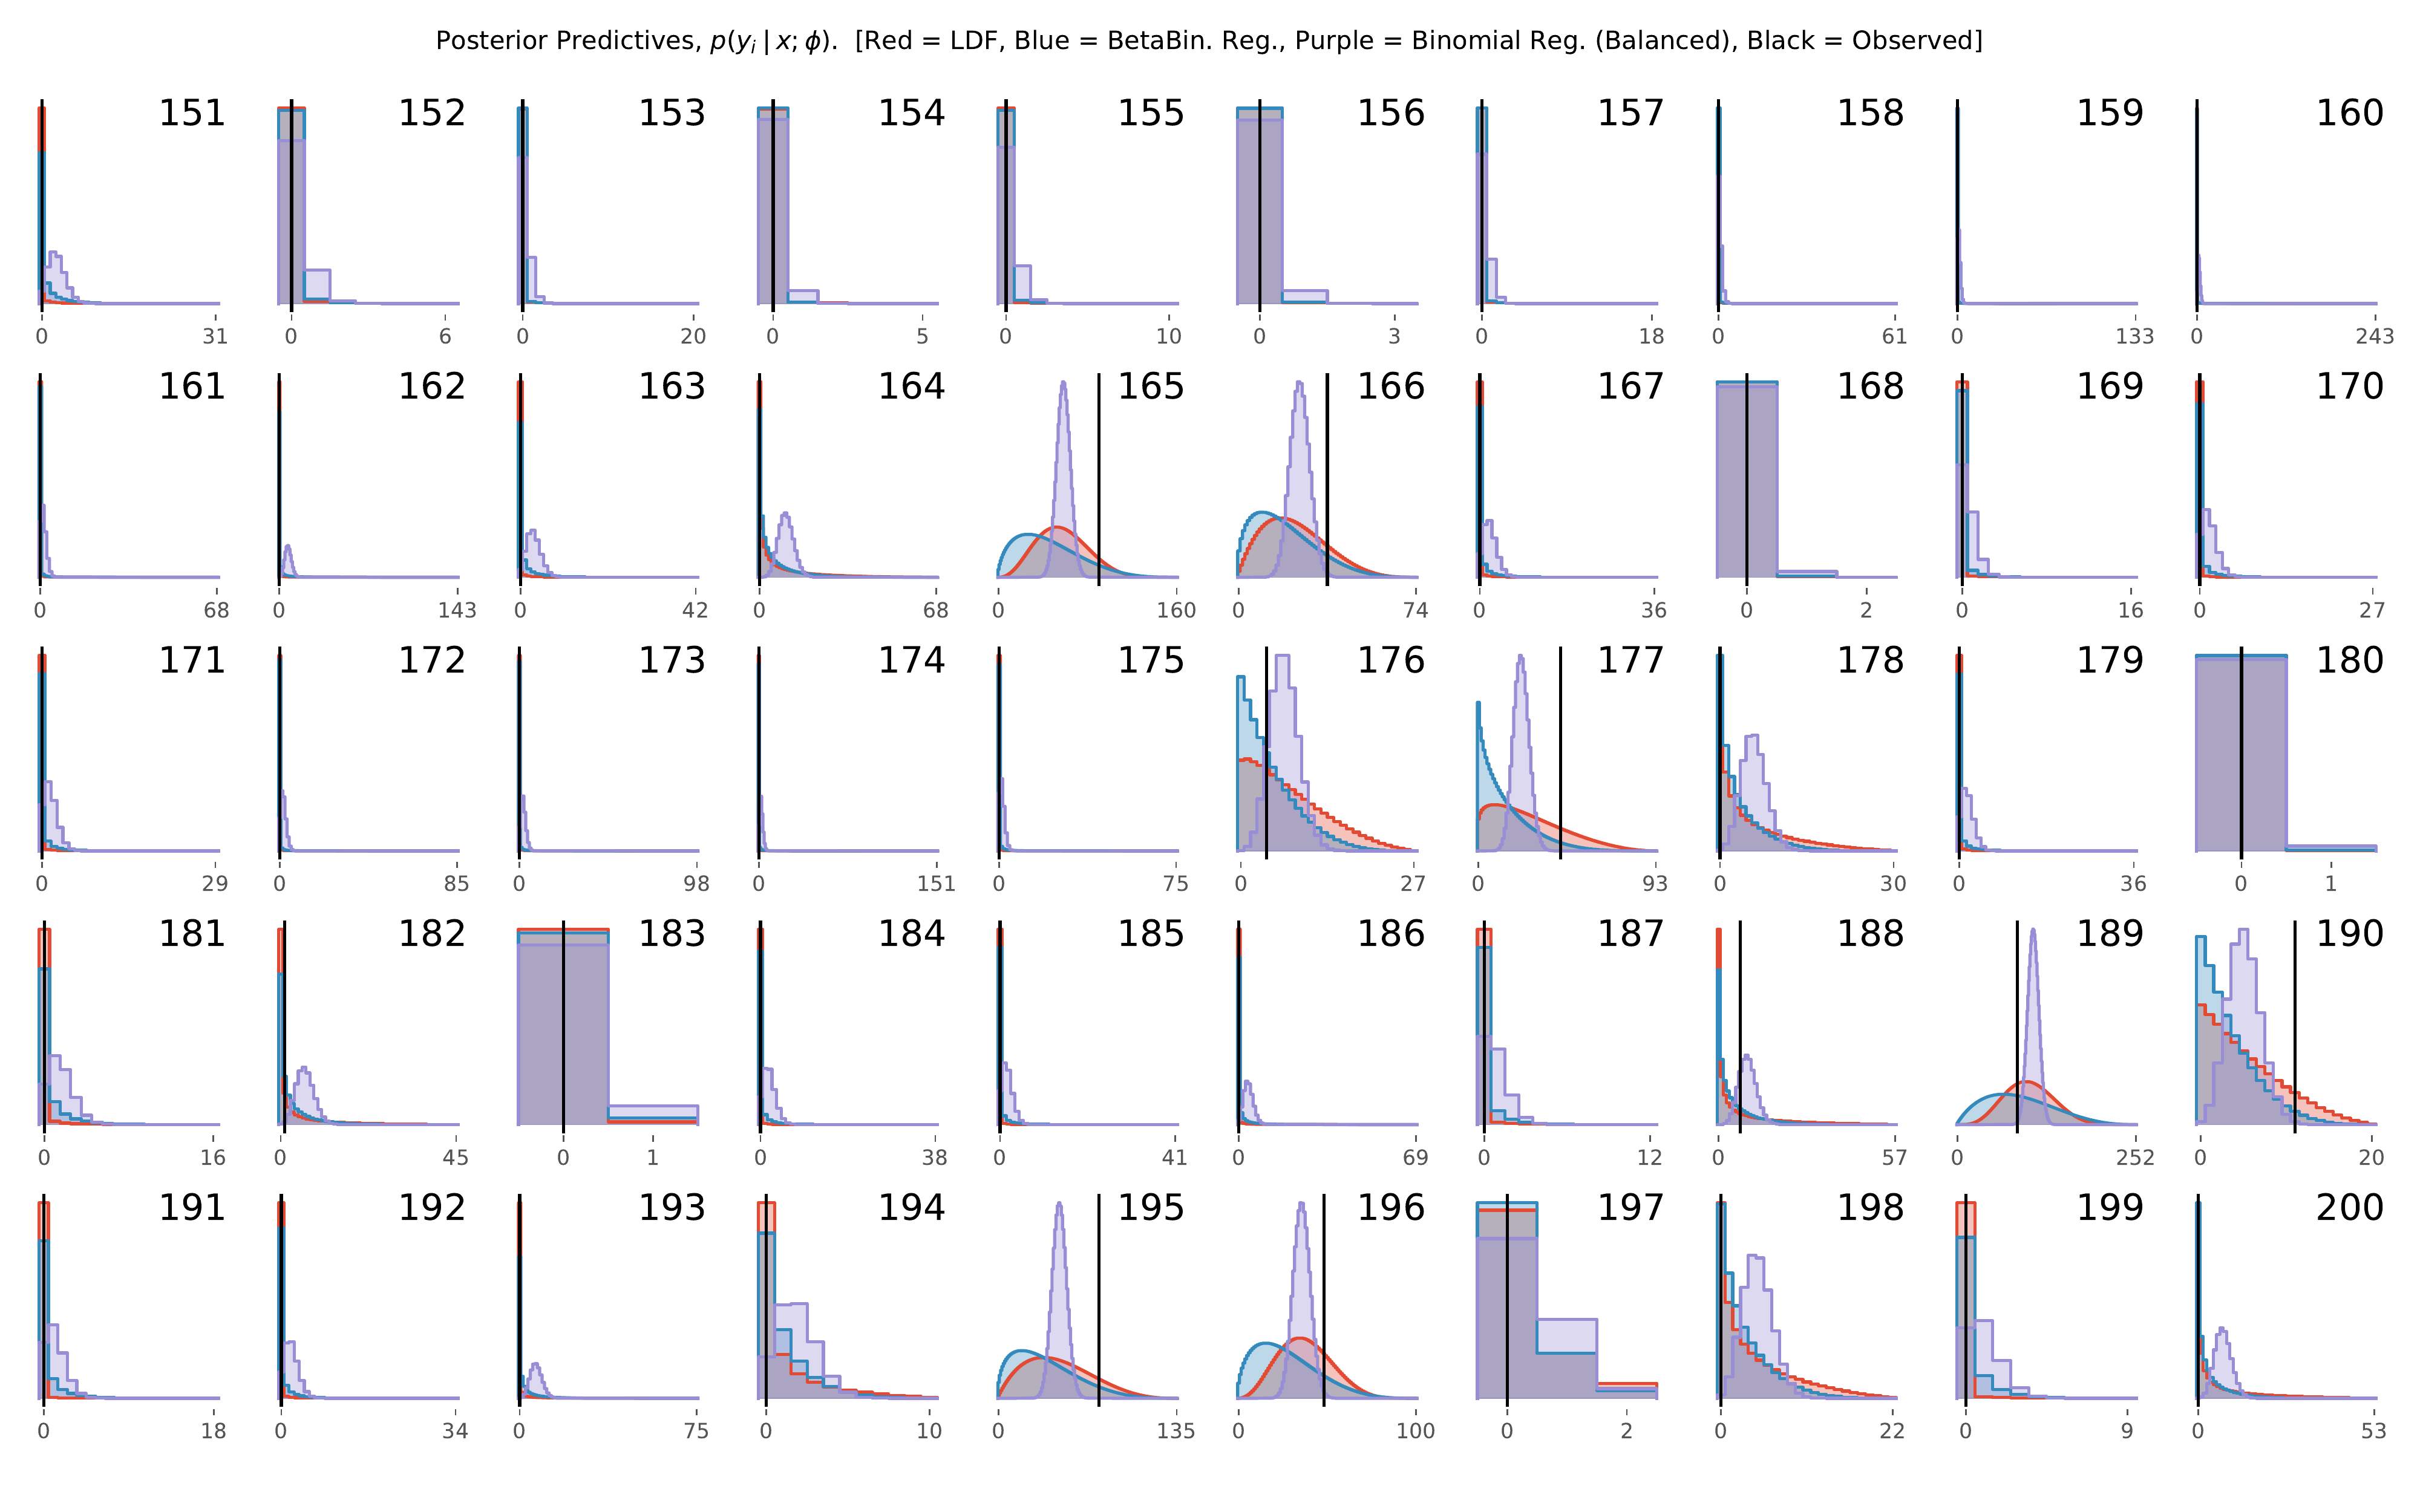}}
    \centerline{\includegraphics[width=0.75\linewidth, trim={0.375cm 1cm 0.375cm 1.5cm},clip]{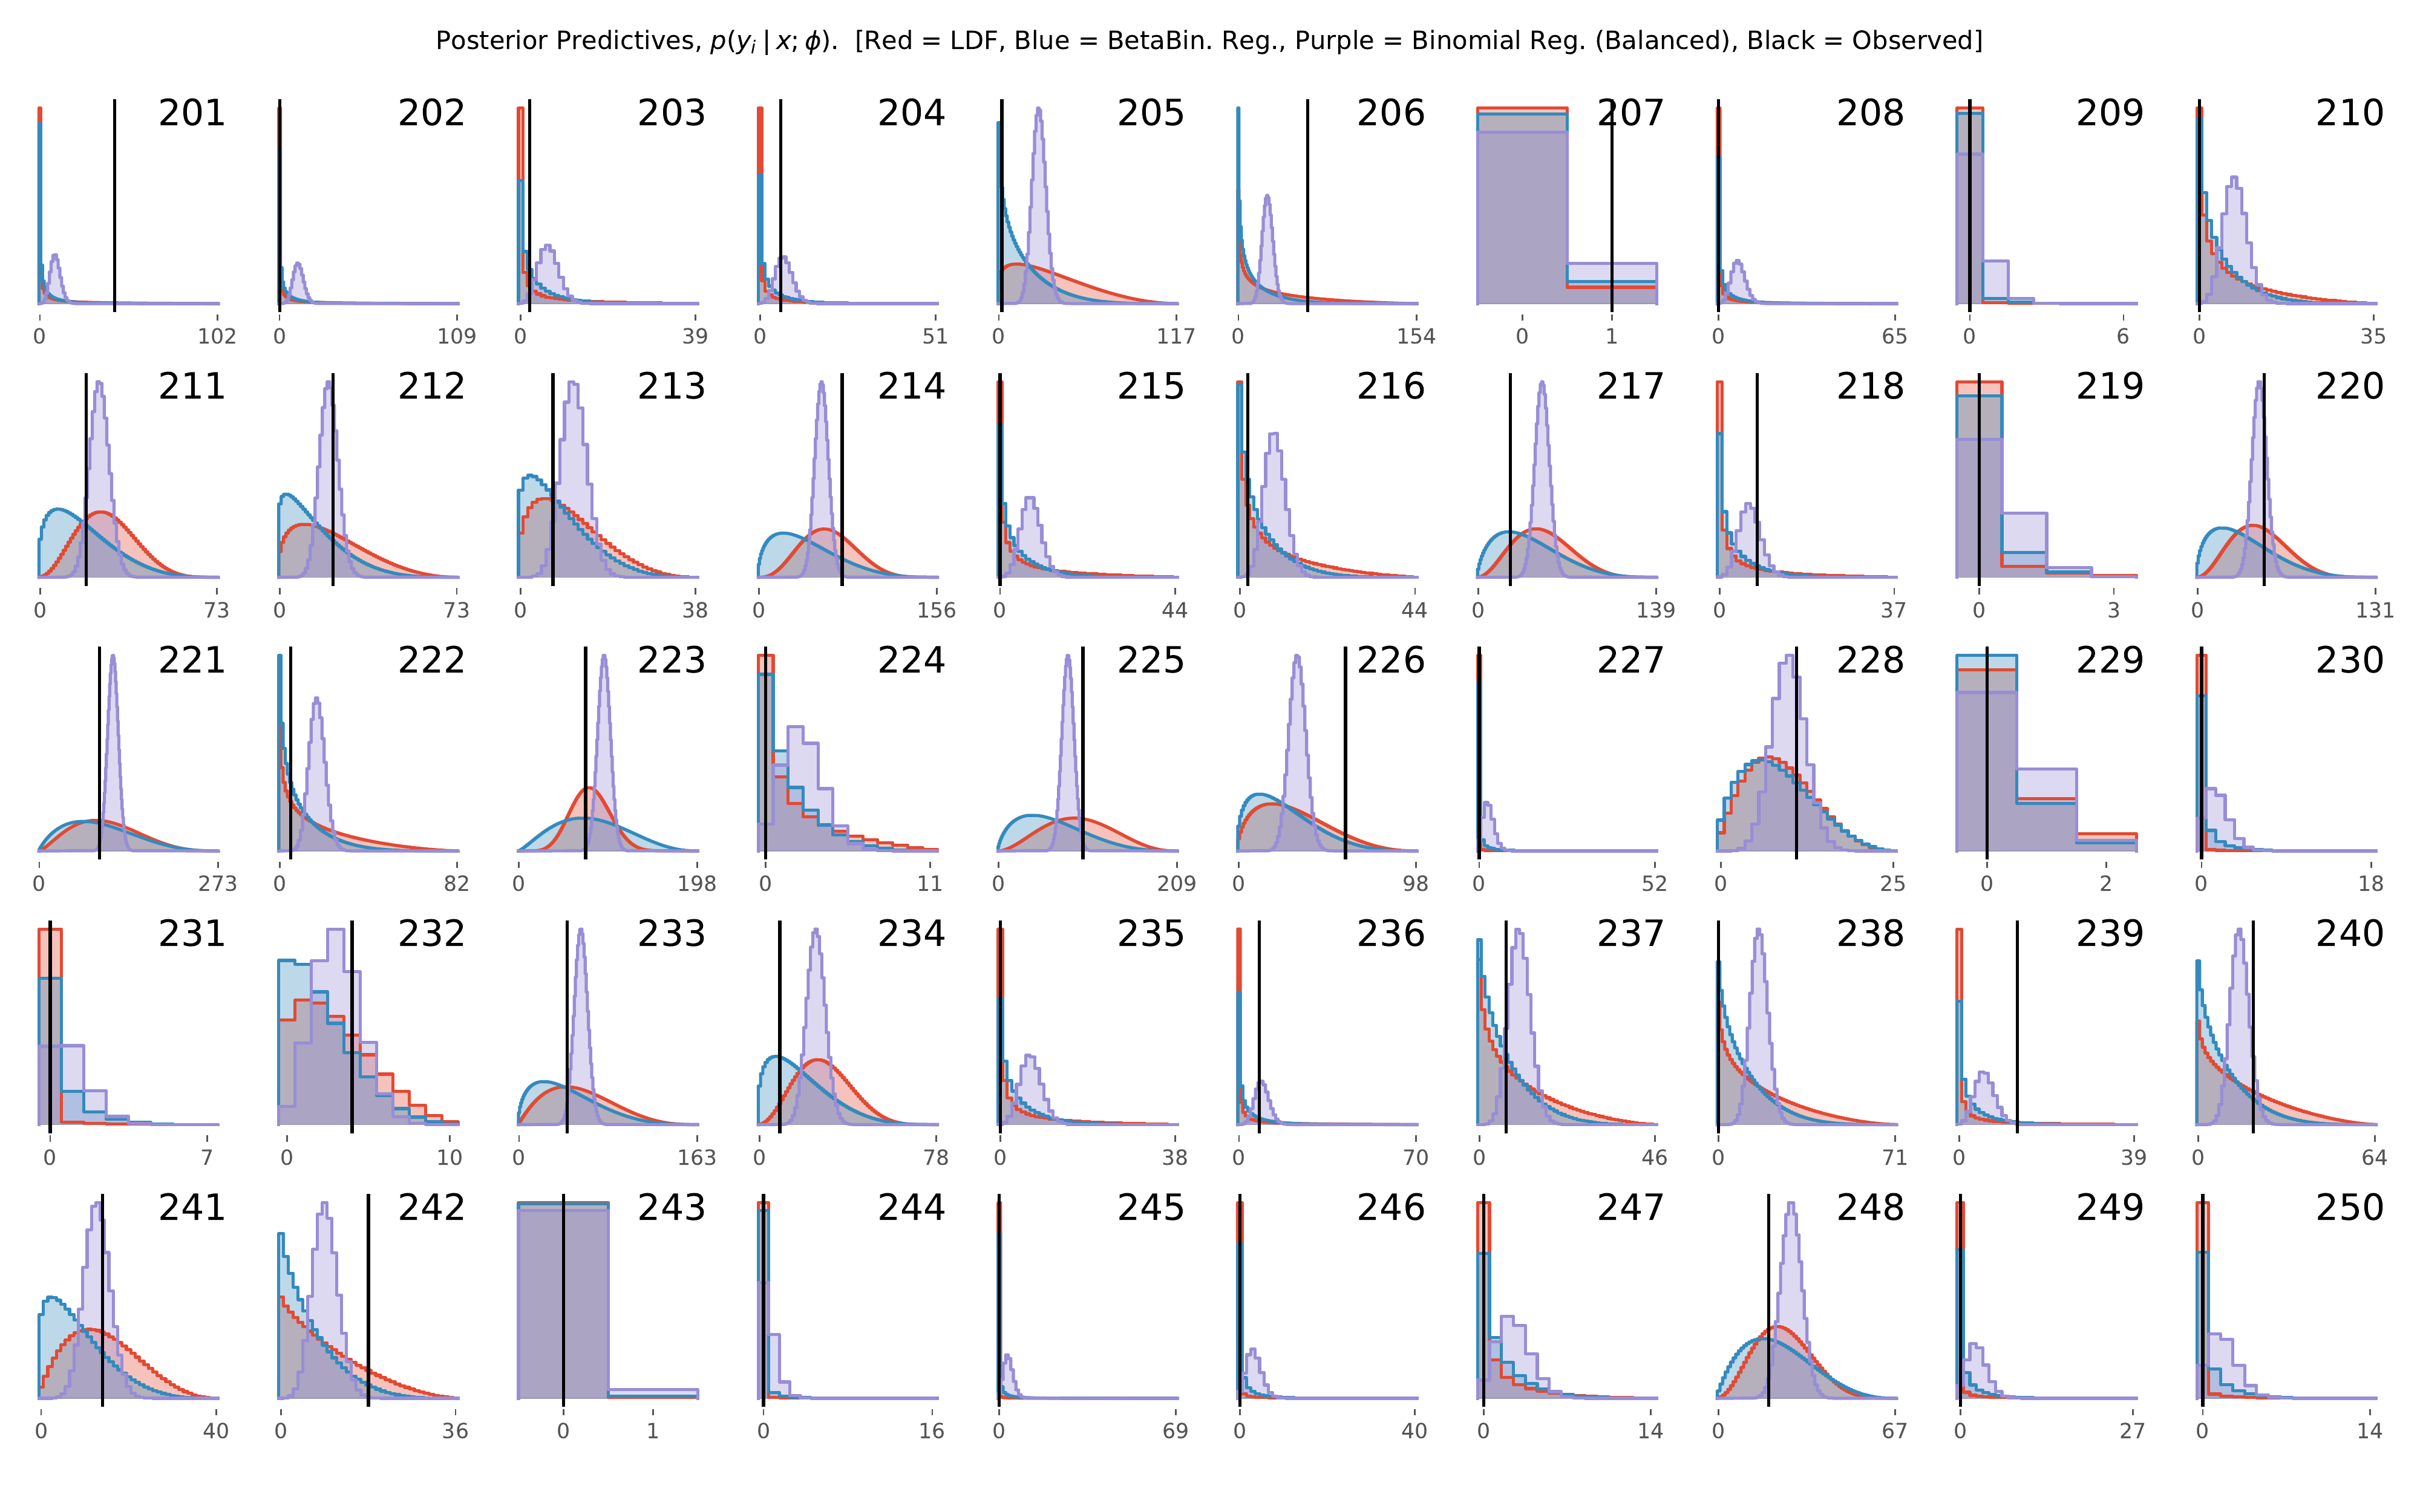}}
     \centerline{\includegraphics[width=0.75\linewidth, trim={0.375cm 1cm 0.375cm 1.5cm},clip]{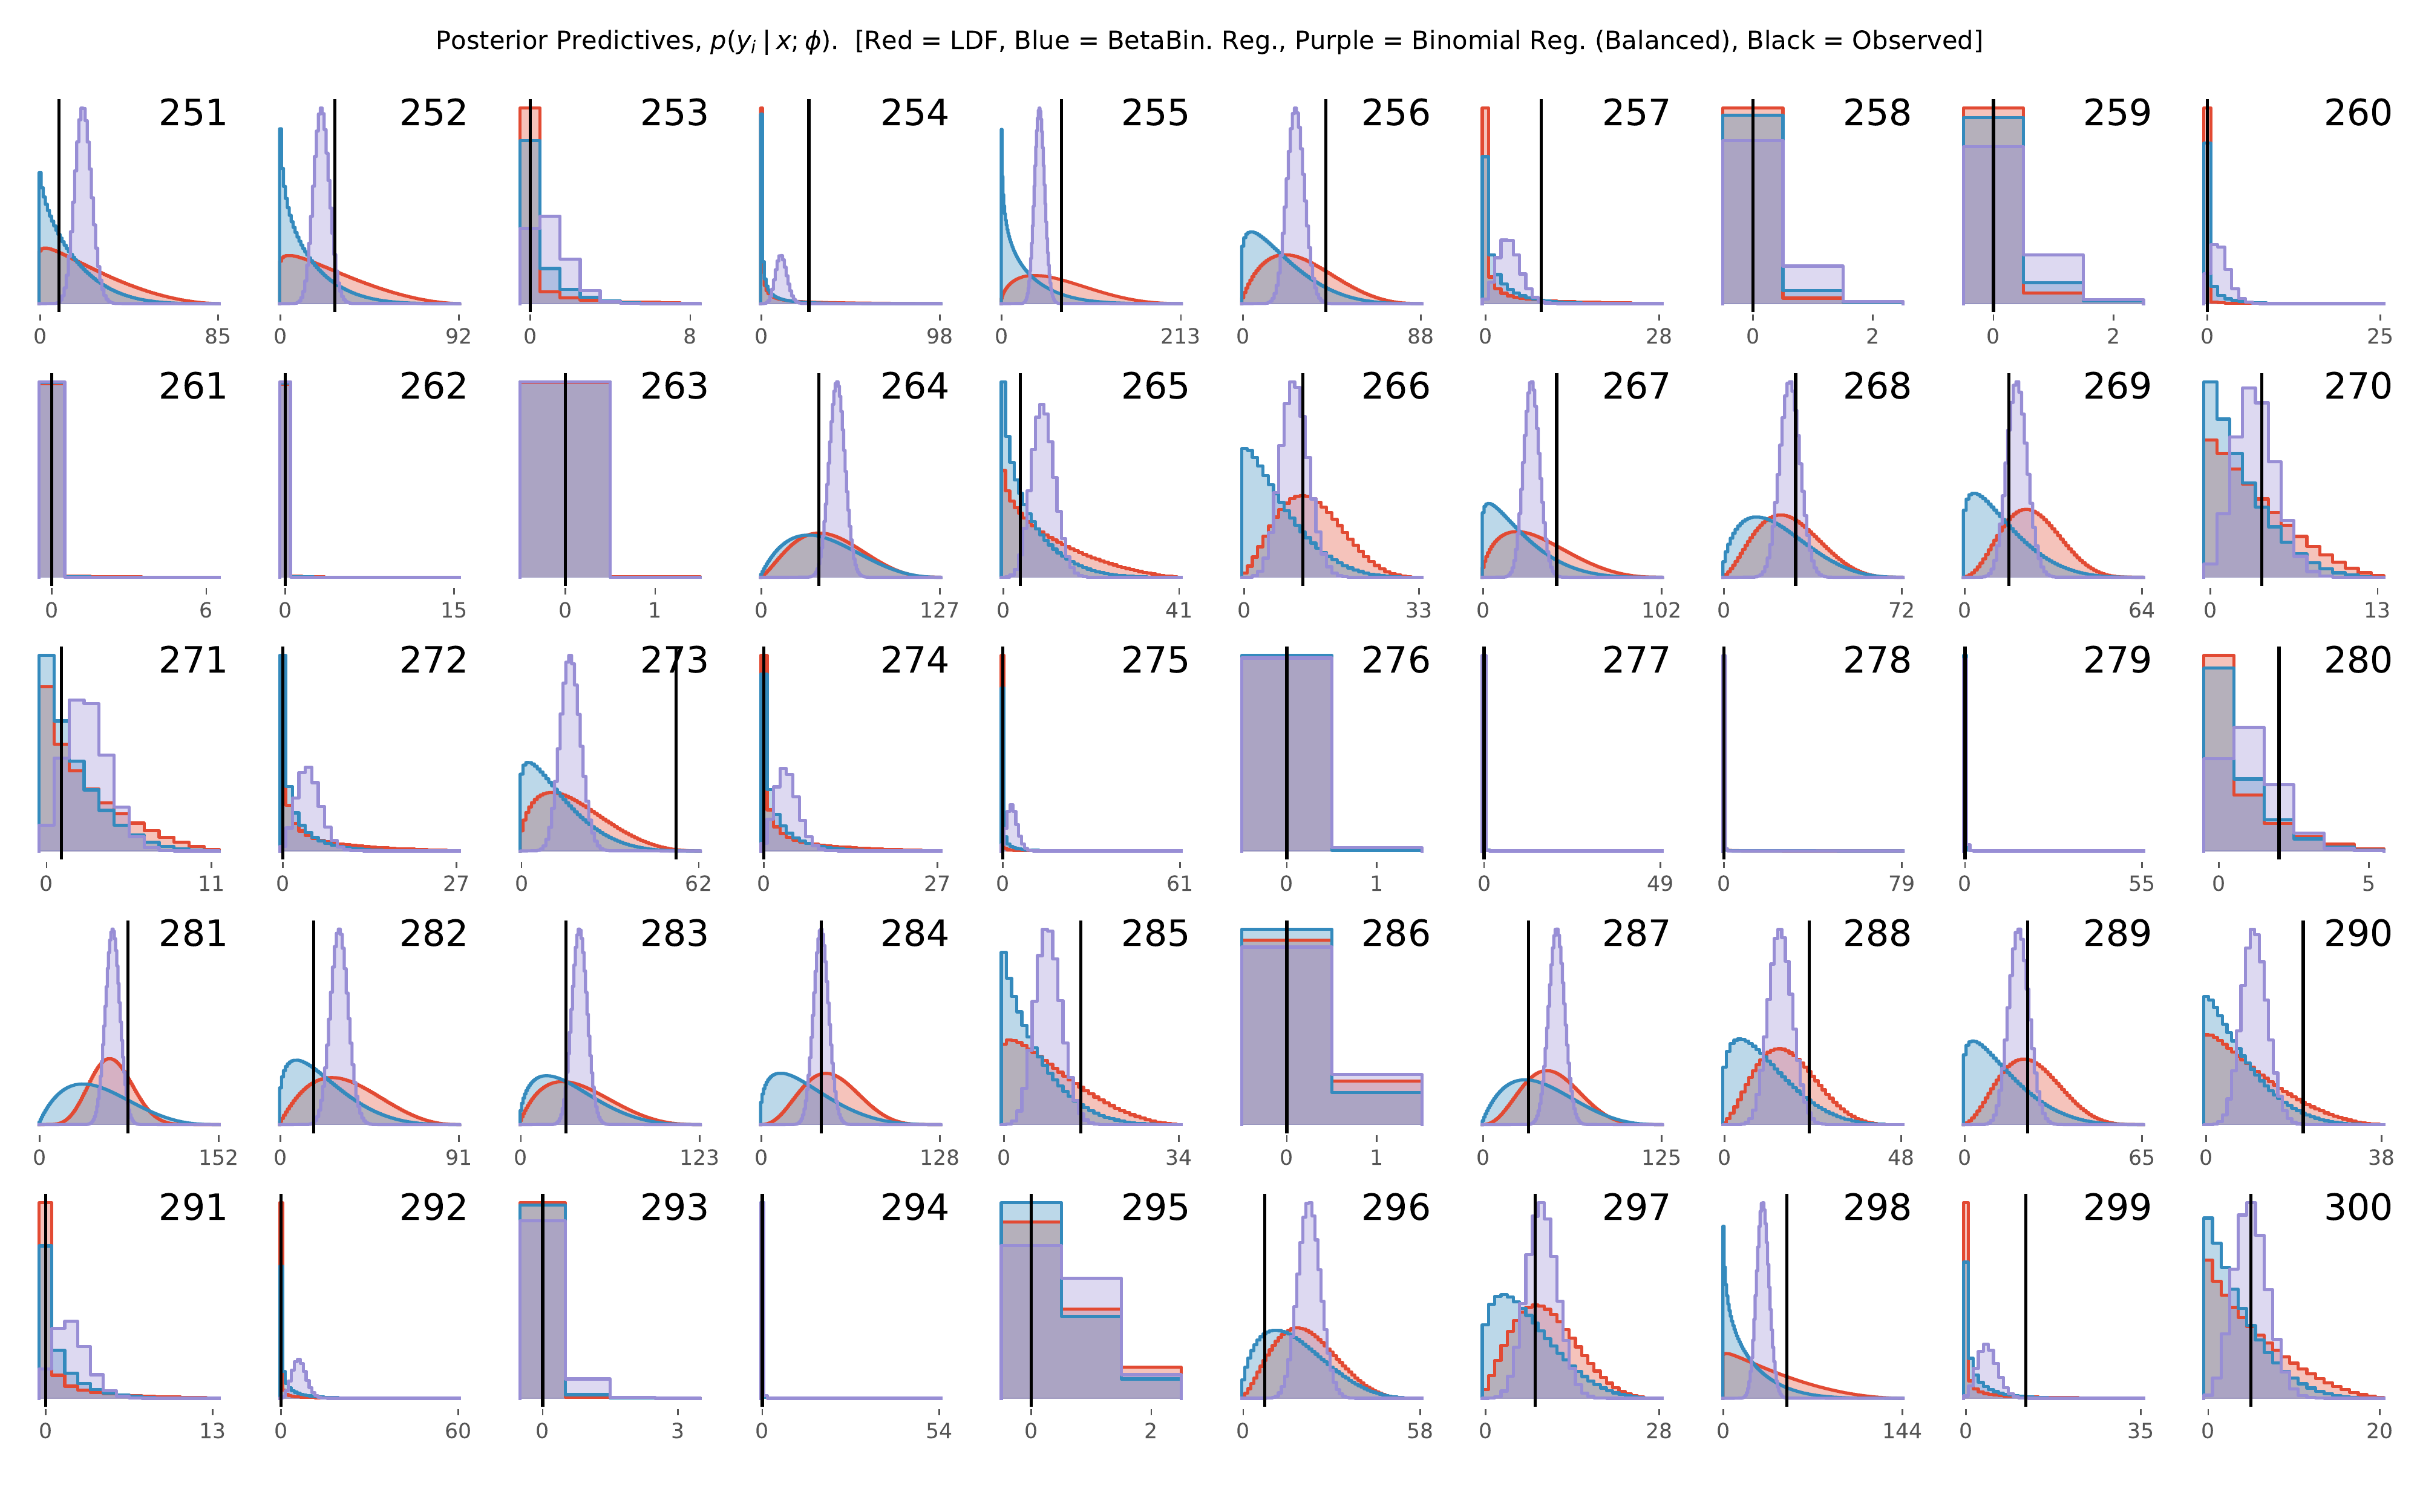}}
    \caption{\small \textbf{Primary data posterior predictives (continued).}  A subset of the predictive likelihoods $p(y_i \given x; \phi)$ for the electrification application.  LDF is red, beta-binomial regression is blue, binomial regression is purple, and the observed value is black.}
    
  \end{center}
  \vspace*{-5mm}
\end{figure}

\begin{figure}[t]
  \vskip 0.1in
  \begin{center}
    \centerline{\includegraphics[width=0.75\linewidth, trim={0.375cm 1cm 0.375cm 1.5cm},clip]{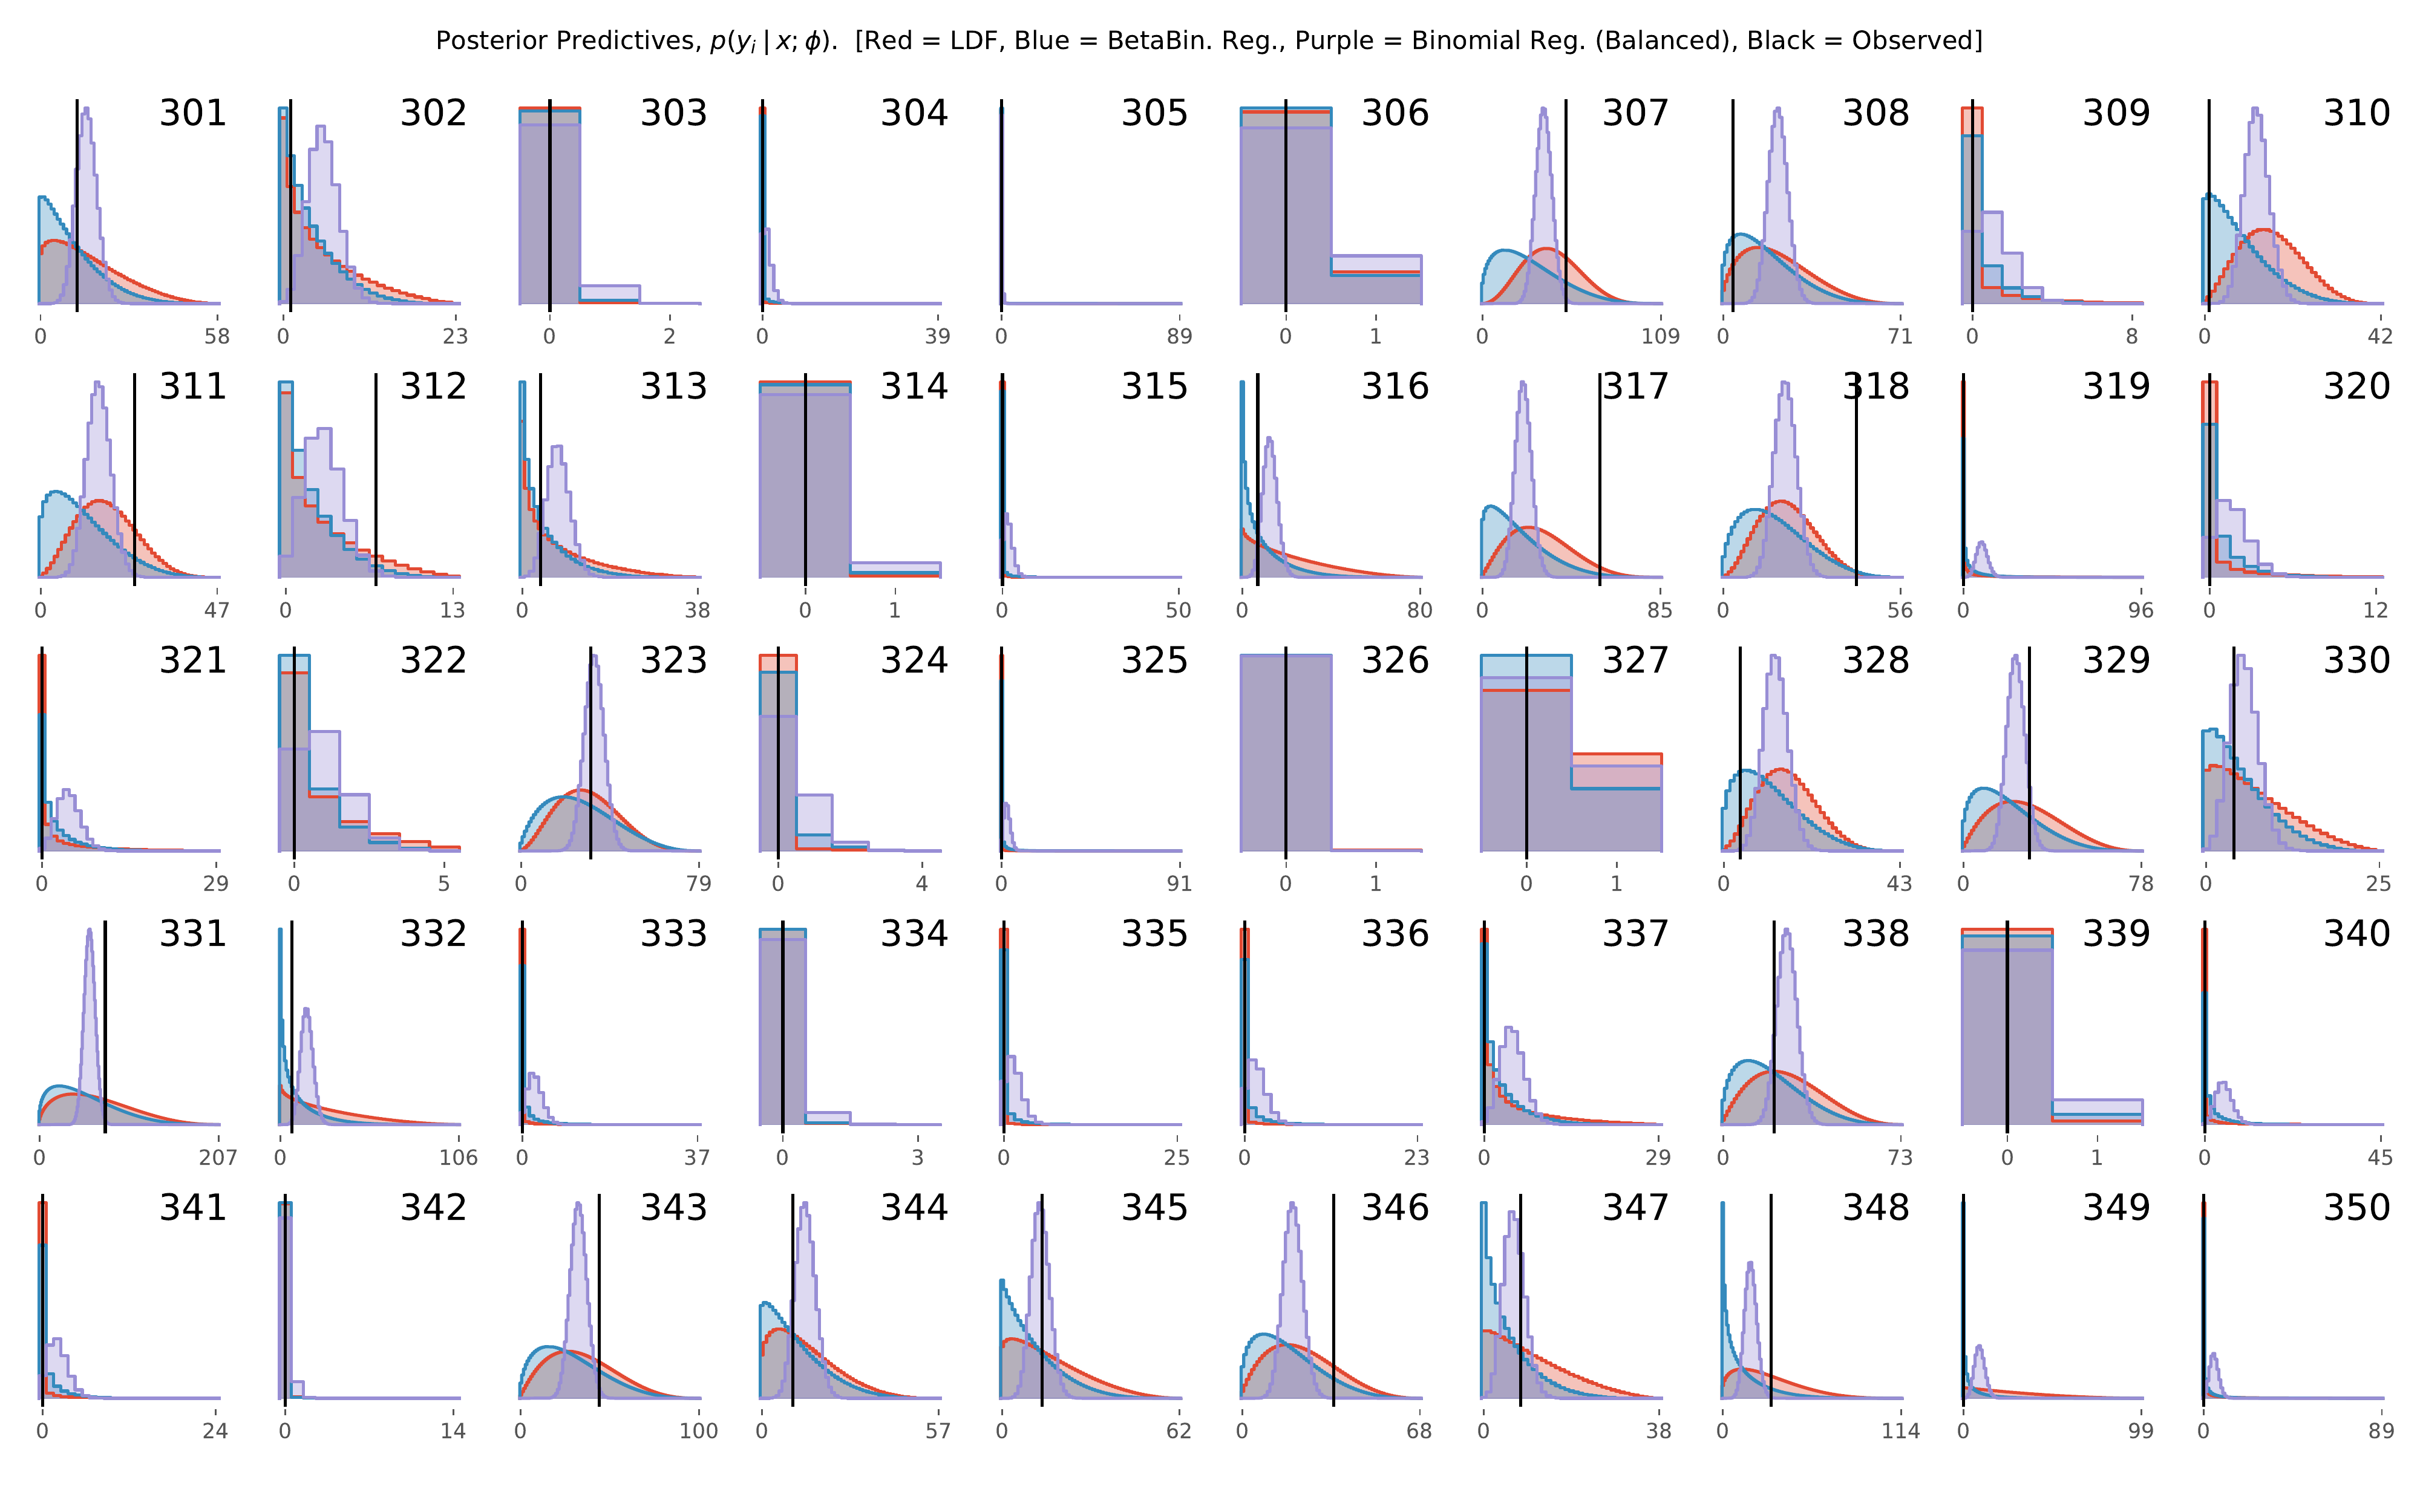}}
    \centerline{\includegraphics[width=0.75\linewidth, trim={0.375cm 1cm 0.375cm 1.5cm},clip]{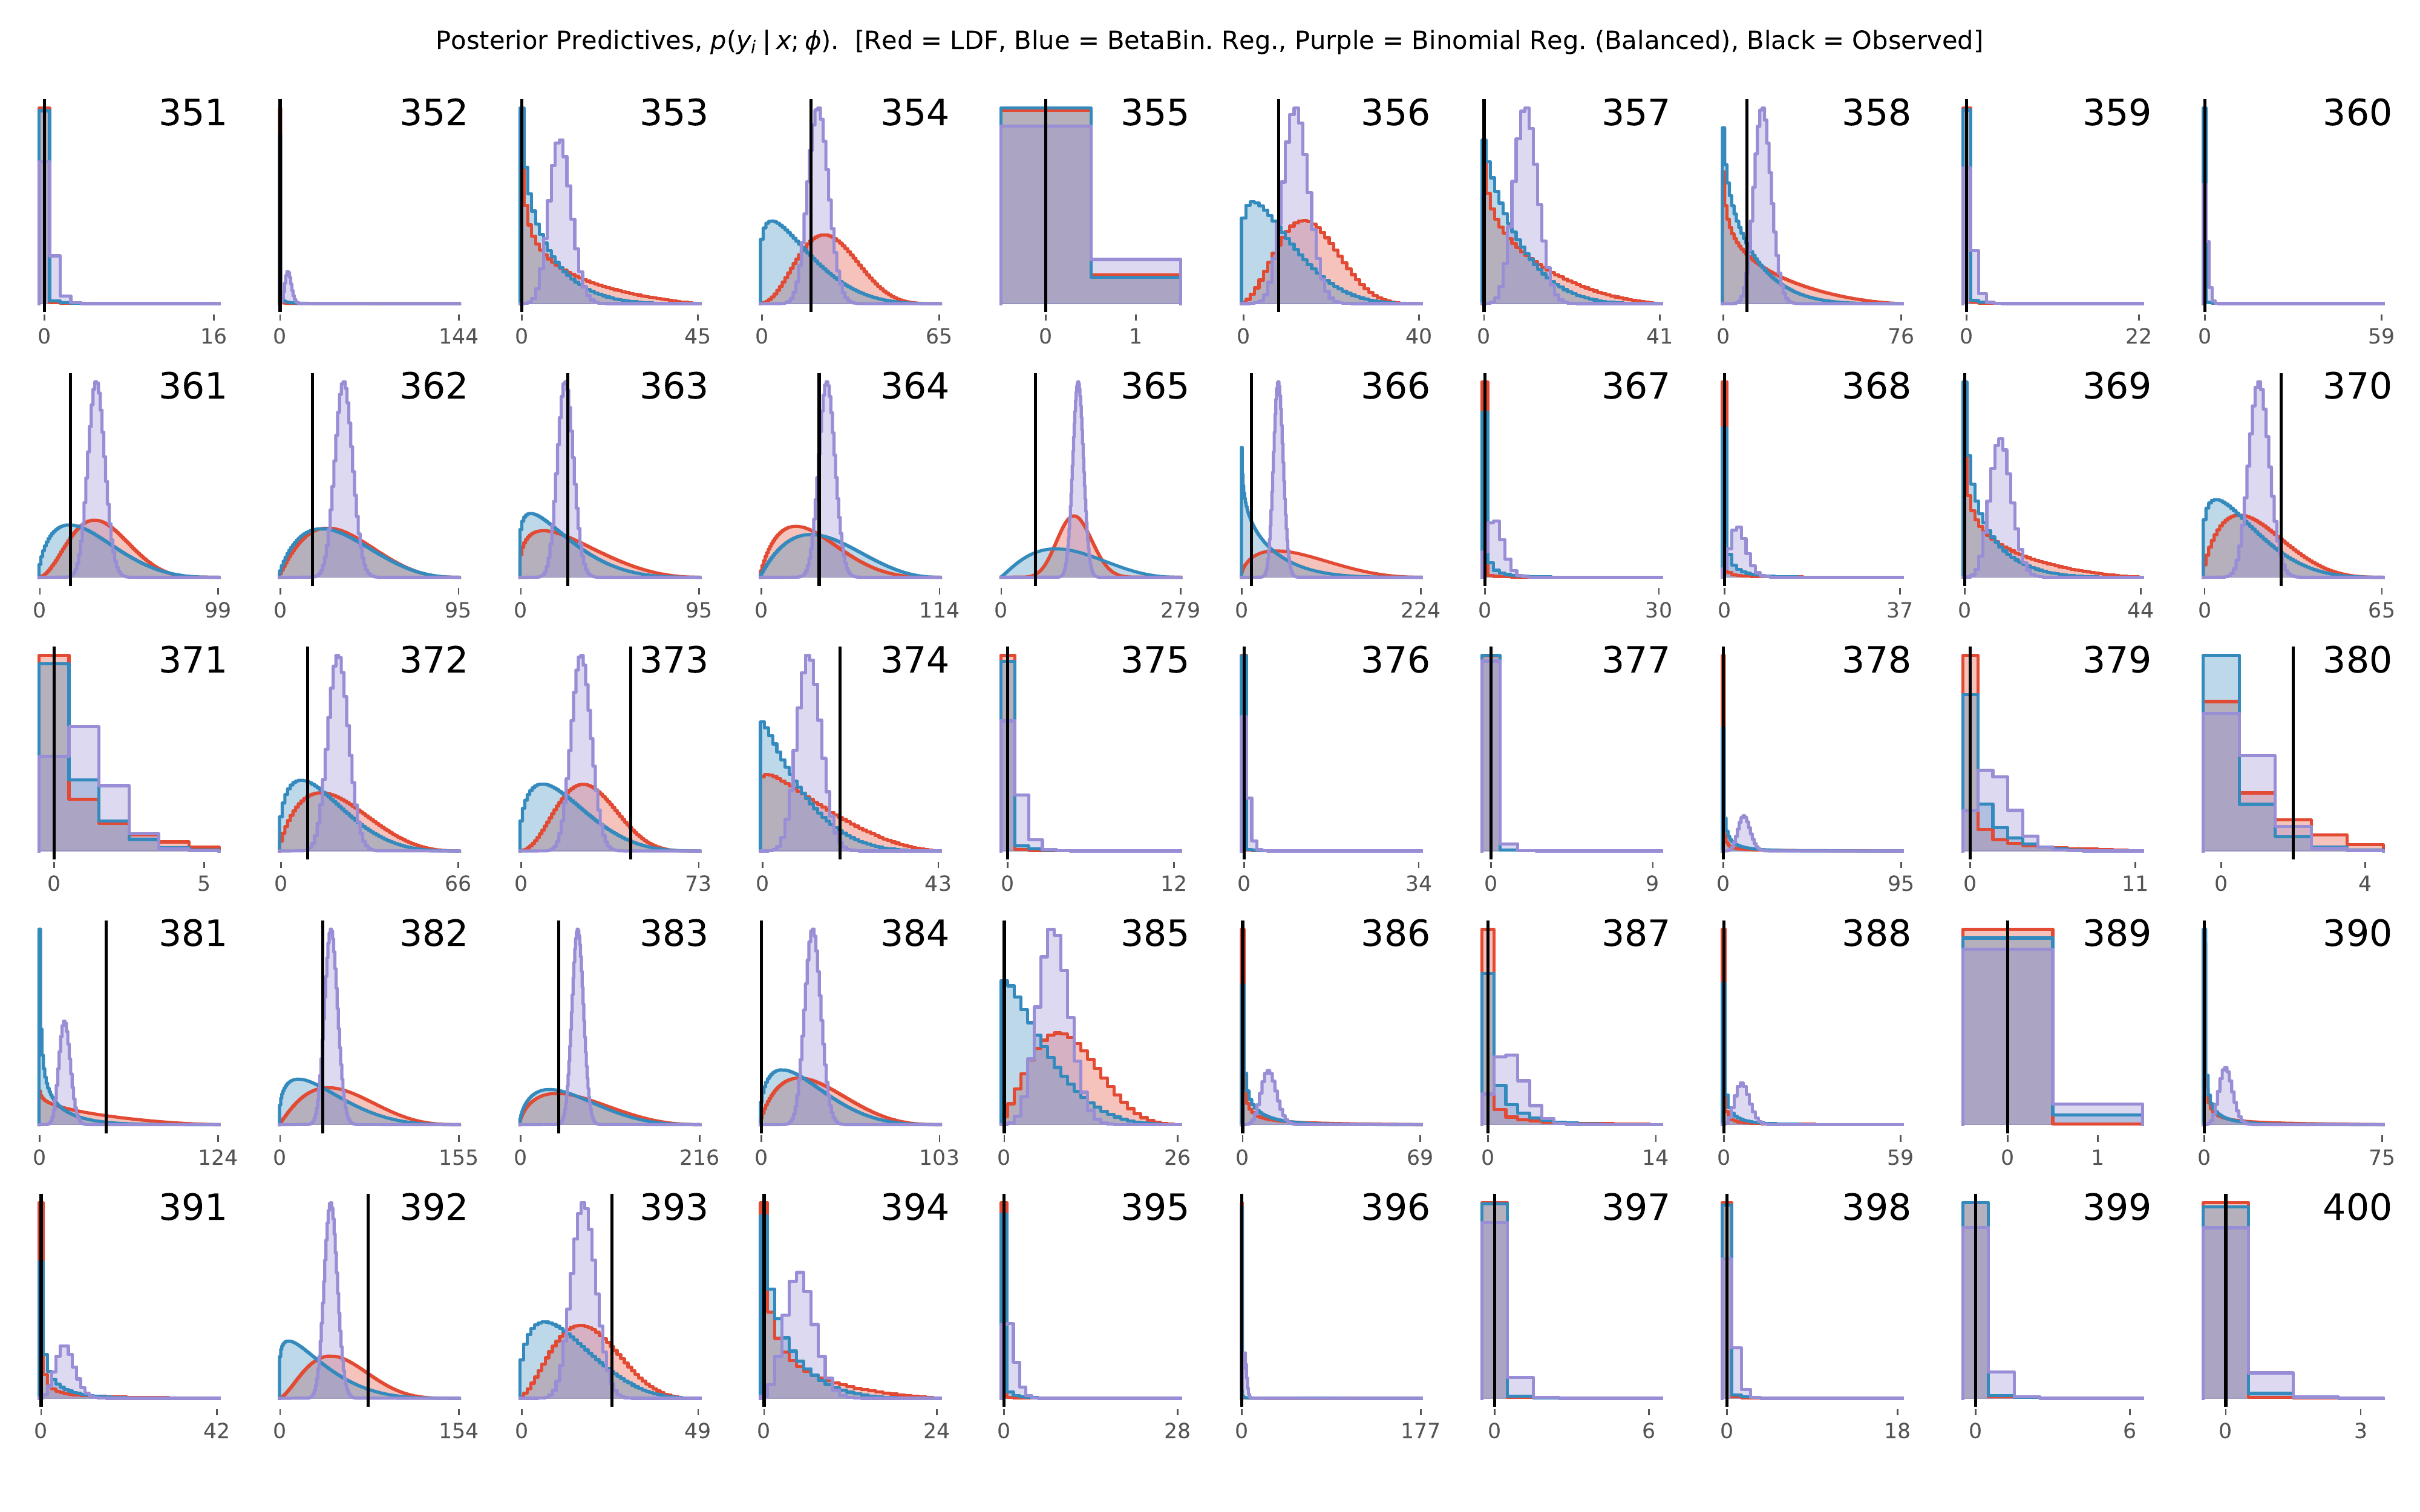}}
     \centerline{\includegraphics[width=0.75\linewidth, trim={0.375cm 1cm 0.375cm 1.5cm},clip]{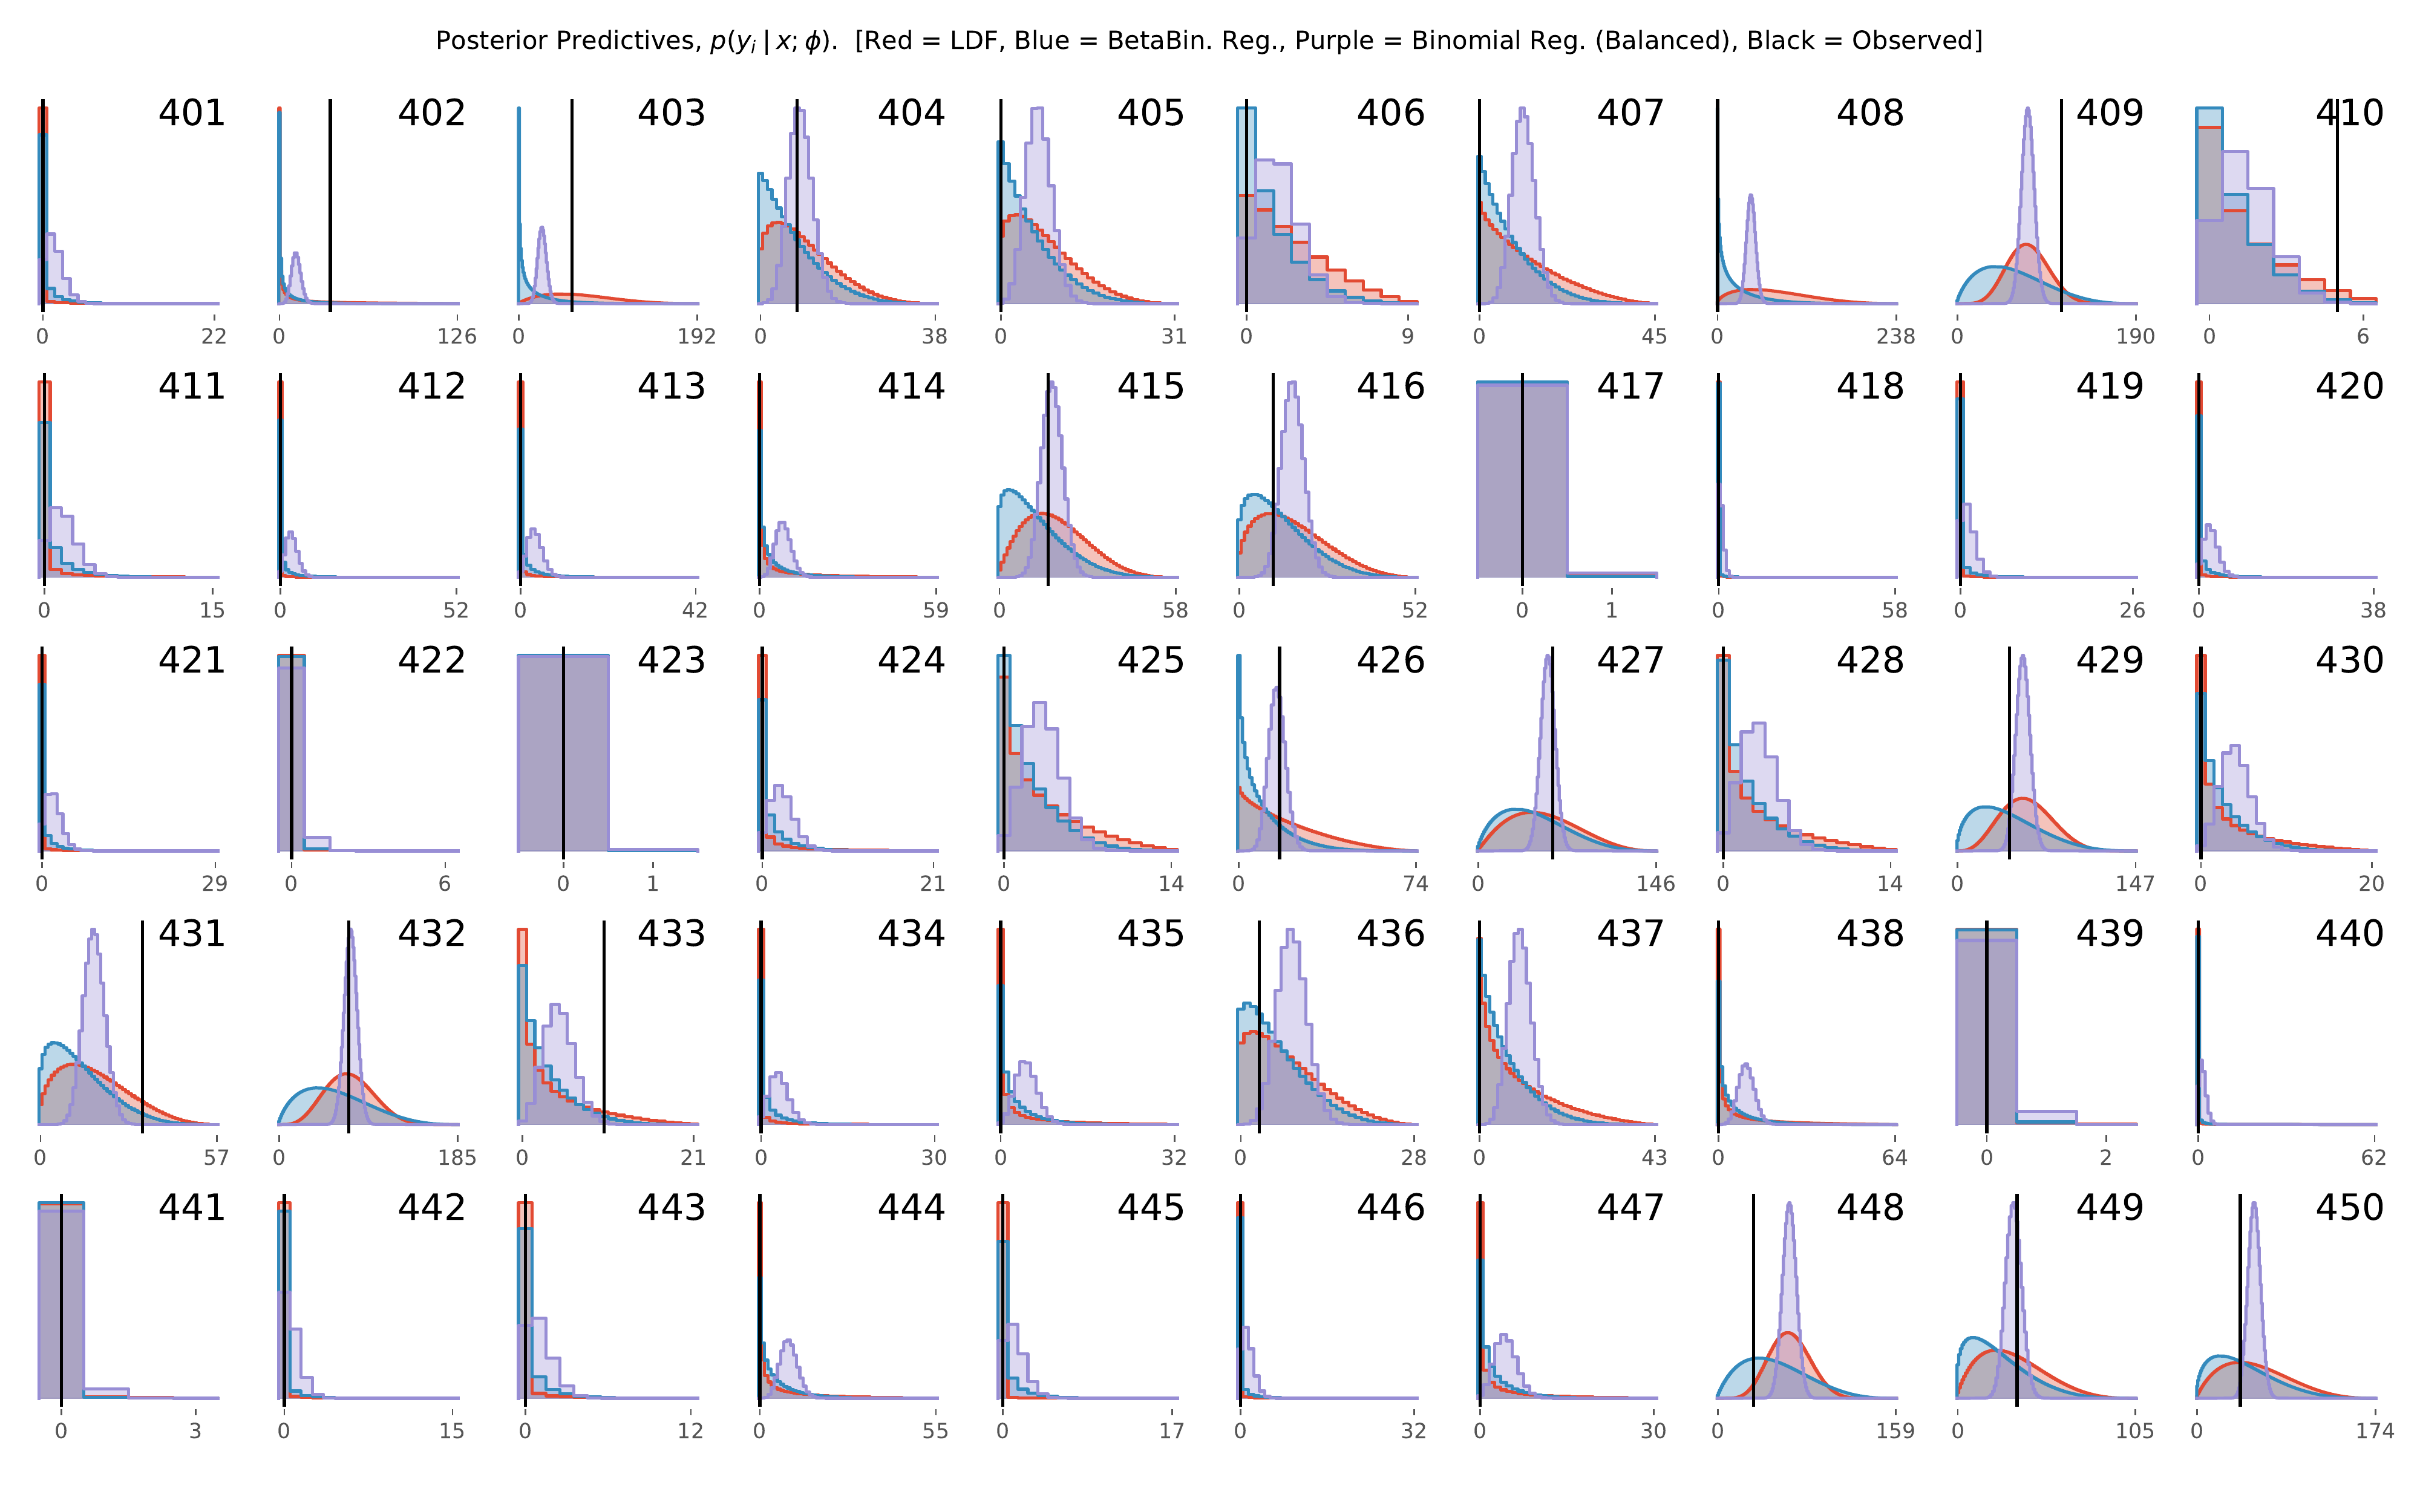}}
    \caption{\small \textbf{Primary data posterior predictives (continued).}  A subset of the predictive likelihoods $p(y_i \given x; \phi)$ for the electrification application.  LDF is red, beta-binomial regression is blue, binomial regression is purple, and the observed value is black.}
    
  \end{center}
  \vspace*{-5mm}
\end{figure}

\begin{figure}[t]
  \vskip 0.1in
  \begin{center}
    \centerline{\includegraphics[width=0.75\linewidth, trim={0.375cm 1cm 0.375cm 1.5cm},clip]{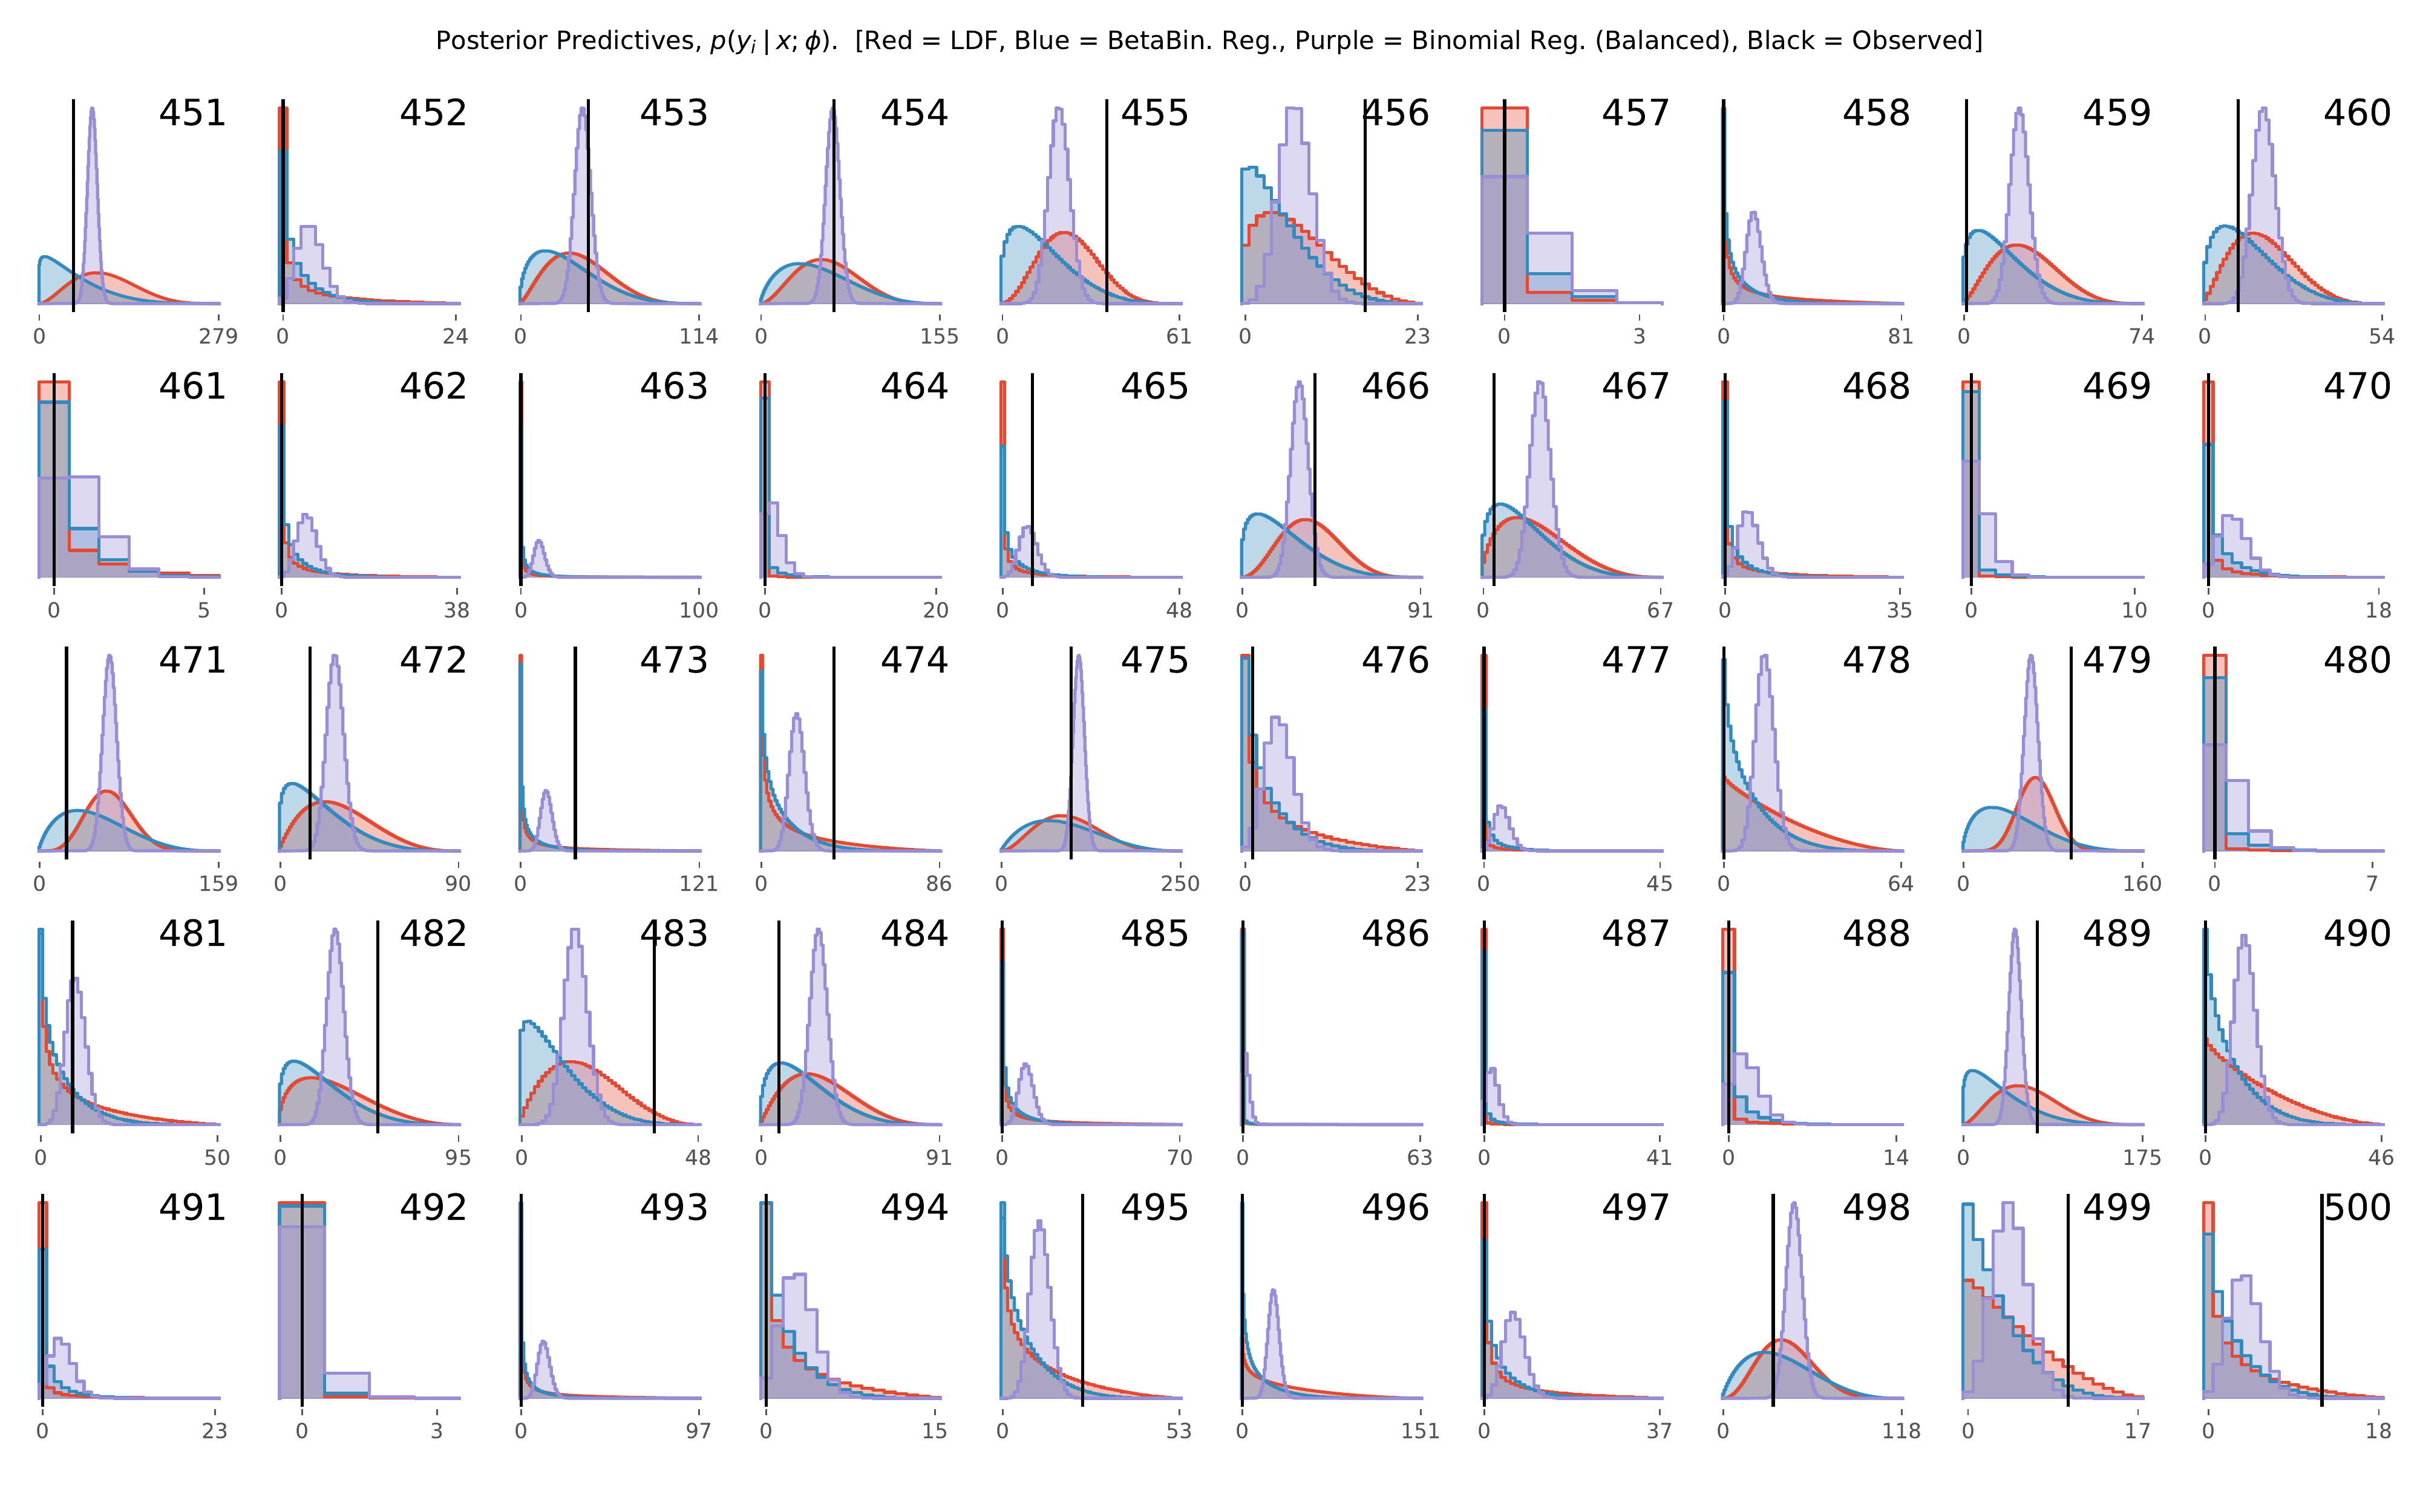}}
    \centerline{\includegraphics[width=0.75\linewidth, trim={0.375cm 1cm 0.375cm 1.5cm},clip]{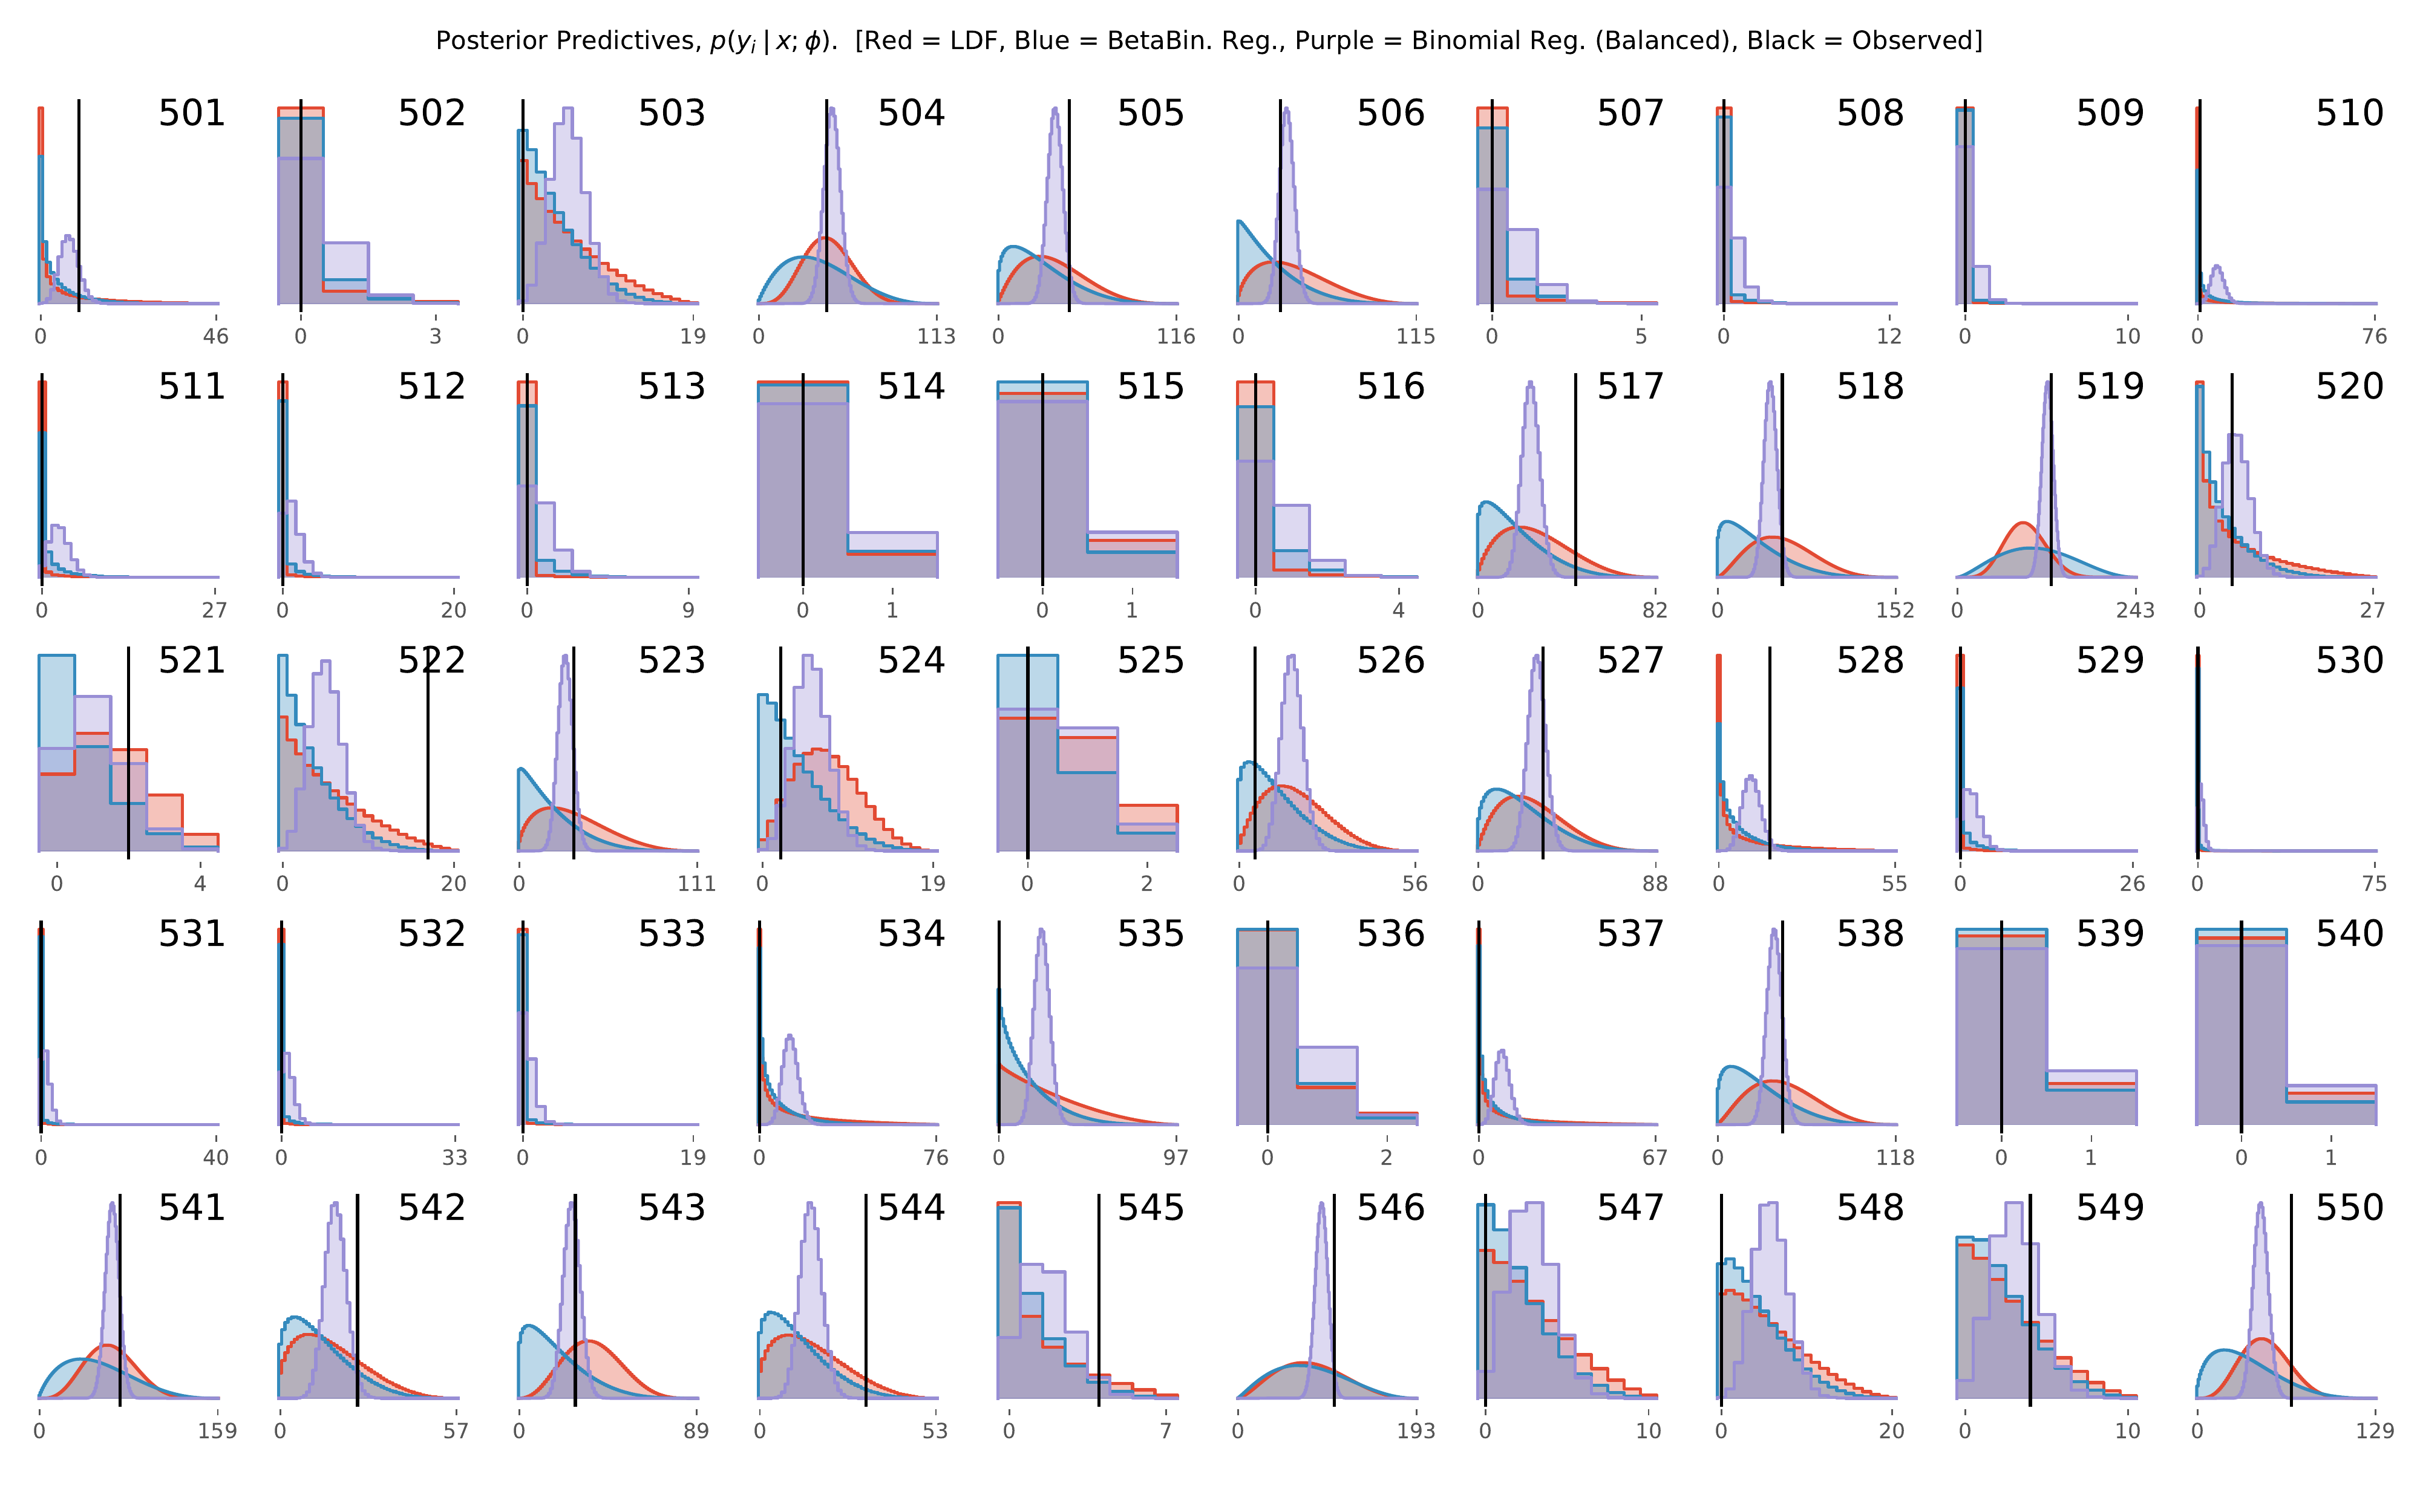}}
     \centerline{\includegraphics[width=0.75\linewidth, trim={0.375cm 1cm 0.375cm 1.5cm},clip]{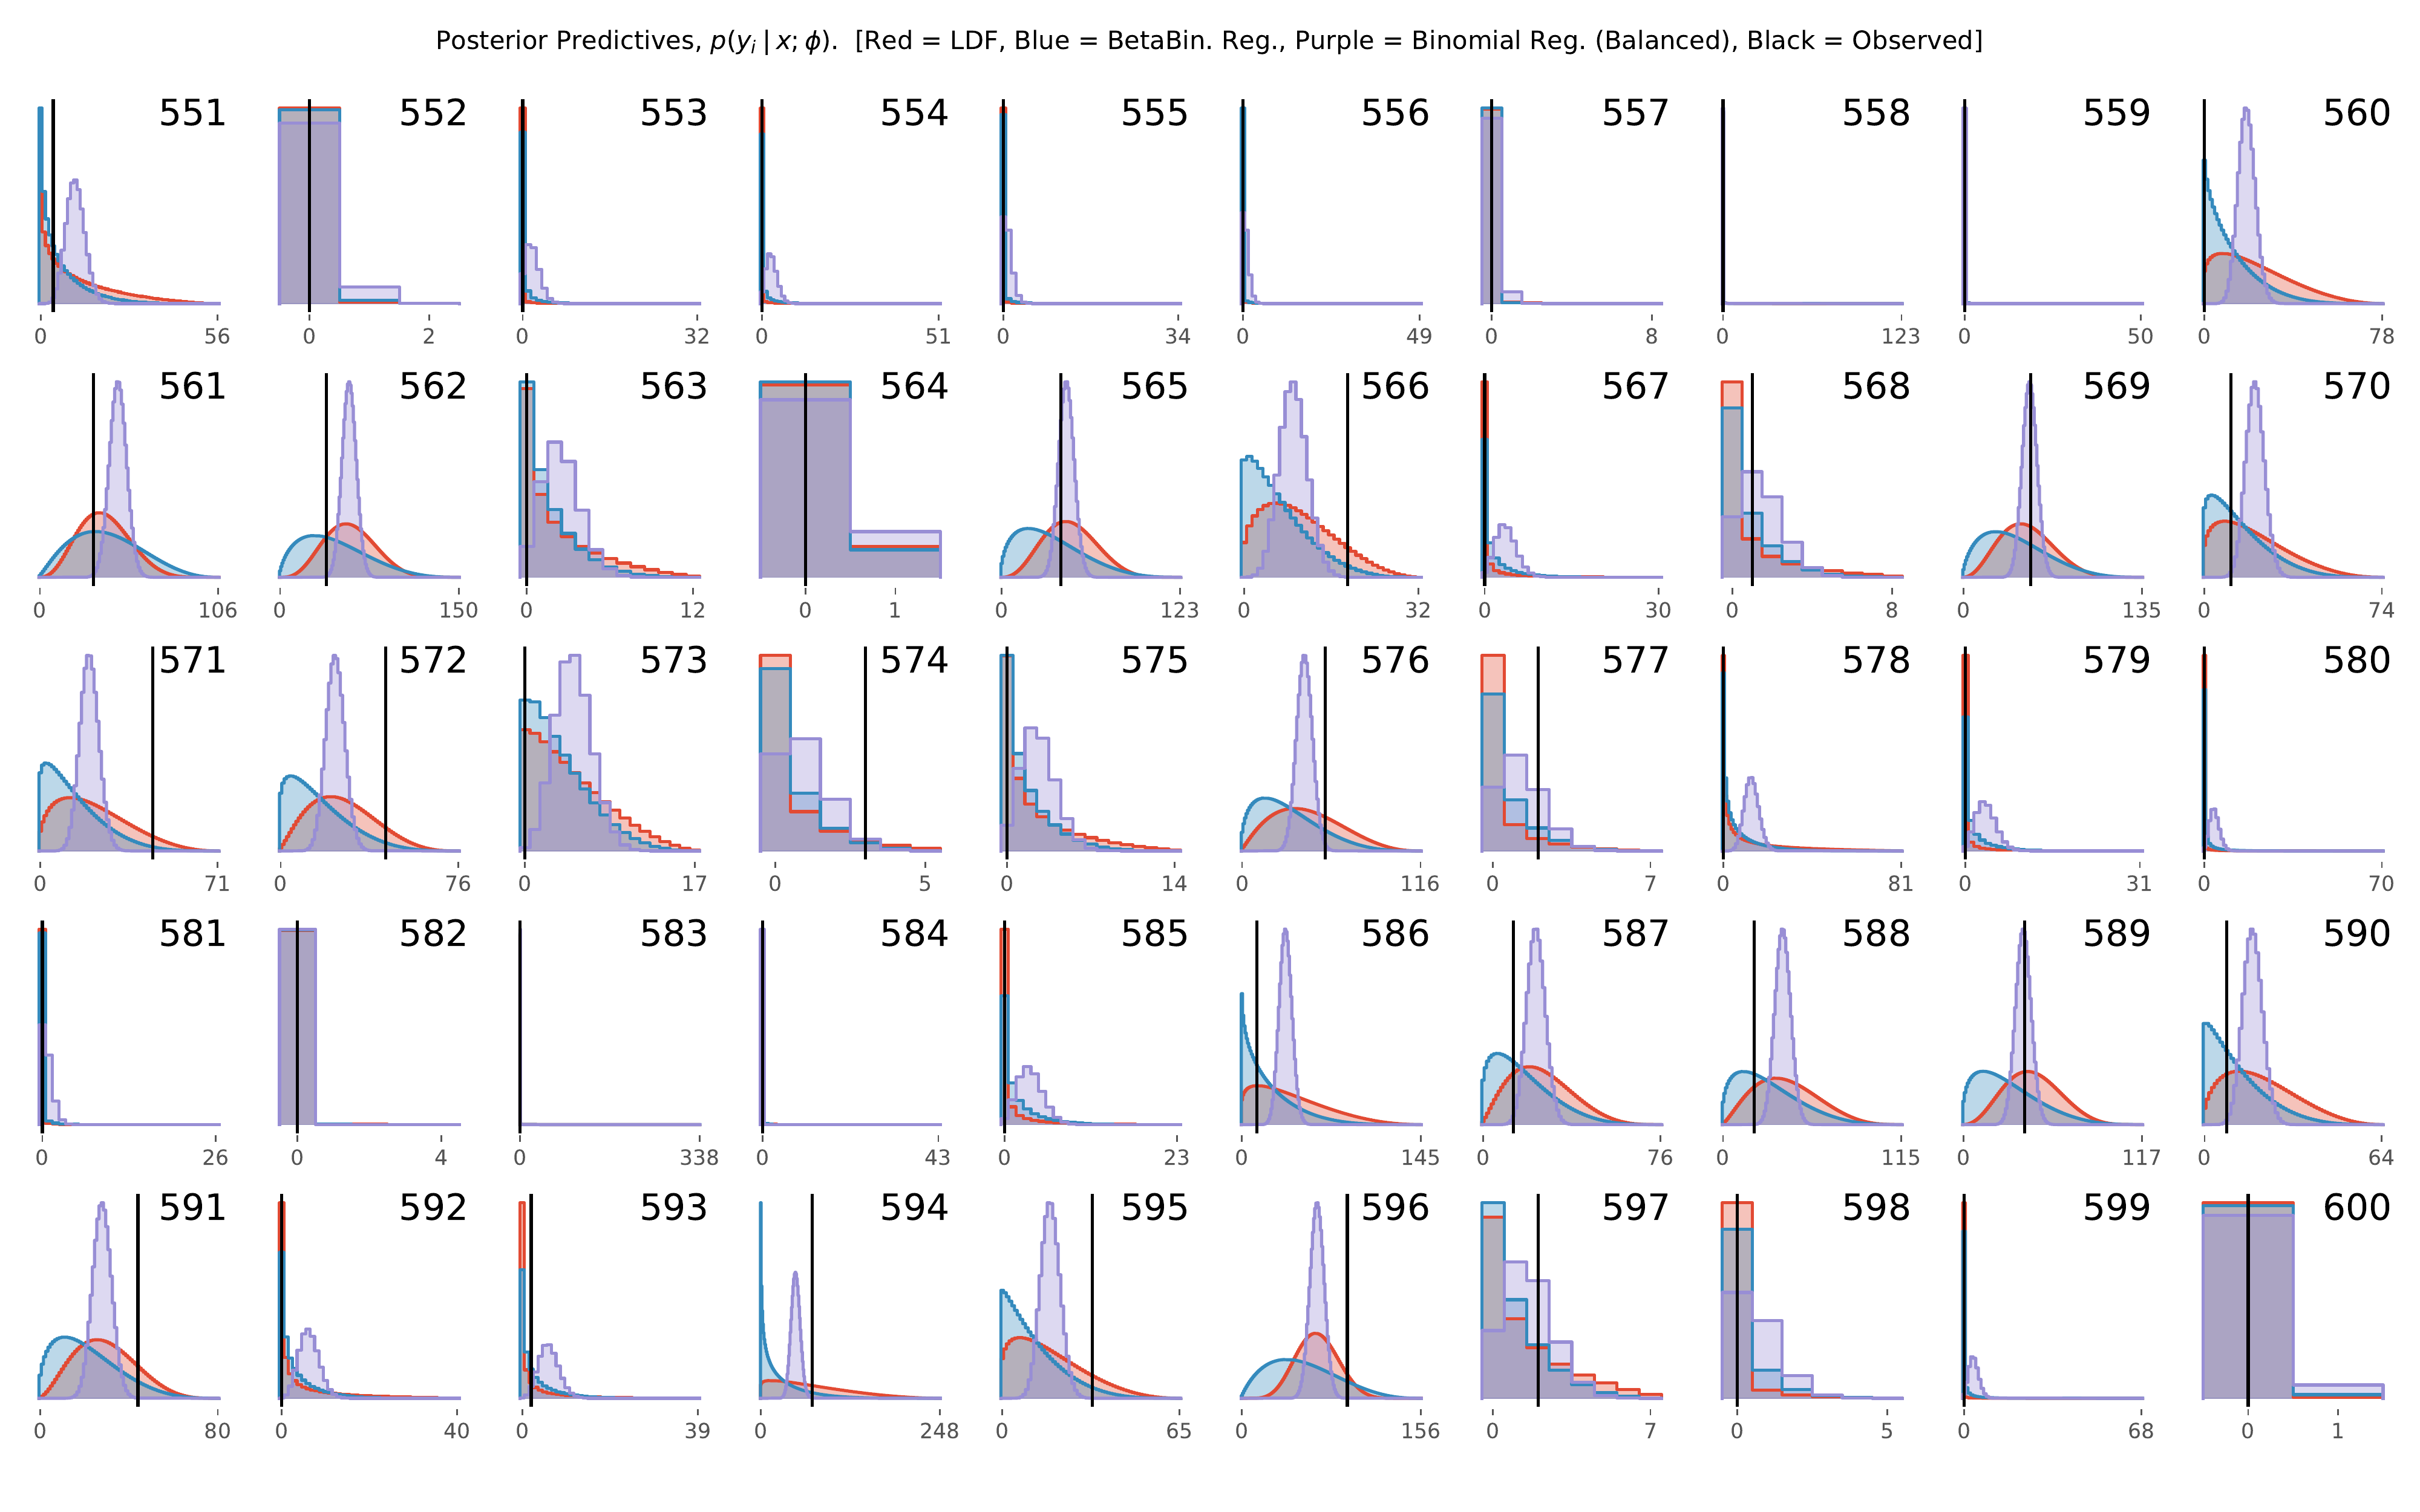}}
    \caption{\small \textbf{Primary data posterior predictives (continued).}  A subset of the predictive likelihoods $p(y_i \given x; \phi)$ for the electrification application.  LDF is red, beta-binomial regression is blue, binomial regression is purple, and the observed value is black.}
    
  \end{center}
  \vspace*{-5mm}
\end{figure}

\begin{figure}[t]
  \vskip 0.1in
  \begin{center}
    \centerline{\includegraphics[width=0.75\linewidth, trim={0.375cm 1cm 0.375cm 1.5cm},clip]{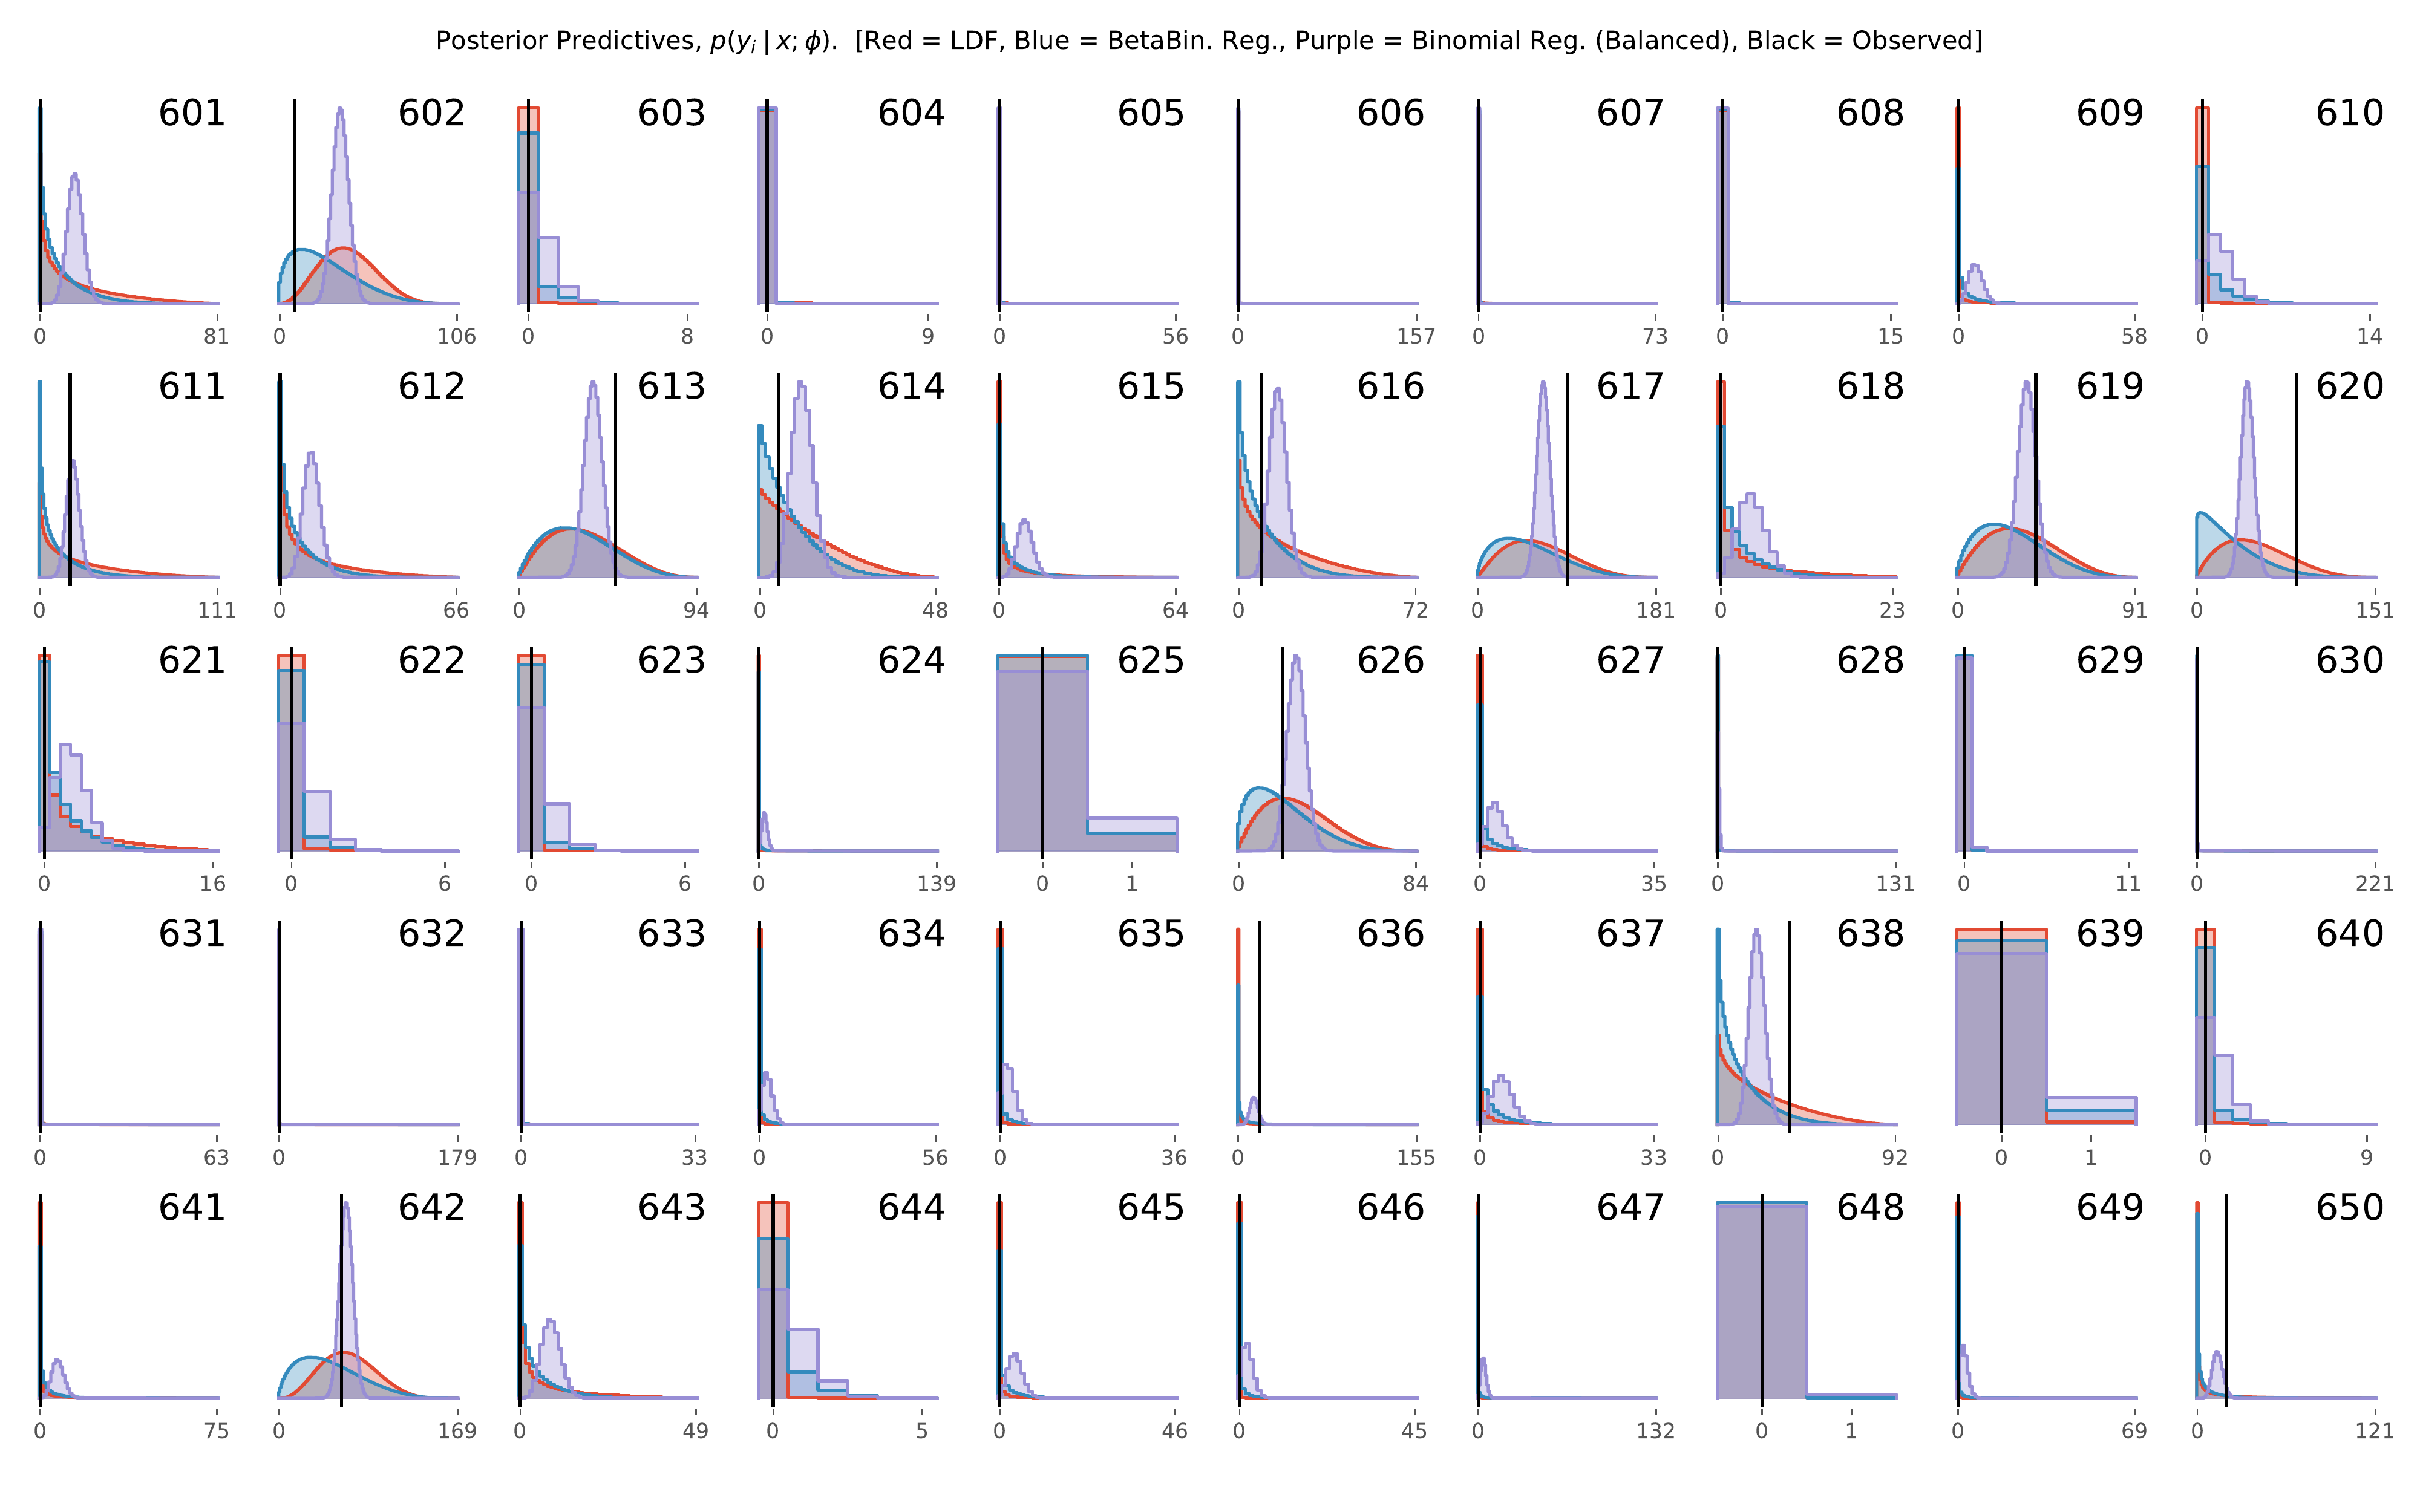}}
    \centerline{\includegraphics[width=0.75\linewidth, trim={0.375cm 1cm 0.375cm 1.5cm},clip]{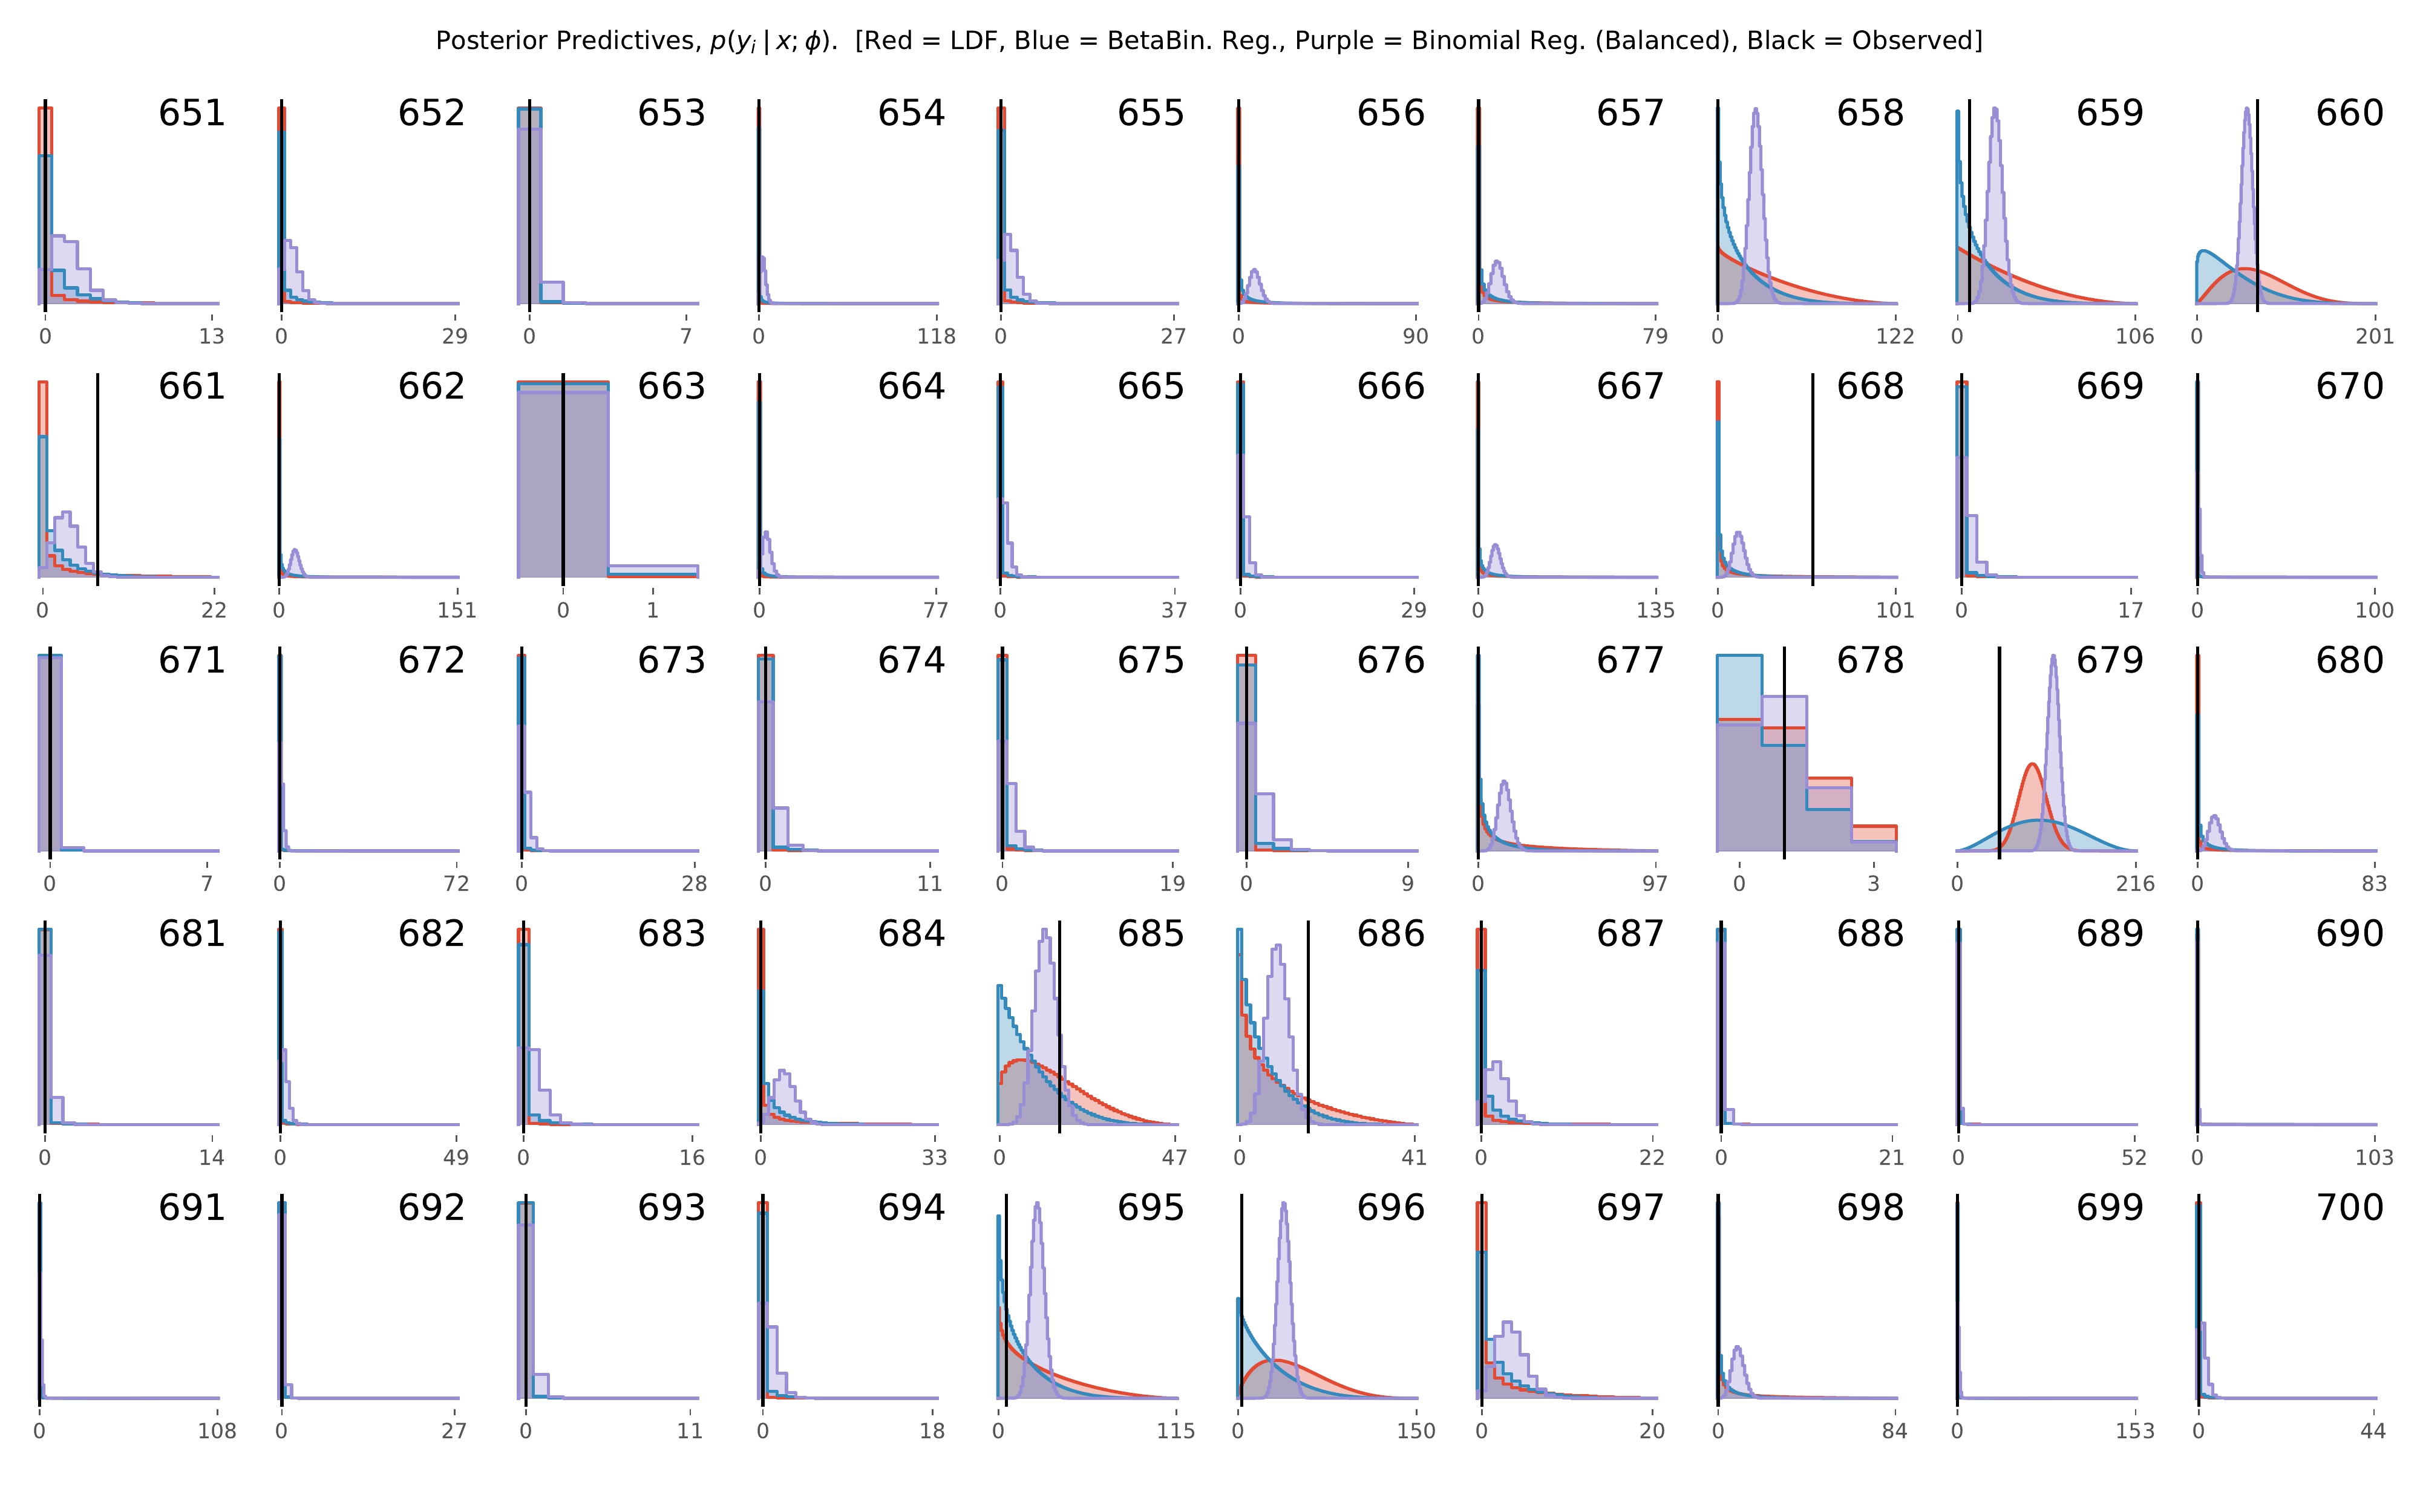}}
     \centerline{\includegraphics[width=0.75\linewidth, trim={0.375cm 1cm 0.375cm 1.5cm},clip]{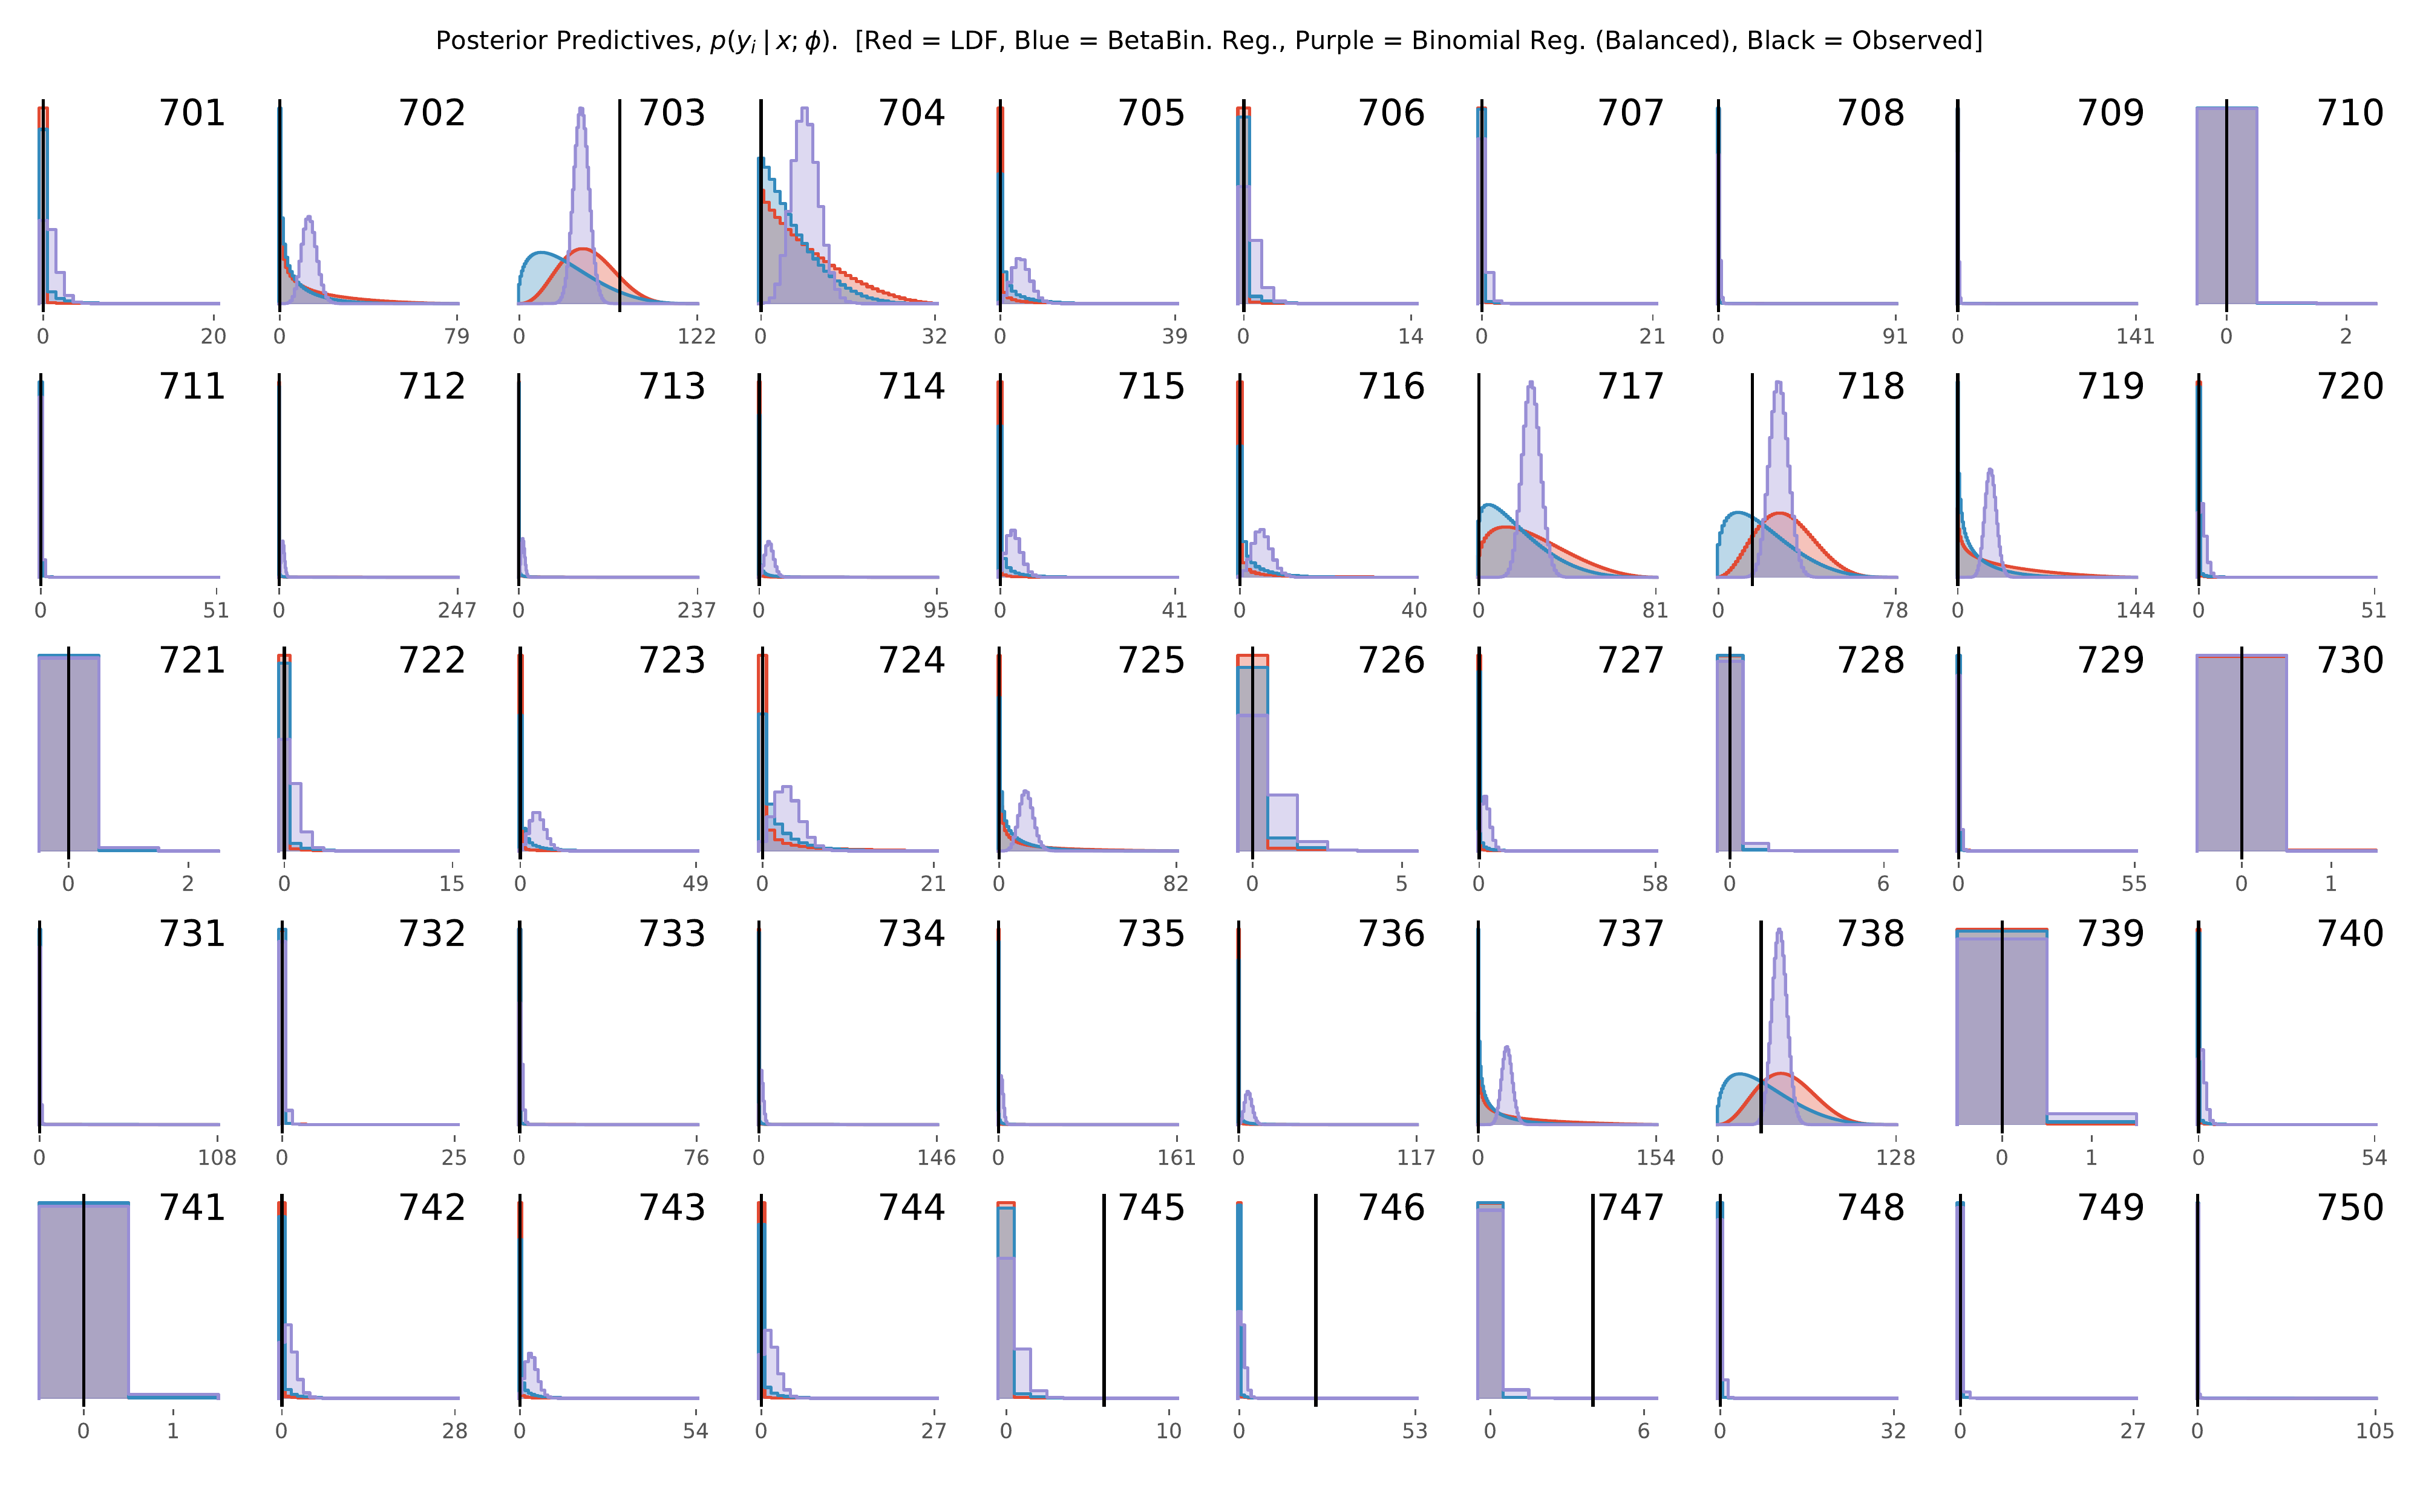}}
    \caption{\small \textbf{Primary data posterior predictives (continued).}  A subset of the predictive likelihoods $p(y_i \given x; \phi)$ for the electrification application.  LDF is red, beta-binomial regression is blue, binomial regression is purple, and the observed value is black.}
    
  \end{center}
  \vspace*{-5mm}
\end{figure}

\begin{figure}[t]
  \vskip 0.1in
  \begin{center}
    \centerline{\includegraphics[width=0.75\linewidth, trim={0.375cm 1cm 0.375cm 1.5cm},clip]{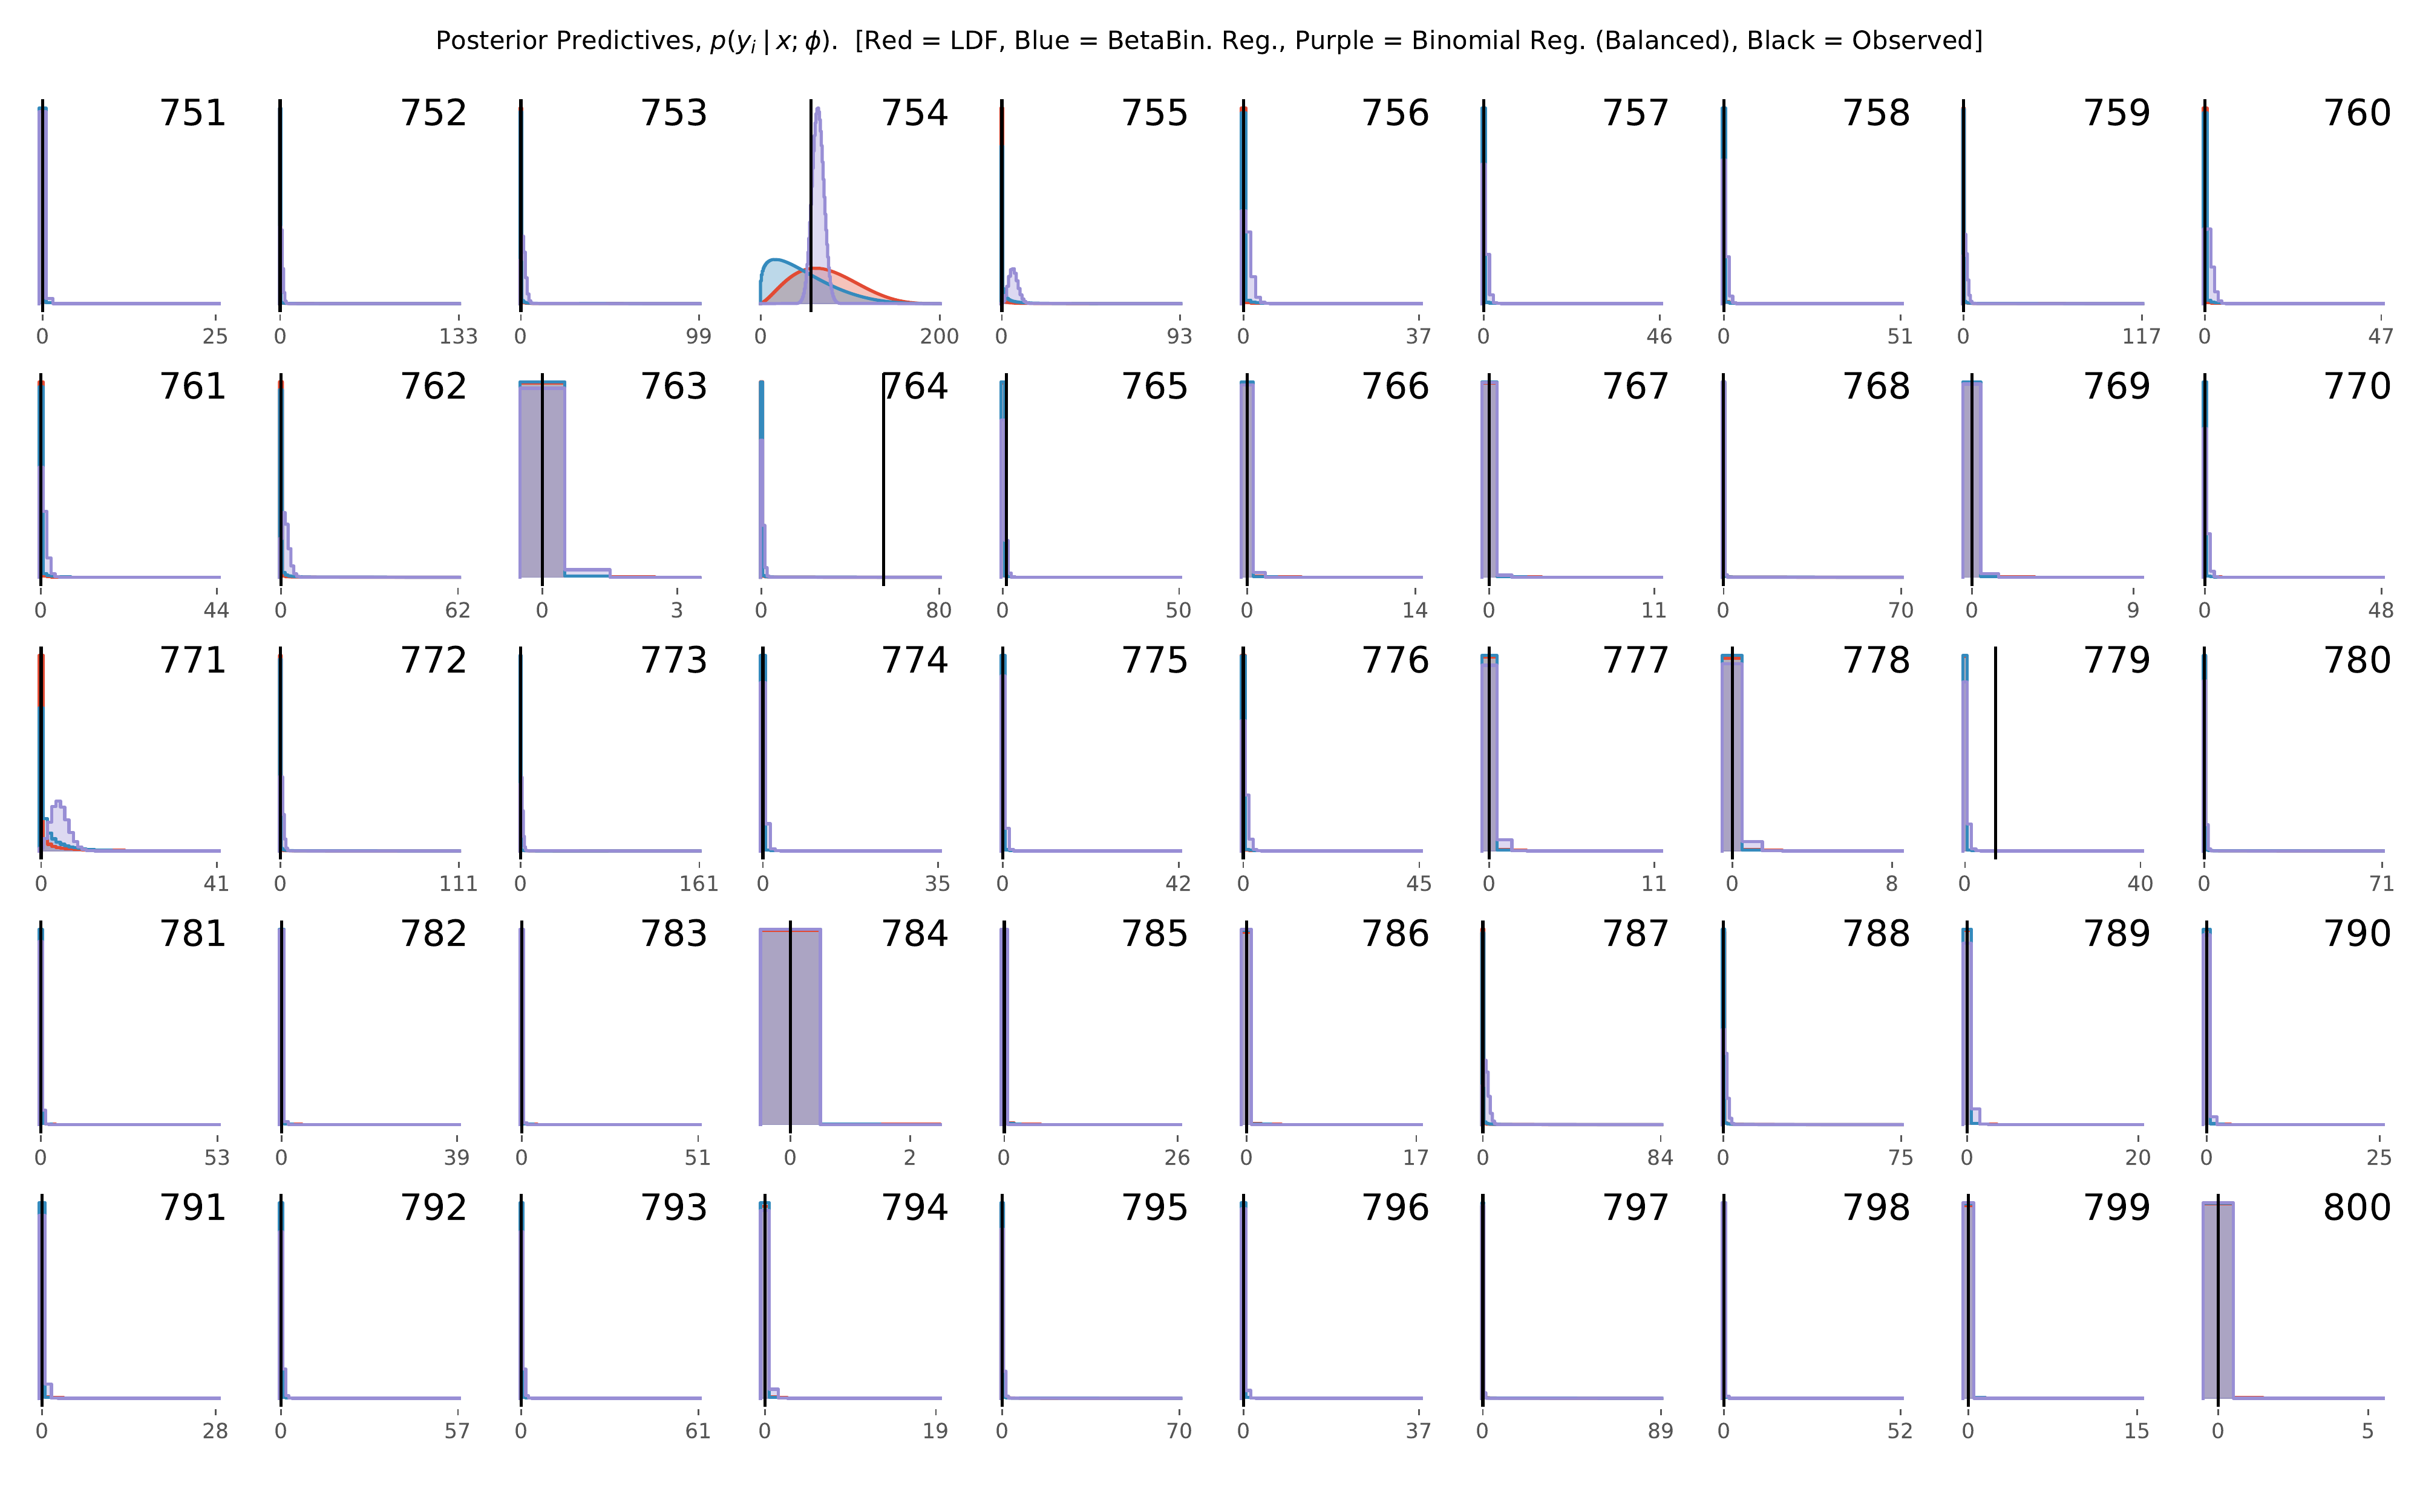}}
    \centerline{\includegraphics[width=0.75\linewidth, trim={0.375cm 1cm 0.375cm 1.5cm},clip]{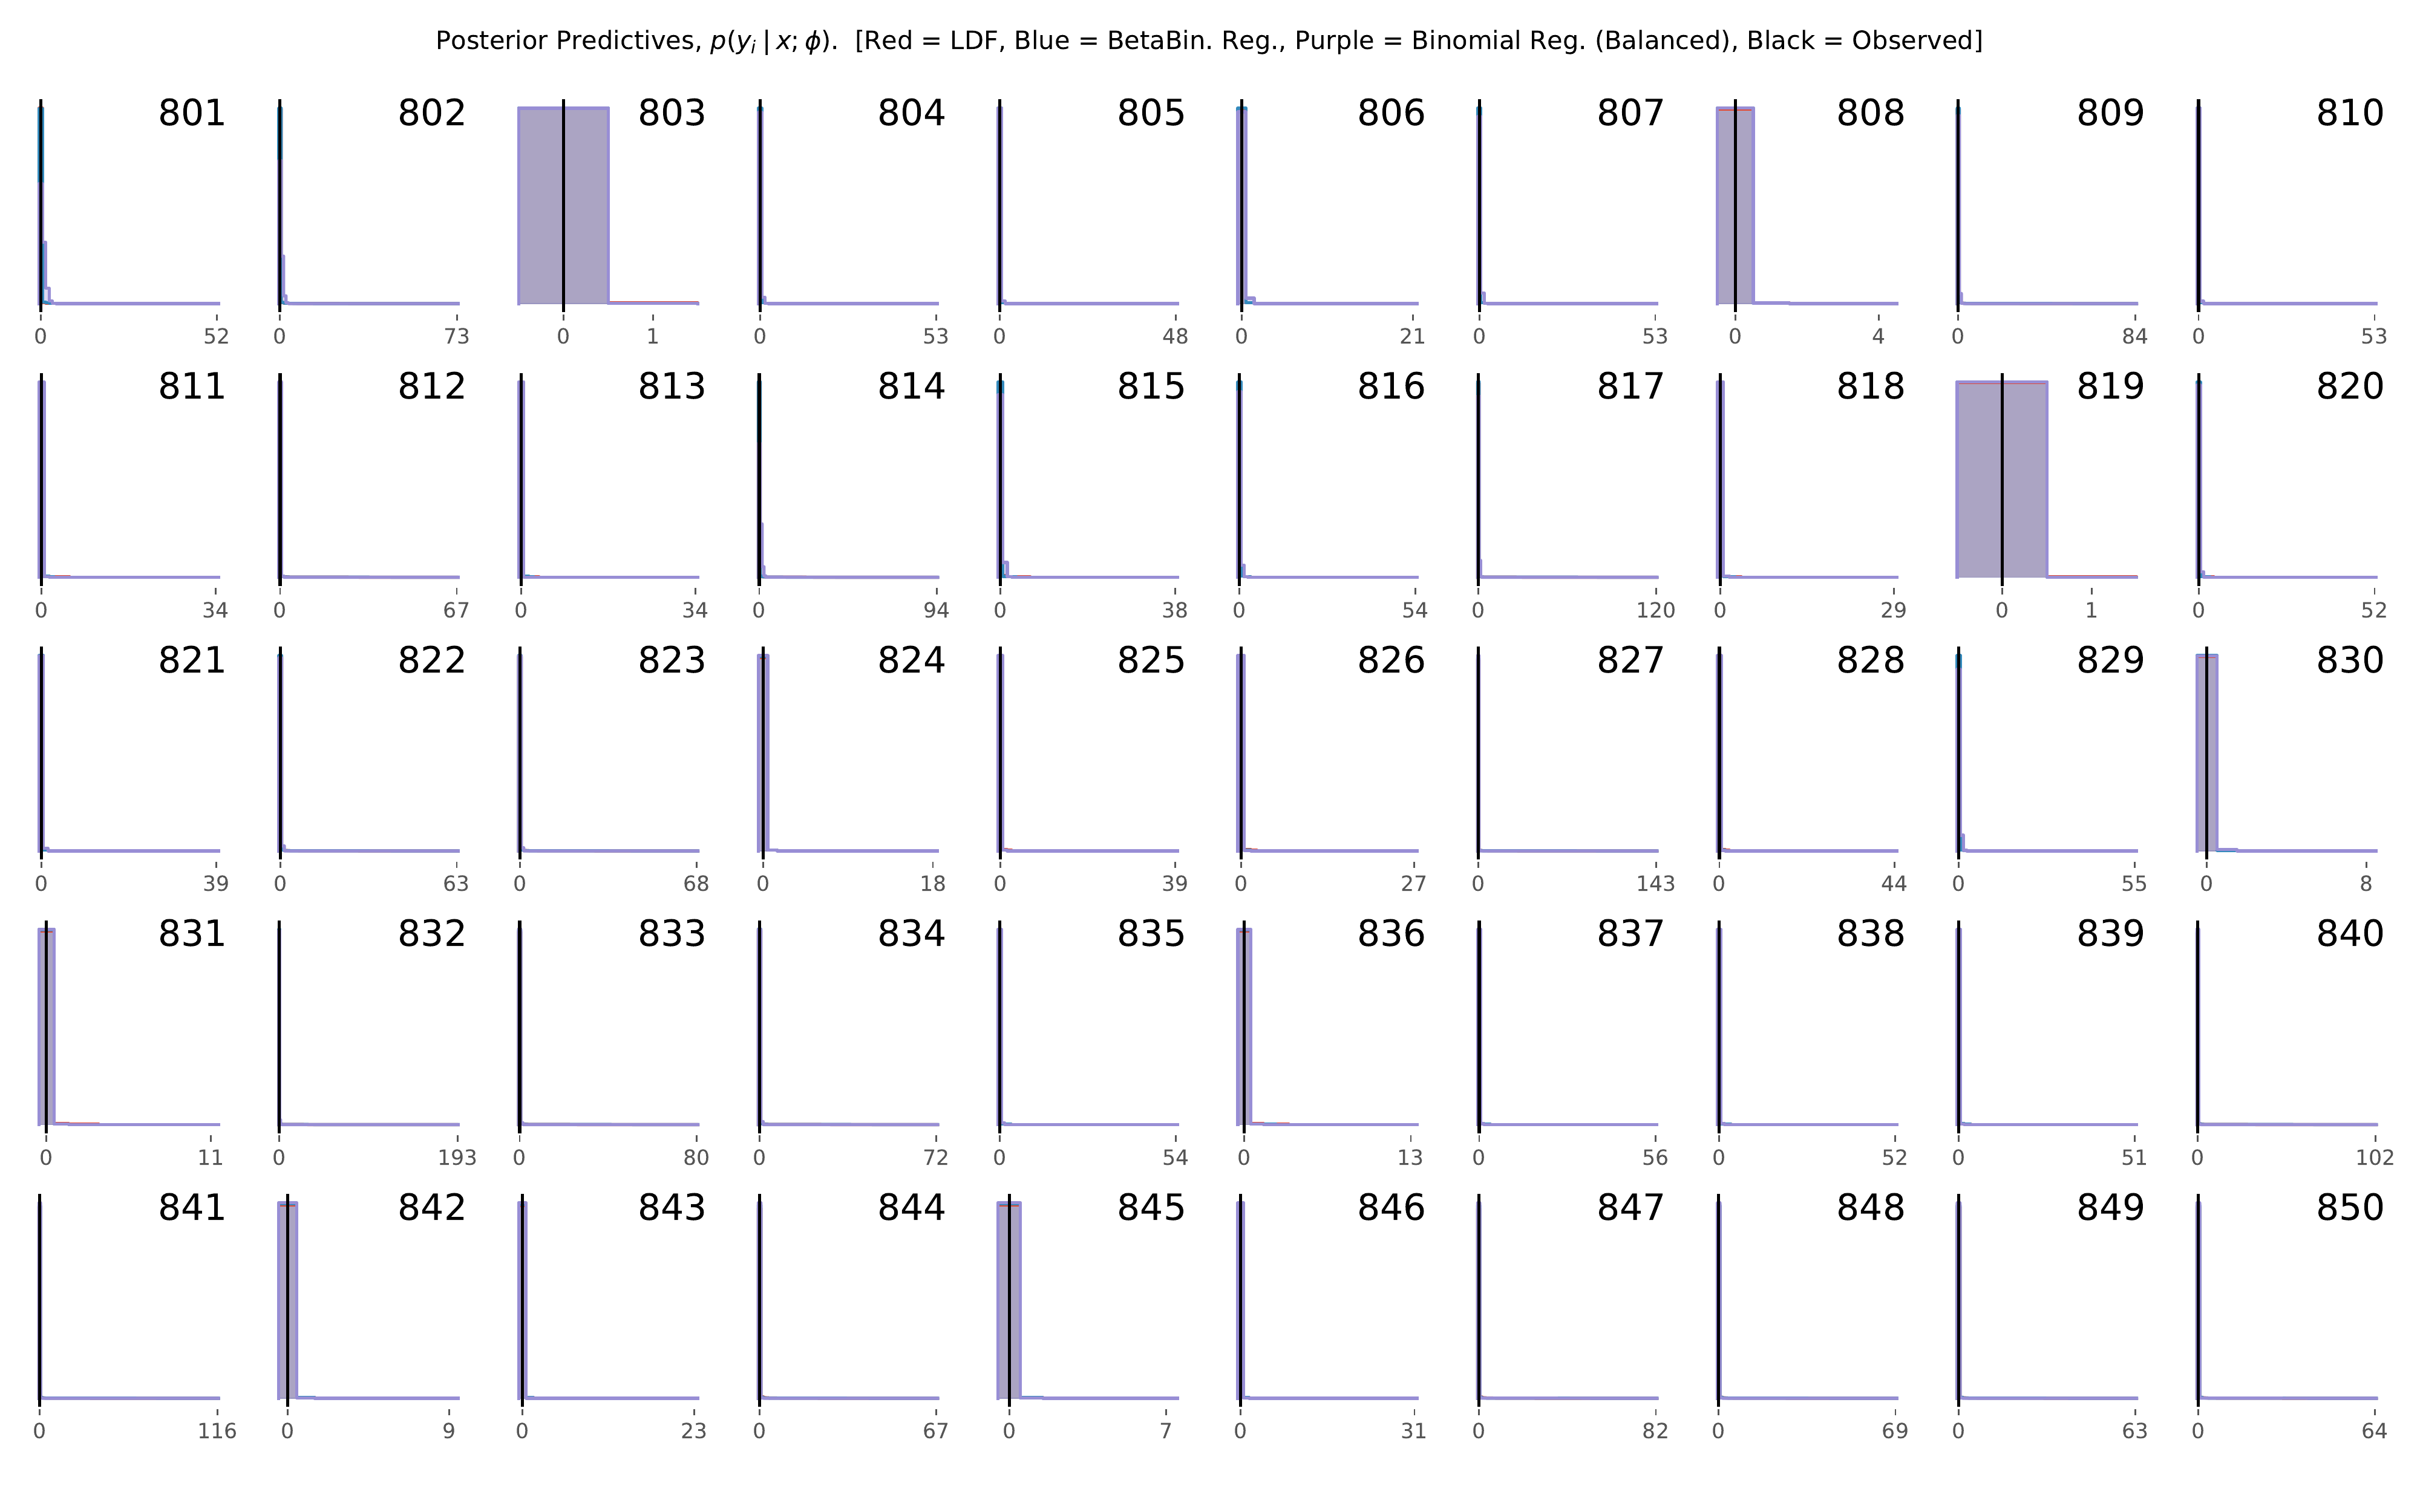}}
     \centerline{\includegraphics[width=0.75\linewidth, trim={0.375cm 19cm 0.375cm 1.5cm},clip]{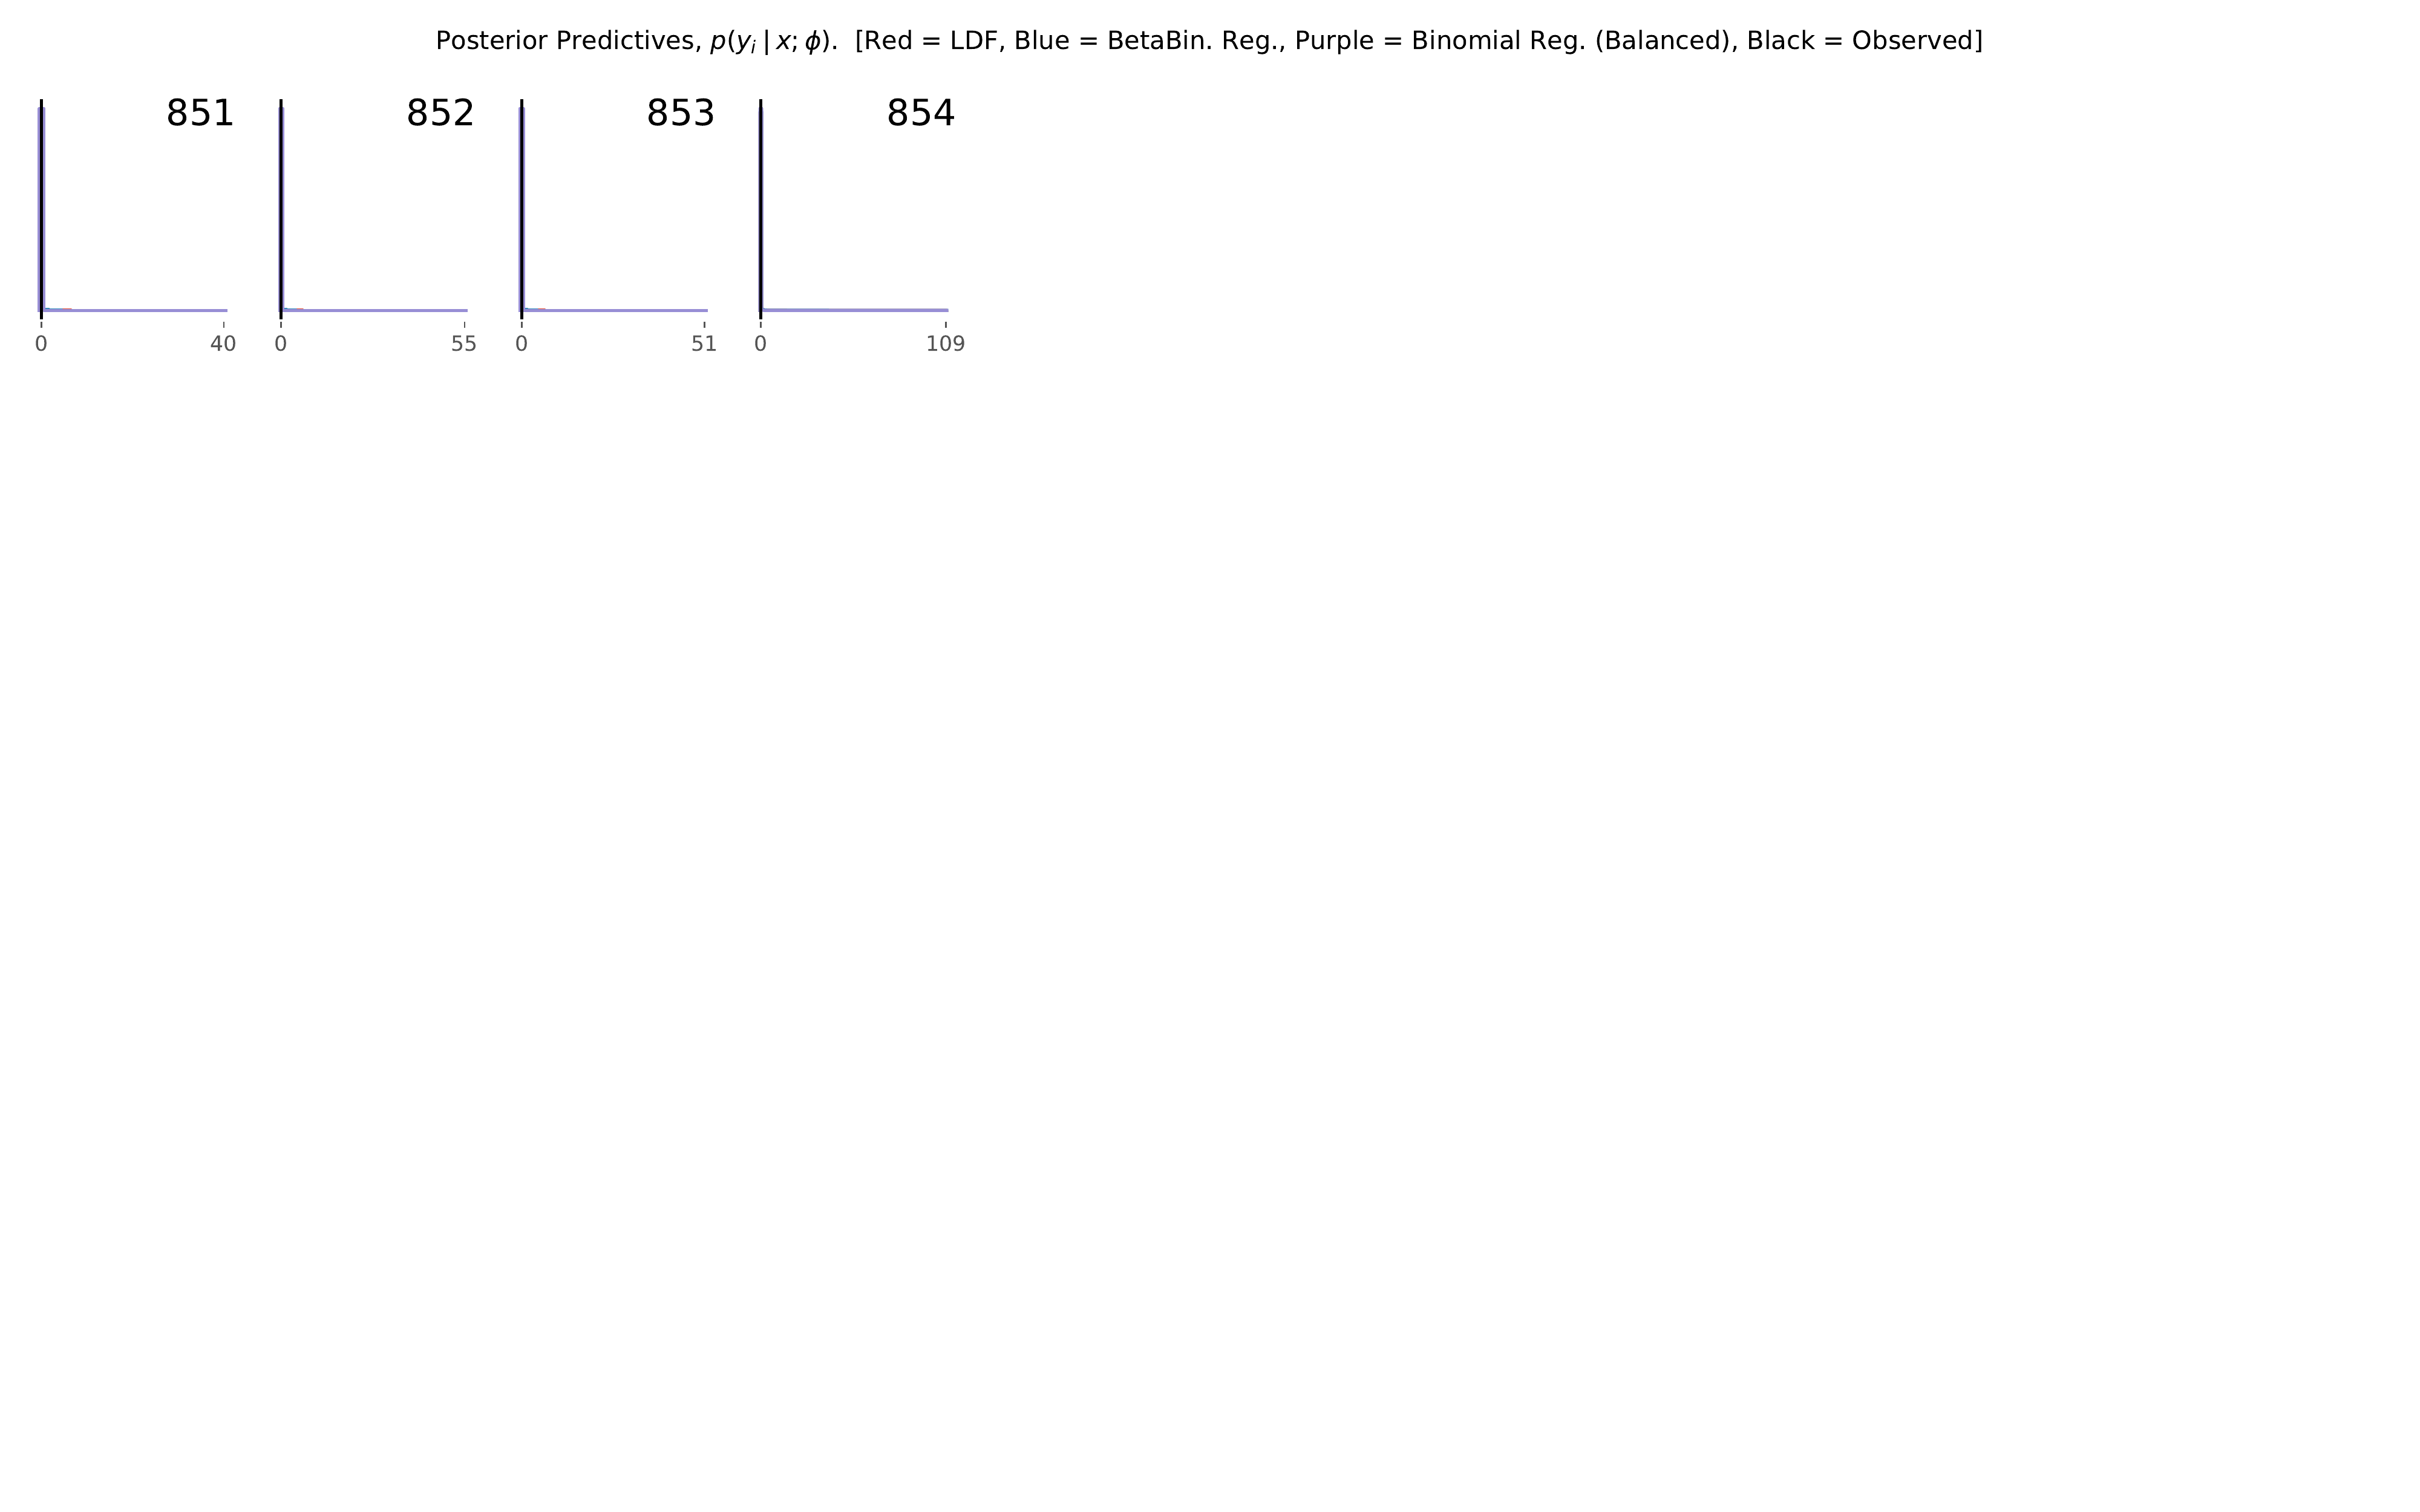}}
    \caption{\small \textbf{Primary data posterior predictives (continued).}  A subset of the predictive likelihoods $p(y_i \given x; \phi)$ for the electrification application.  LDF is red, beta-binomial regression is blue, binomial regression is purple, and the observed value is black.}
    \label{fig-supp-elec-predictive-end}
  \end{center}
  \vspace*{-5mm}
\end{figure}
